# Supplementary material for: Les Houches 2015: Physics at TeV Colliders Standard Model Working Group Report
Source: arXiv:1605.04692 source file (2016-05-16)
Supplement: Supplementary file 1 [file quarkgluon_fig_I2_GA_10_05_hadron_alphadep.pdf]

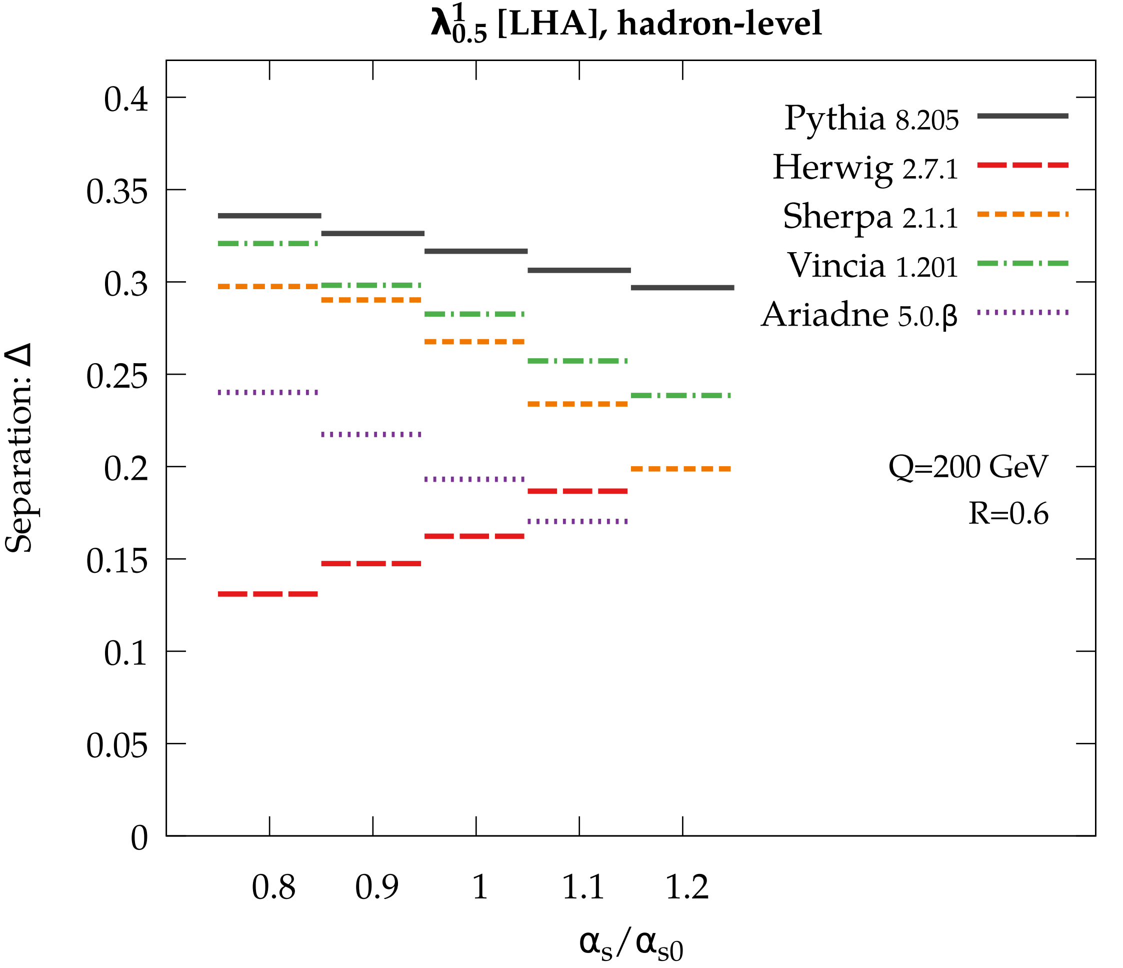

$\lambda^1_{0.5}$ [LHA], hadron-level
Pythia 8.205
Herwig 2.7.1
Sherpa 2.1.1
Vincia 1.201
Ariadne 5.0.β
Q=200 GeV
R=0.6
Separation: Δ
0.4
0.35
0.3
0.25
0.2
0.15
0.1
0.05
0
0.8
0.9
1
1.1
1.2
$\alpha_s/\alpha_{s0}$

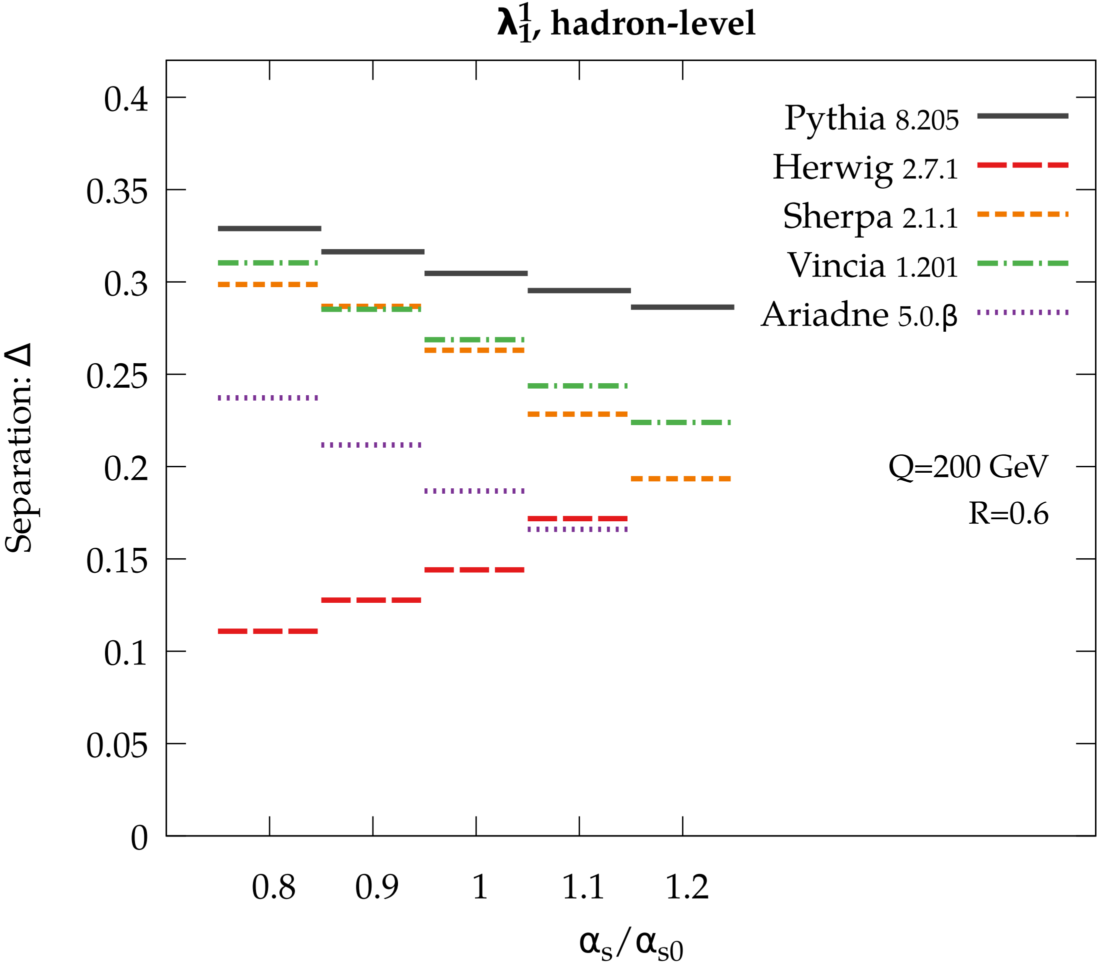

λ$_1^1$, hadron-level
Pythia 8.205
Herwig 2.7.1
Sherpa 2.1.1
Vincia 1.201
Ariadne 5.0.β
Q=200 GeV
R=0.6
Separation: Δ
0
0.05
0.1
0.15
0.2
0.25
0.3
0.35
0.4
0.8
0.9
1
1.1
1.2
$\alpha_s/\alpha_{s0}$

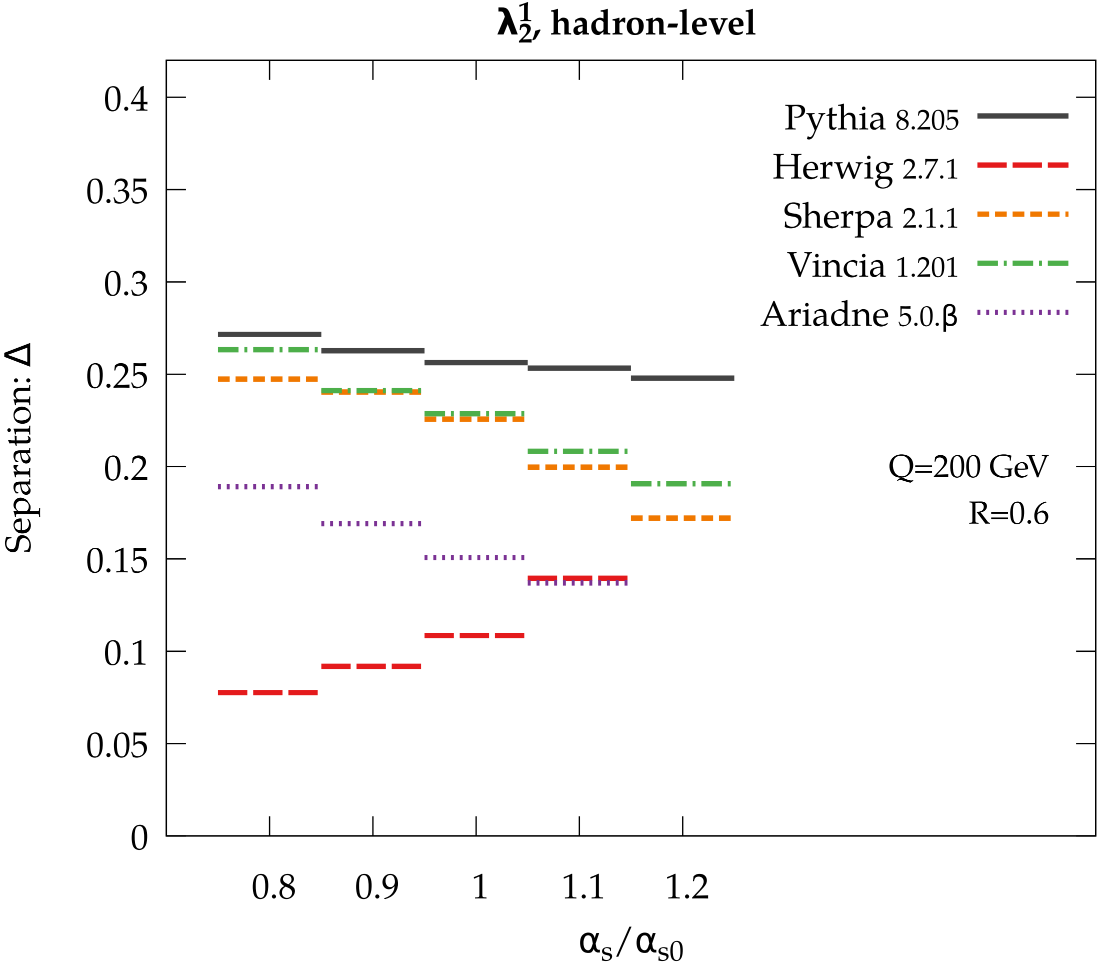

λ$_2^1$, hadron-level
Separation: Δ
0.4
0.35
0.3
0.25
0.2
0.15
0.1
0.05
0
0.8
0.9
1
1.1
1.2
αs/αs0
Pythia 8.205
Herwig 2.7.1
Sherpa 2.1.1
Vincia 1.201
Ariadne 5.0.β
Q=200 GeV
R=0.6

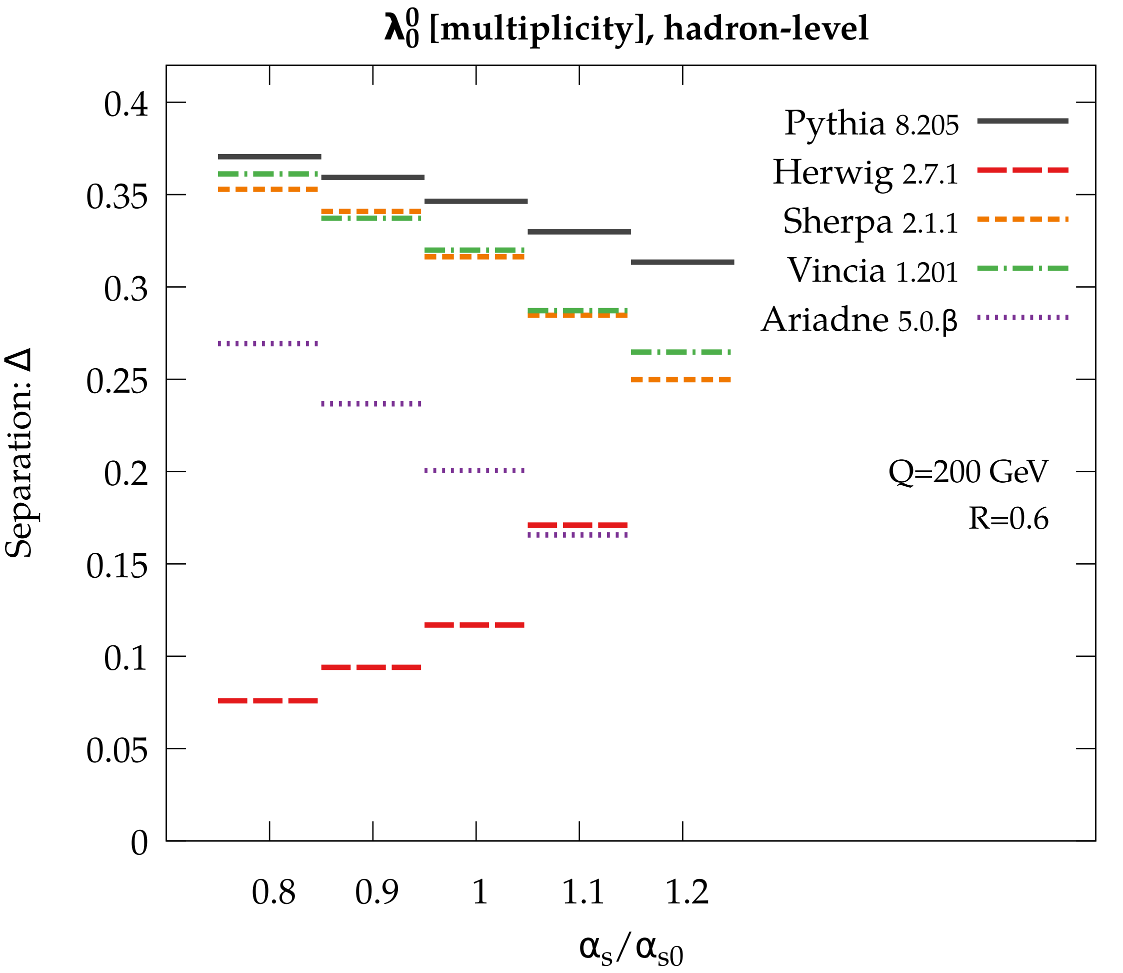

$\lambda_0^0$ [multiplicity], hadron-level
Pythia 8.205
Herwig 2.7.1
Sherpa 2.1.1
Vincia 1.201
Ariadne 5.0.β
Q=200 GeV
R=0.6
Separation: Δ
0.4
0.35
0.3
0.25
0.2
0.15
0.1
0.05
0
0.8
0.9
1
1.1
1.2
$\alpha_s/\alpha_{s0}$

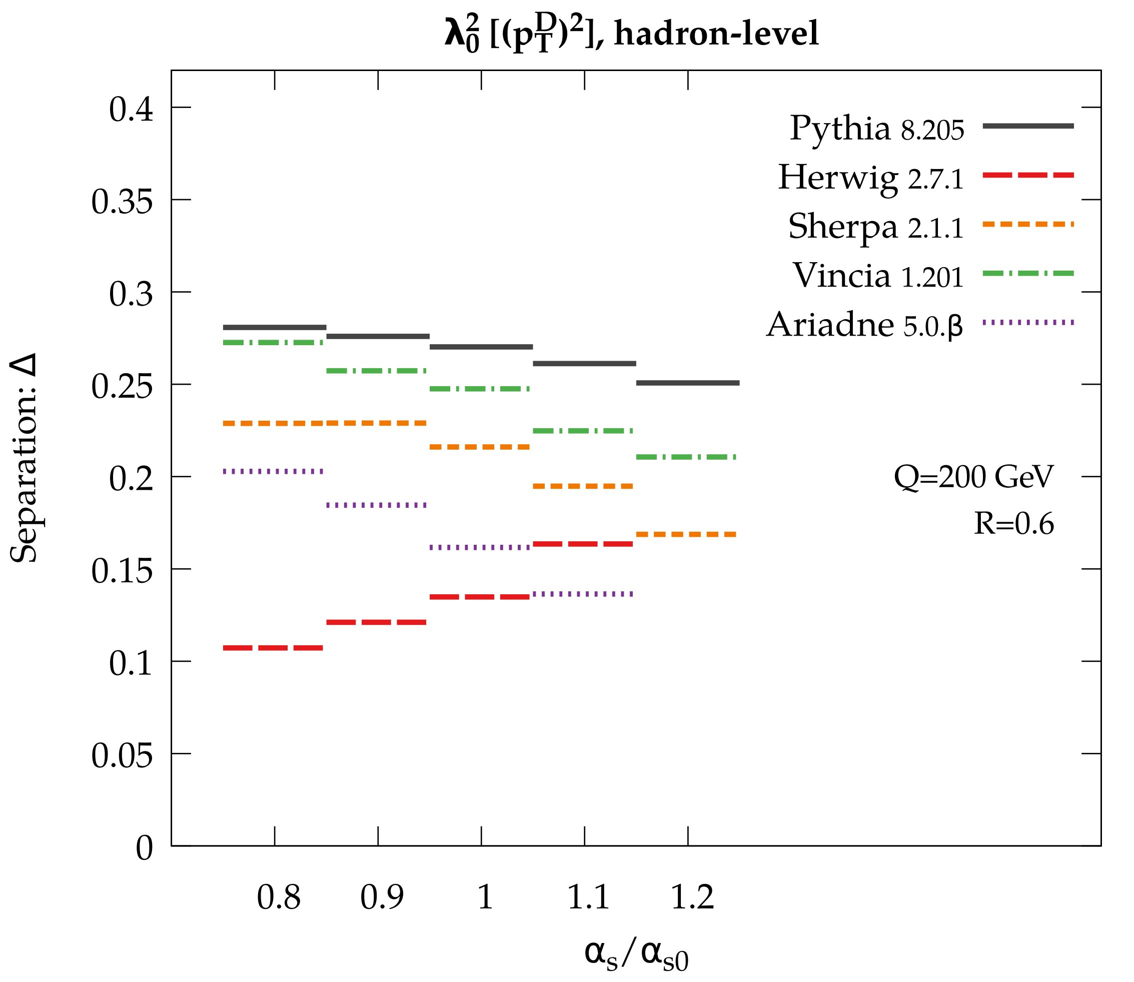

$\lambda_0^2$ [$(p_T^D)^2$], hadron-level
Pythia 8.205
Herwig 2.7.1
Sherpa 2.1.1
Vincia 1.201
Ariadne 5.0.β
Q=200 GeV
R=0.6
Separation: Δ
0.4
0.35
0.3
0.25
0.2
0.15
0.1
0.05
0
0.8
0.9
1
1.1
1.2
$\alpha_s/\alpha_{s0}$

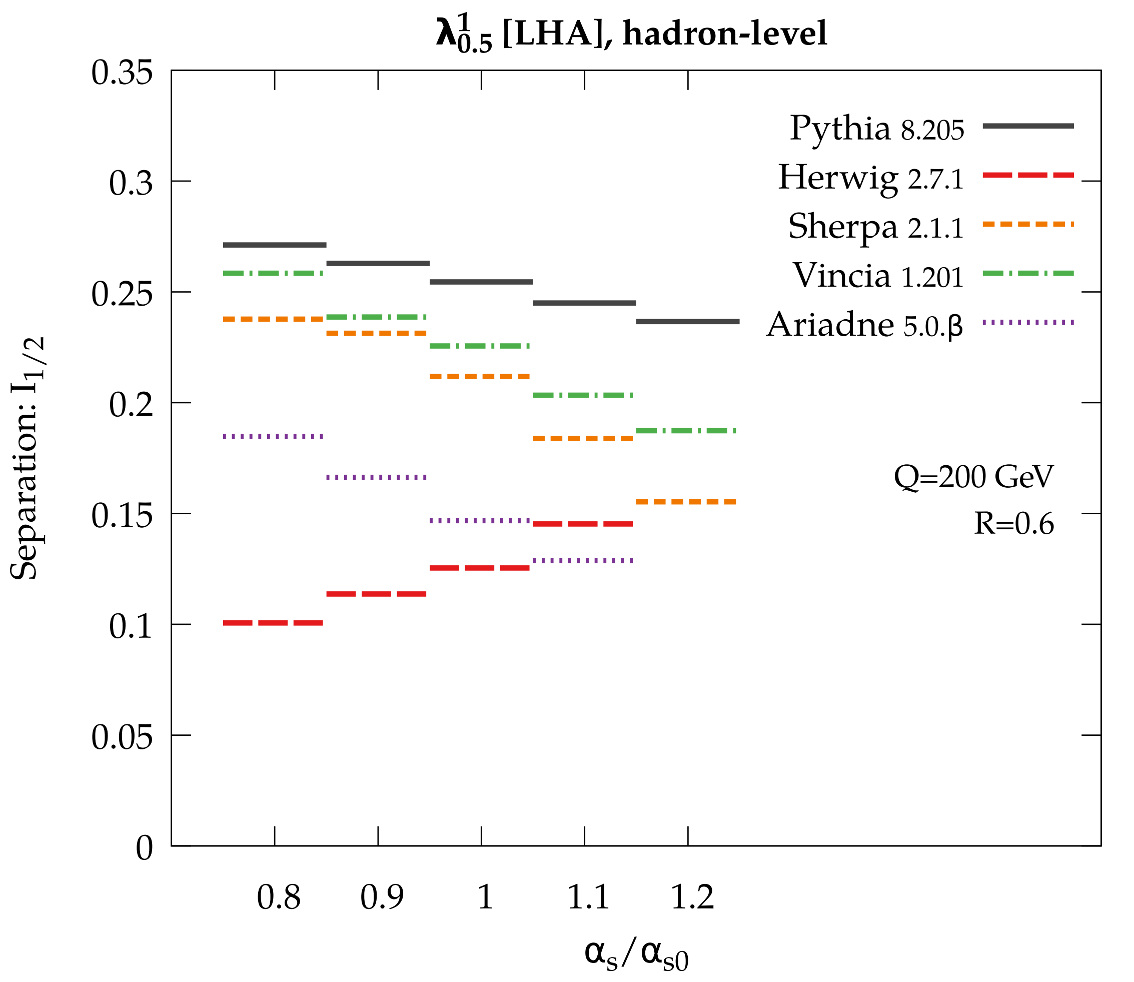

$\lambda^1_{0.5}$ [LHA], hadron-level
Separation: $I_{1/2}$
$\alpha_s/\alpha_{s0}$
0
0.05
0.1
0.15
0.2
0.25
0.3
0.35
0.8
0.9
1
1.1
1.2
Pythia 8.205
Herwig 2.7.1
Sherpa 2.1.1
Vincia 1.201
Ariadne 5.0.β
Q=200 GeV
R=0.6

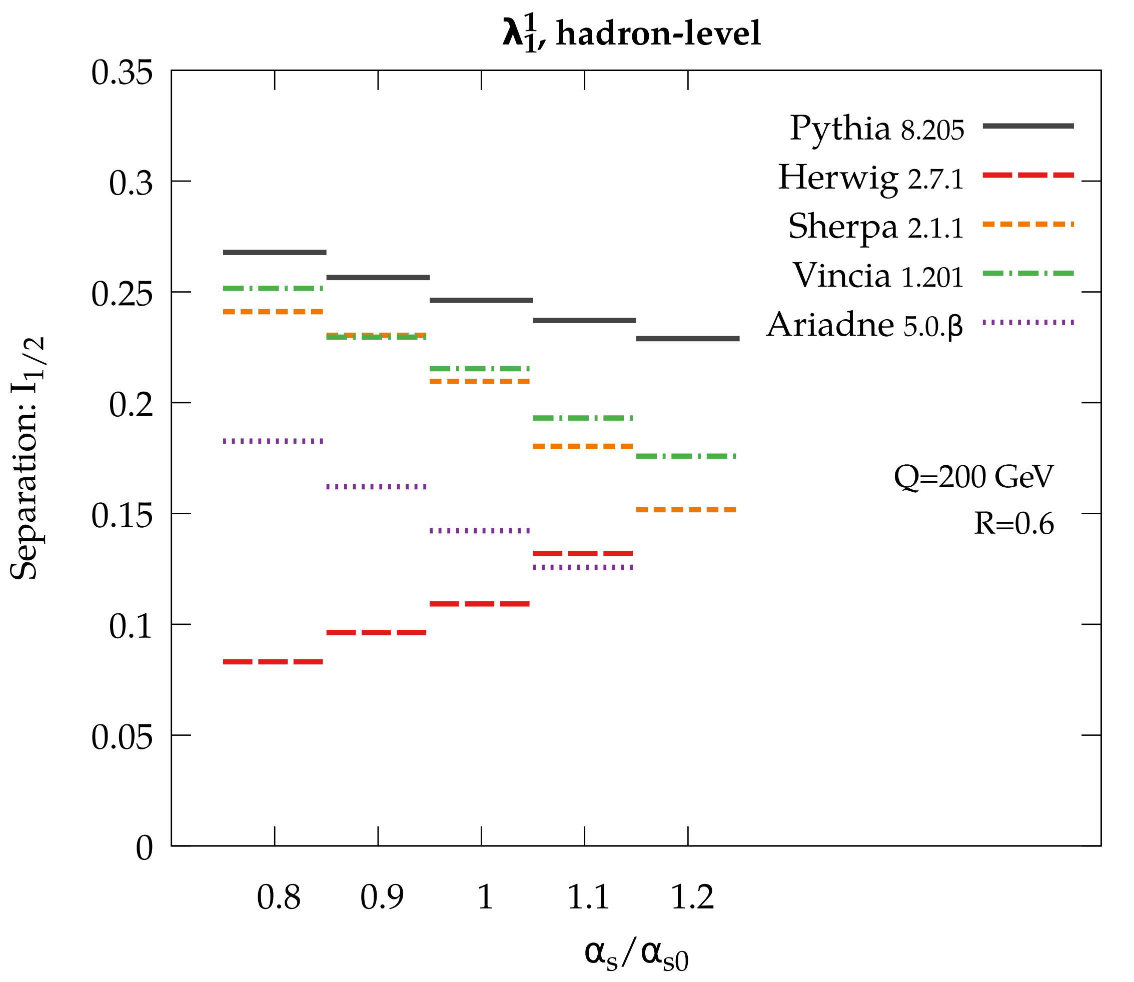

$\lambda_1^1$, hadron-level
Separation: $I_{1/2}$
0.35
0.3
0.25
0.2
0.15
0.1
0.05
0
0.8
0.9
1
1.1
1.2
$\alpha_s/\alpha_{s0}$
Pythia 8.205
Herwig 2.7.1
Sherpa 2.1.1
Vincia 1.201
Ariadne 5.0.β
Q=200 GeV
R=0.6

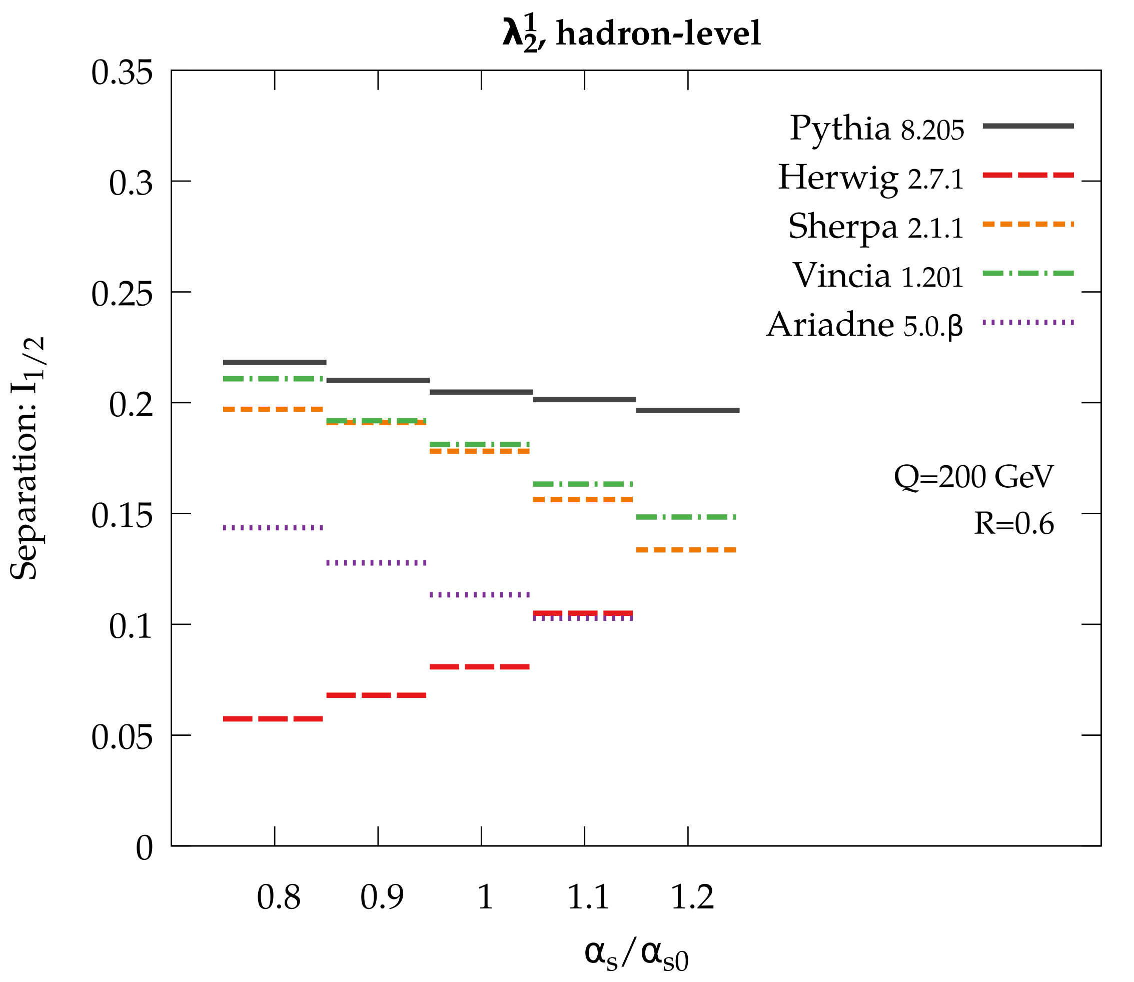

$\lambda_2^1$, hadron-level
Pythia 8.205
Herwig 2.7.1
Sherpa 2.1.1
Vincia 1.201
Ariadne 5.0.β
Q=200 GeV
R=0.6
Separation: $I_{1/2}$
$\alpha_s/\alpha_{s0}$
0
0.05
0.1
0.15
0.2
0.25
0.3
0.35
0.8
0.9
1
1.1
1.2

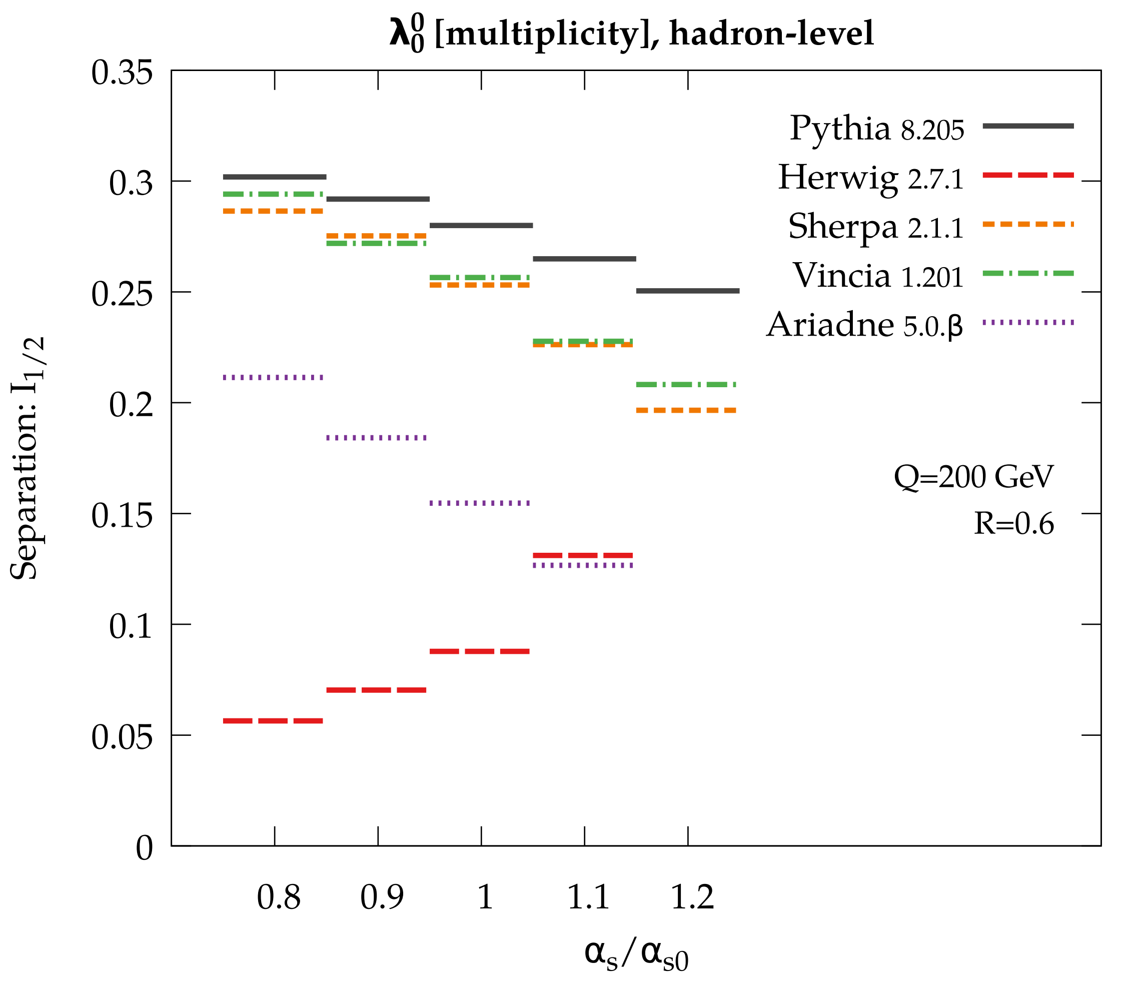

$\lambda_0^0$ [multiplicity], hadron-level
Separation: $I_{1/2}$
0.35
0.3
0.25
0.2
0.15
0.1
0.05
0
0.8
0.9
1
1.1
1.2
$\alpha_s/\alpha_{s0}$
Pythia 8.205
Herwig 2.7.1
Sherpa 2.1.1
Vincia 1.201
Ariadne 5.0.β
Q=200 GeV
R=0.6

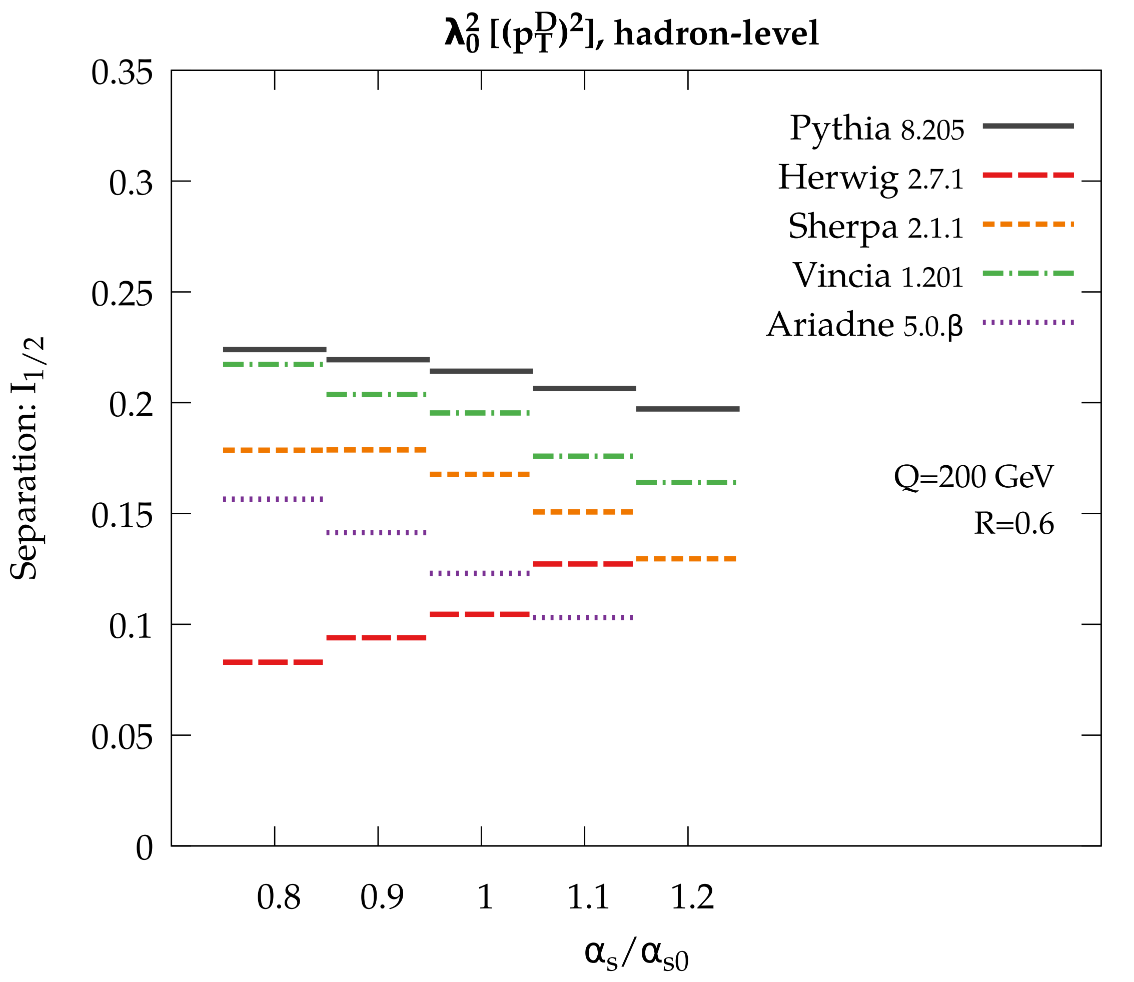

$\lambda_0^2$ $[(p_T^D)^2]$, hadron-level
Pythia 8.205
Herwig 2.7.1
Sherpa 2.1.1
Vincia 1.201
Ariadne 5.0.β
Q=200 GeV
R=0.6
Separation: $I_{1/2}$
$\alpha_s/\alpha_{s0}$
0.35
0.3
0.25
0.2
0.15
0.1
0.05
0
0.8
0.9
1
1.1
1.2

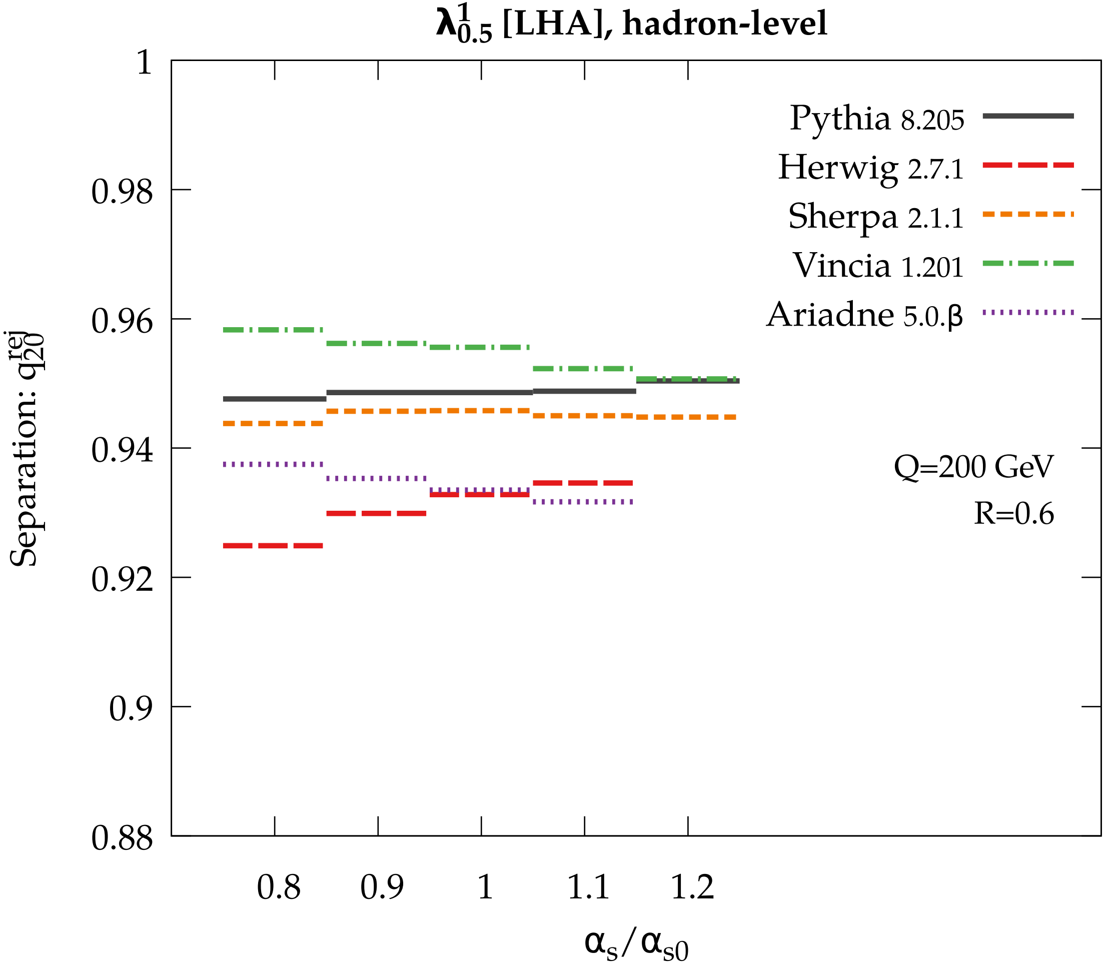
$\lambda_{0.5}^{1}$ [LHA], hadron-level
Separation: $q_{20}^{rej}$
$\alpha_s/\alpha_{s0}$
Pythia 8.205
Herwig 2.7.1
Sherpa 2.1.1
Vincia 1.201
Ariadne 5.0.β
Q=200 GeV
R=0.6
1
0.98
0.96
0.94
0.92
0.9
0.88
0.8
0.9
1
1.1
1.2

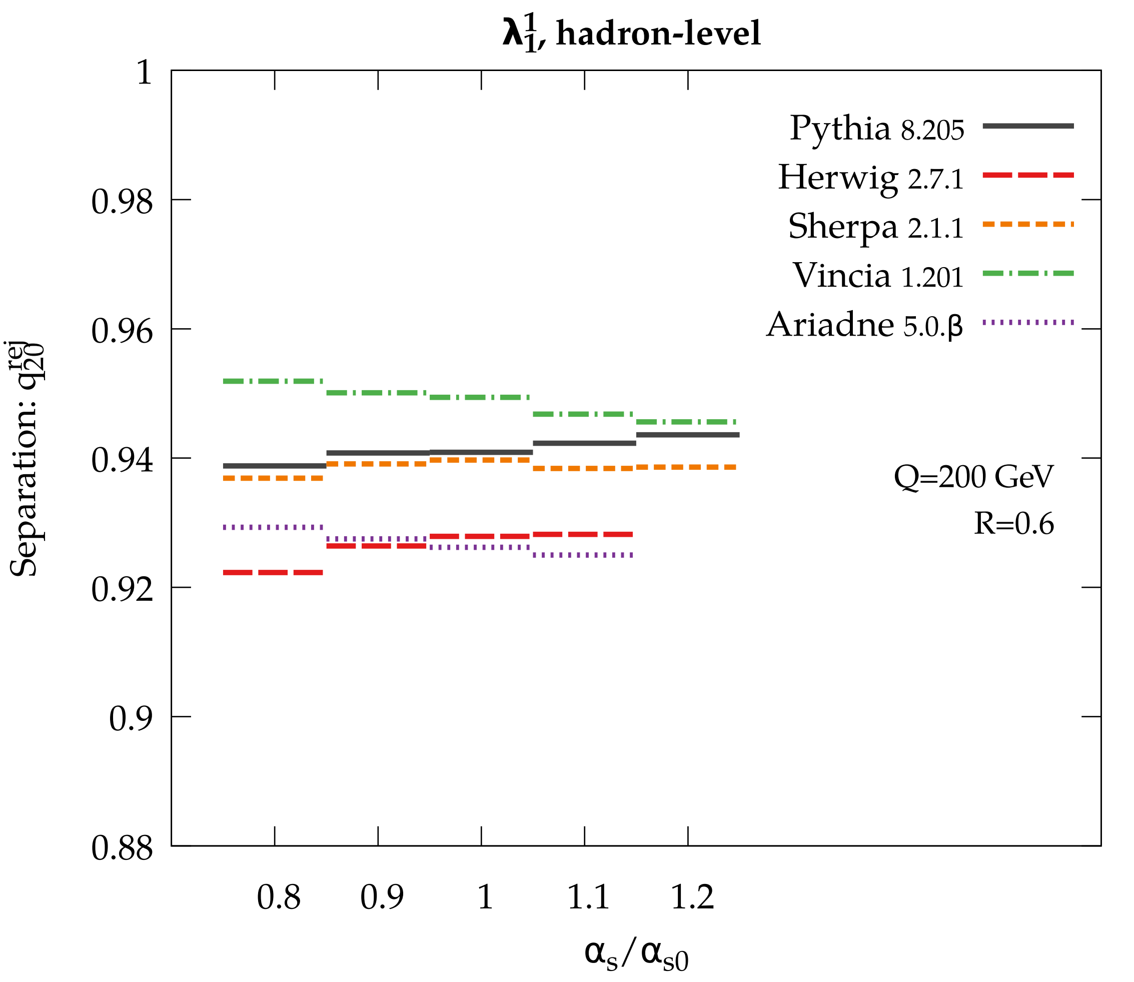
$\lambda_1^1$, hadron-level
Pythia 8.205
Herwig 2.7.1
Sherpa 2.1.1
Vincia 1.201
Ariadne 5.0.β
Q=200 GeV
R=0.6
Separation: $q_{20}^{rej}$
$\alpha_s/\alpha_{s0}$
1
0.98
0.96
0.94
0.92
0.9
0.88
0.8
0.9
1
1.1
1.2

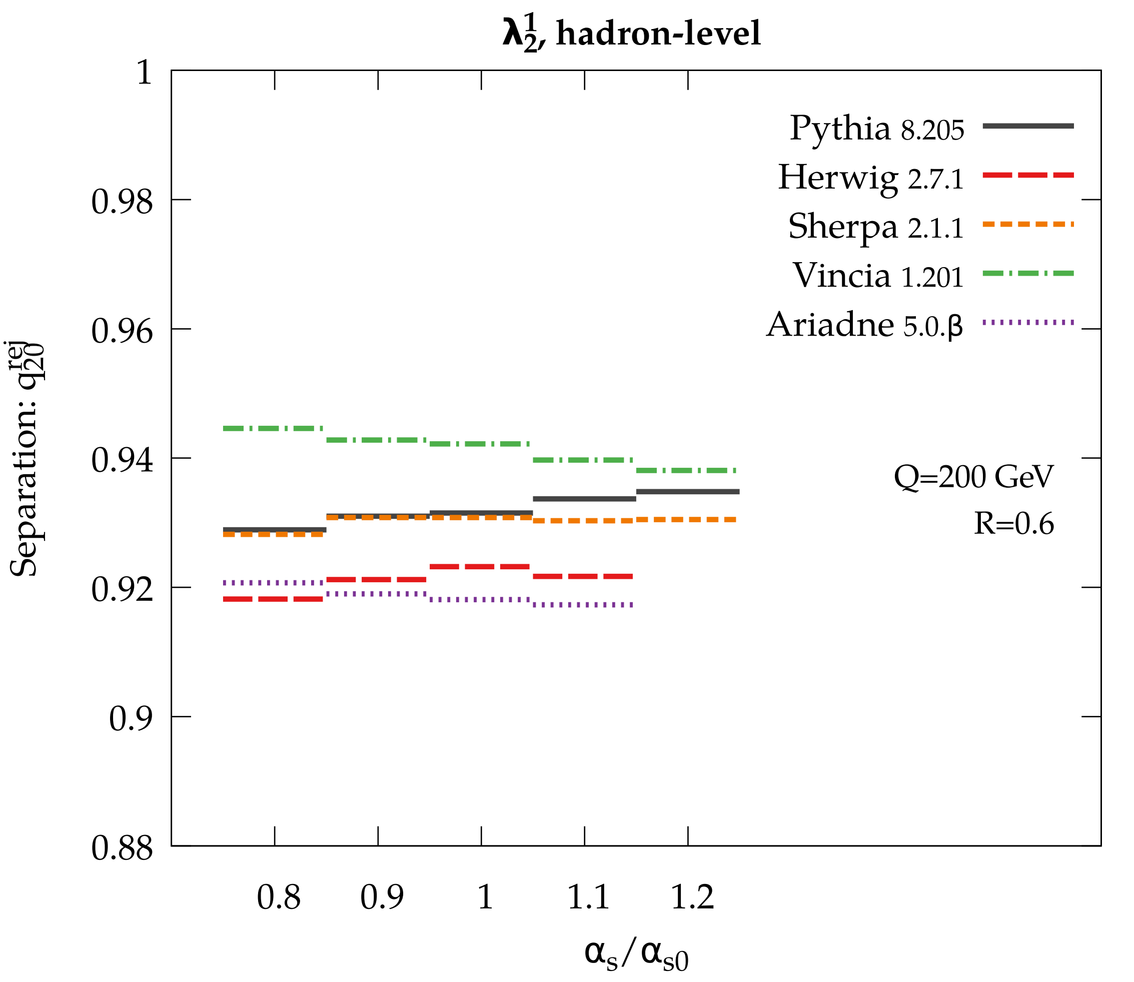

λ_2^1, hadron-level
Separation: q_20^rej
α_s/α_s0
Pythia 8.205
Herwig 2.7.1
Sherpa 2.1.1
Vincia 1.201
Ariadne 5.0.β
Q=200 GeV
R=0.6
1
0.98
0.96
0.94
0.92
0.9
0.88
0.8
0.9
1
1.1
1.2

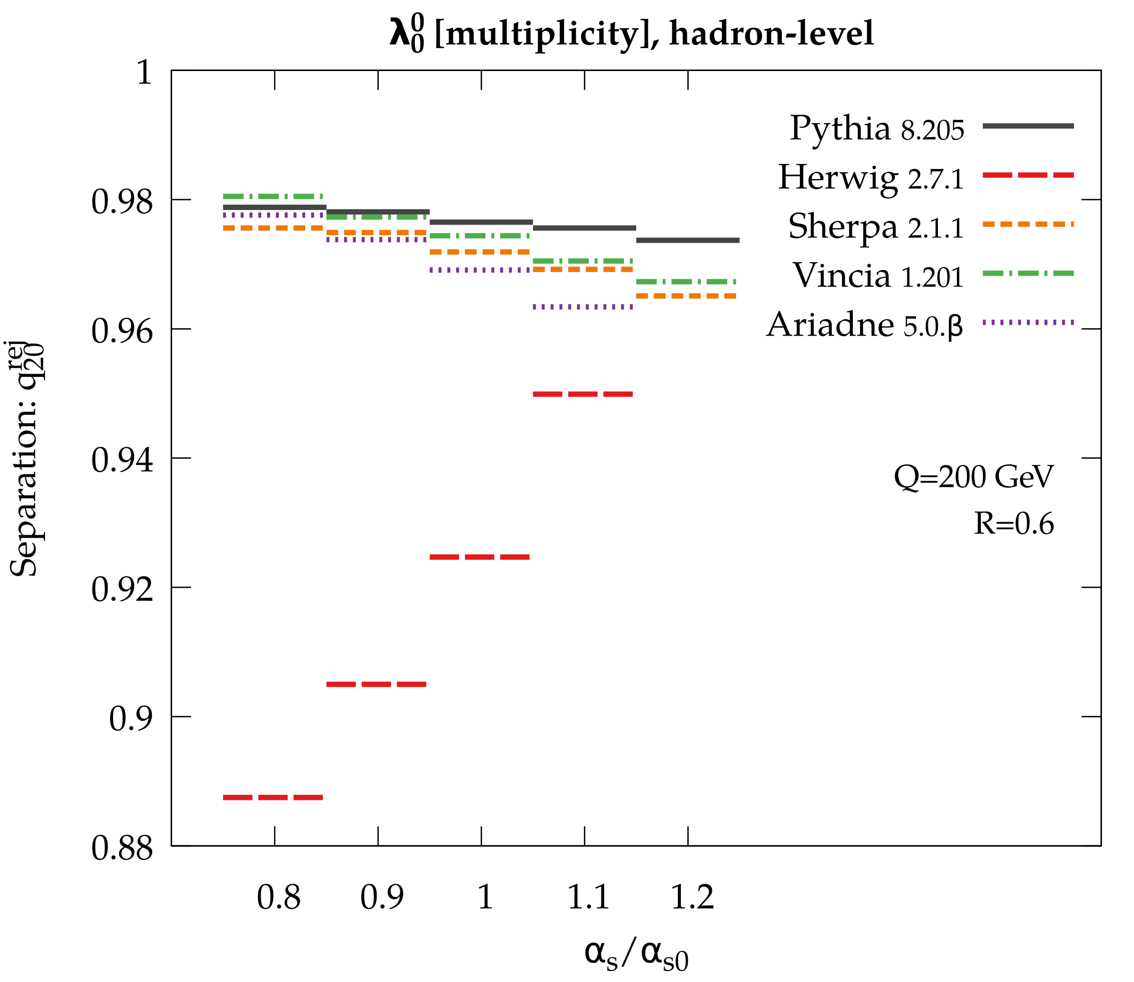

$\lambda_0^0$ [multiplicity], hadron-level
Pythia 8.205
Herwig 2.7.1
Sherpa 2.1.1
Vincia 1.201
Ariadne 5.0.β
Q=200 GeV
R=0.6
Separation: $q_{20}^{rej}$
1
0.98
0.96
0.94
0.92
0.9
0.88
0.8
0.9
1
1.1
1.2
$\alpha_s/\alpha_{s0}$

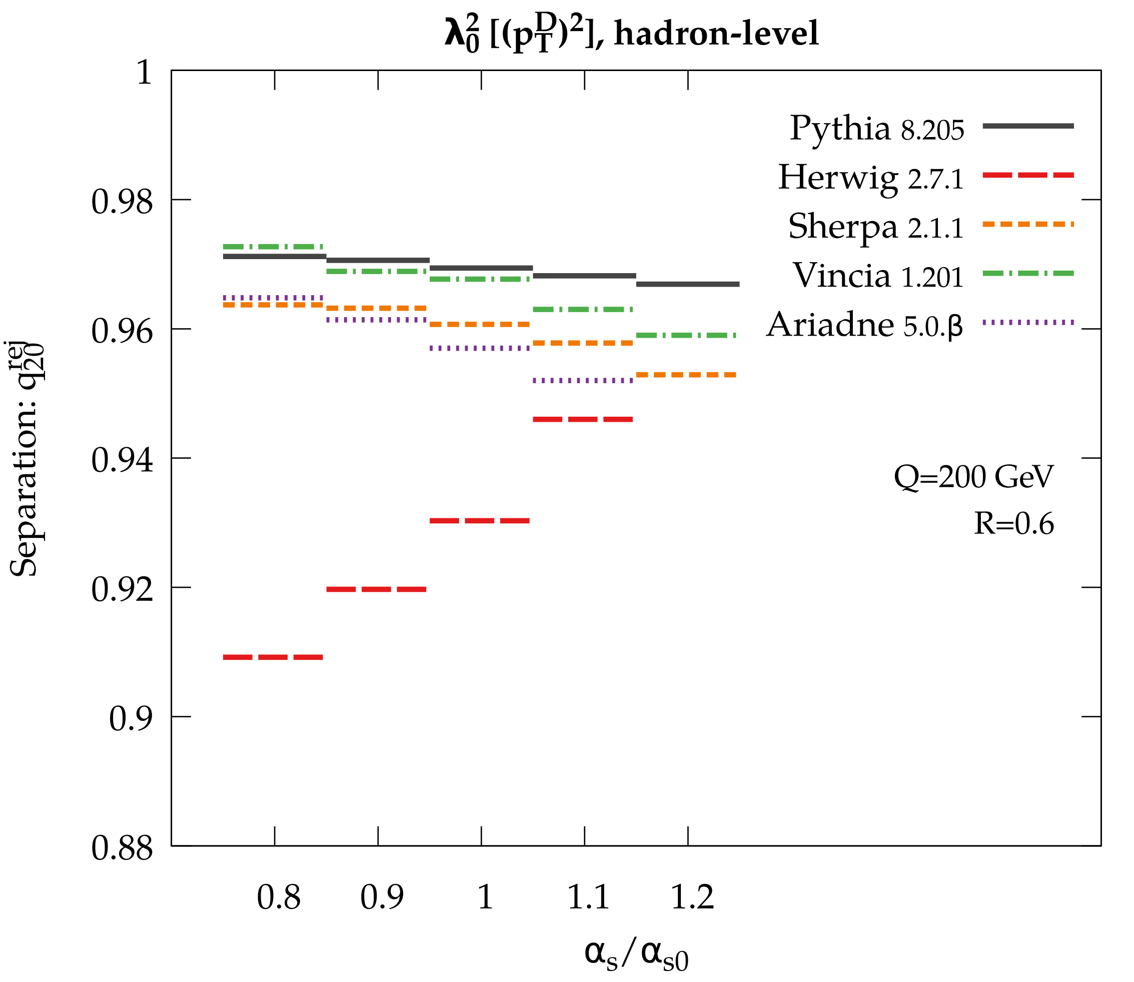

$\lambda_0^2$ [$(p_T^D)^2$], hadron-level
Pythia 8.205
Herwig 2.7.1
Sherpa 2.1.1
Vincia 1.201
Ariadne 5.0.β
Q=200 GeV
R=0.6
Separation: $q_{20}^{rej}$
1
0.98
0.96
0.94
0.92
0.9
0.88
0.8
0.9
1
1.1
1.2
$\alpha_s/\alpha_{s0}$

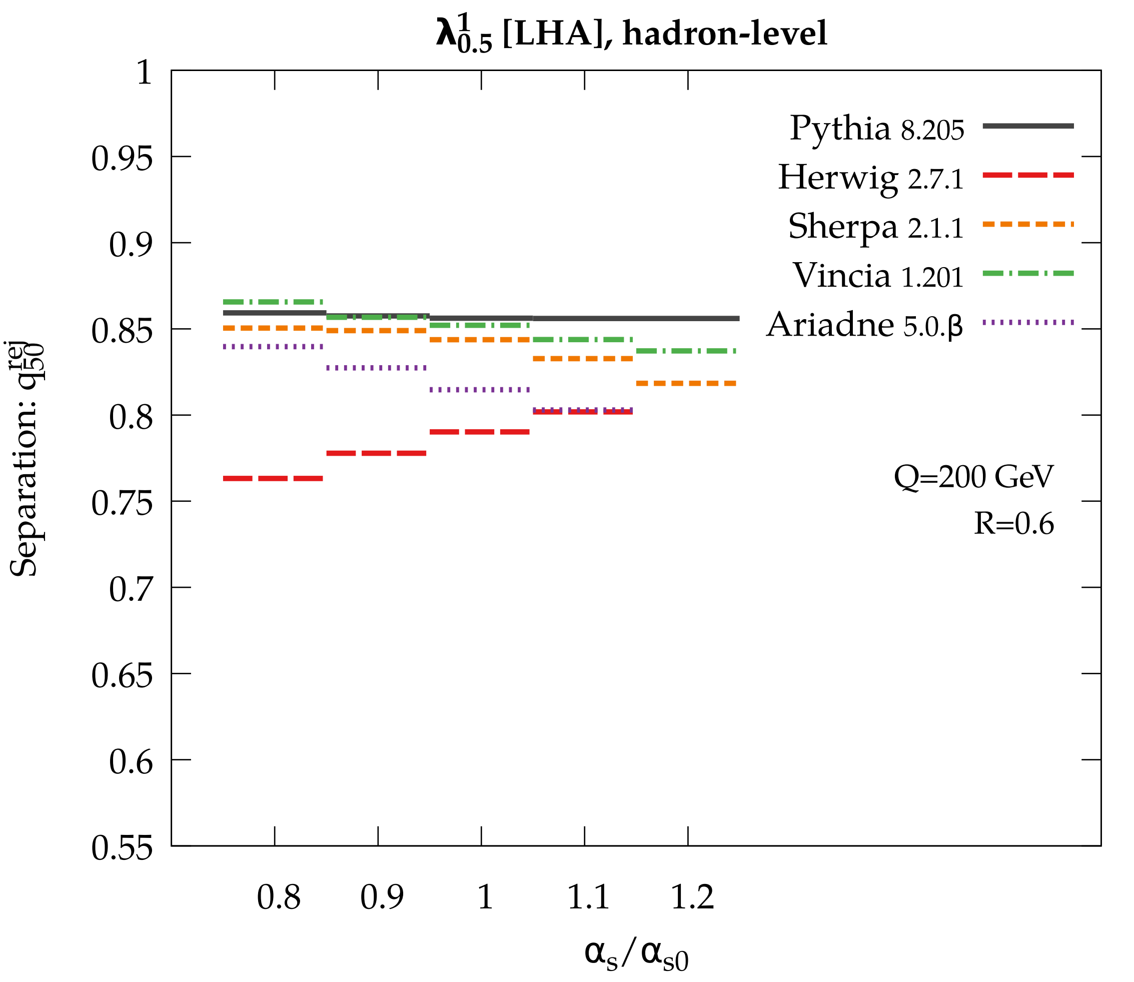

$\lambda^1_{0.5}$ [LHA], hadron-level
Pythia 8.205
Herwig 2.7.1
Sherpa 2.1.1
Vincia 1.201
Ariadne 5.0.β
Q=200 GeV
R=0.6
Separation: $q^{rej}_{50}$
$\alpha_s/\alpha_{s0}$
1
0.95
0.9
0.85
0.8
0.75
0.7
0.65
0.6
0.55
0.8
0.9
1
1.1
1.2

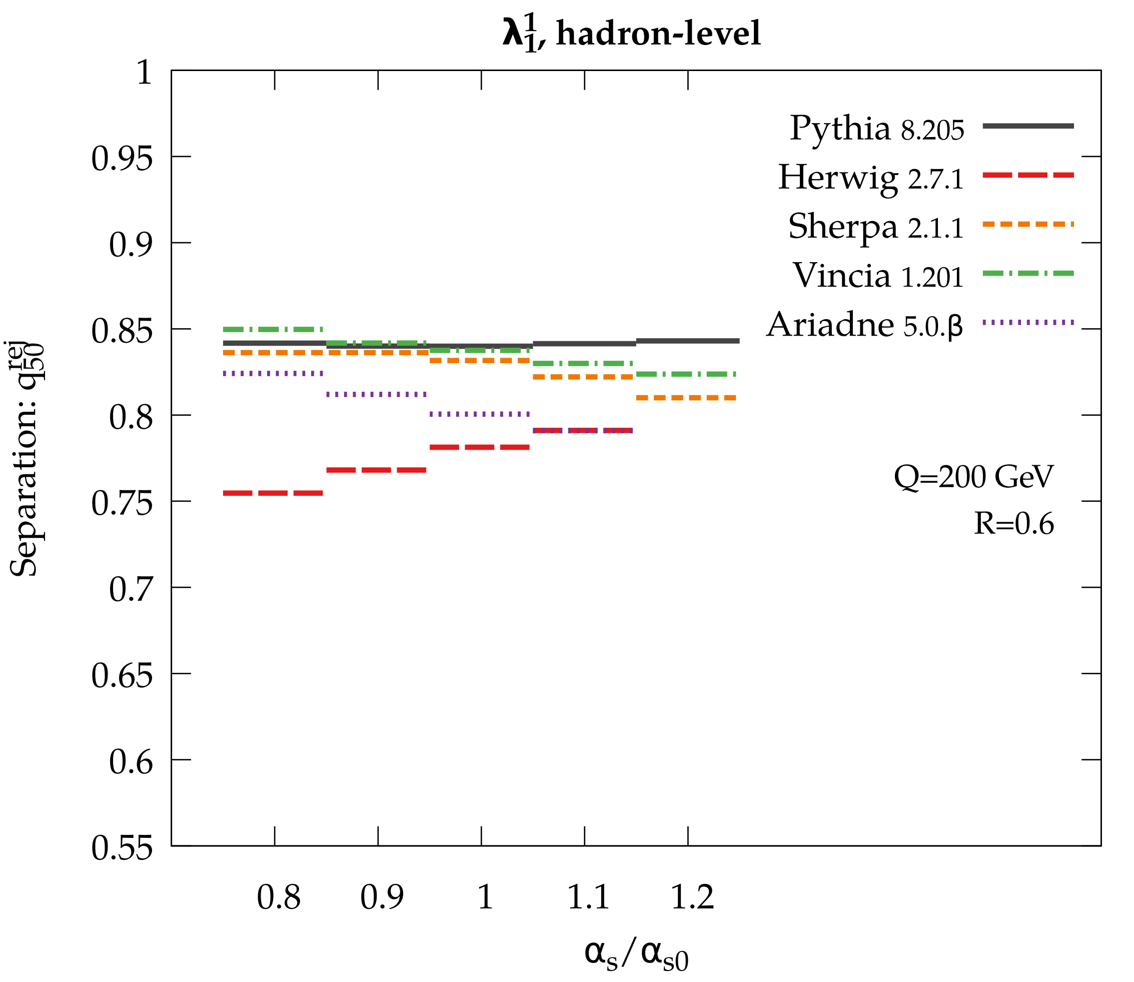

$\lambda_1^1$, hadron-level
Separation: $q_{50}^{rej}$
$\alpha_s/\alpha_{s0}$
1
0.95
0.9
0.85
0.8
0.75
0.7
0.65
0.6
0.55
0.8
0.9
1
1.1
1.2
Pythia 8.205
Herwig 2.7.1
Sherpa 2.1.1
Vincia 1.201
Ariadne 5.0.β
Q=200 GeV
R=0.6

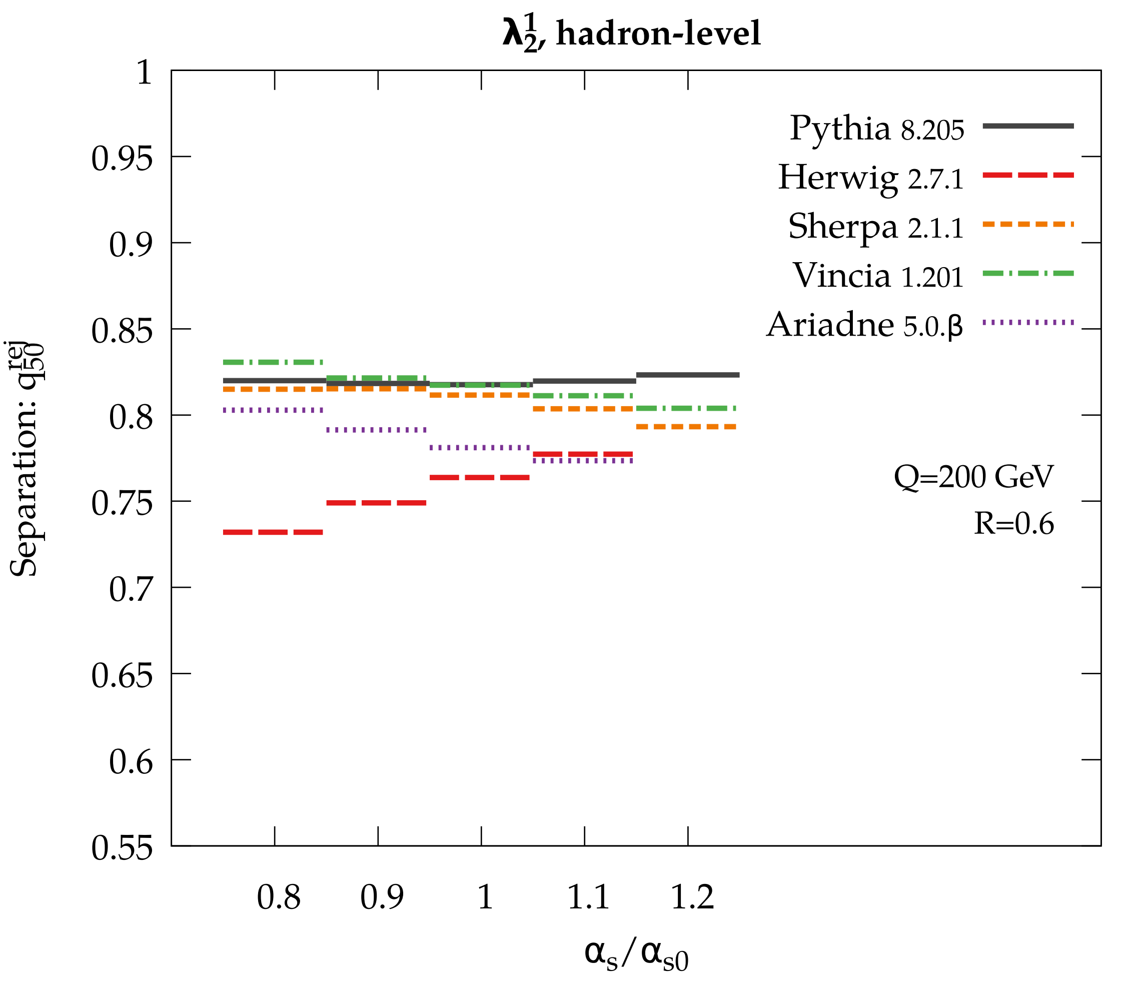

$\lambda_2^1$, hadron-level
Pythia 8.205
Herwig 2.7.1
Sherpa 2.1.1
Vincia 1.201
Ariadne 5.0.β
Q=200 GeV
R=0.6
Separation: $q_{50}^{rej}$
$\alpha_s/\alpha_{s0}$
1
0.95
0.9
0.85
0.8
0.75
0.7
0.65
0.6
0.55
0.8
0.9
1
1.1
1.2

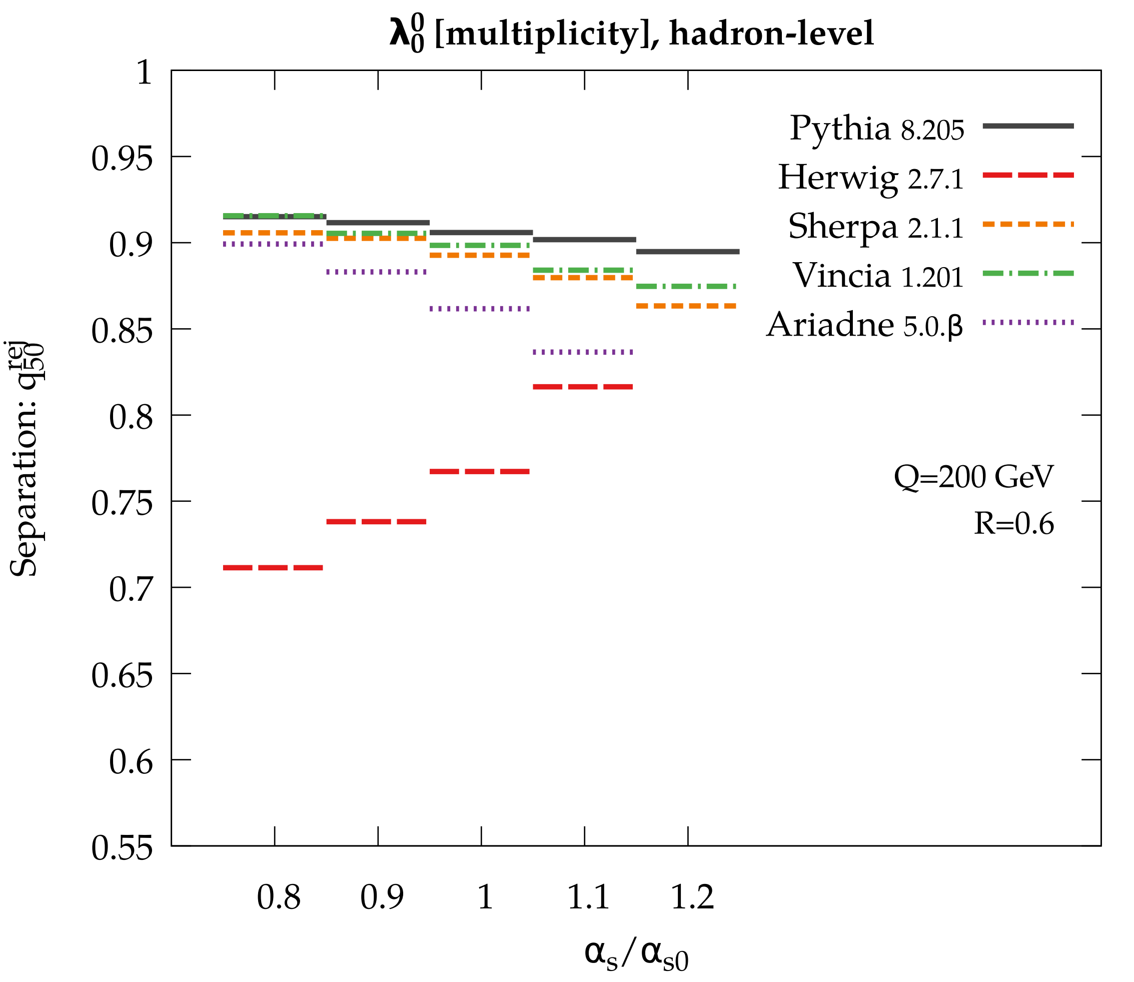

$\lambda_0^0$ [multiplicity], hadron-level
Separation: $q_{50}^{rej}$
$\alpha_s/\alpha_{s0}$
Pythia 8.205
Herwig 2.7.1
Sherpa 2.1.1
Vincia 1.201
Ariadne 5.0.β
Q=200 GeV
R=0.6
1
0.95
0.9
0.85
0.8
0.75
0.7
0.65
0.6
0.55
0.8
0.9
1
1.1
1.2

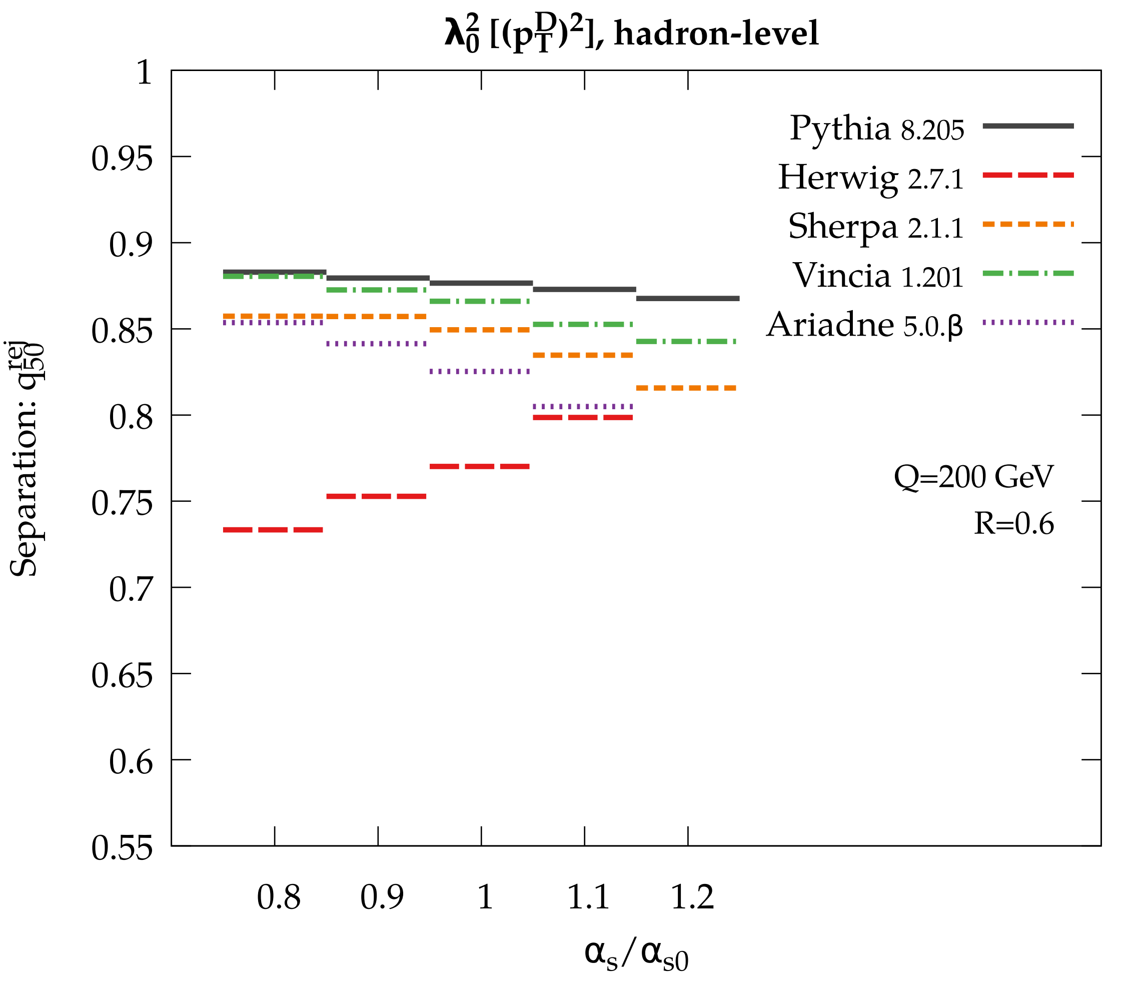

$\lambda_0^2$ [$(p_T^D)^2$], hadron-level
Separation: $q_{50}^{rej}$
$\alpha_s/\alpha_{s0}$
1
0.95
0.9
0.85
0.8
0.75
0.7
0.65
0.6
0.55
0.8
0.9
1
1.1
1.2
Pythia 8.205
Herwig 2.7.1
Sherpa 2.1.1
Vincia 1.201
Ariadne 5.0.β
Q=200 GeV
R=0.6

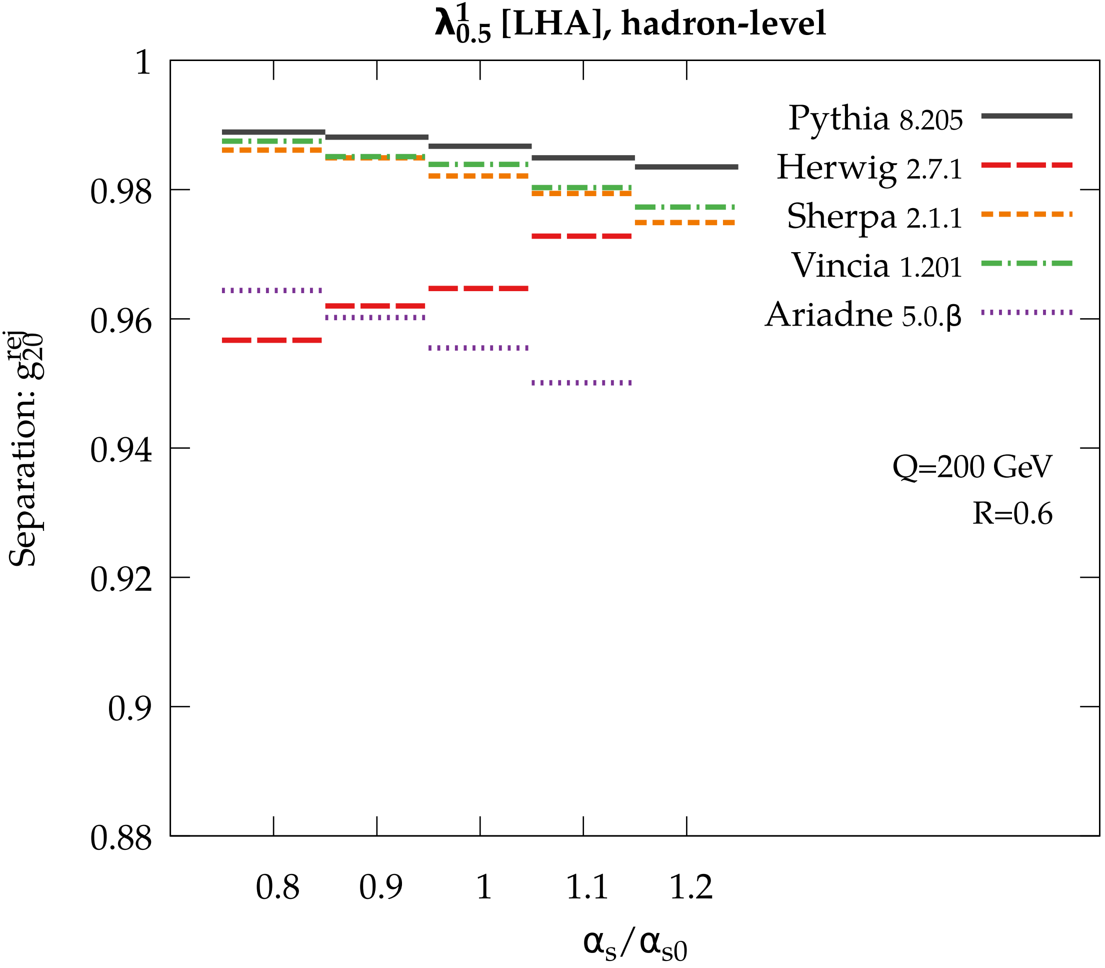

$\lambda^1_{0.5}$ [LHA], hadron-level
Pythia 8.205
Herwig 2.7.1
Sherpa 2.1.1
Vincia 1.201
Ariadne 5.0.β
Q=200 GeV
R=0.6
Separation: $g^{rej}_{20}$
1
0.98
0.96
0.94
0.92
0.9
0.88
0.8
0.9
1
1.1
1.2
$\alpha_s/\alpha_{s0}$

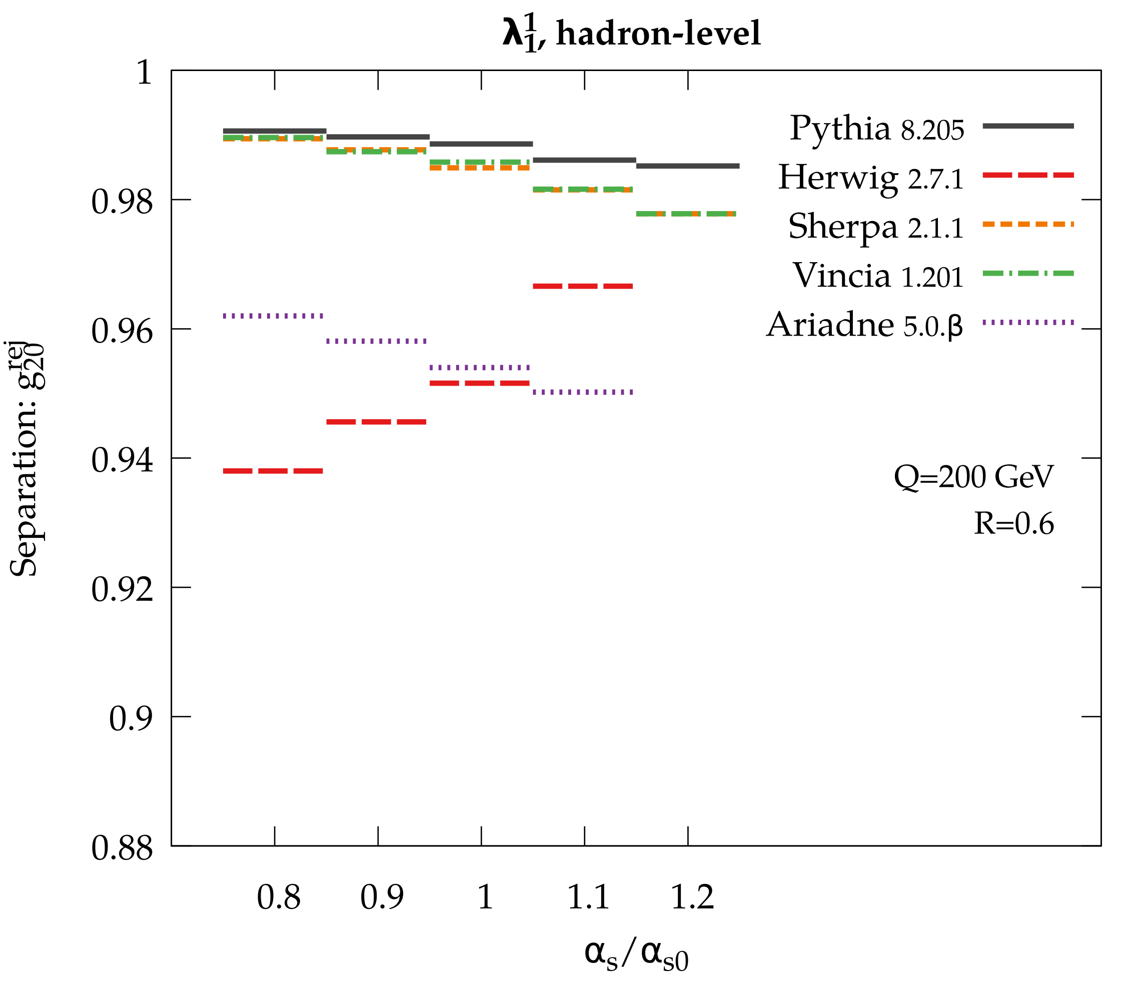

$\lambda_1^1$, hadron-level
Pythia 8.205
Herwig 2.7.1
Sherpa 2.1.1
Vincia 1.201
Ariadne 5.0.β
Q=200 GeV
R=0.6
Separation: $g_{20}^{rej}$
$\alpha_s/\alpha_{s0}$
1
0.98
0.96
0.94
0.92
0.9
0.88
0.8
0.9
1
1.1
1.2

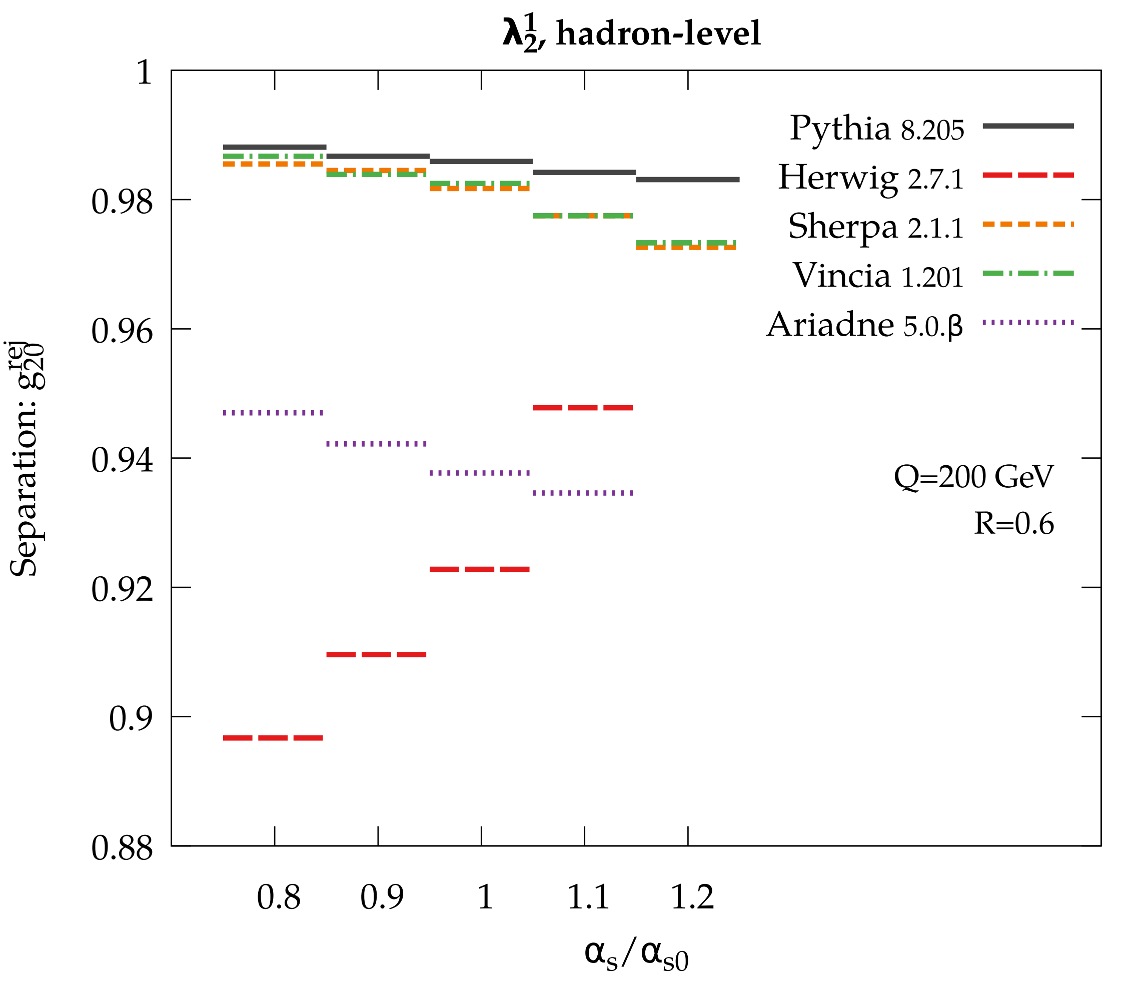

$\lambda_2^1$, hadron-level
Pythia 8.205
Herwig 2.7.1
Sherpa 2.1.1
Vincia 1.201
Ariadne 5.0.β
Q=200 GeV
R=0.6
Separation: $g_{20}^{rej}$
$\alpha_s/\alpha_{s0}$
1
0.98
0.96
0.94
0.92
0.9
0.88
0.8
0.9
1
1.1
1.2

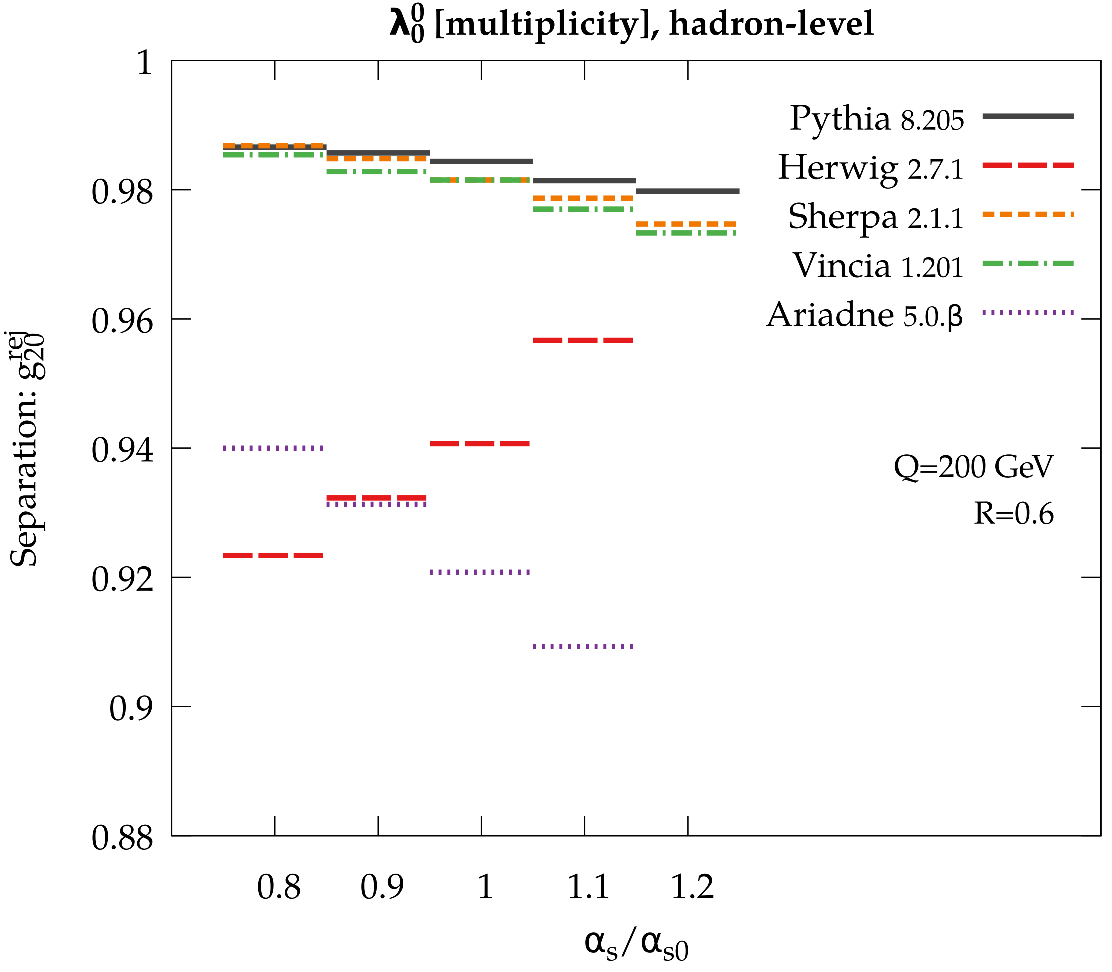

$\lambda_0^0$ [multiplicity], hadron-level
Separation: $g_{20}^{rej}$
$\alpha_s/\alpha_{s0}$
1
0.98
0.96
0.94
0.92
0.9
0.88
0.8
0.9
1
1.1
1.2
Pythia 8.205
Herwig 2.7.1
Sherpa 2.1.1
Vincia 1.201
Ariadne 5.0.β
Q=200 GeV
R=0.6

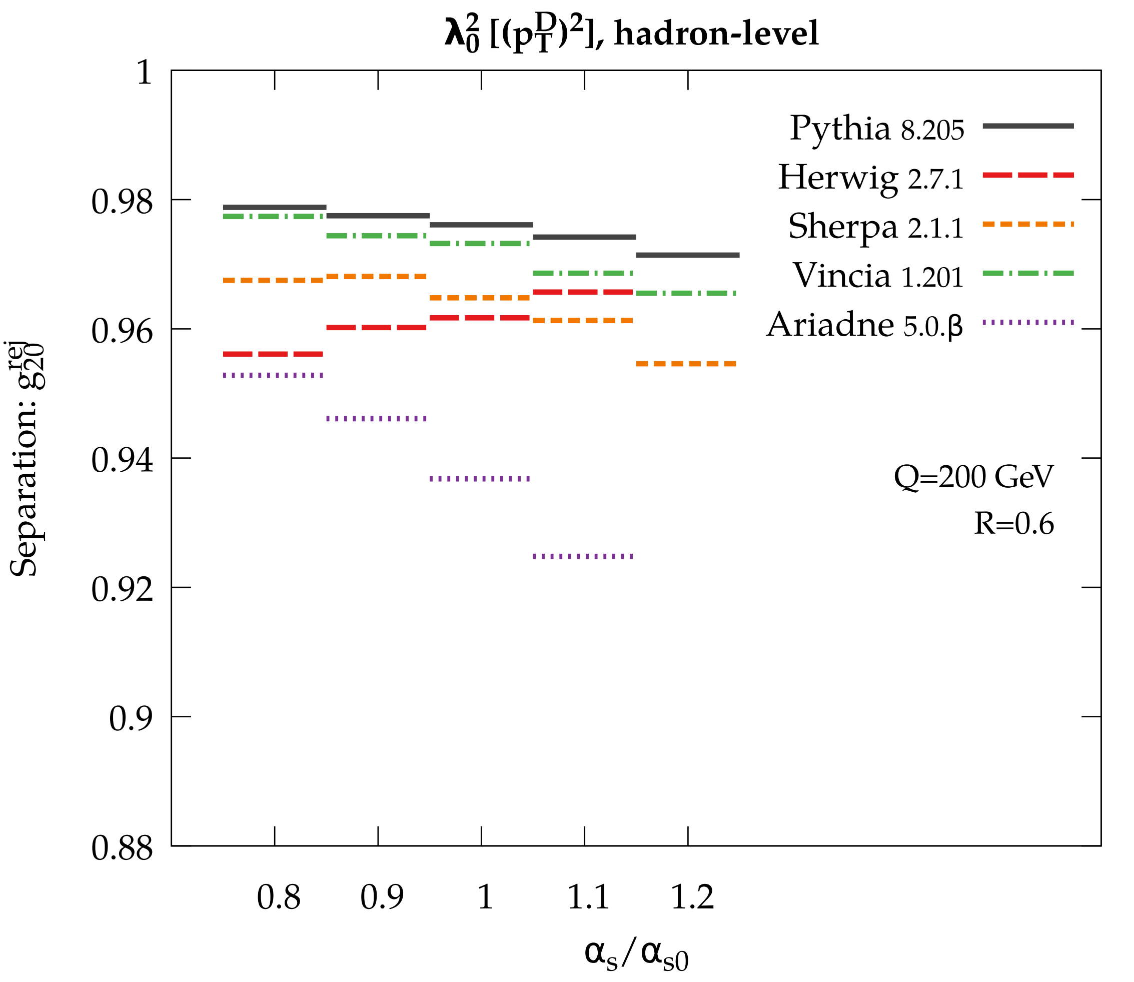

$\lambda_0^2$ [$(p_T^D)^2$], hadron-level
Separation: $g_{20}^{rej}$
1
0.98
0.96
0.94
0.92
0.9
0.88
0.8
0.9
1
1.1
1.2
$\alpha_s/\alpha_{s0}$
Pythia 8.205
Herwig 2.7.1
Sherpa 2.1.1
Vincia 1.201
Ariadne 5.0.β
Q=200 GeV
R=0.6

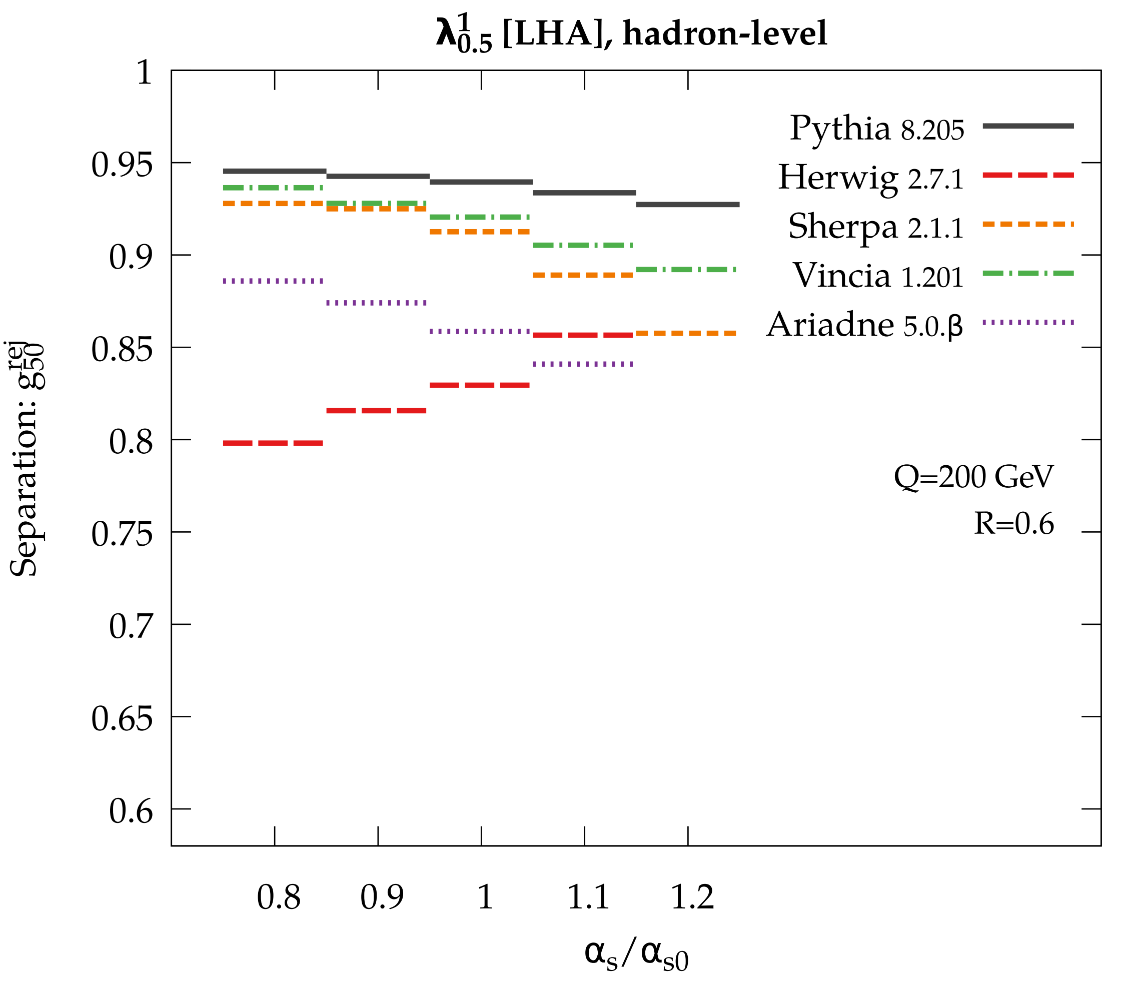

$\lambda^1_{0.5}$ [LHA], hadron-level
Separation: $g^{rej}_{50}$
1
0.95
0.9
0.85
0.8
0.75
0.7
0.65
0.6
0.8
0.9
1
1.1
1.2
$\alpha_s/\alpha_{s0}$
Pythia 8.205
Herwig 2.7.1
Sherpa 2.1.1
Vincia 1.201
Ariadne 5.0.β
Q=200 GeV
R=0.6

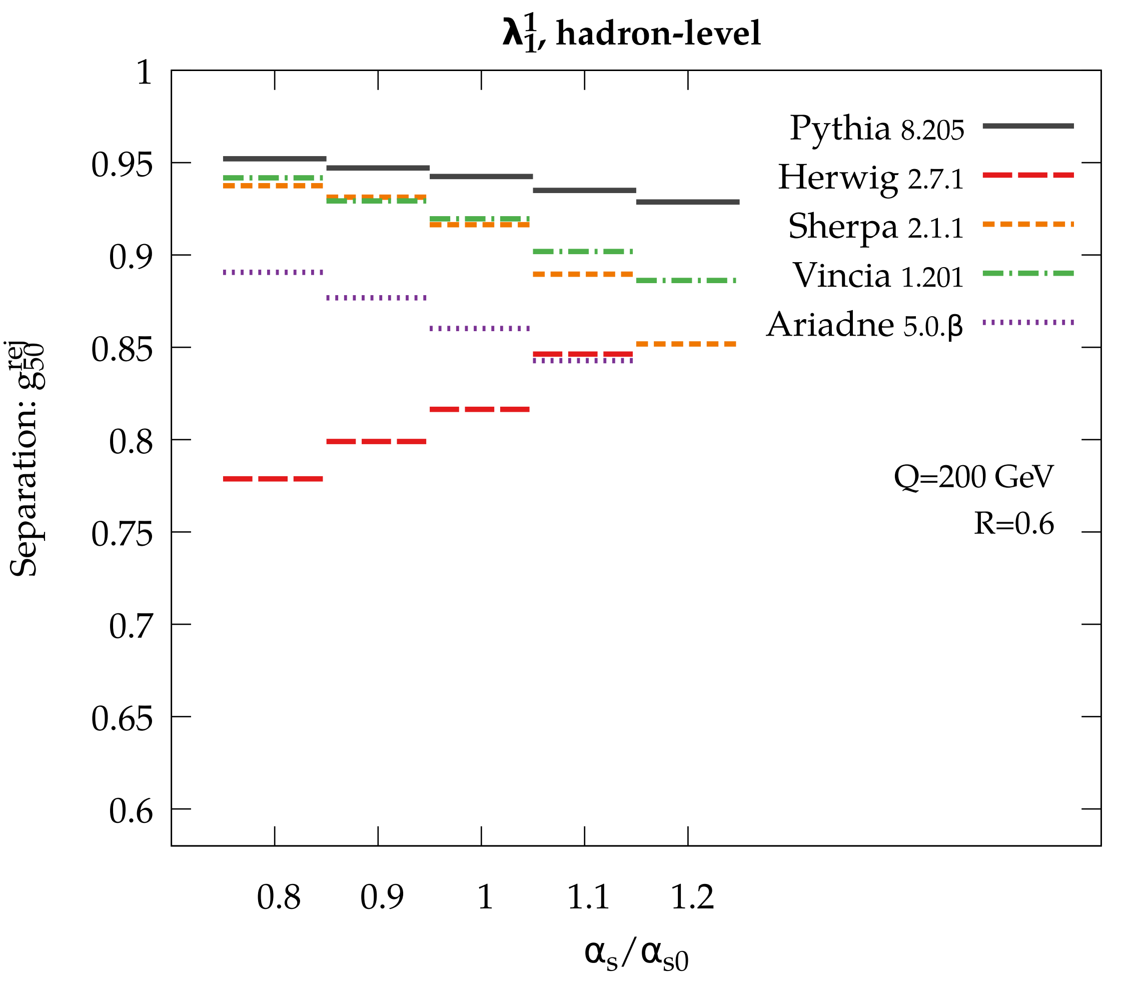

$\lambda_1^1$, hadron-level
Pythia 8.205
Herwig 2.7.1
Sherpa 2.1.1
Vincia 1.201
Ariadne 5.0.β
Q=200 GeV
R=0.6
Separation: $g_{50}^{rej}$
$\alpha_s/\alpha_{s0}$
1
0.95
0.9
0.85
0.8
0.75
0.7
0.65
0.6
0.8
0.9
1
1.1
1.2

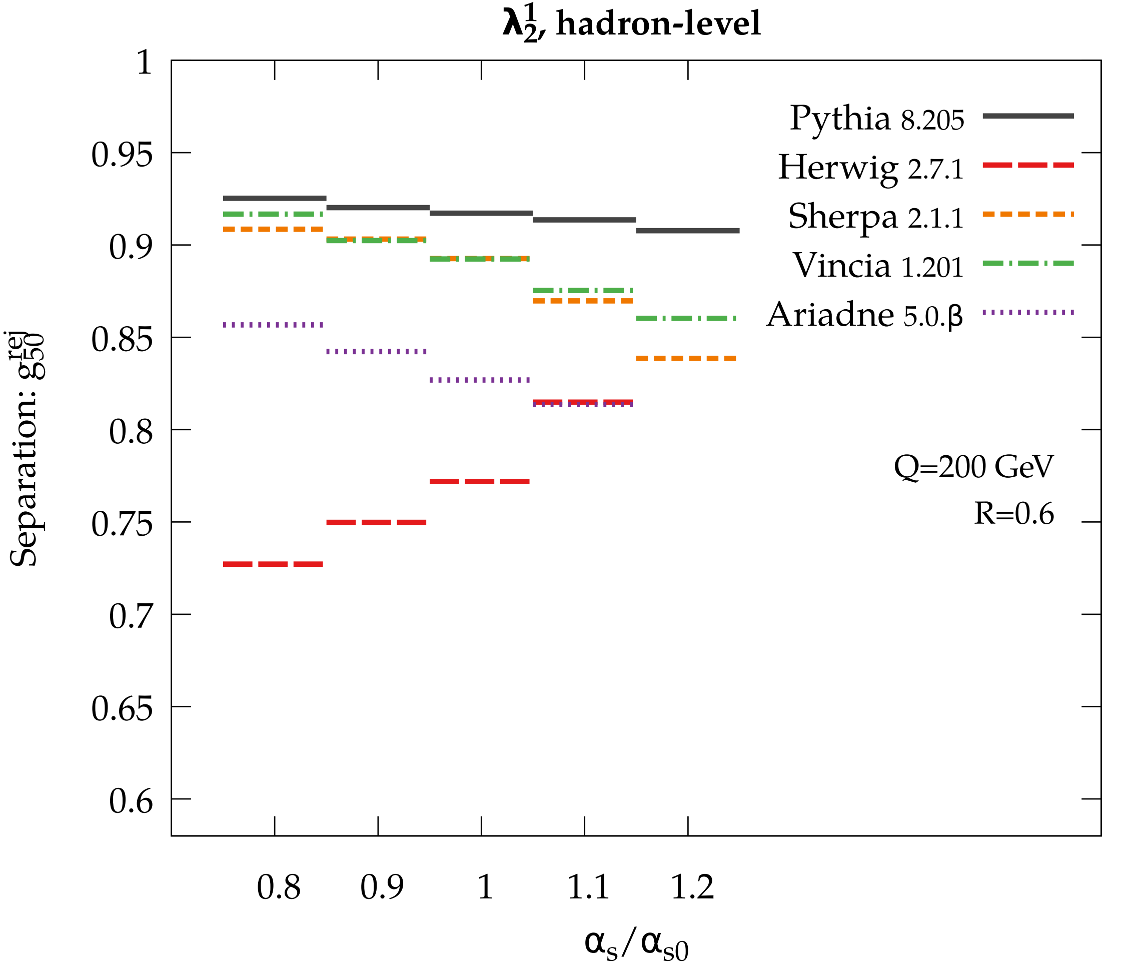

$\lambda_2^1$, hadron-level
Separation: $g_{50}^{rej}$
$\alpha_s/\alpha_{s0}$
Pythia 8.205
Herwig 2.7.1
Sherpa 2.1.1
Vincia 1.201
Ariadne 5.0.β
Q=200 GeV
R=0.6
1
0.95
0.9
0.85
0.8
0.75
0.7
0.65
0.6
0.8
0.9
1
1.1
1.2

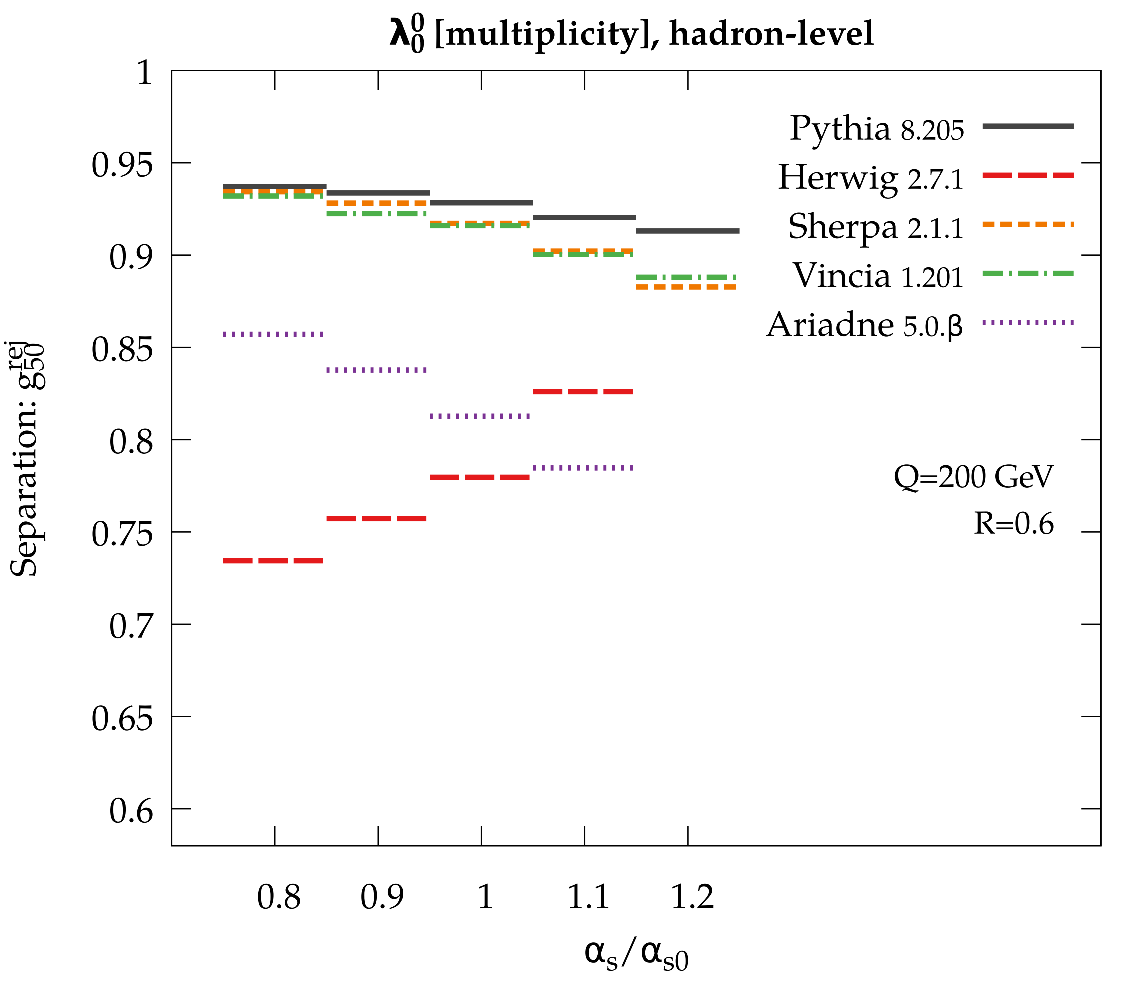

$\lambda_0^0$ [multiplicity], hadron-level
Separation: $g_{50}^{rej}$
$\alpha_s/\alpha_{s0}$
Pythia 8.205
Herwig 2.7.1
Sherpa 2.1.1
Vincia 1.201
Ariadne 5.0.β
Q=200 GeV
R=0.6
1
0.95
0.9
0.85
0.8
0.75
0.7
0.65
0.6
0.8
0.9
1
1.1
1.2

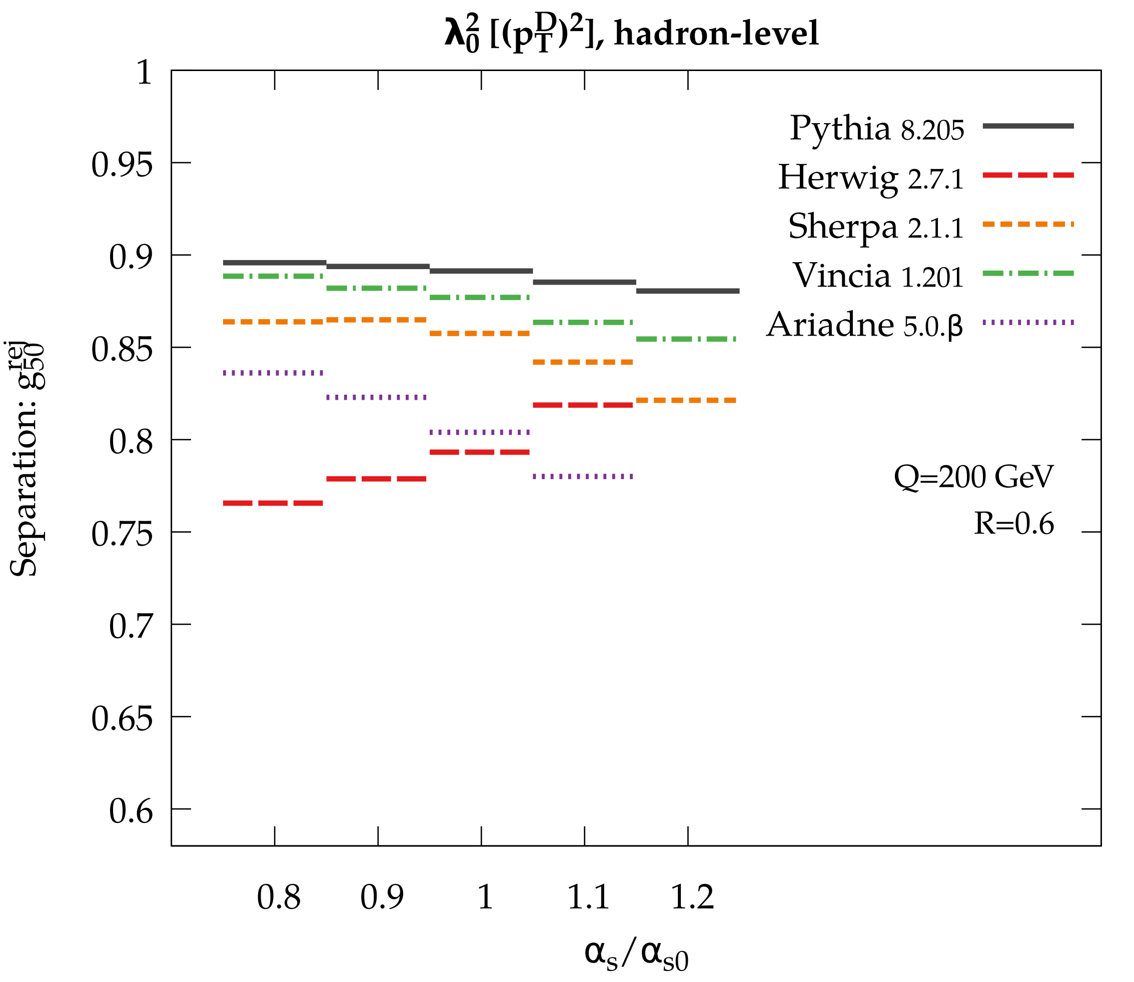

$\lambda_0^2$ [$(p_T^D)^2$], hadron-level
Separation: $g_{50}^{rej}$
1
0.95
0.9
0.85
0.8
0.75
0.7
0.65
0.6
0.8
0.9
1
1.1
1.2
$\alpha_s/\alpha_{s0}$
Pythia 8.205
Herwig 2.7.1
Sherpa 2.1.1
Vincia 1.201
Ariadne 5.0.β
Q=200 GeV
R=0.6

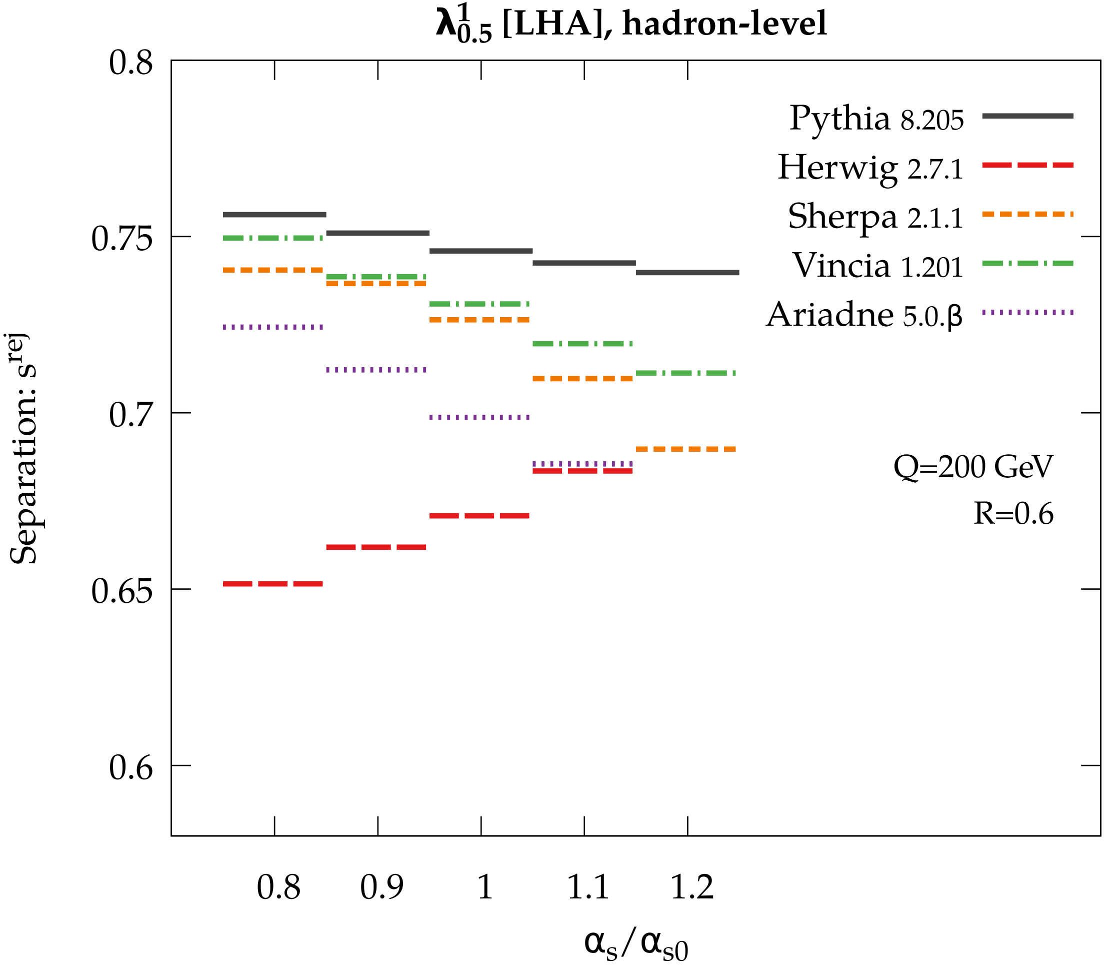

λ^1_0.5 [LHA], hadron-level
Pythia 8.205
Herwig 2.7.1
Sherpa 2.1.1
Vincia 1.201
Ariadne 5.0.β
Q=200 GeV
R=0.6
Separation: s^rej
α_s/α_s0
0.8
0.75
0.7
0.65
0.6
0.8
0.9
1
1.1
1.2

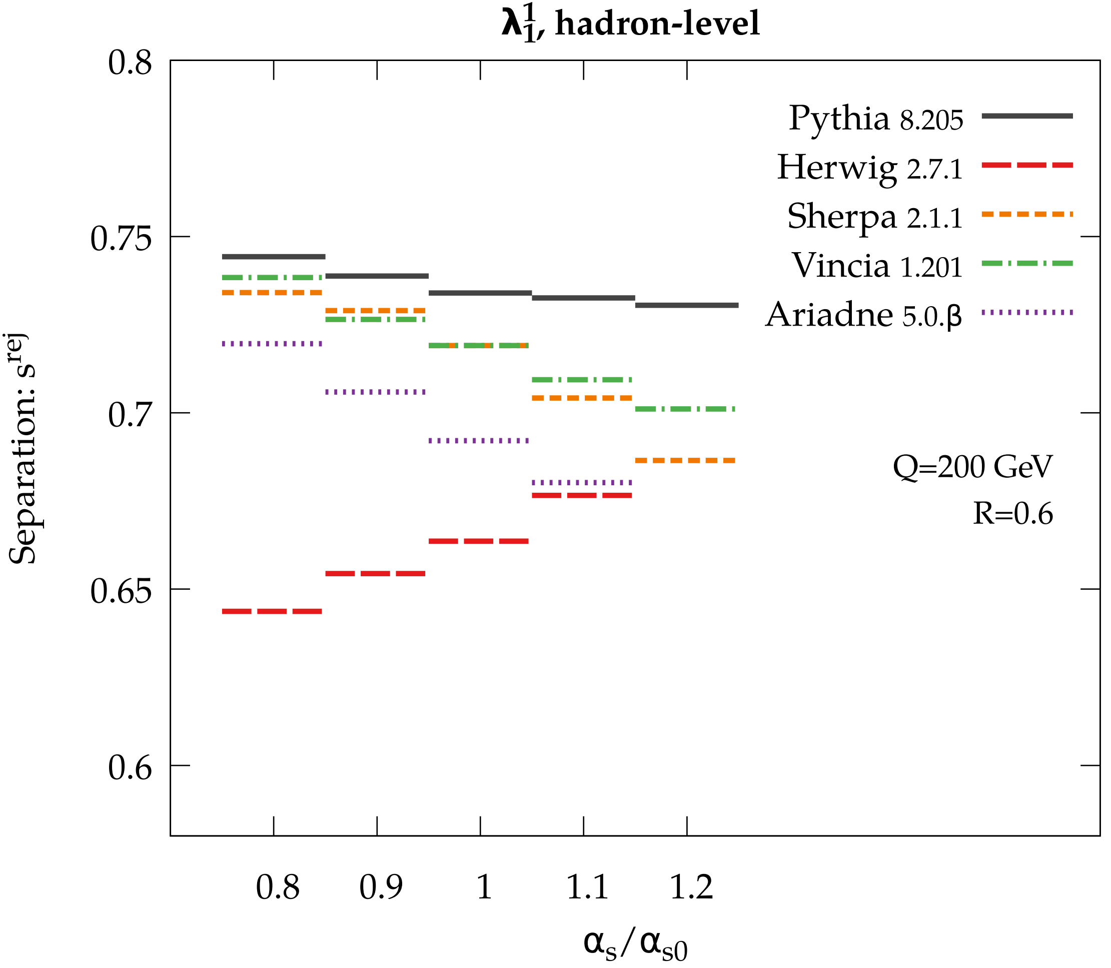
$\lambda_1^1$, hadron-level
Pythia 8.205
Herwig 2.7.1
Sherpa 2.1.1
Vincia 1.201
Ariadne 5.0.β
Q=200 GeV
R=0.6
Separation: $s^{rej}$
0.8
0.75
0.7
0.65
0.6
0.8
0.9
1
1.1
1.2
$\alpha_s/\alpha_{s0}$

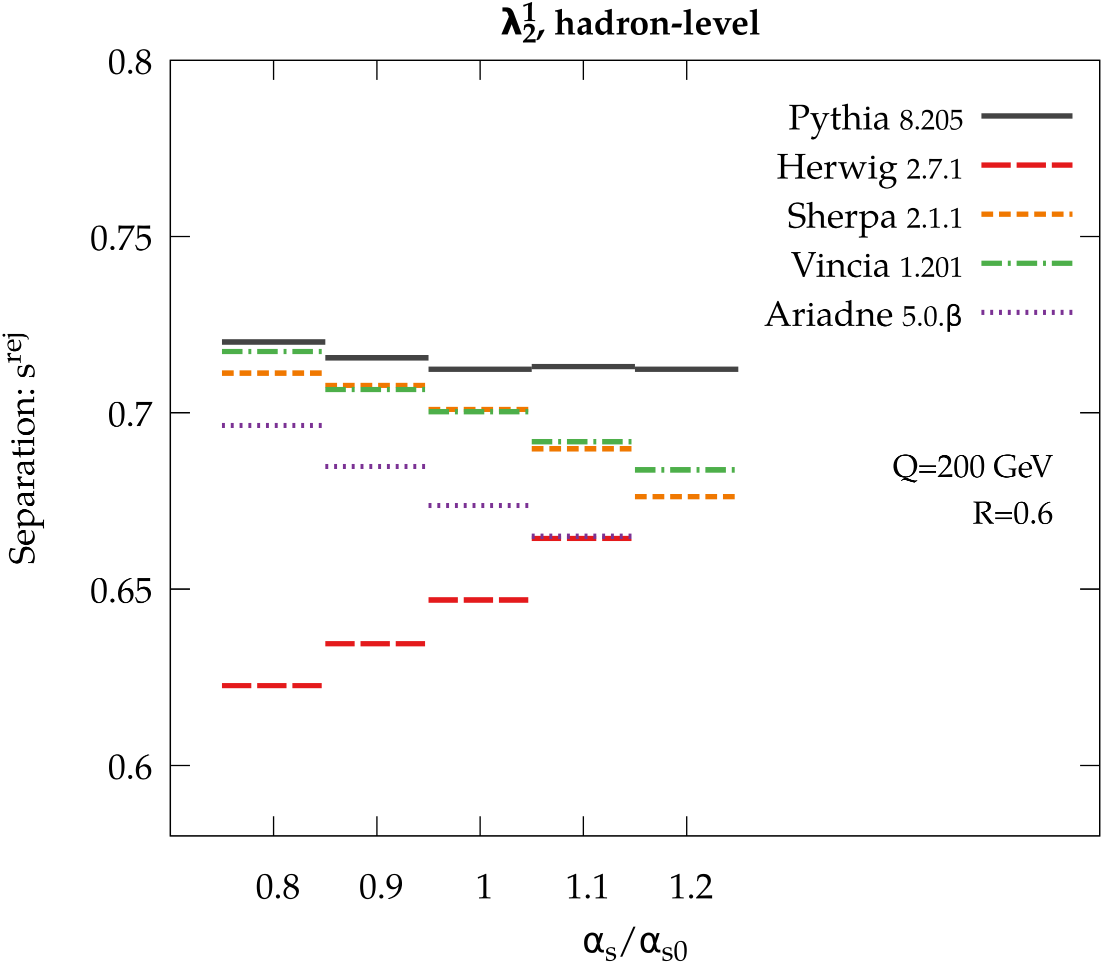

$\lambda^1_2$, hadron-level
0.8
0.75
0.7
0.65
0.6
Separation: $s^{rej}$
Pythia 8.205
Herwig 2.7.1
Sherpa 2.1.1
Vincia 1.201
Ariadne 5.0.β
Q=200 GeV
R=0.6
0.8
0.9
1
1.1
1.2
$\alpha_s/\alpha_{s0}$

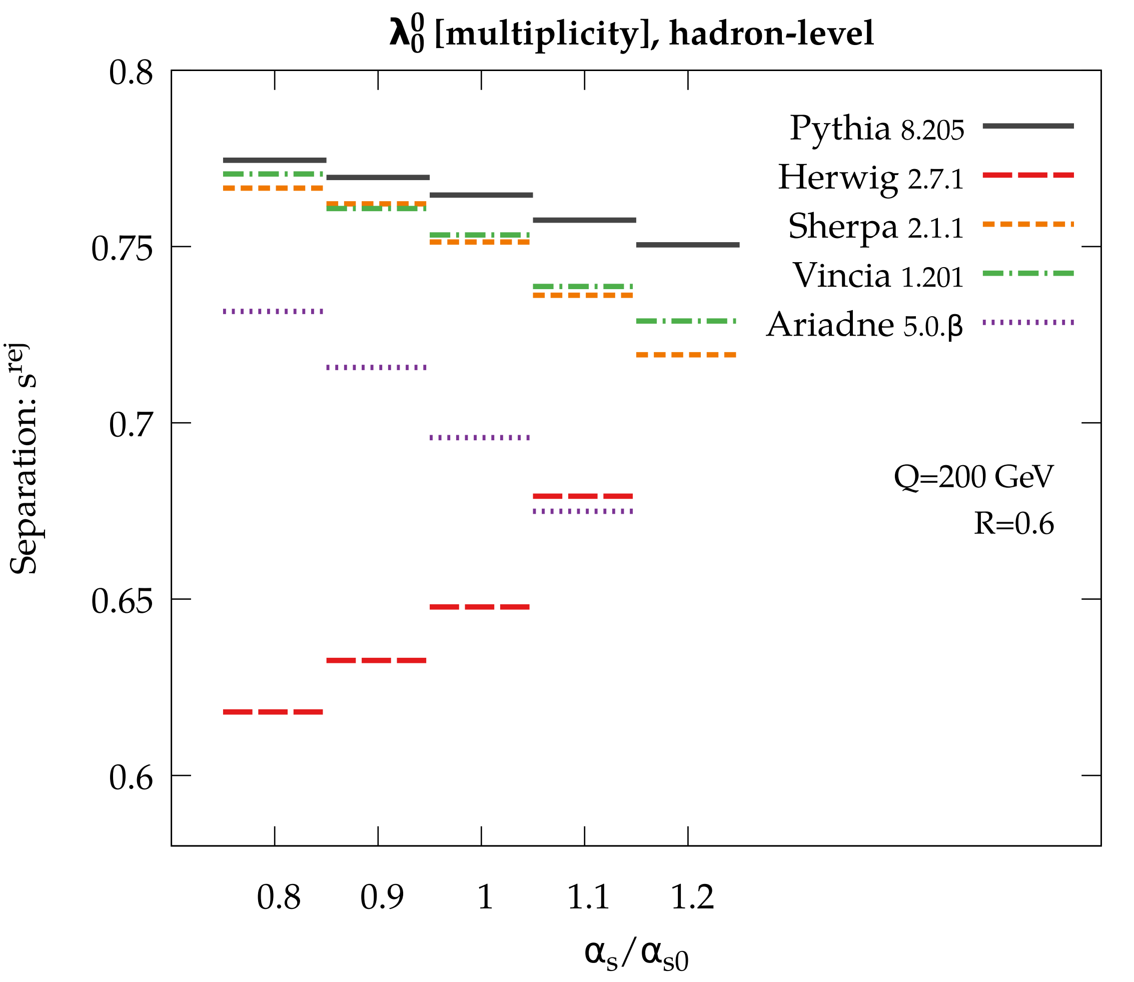

$\lambda_0^0$ [multiplicity], hadron-level
Pythia 8.205
Herwig 2.7.1
Sherpa 2.1.1
Vincia 1.201
Ariadne 5.0.β
Q=200 GeV
R=0.6
Separation: $s^{rej}$
0.8
0.75
0.7
0.65
0.6
0.8
0.9
1
1.1
1.2
$\alpha_s/\alpha_{s0}$

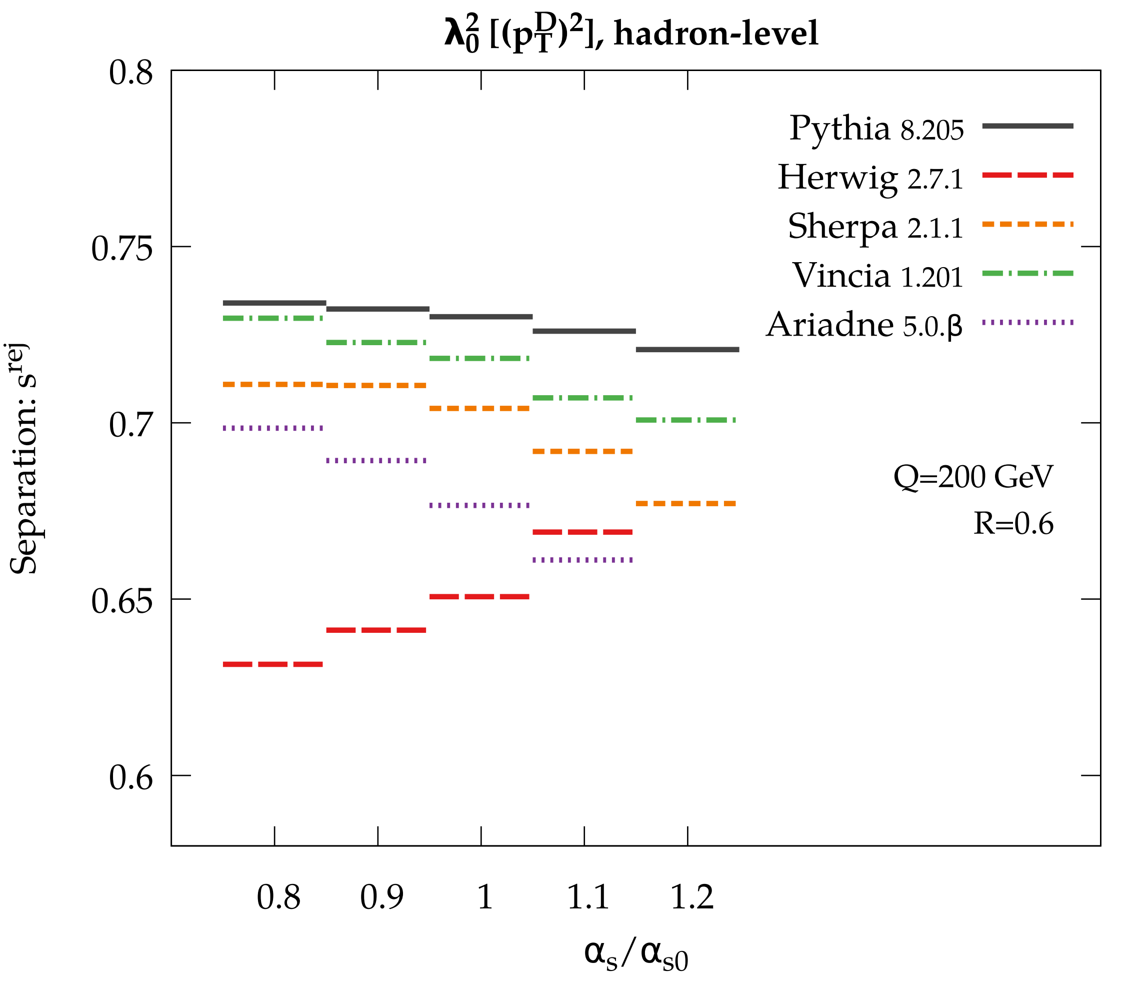

$\lambda_0^2\ [(p_T^D)^2]$, hadron-level
Separation: $s^{rej}$
0.8
0.75
0.7
0.65
0.6
Pythia 8.205
Herwig 2.7.1
Sherpa 2.1.1
Vincia 1.201
Ariadne 5.0.β
Q=200 GeV
R=0.6
0.8
0.9
1
1.1
1.2
$\alpha_s/\alpha_{s0}$
