# Supplementary material for: Les Houches 2015: Physics at TeV Colliders Standard Model Working Group Report
Source: arXiv:1605.04692 source file (2016-05-16)
Supplement: Supplementary file 2 [file quarkgluon_fig_I2_GA_10_05_parton_Qdep.pdf]

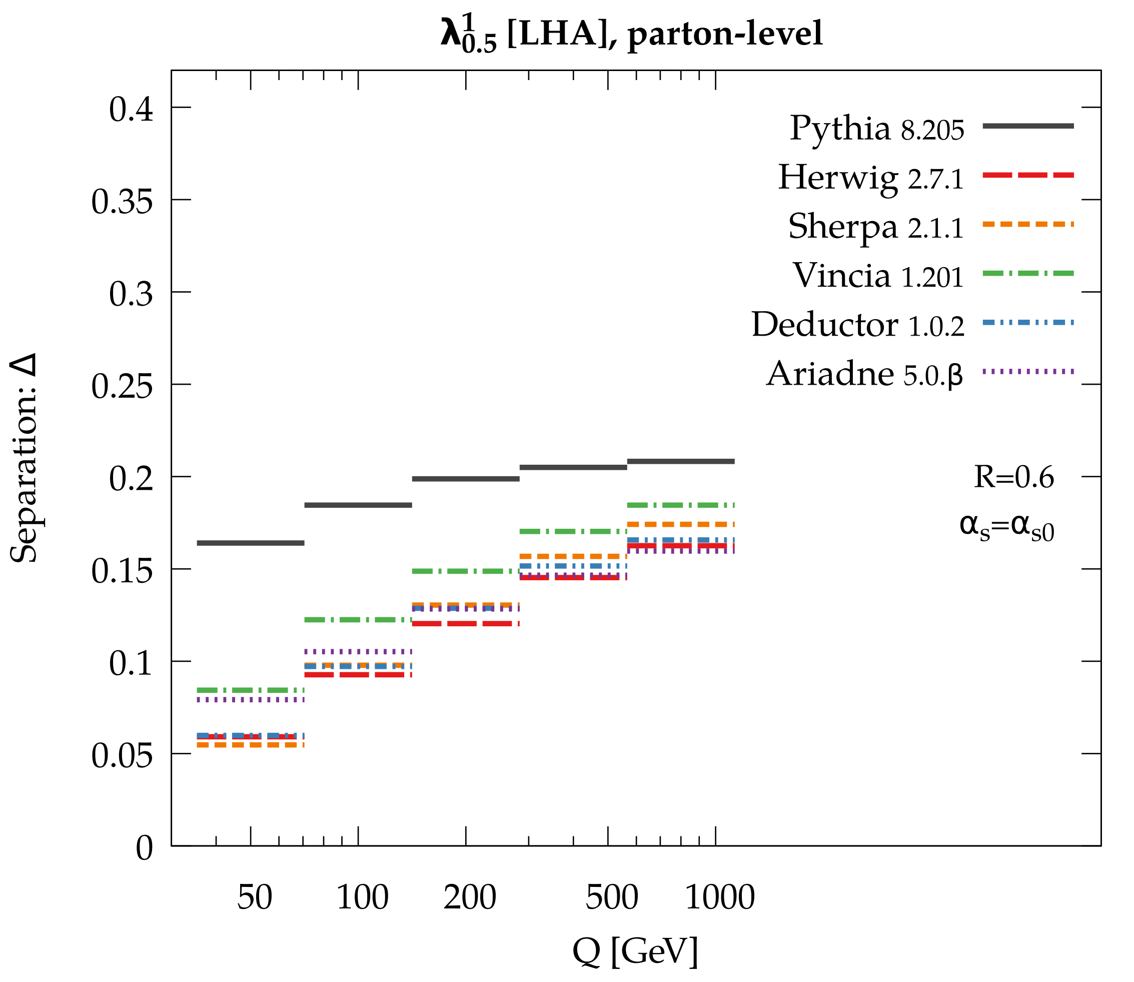

λ^1_0.5 [LHA], parton-level
Pythia 8.205
Herwig 2.7.1
Sherpa 2.1.1
Vincia 1.201
Deductor 1.0.2
Ariadne 5.0.β
R=0.6
αs=αs0
Separation: Δ
0
0.05
0.1
0.15
0.2
0.25
0.3
0.35
0.4
50
100
200
500
1000
Q [GeV]

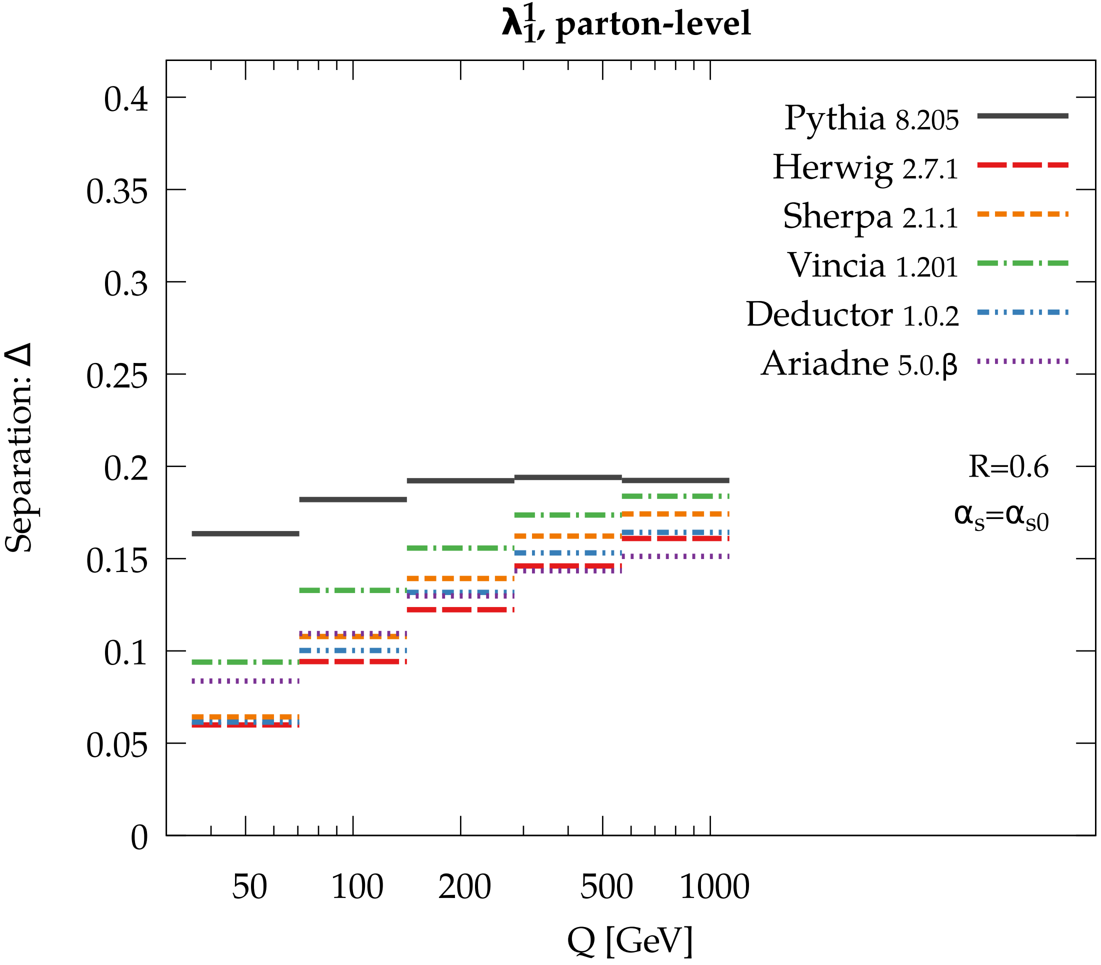

$\lambda_1^1$, parton-level
Pythia 8.205
Herwig 2.7.1
Sherpa 2.1.1
Vincia 1.201
Deductor 1.0.2
Ariadne 5.0.β
R=0.6
$\alpha_s=\alpha_{s0}$
Separation: Δ
0.4
0.35
0.3
0.25
0.2
0.15
0.1
0.05
0
50
100
200
500
1000
Q [GeV]

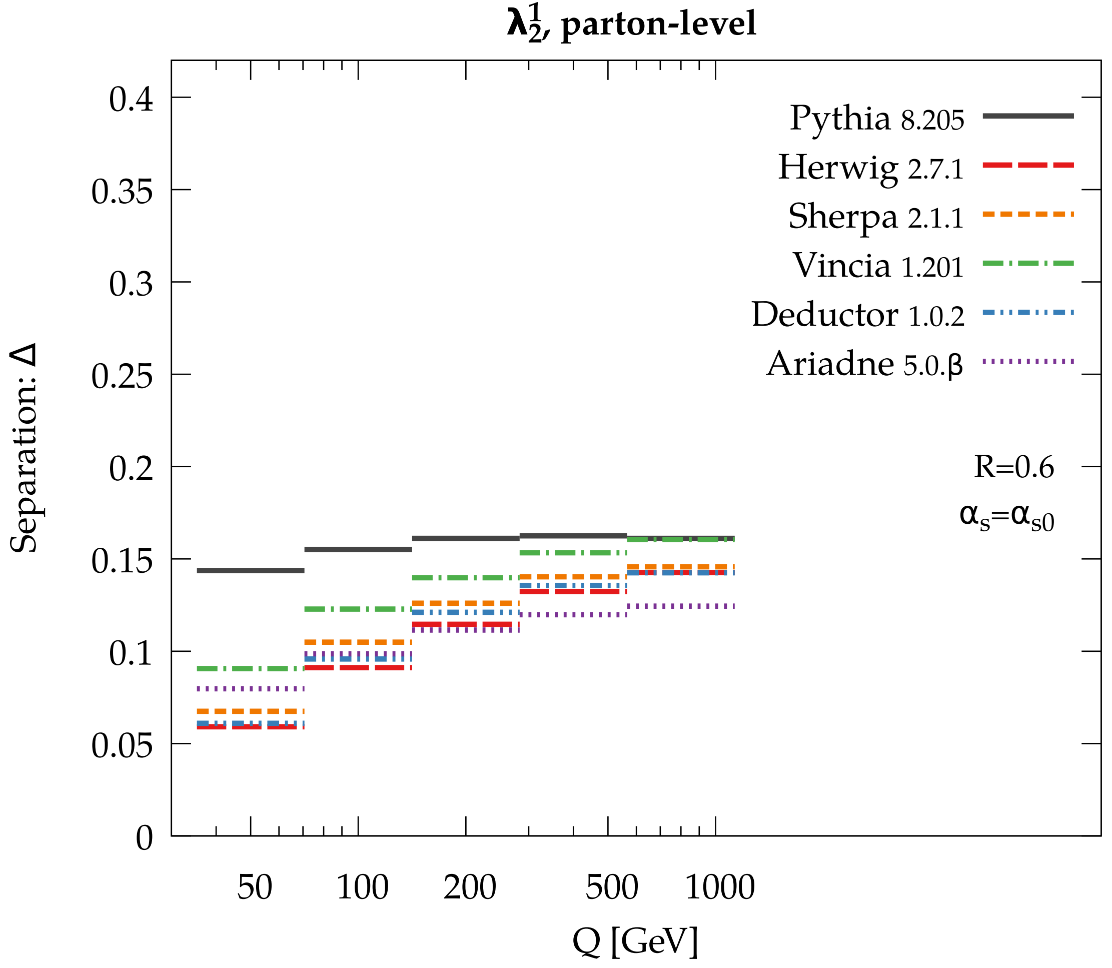

$\lambda_2^1$, parton-level
Separation: Δ
0
0.05
0.1
0.15
0.2
0.25
0.3
0.35
0.4
50
100
200
500
1000
Q [GeV]
Pythia 8.205
Herwig 2.7.1
Sherpa 2.1.1
Vincia 1.201
Deductor 1.0.2
Ariadne 5.0.β
R=0.6
$\alpha_s=\alpha_{s0}$

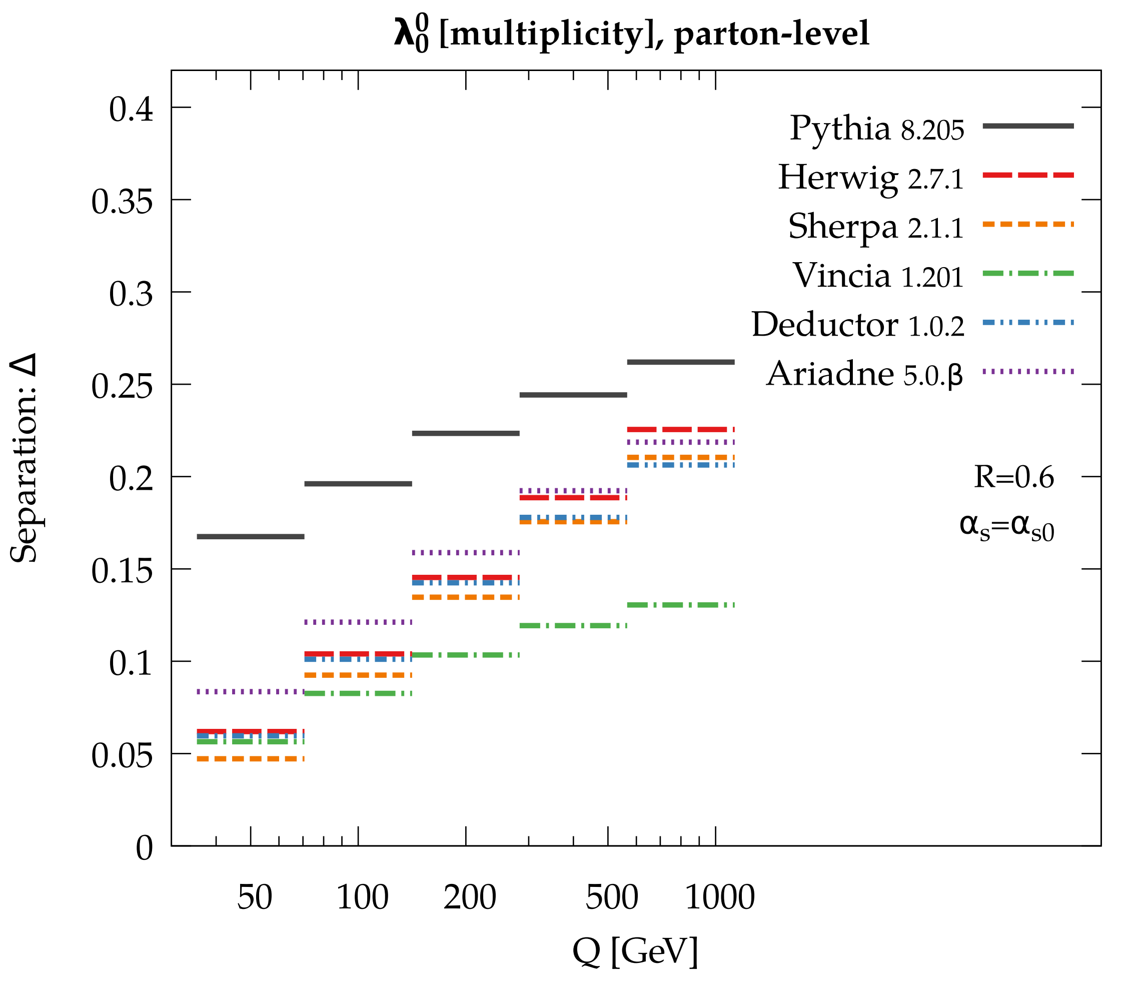

$\lambda_0^0$ [multiplicity], parton-level
Separation: Δ
Q [GeV]
Pythia 8.205
Herwig 2.7.1
Sherpa 2.1.1
Vincia 1.201
Deductor 1.0.2
Ariadne 5.0.β
R=0.6
$\alpha_s=\alpha_{s0}$
0
0.05
0.1
0.15
0.2
0.25
0.3
0.35
0.4
50
100
200
500
1000

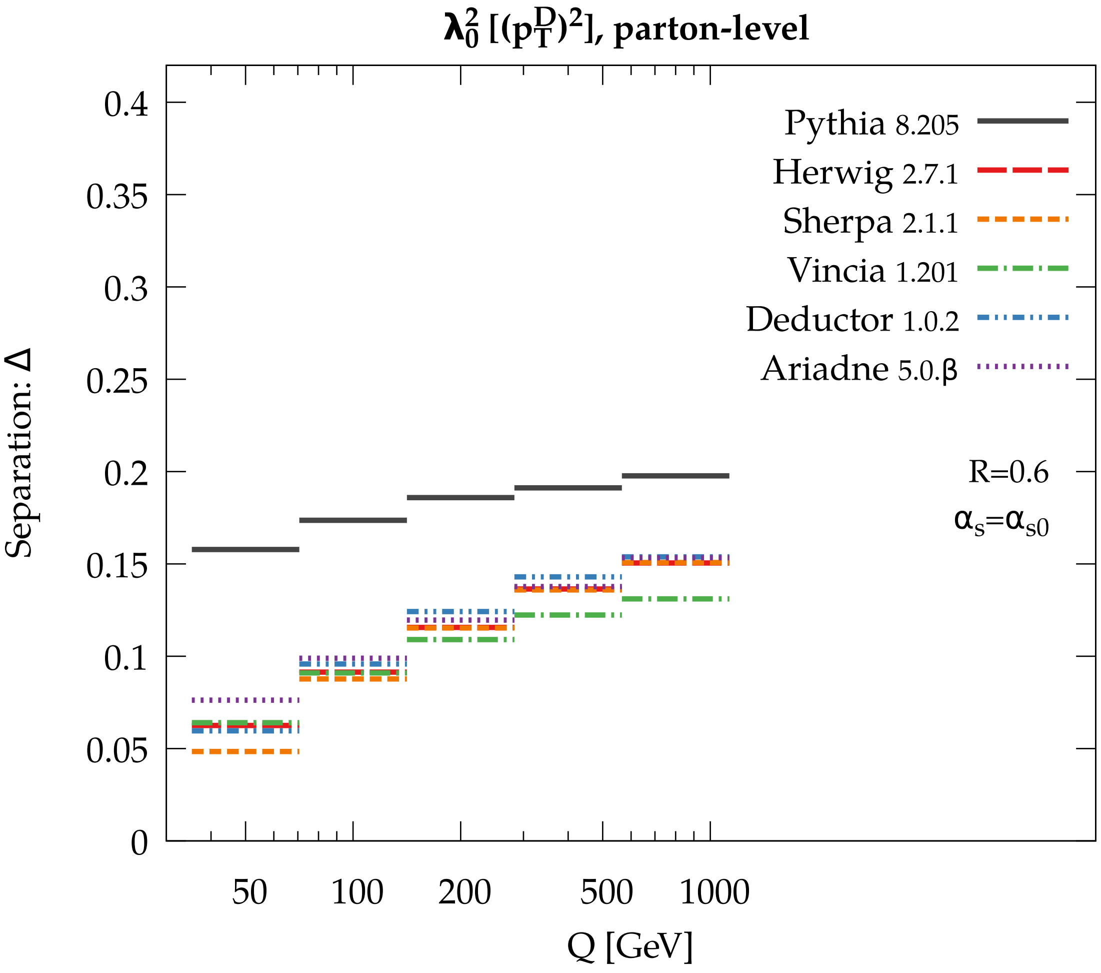

$\lambda_0^2$ [$(p_T^D)^2$], parton-level
Separation: Δ
Q [GeV]
0
0.05
0.1
0.15
0.2
0.25
0.3
0.35
0.4
50
100
200
500
1000
Pythia 8.205
Herwig 2.7.1
Sherpa 2.1.1
Vincia 1.201
Deductor 1.0.2
Ariadne 5.0.β
R=0.6
$\alpha_s=\alpha_{s0}$

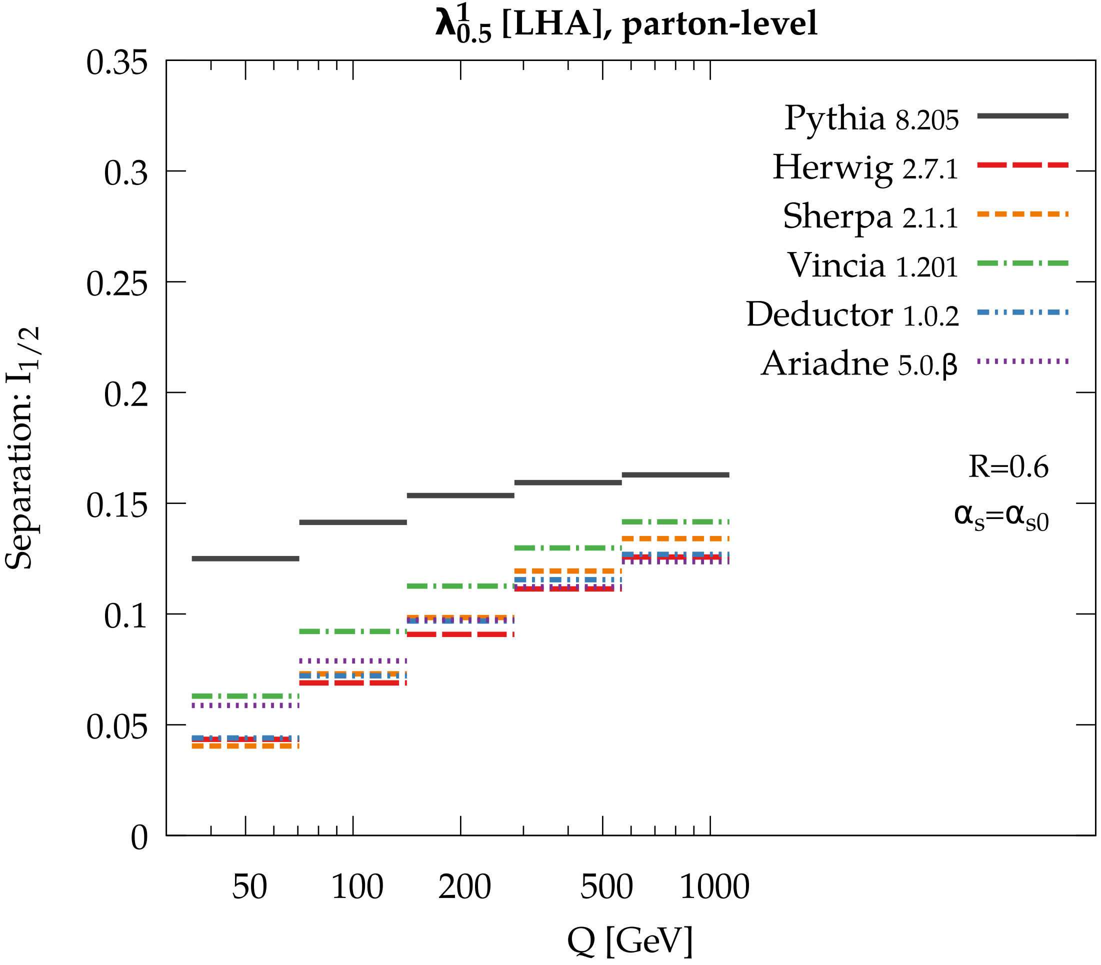

$\lambda^1_{0.5}$ [LHA], parton-level
Separation: $I_{1/2}$
0.35
0.3
0.25
0.2
0.15
0.1
0.05
0
50
100
200
500
1000
Q [GeV]
Pythia 8.205
Herwig 2.7.1
Sherpa 2.1.1
Vincia 1.201
Deductor 1.0.2
Ariadne 5.0.β
R=0.6
$\alpha_s=\alpha_{s0}$

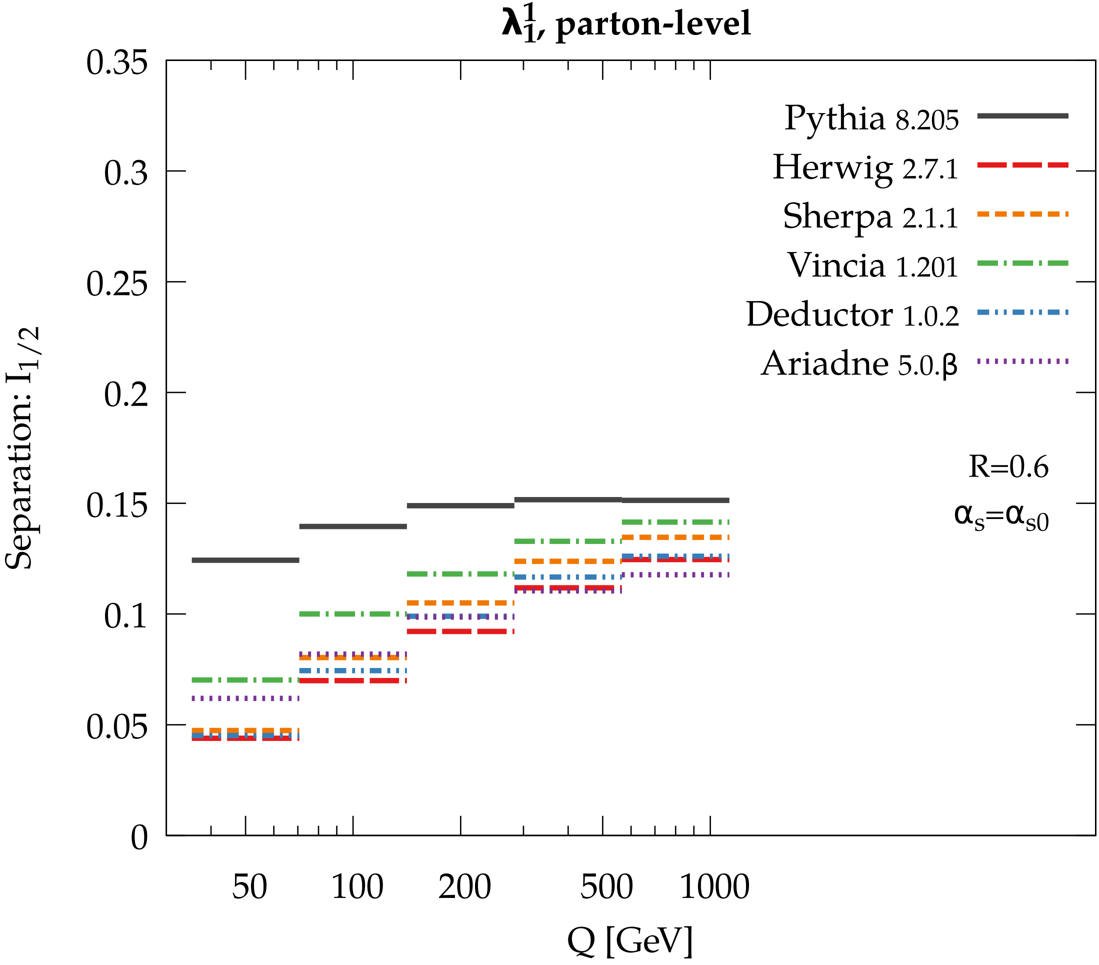

$\lambda_1^1$, parton-level
0.35
0.3
0.25
0.2
0.15
0.1
0.05
0
Separation: $I_{1/2}$
Pythia 8.205
Herwig 2.7.1
Sherpa 2.1.1
Vincia 1.201
Deductor 1.0.2
Ariadne 5.0.β
R=0.6
$\alpha_s=\alpha_{s0}$
50
100
200
500
1000
Q [GeV]

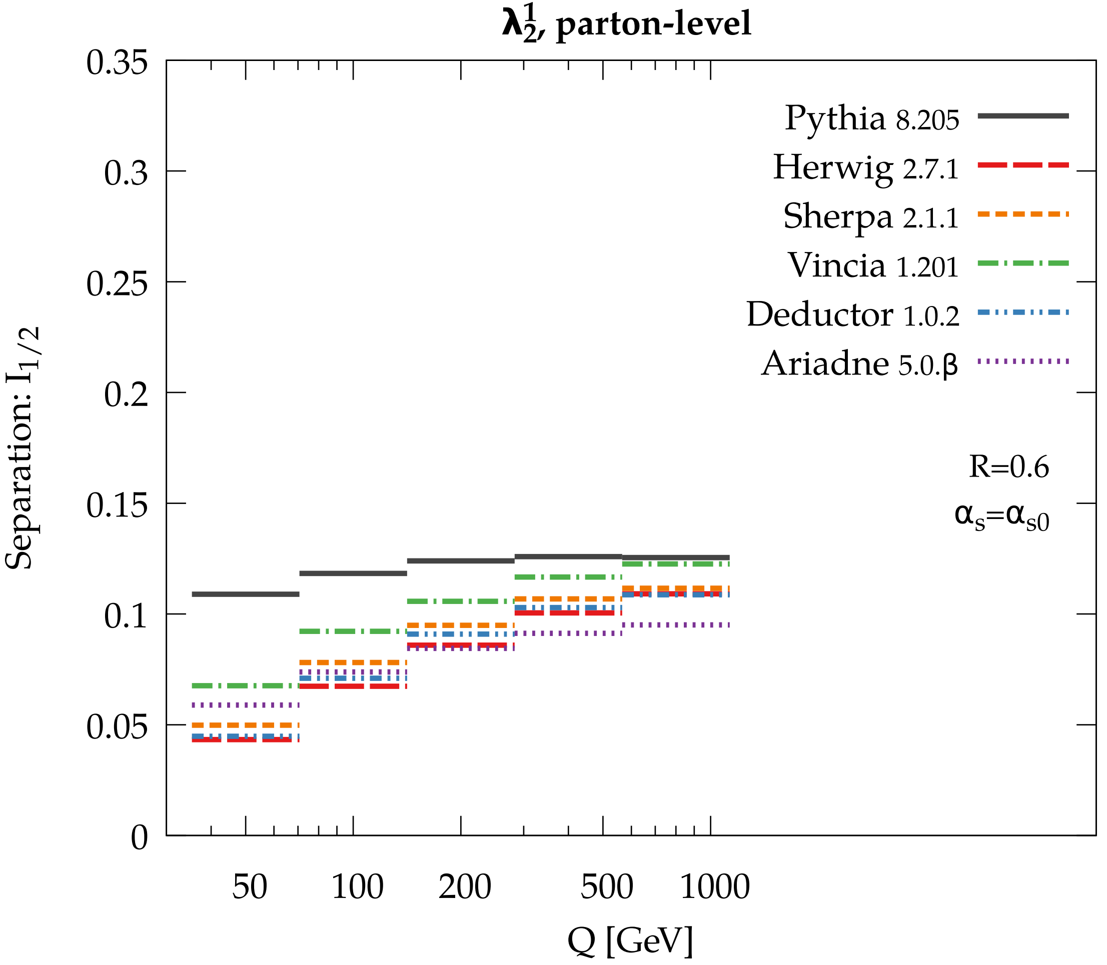

$\lambda_2^1$, parton-level
Separation: $I_{1/2}$
Q [GeV]
0
0.05
0.1
0.15
0.2
0.25
0.3
0.35
50
100
200
500
1000
Pythia 8.205
Herwig 2.7.1
Sherpa 2.1.1
Vincia 1.201
Deductor 1.0.2
Ariadne 5.0.β
R=0.6
$\alpha_s=\alpha_{s0}$

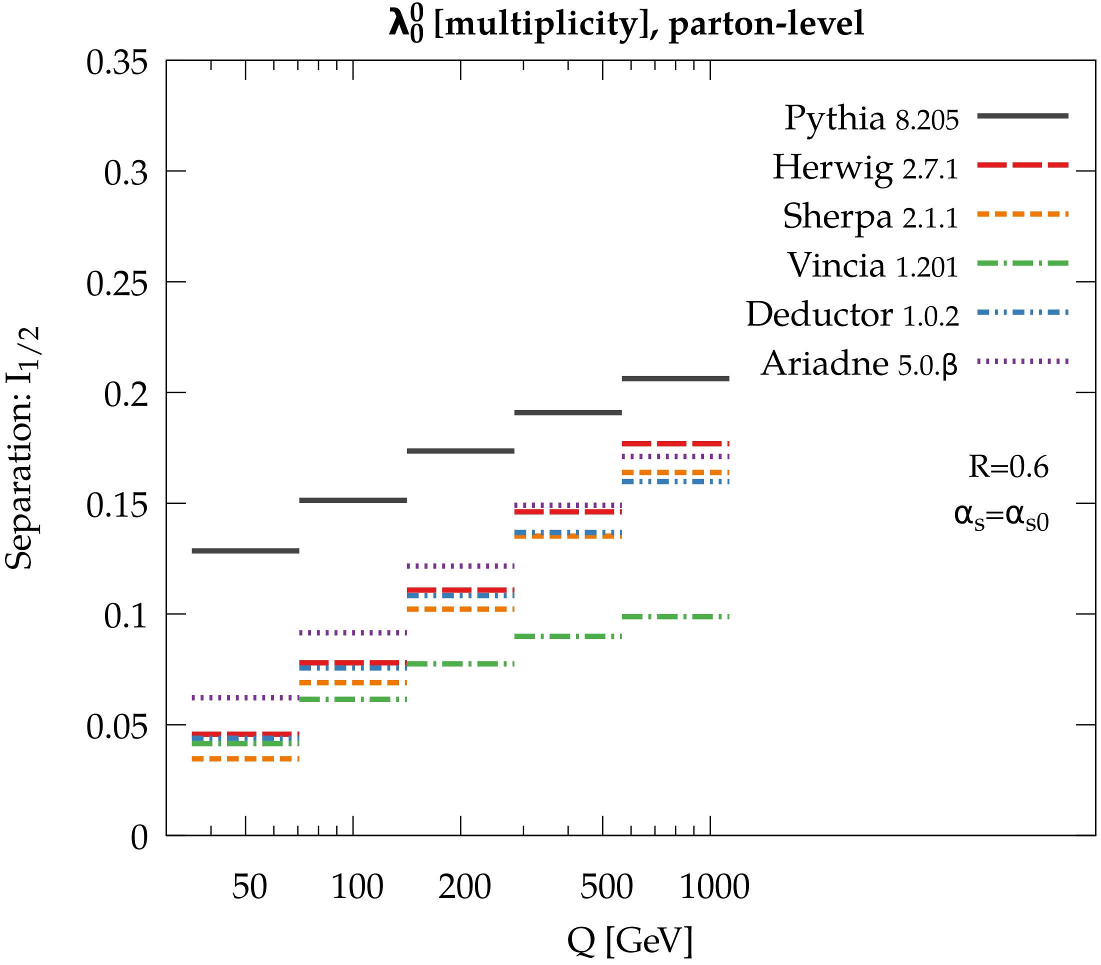

$\lambda_0^0$ [multiplicity], parton-level
Pythia 8.205
Herwig 2.7.1
Sherpa 2.1.1
Vincia 1.201
Deductor 1.0.2
Ariadne 5.0.β
R=0.6
$\alpha_s=\alpha_{s0}$
Separation: $I_{1/2}$
0
0.05
0.1
0.15
0.2
0.25
0.3
0.35
50
100
200
500
1000
Q [GeV]

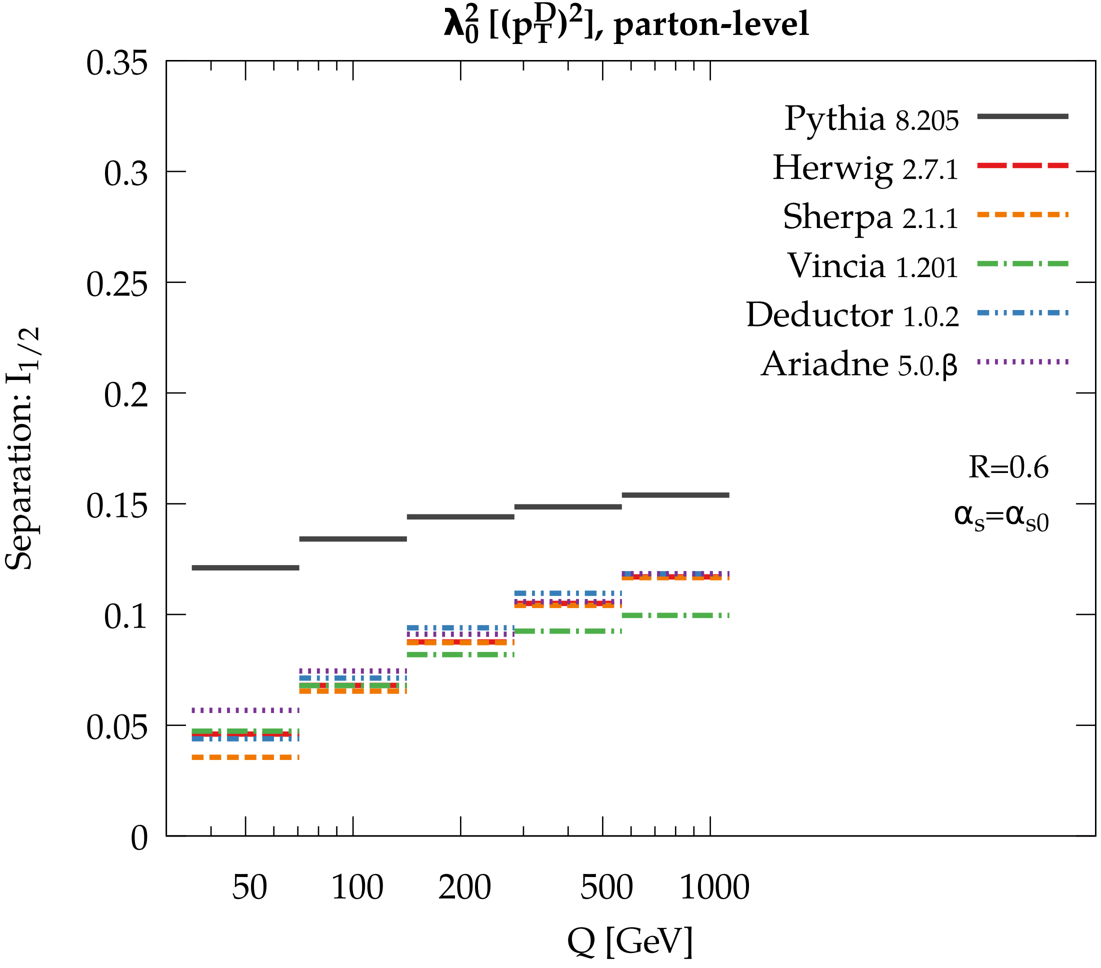
$\lambda_0^2\ [(p_T^D)^2]$, parton-level
Separation: $I_{1/2}$
0.35
0.3
0.25
0.2
0.15
0.1
0.05
0
50
100
200
500
1000
Q [GeV]
Pythia 8.205
Herwig 2.7.1
Sherpa 2.1.1
Vincia 1.201
Deductor 1.0.2
Ariadne 5.0.β
R=0.6
$\alpha_s=\alpha_{s0}$

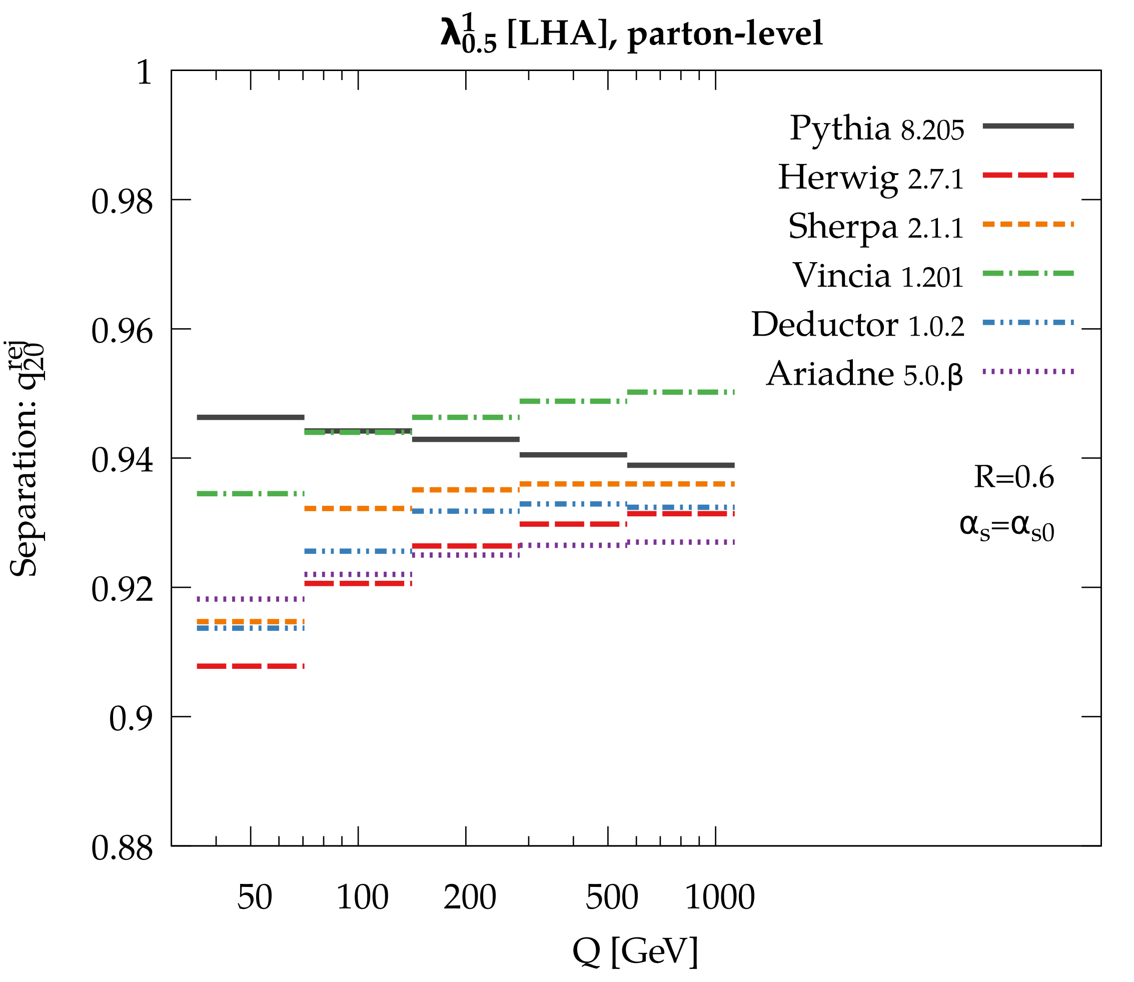

$\lambda^1_{0.5}$ [LHA], parton-level
Separation: $q^{rej}_{20}$
Q [GeV]
Pythia 8.205
Herwig 2.7.1
Sherpa 2.1.1
Vincia 1.201
Deductor 1.0.2
Ariadne 5.0.β
R=0.6
$\alpha_s=\alpha_{s0}$
1
0.98
0.96
0.94
0.92
0.9
0.88
50
100
200
500
1000

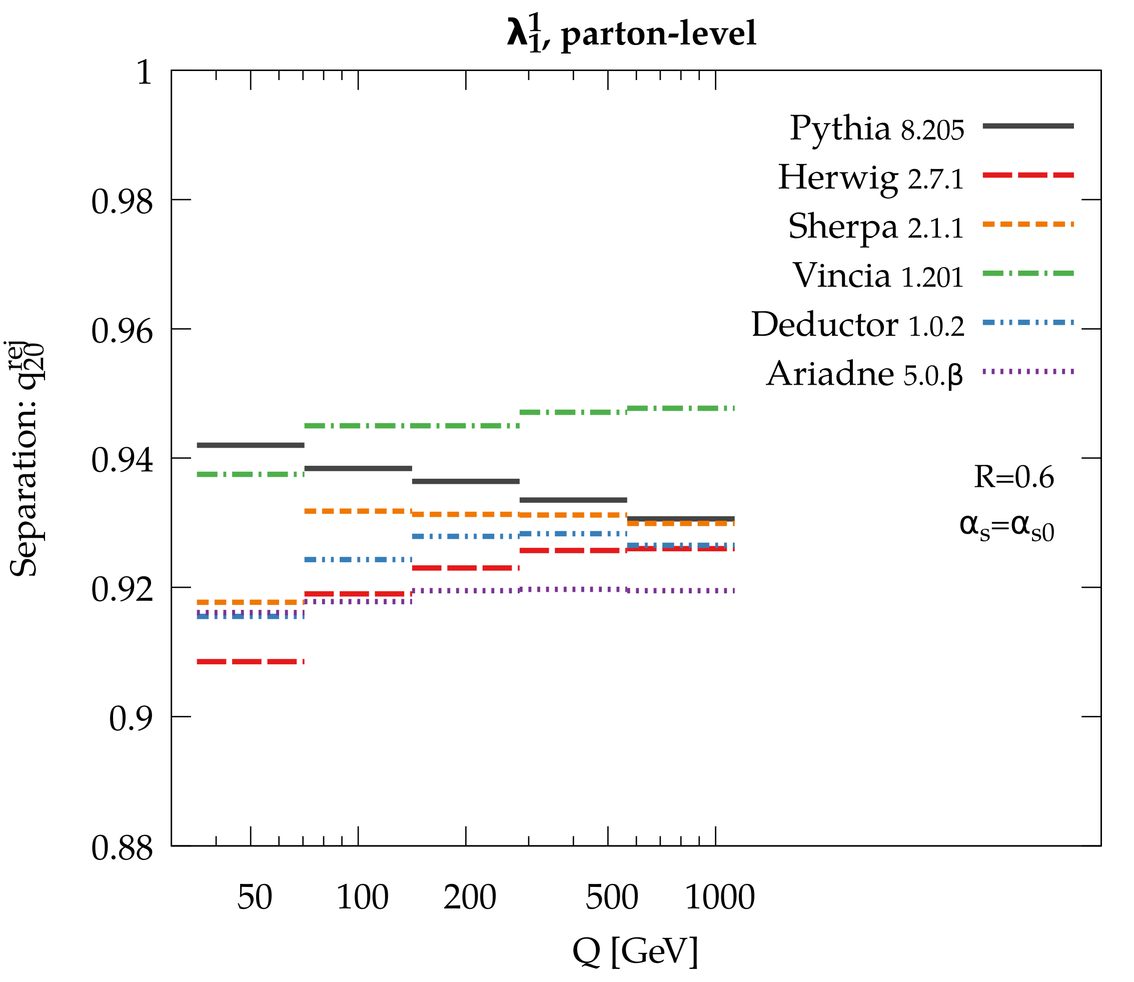

λ₁¹, parton-level
Separation: q20rej
Q [GeV]
1
0.98
0.96
0.94
0.92
0.9
0.88
50
100
200
500
1000
Pythia 8.205
Herwig 2.7.1
Sherpa 2.1.1
Vincia 1.201
Deductor 1.0.2
Ariadne 5.0.β
R=0.6
αs=αs0

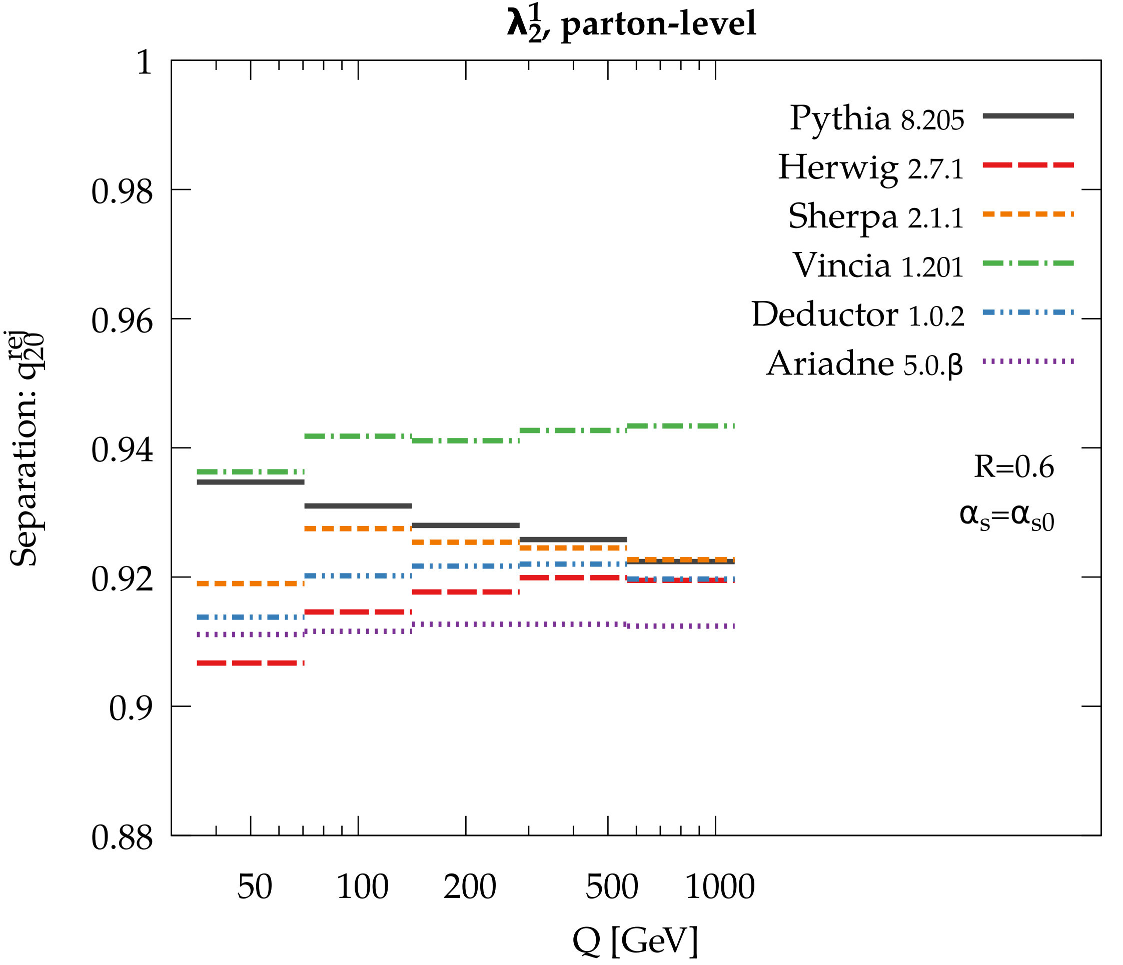

λ₂¹, parton-level
Pythia 8.205
Herwig 2.7.1
Sherpa 2.1.1
Vincia 1.201
Deductor 1.0.2
Ariadne 5.0.β
R=0.6
αs=αs0
Separation: q20rej
Q [GeV]
1
0.98
0.96
0.94
0.92
0.9
0.88
50
100
200
500
1000

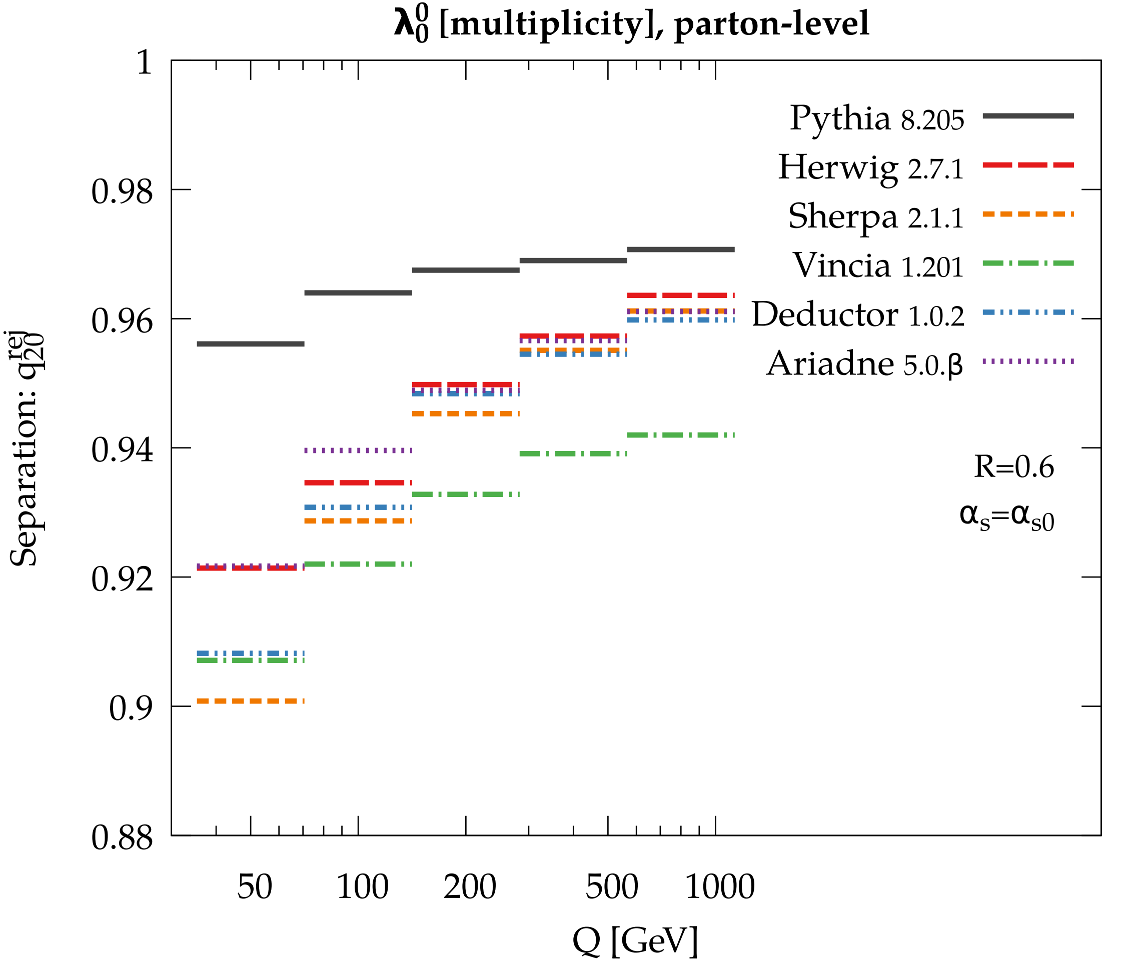

$\lambda_0^0$ [multiplicity], parton-level
Pythia 8.205
Herwig 2.7.1
Sherpa 2.1.1
Vincia 1.201
Deductor 1.0.2
Ariadne 5.0.β
R=0.6
$\alpha_s=\alpha_{s0}$
Separation: $q_{20}^{rej}$
Q [GeV]
1
0.98
0.96
0.94
0.92
0.9
0.88
50
100
200
500
1000

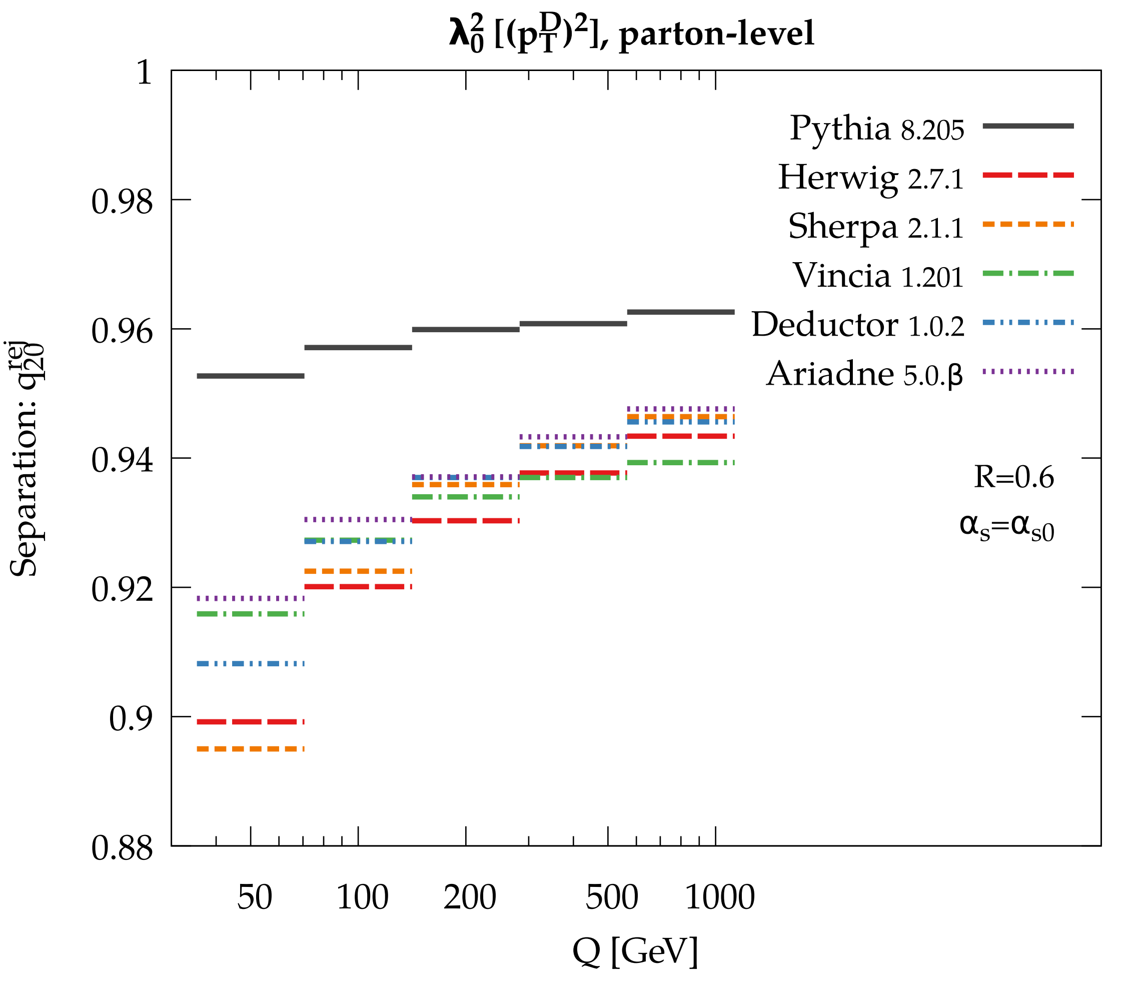

$\lambda_0^2\ [(p_T^D)^2]$, parton-level
Separation: $q_{20}^{rej}$
Q [GeV]
1
0.98
0.96
0.94
0.92
0.9
0.88
50
100
200
500
1000
Pythia 8.205
Herwig 2.7.1
Sherpa 2.1.1
Vincia 1.201
Deductor 1.0.2
Ariadne 5.0.β
R=0.6
$\alpha_s=\alpha_{s0}$

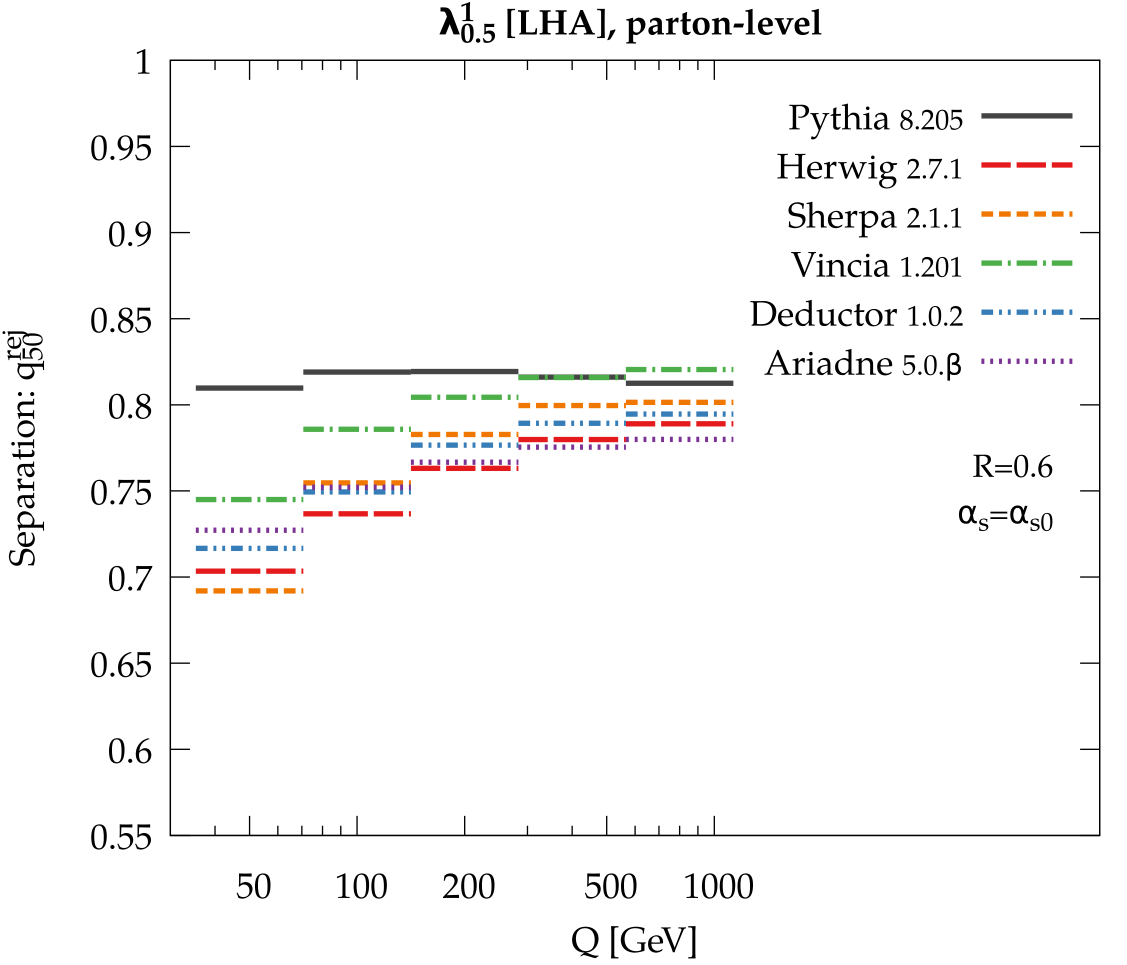

$\lambda_{0.5}^{1}$ [LHA], parton-level
Pythia 8.205
Herwig 2.7.1
Sherpa 2.1.1
Vincia 1.201
Deductor 1.0.2
Ariadne 5.0.β
R=0.6
$\alpha_s=\alpha_{s0}$
Separation: $q_{50}^{rej}$
Q [GeV]
1
0.95
0.9
0.85
0.8
0.75
0.7
0.65
0.6
0.55
50
100
200
500
1000

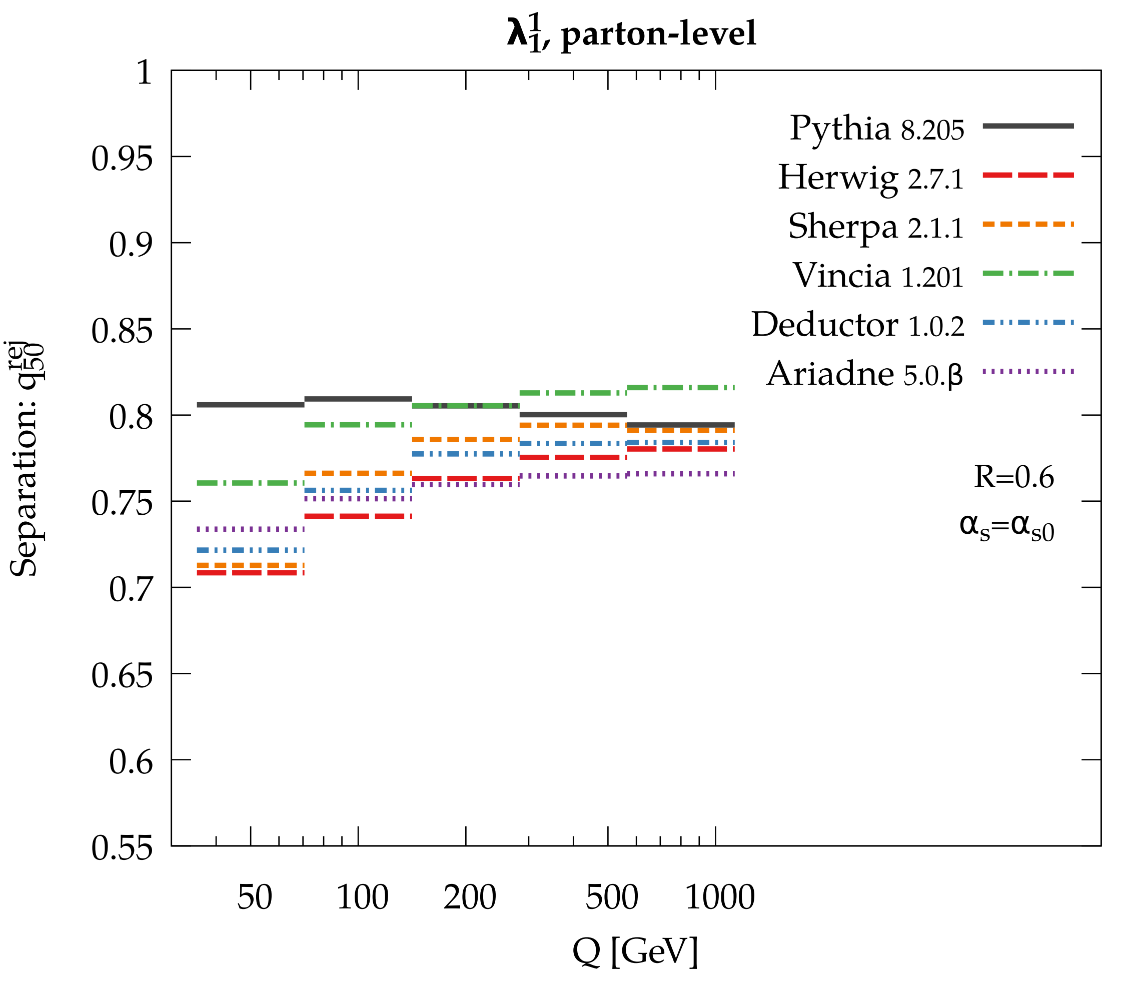

$\lambda_1^1$, parton-level
Pythia 8.205
Herwig 2.7.1
Sherpa 2.1.1
Vincia 1.201
Deductor 1.0.2
Ariadne 5.0.β
R=0.6
$\alpha_s=\alpha_{s0}$
Separation: $q_{50}^{rej}$
Q [GeV]
1
0.95
0.9
0.85
0.8
0.75
0.7
0.65
0.6
0.55
50
100
200
500
1000

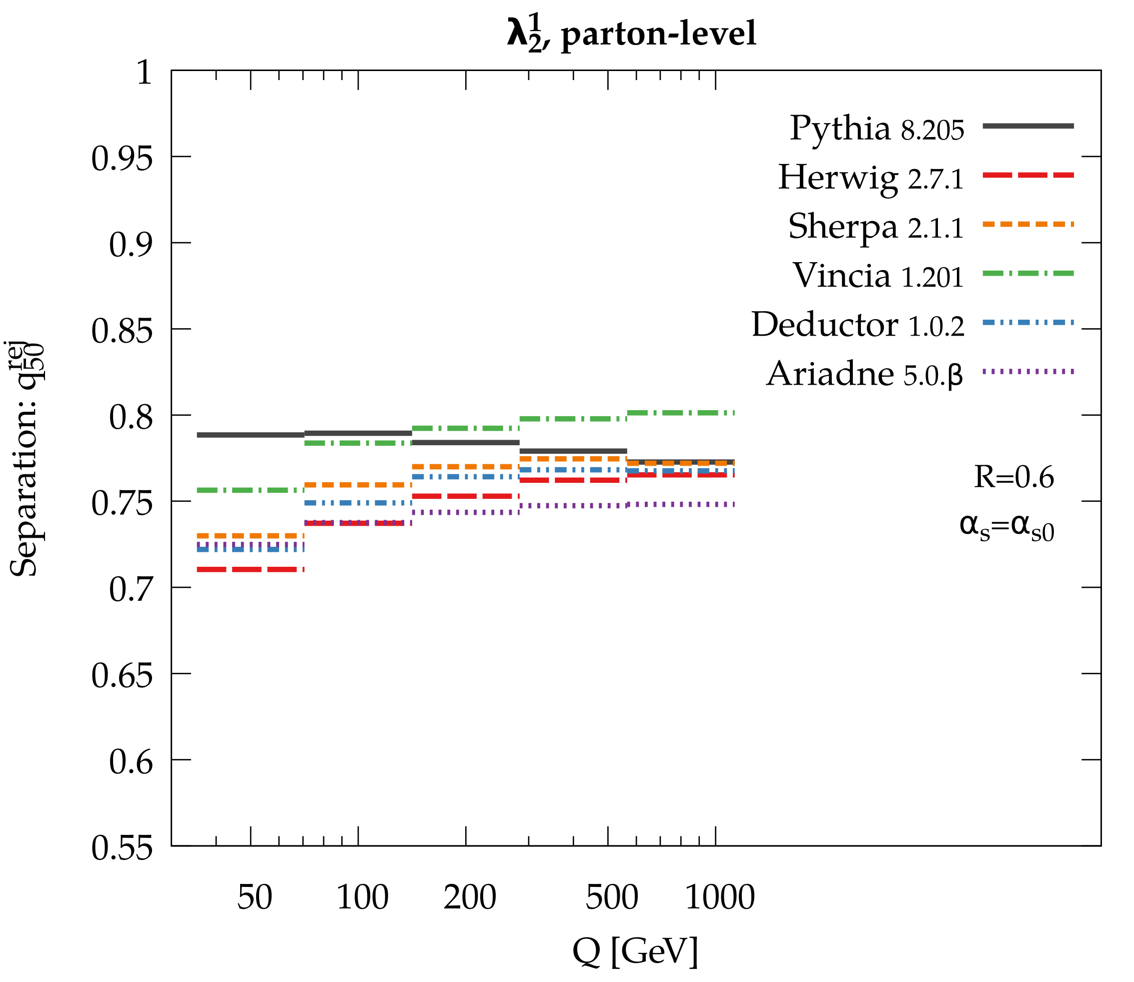

λ₂¹, parton-level
Pythia 8.205
Herwig 2.7.1
Sherpa 2.1.1
Vincia 1.201
Deductor 1.0.2
Ariadne 5.0.β
R=0.6
αs=αs0
Separation: q50rej
Q [GeV]
1
0.95
0.9
0.85
0.8
0.75
0.7
0.65
0.6
0.55
50
100
200
500
1000

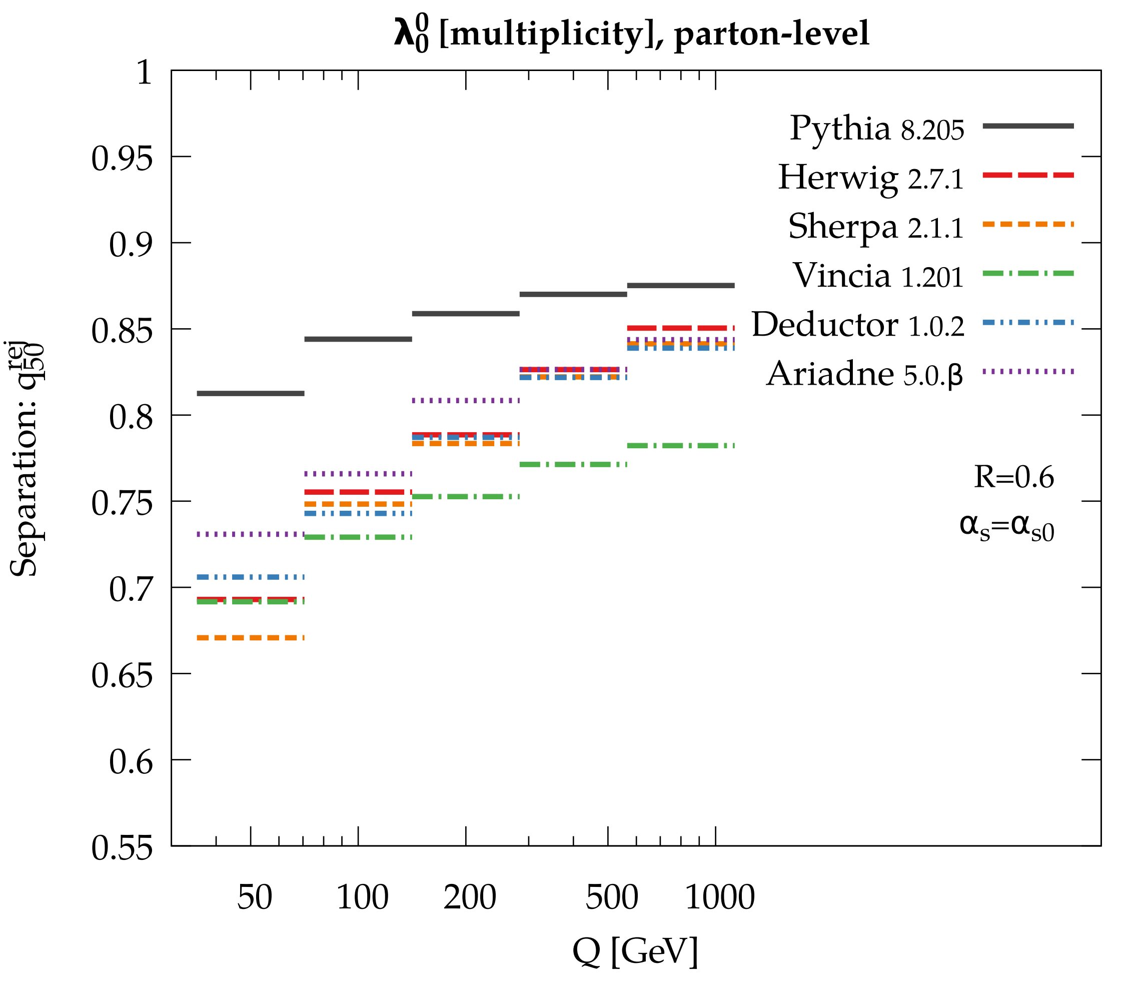

$\lambda_0^0$ [multiplicity], parton-level
Separation: $q_{50}^{rej}$
Q [GeV]
1
0.95
0.9
0.85
0.8
0.75
0.7
0.65
0.6
0.55
50
100
200
500
1000
Pythia 8.205
Herwig 2.7.1
Sherpa 2.1.1
Vincia 1.201
Deductor 1.0.2
Ariadne 5.0.β
R=0.6
$\alpha_s=\alpha_{s0}$

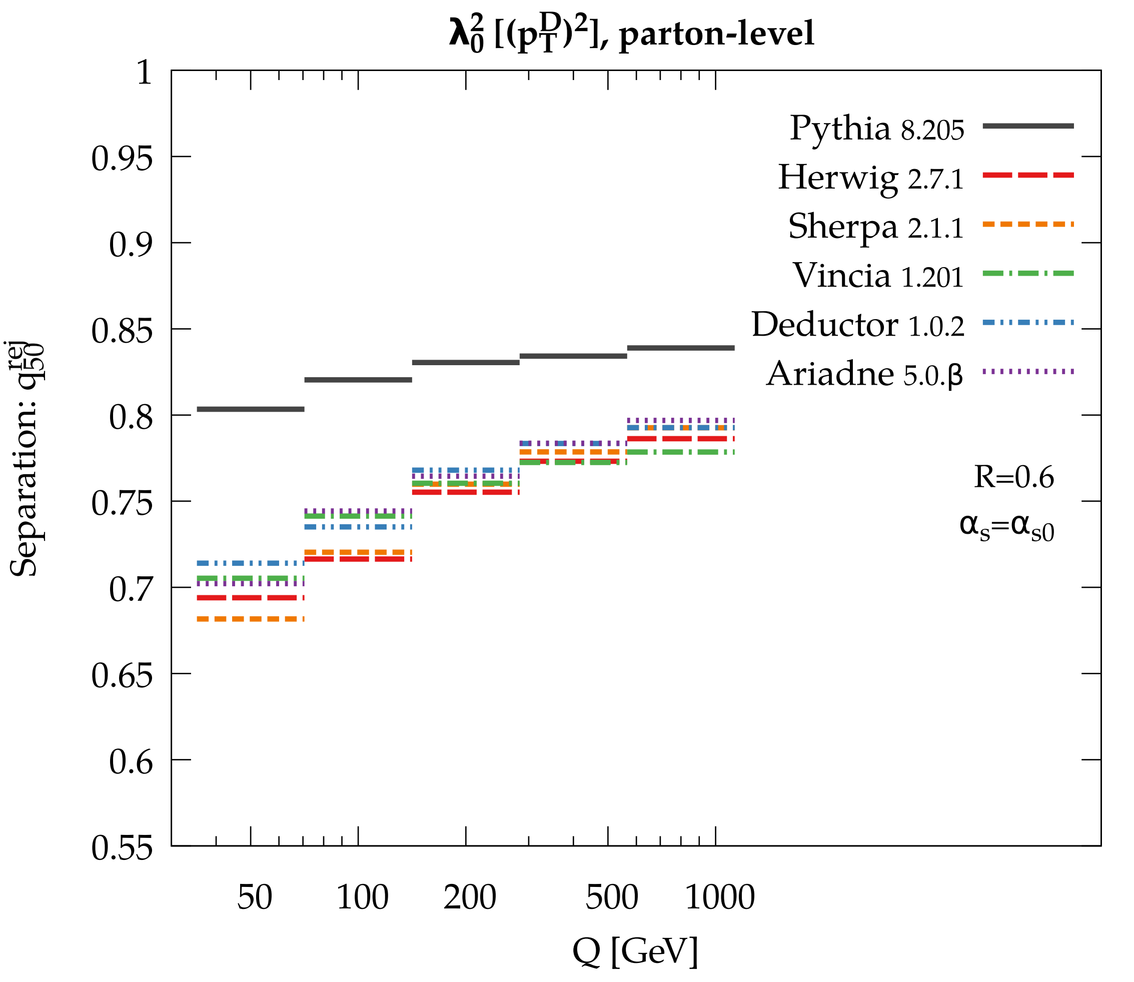

$\lambda_0^2\ [(p_T^D)^2]$, parton-level
Pythia 8.205
Herwig 2.7.1
Sherpa 2.1.1
Vincia 1.201
Deductor 1.0.2
Ariadne 5.0.β
R=0.6
$\alpha_s=\alpha_{s0}$
Separation: $q_{50}^{rej}$
1
0.95
0.9
0.85
0.8
0.75
0.7
0.65
0.6
0.55
50
100
200
500
1000
Q [GeV]

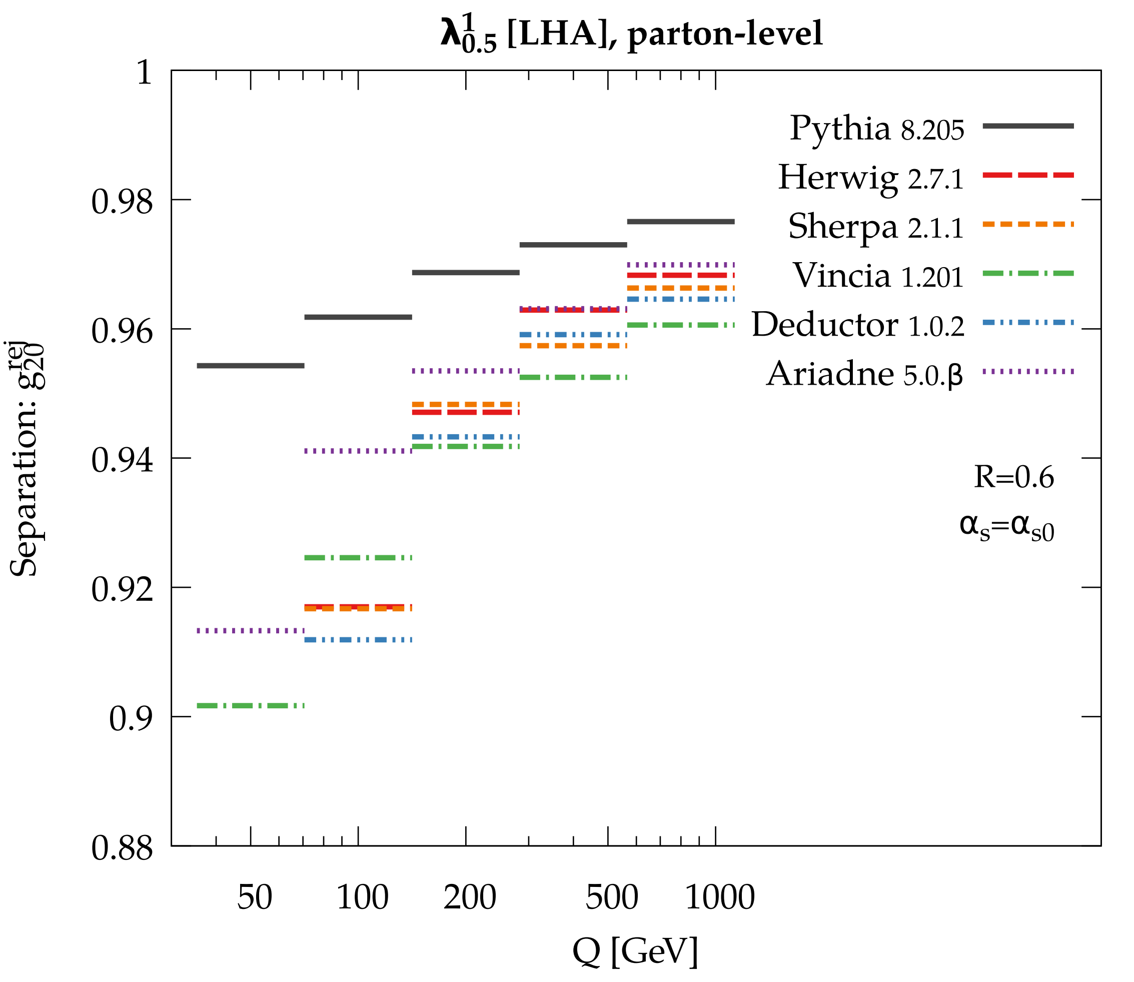

λ^1_0.5 [LHA], parton-level
Separation: g^rej_20
Q [GeV]
Pythia 8.205
Herwig 2.7.1
Sherpa 2.1.1
Vincia 1.201
Deductor 1.0.2
Ariadne 5.0.β
R=0.6
αs=αs0
1
0.98
0.96
0.94
0.92
0.9
0.88
50
100
200
500
1000

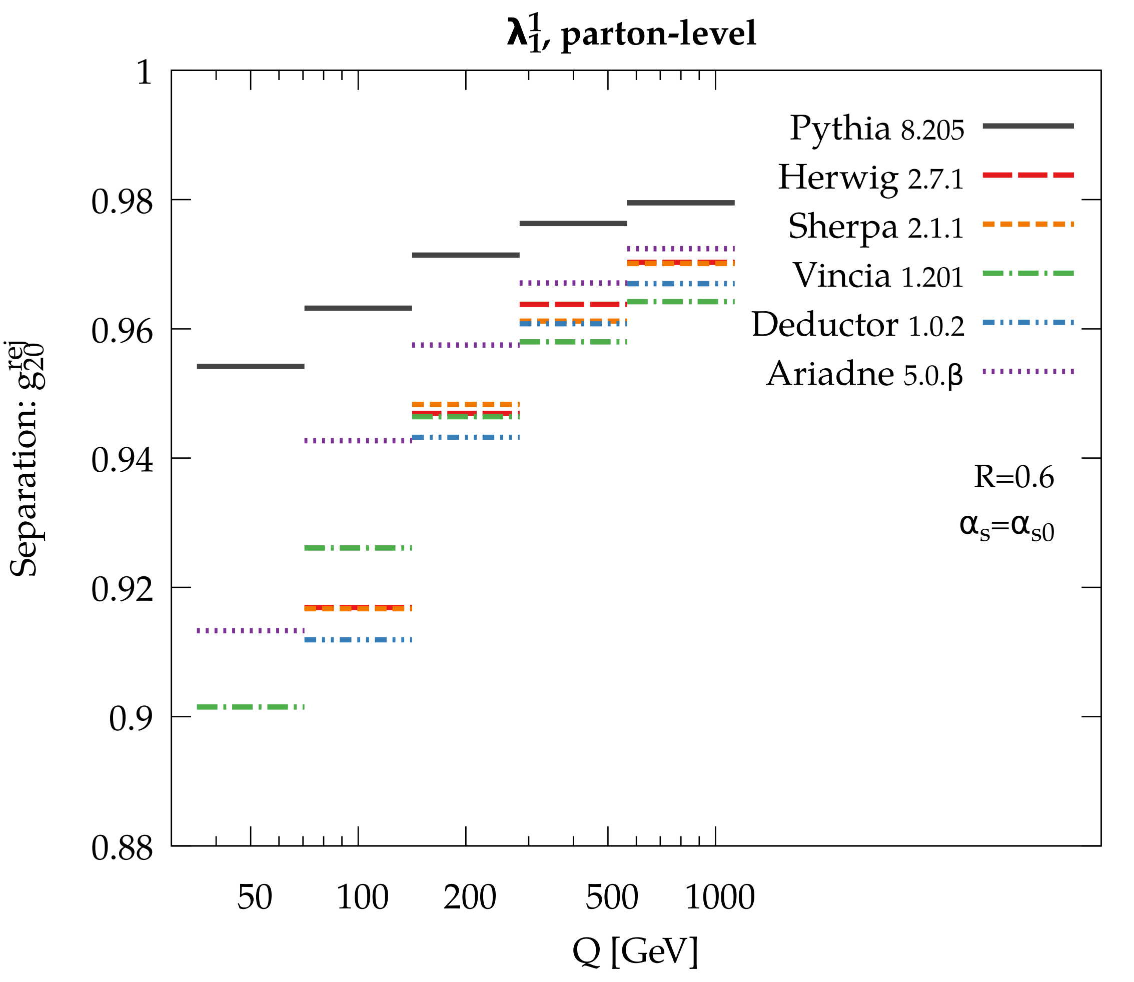

λ₁¹, parton-level
Pythia 8.205
Herwig 2.7.1
Sherpa 2.1.1
Vincia 1.201
Deductor 1.0.2
Ariadne 5.0.β
R=0.6
αs=αs0
Separation: g20rej
Q [GeV]
1
0.98
0.96
0.94
0.92
0.9
0.88
50
100
200
500
1000

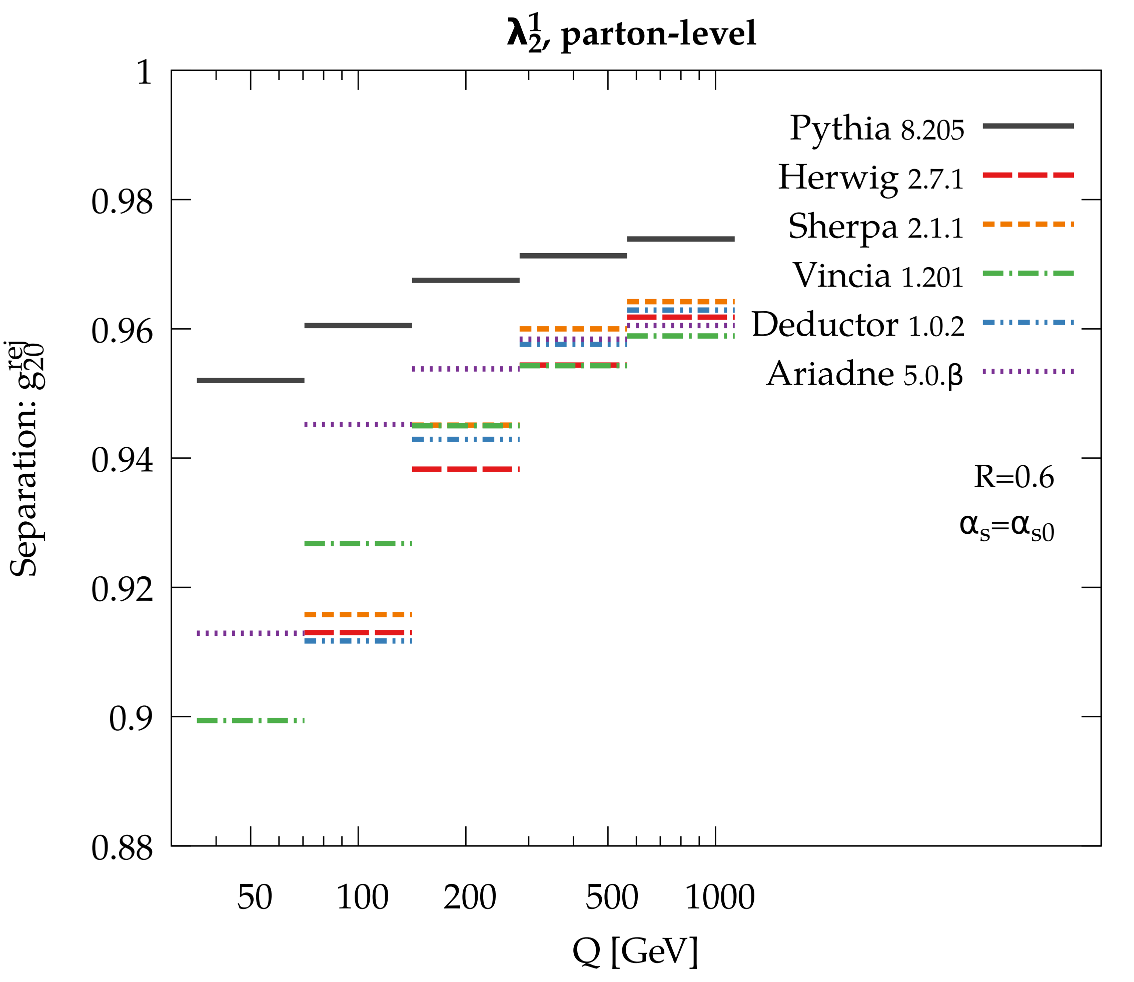

$\lambda_2^1$, parton-level
1
0.98
0.96
0.94
0.92
0.9
0.88
Separation: $g_{20}^{\mathrm{rej}}$
50
100
200
500
1000
Q [GeV]
Pythia 8.205
Herwig 2.7.1
Sherpa 2.1.1
Vincia 1.201
Deductor 1.0.2
Ariadne 5.0.β
R=0.6
$\alpha_s=\alpha_{s0}$

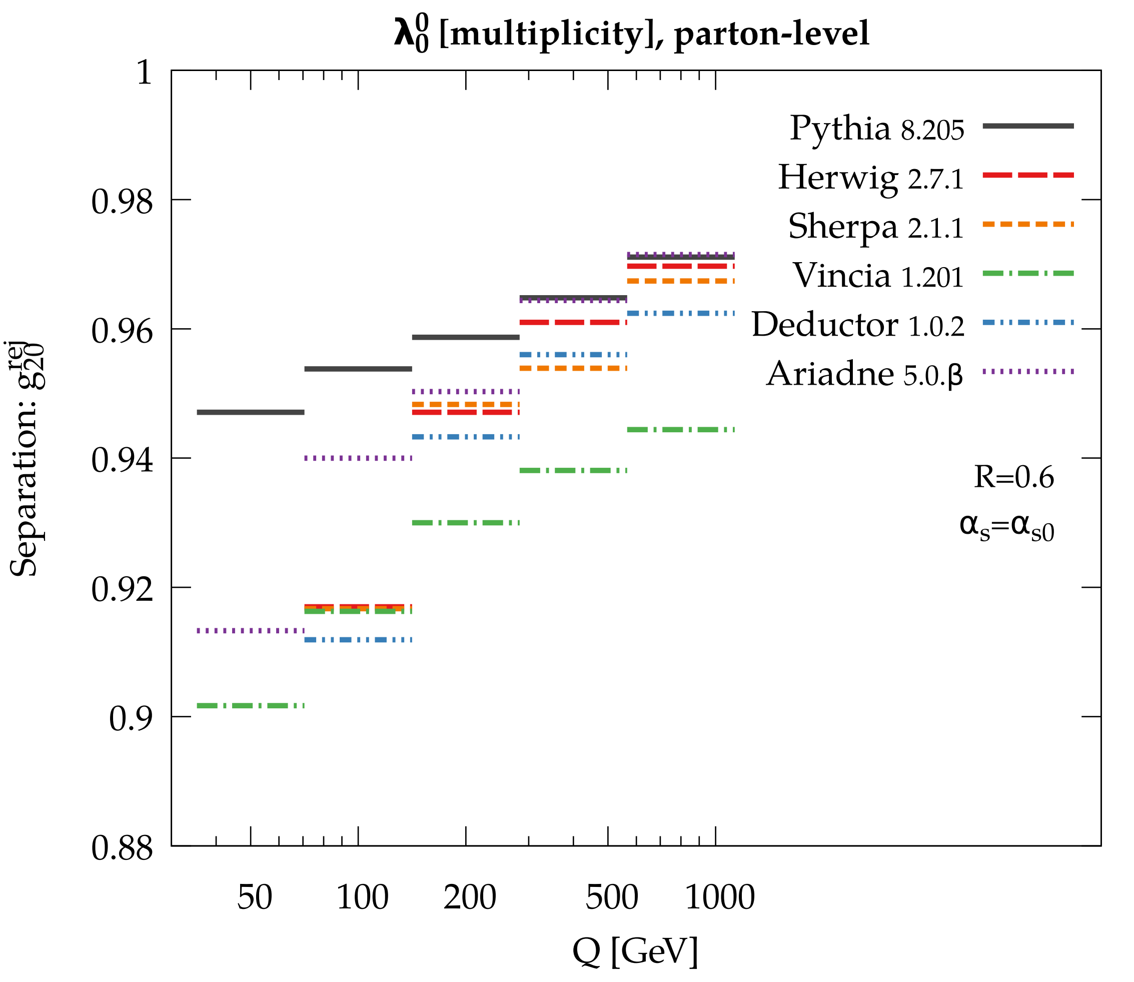

$\lambda_0^0$ [multiplicity], parton-level
Separation: $g_{20}^{rej}$
Q [GeV]
1
0.98
0.96
0.94
0.92
0.9
0.88
50
100
200
500
1000
Pythia 8.205
Herwig 2.7.1
Sherpa 2.1.1
Vincia 1.201
Deductor 1.0.2
Ariadne 5.0.β
R=0.6
$\alpha_s=\alpha_{s0}$

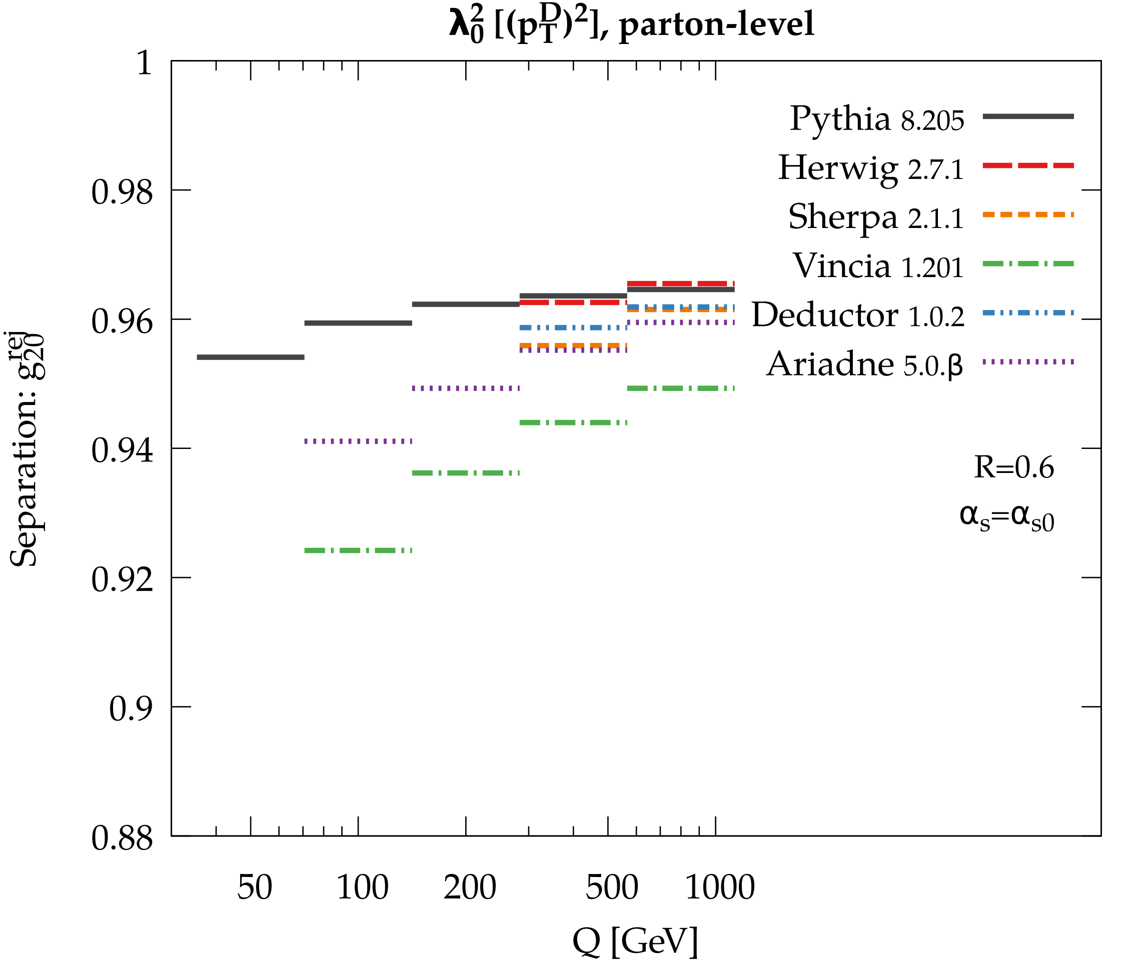
$\lambda_0^2$ [$(p_T^D)^2$], parton-level
Separation: $g_{20}^{rej}$
Q [GeV]
1
0.98
0.96
0.94
0.92
0.9
0.88
50
100
200
500
1000
Pythia 8.205
Herwig 2.7.1
Sherpa 2.1.1
Vincia 1.201
Deductor 1.0.2
Ariadne 5.0.β
R=0.6
$\alpha_s$=$\alpha_{s0}$

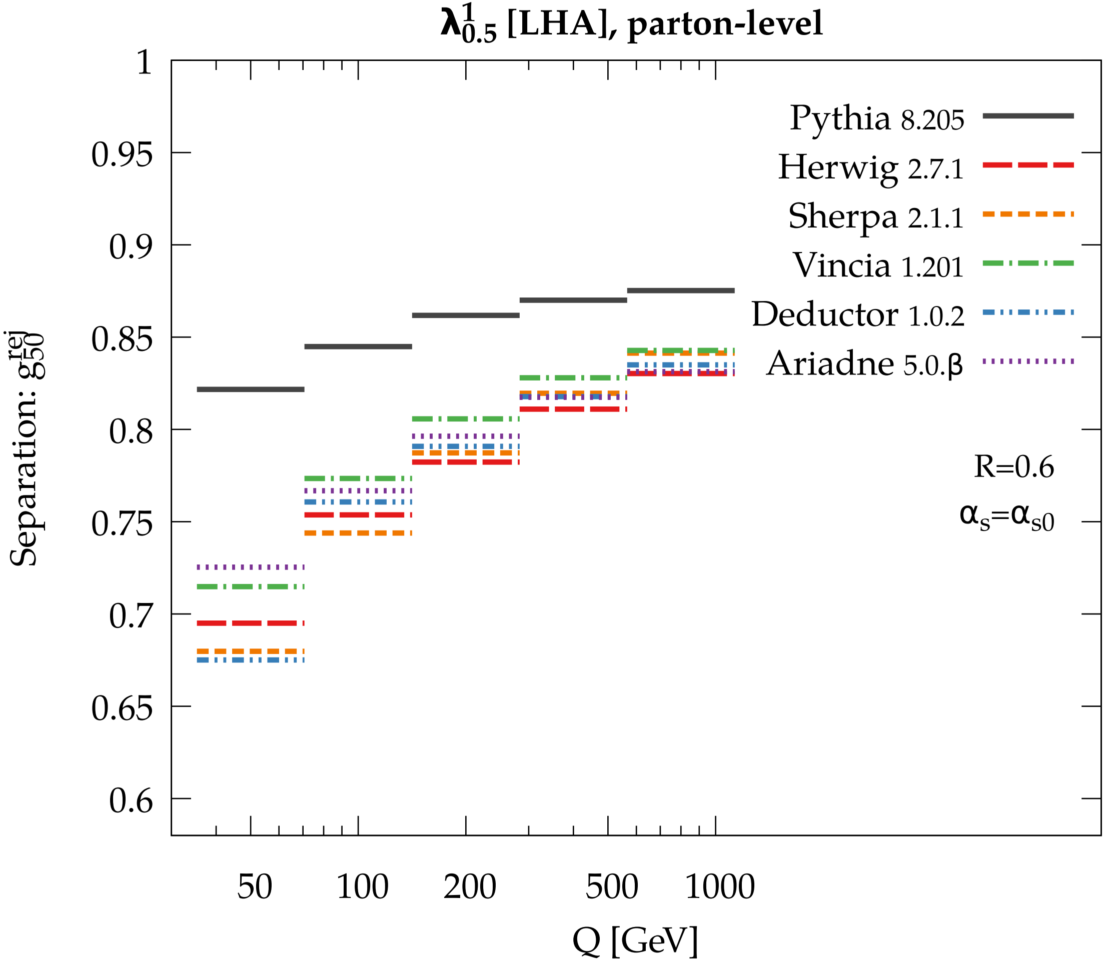

λ$^1_{0.5}$ [LHA], parton-level
Pythia 8.205
Herwig 2.7.1
Sherpa 2.1.1
Vincia 1.201
Deductor 1.0.2
Ariadne 5.0.β
R=0.6
α$_s$=α$_{s0}$
Separation: $g_{50}^{rej}$
Q [GeV]
1
0.95
0.9
0.85
0.8
0.75
0.7
0.65
0.6
50
100
200
500
1000

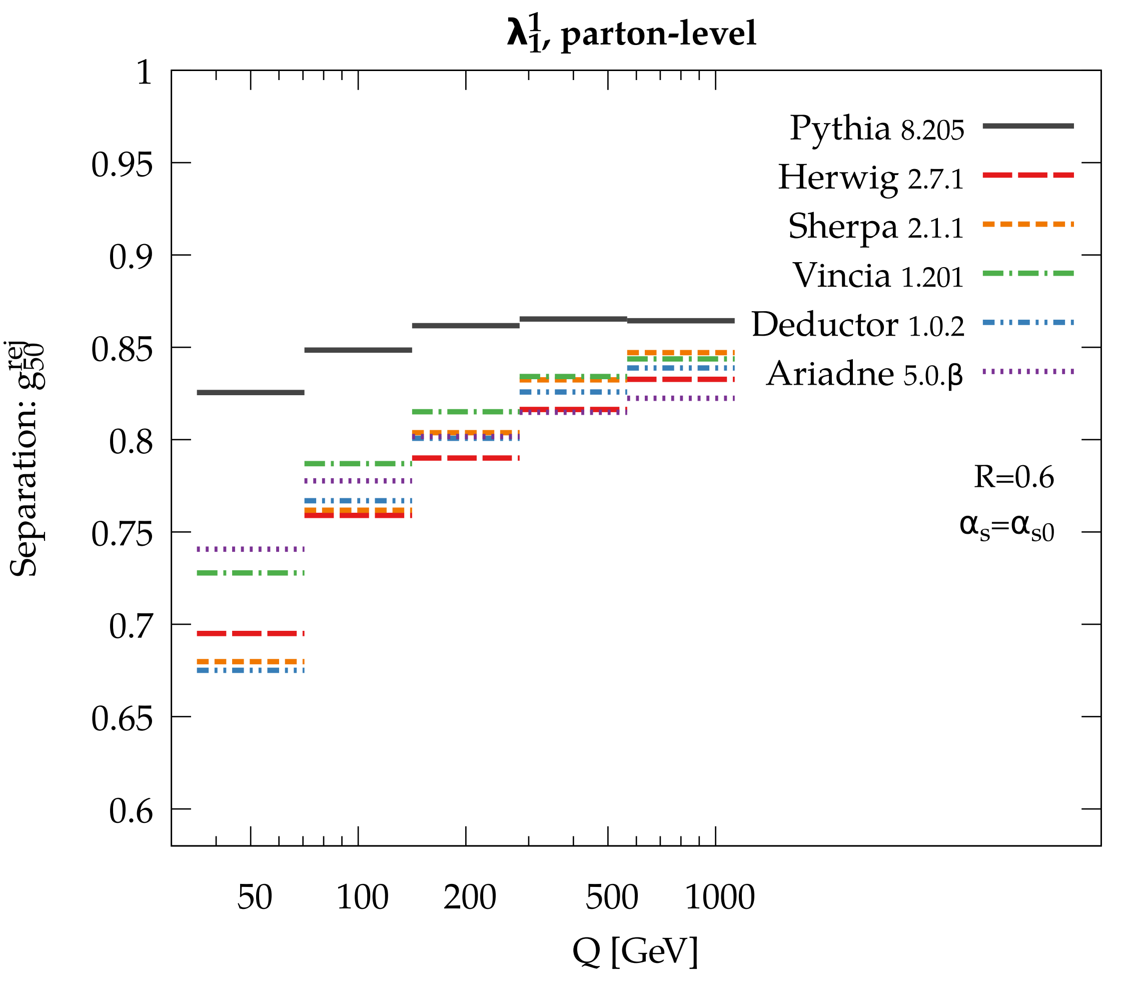

$\lambda_1^1$, parton-level
1
0.95
0.9
0.85
0.8
0.75
0.7
0.65
0.6
Separation: $g_{50}^{rej}$
50
100
200
500
1000
Q [GeV]
Pythia 8.205
Herwig 2.7.1
Sherpa 2.1.1
Vincia 1.201
Deductor 1.0.2
Ariadne 5.0.β
R=0.6
$\alpha_s=\alpha_{s0}$

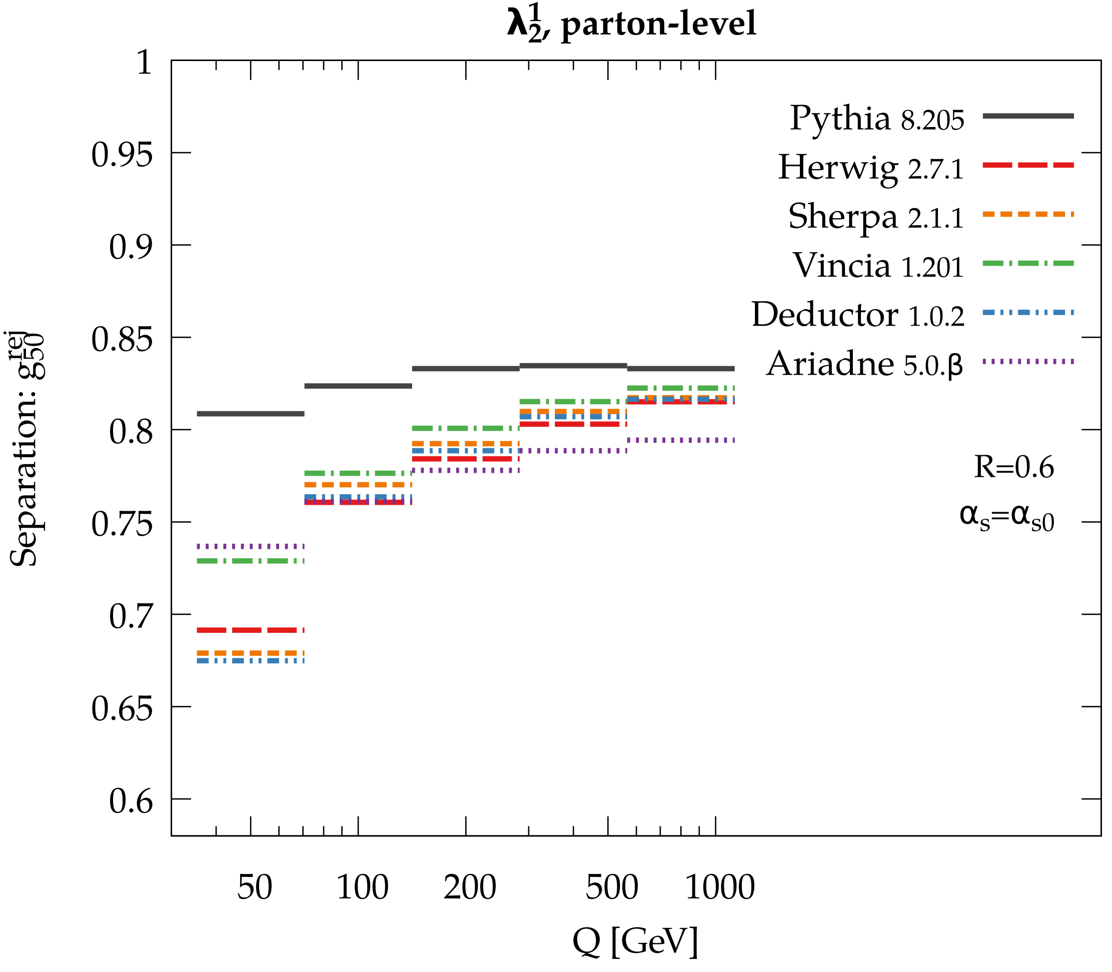

λ21, parton-level
Pythia 8.205
Herwig 2.7.1
Sherpa 2.1.1
Vincia 1.201
Deductor 1.0.2
Ariadne 5.0.β
R=0.6
αs=αs0
Separation: g50rej
Q [GeV]
0.6
0.65
0.7
0.75
0.8
0.85
0.9
0.95
1
50
100
200
500
1000

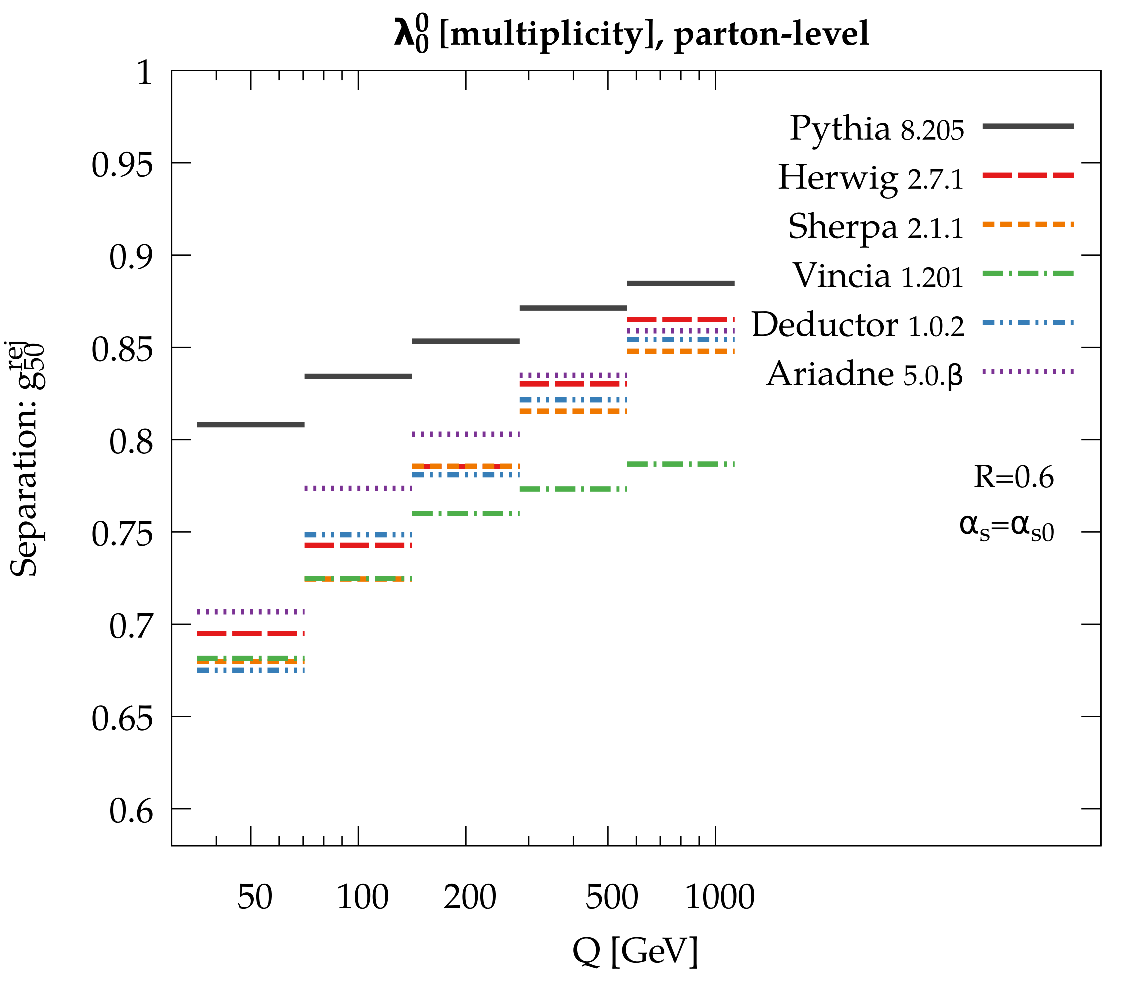

$\lambda_0^0$ [multiplicity], parton-level
Separation: $g_{50}^{rej}$
Q [GeV]
1
0.95
0.9
0.85
0.8
0.75
0.7
0.65
0.6
50
100
200
500
1000
Pythia 8.205
Herwig 2.7.1
Sherpa 2.1.1
Vincia 1.201
Deductor 1.0.2
Ariadne 5.0.β
R=0.6
$\alpha_s = \alpha_{s0}$

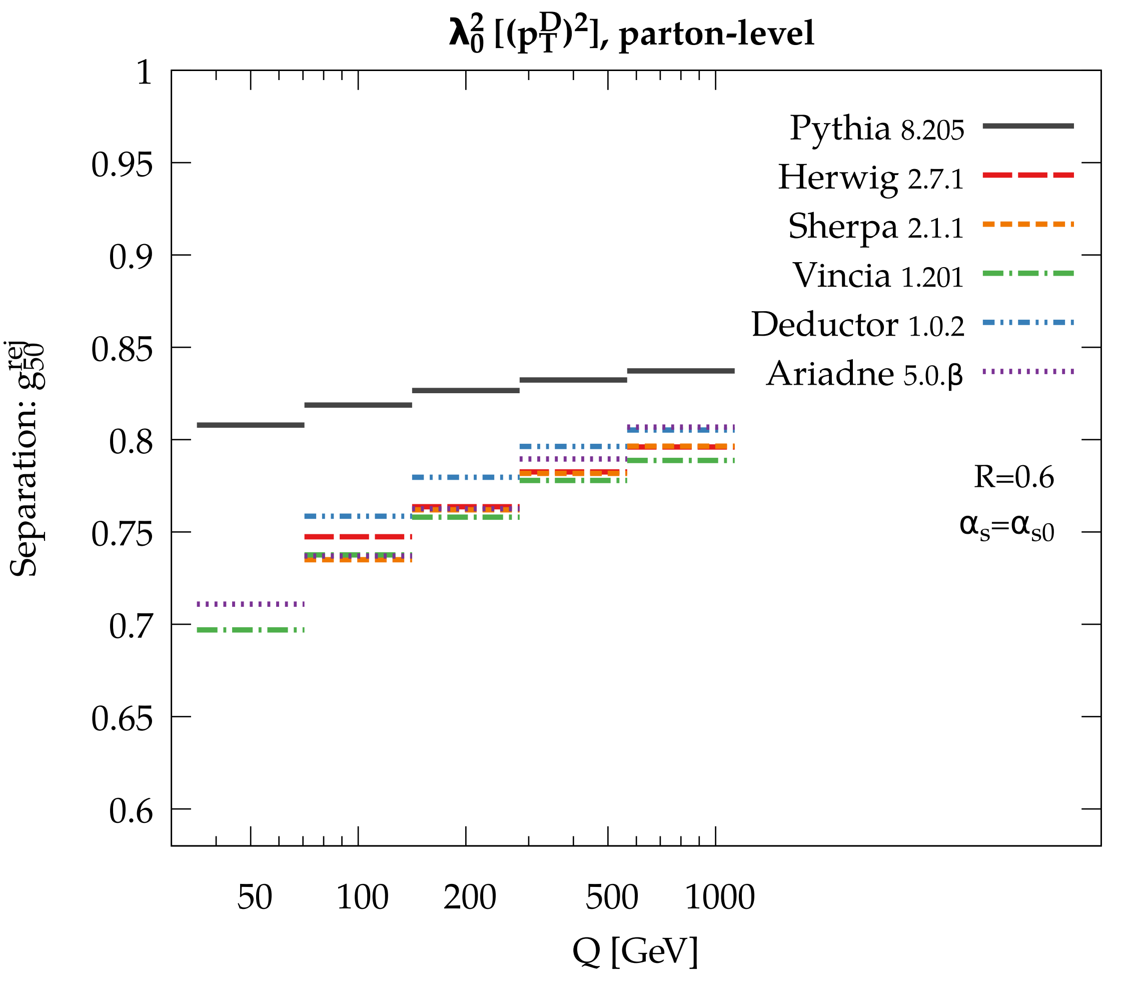

$\lambda_0^2\ [(p_T^D)^2]$, parton-level
Separation: $g_{50}^{rej}$
Q [GeV]
Pythia 8.205
Herwig 2.7.1
Sherpa 2.1.1
Vincia 1.201
Deductor 1.0.2
Ariadne 5.0.β
R=0.6
$\alpha_s=\alpha_{s0}$
1
0.95
0.9
0.85
0.8
0.75
0.7
0.65
0.6
50
100
200
500
1000

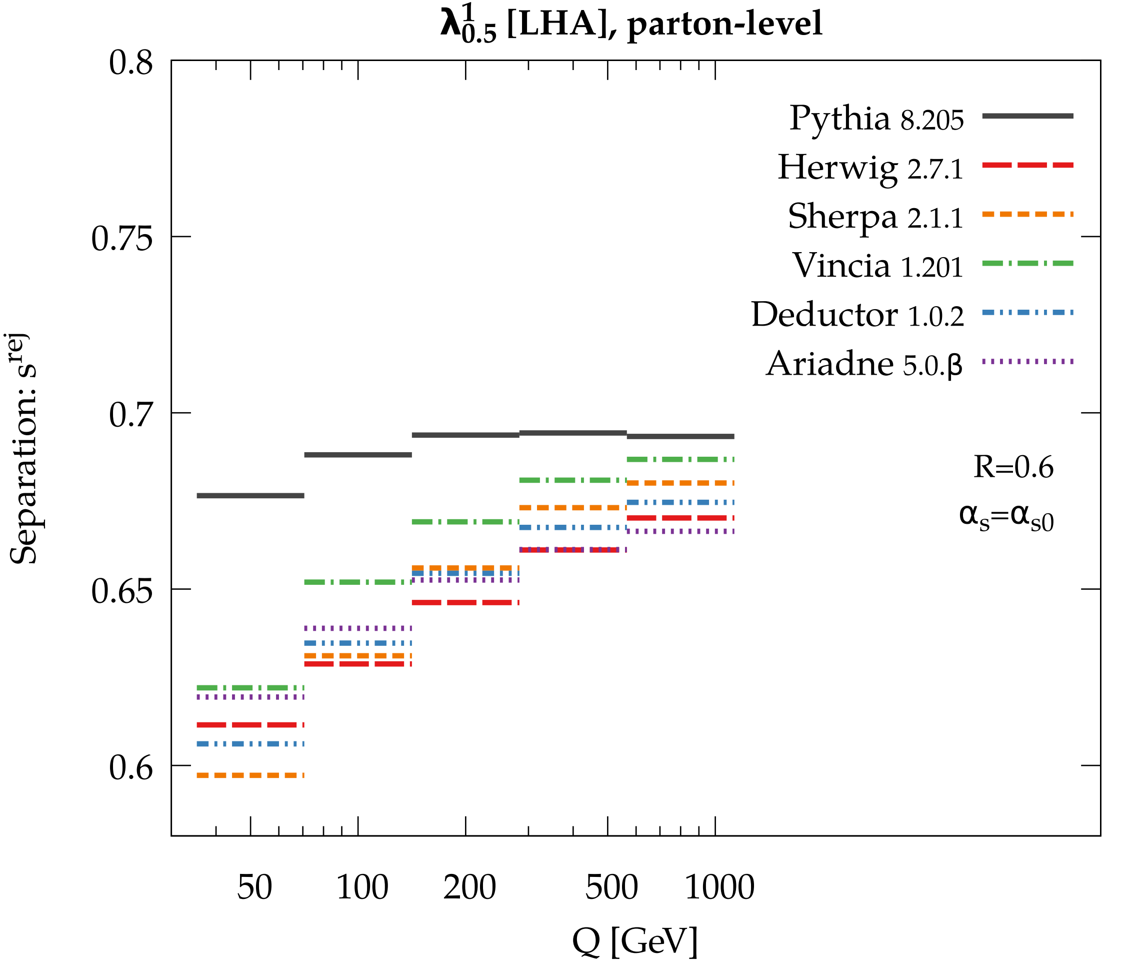

$\lambda^1_{0.5}$ [LHA], parton-level
Separation: $s^{rej}$
0.8
0.75
0.7
0.65
0.6
Pythia 8.205
Herwig 2.7.1
Sherpa 2.1.1
Vincia 1.201
Deductor 1.0.2
Ariadne 5.0.β
R=0.6
$\alpha_s = \alpha_{s0}$
50
100
200
500
1000
Q [GeV]

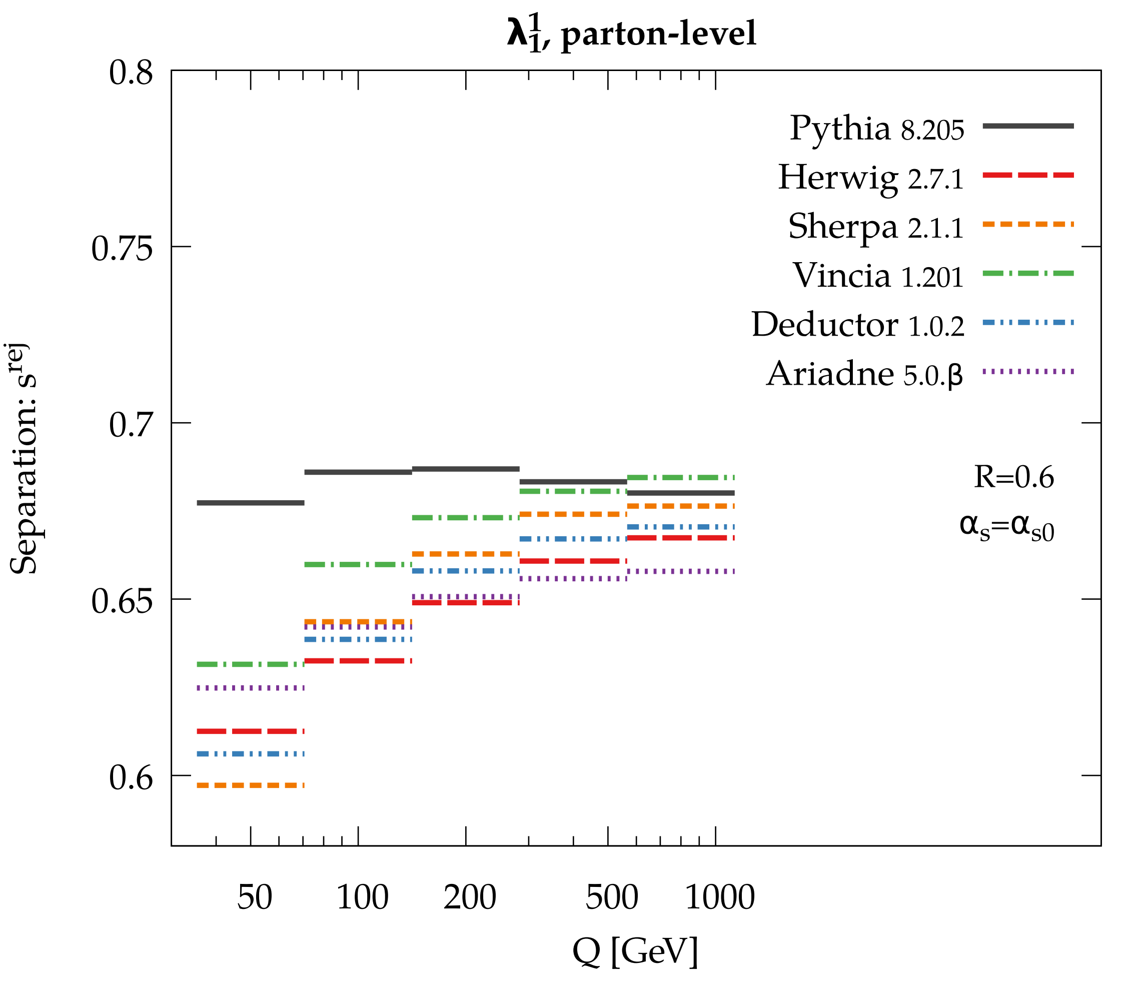

$\lambda_1^1$, parton-level
Separation: $s^{rej}$
0.8
0.75
0.7
0.65
0.6
Pythia 8.205
Herwig 2.7.1
Sherpa 2.1.1
Vincia 1.201
Deductor 1.0.2
Ariadne 5.0.β
R=0.6
$\alpha_s=\alpha_{s0}$
50
100
200
500
1000
Q [GeV]

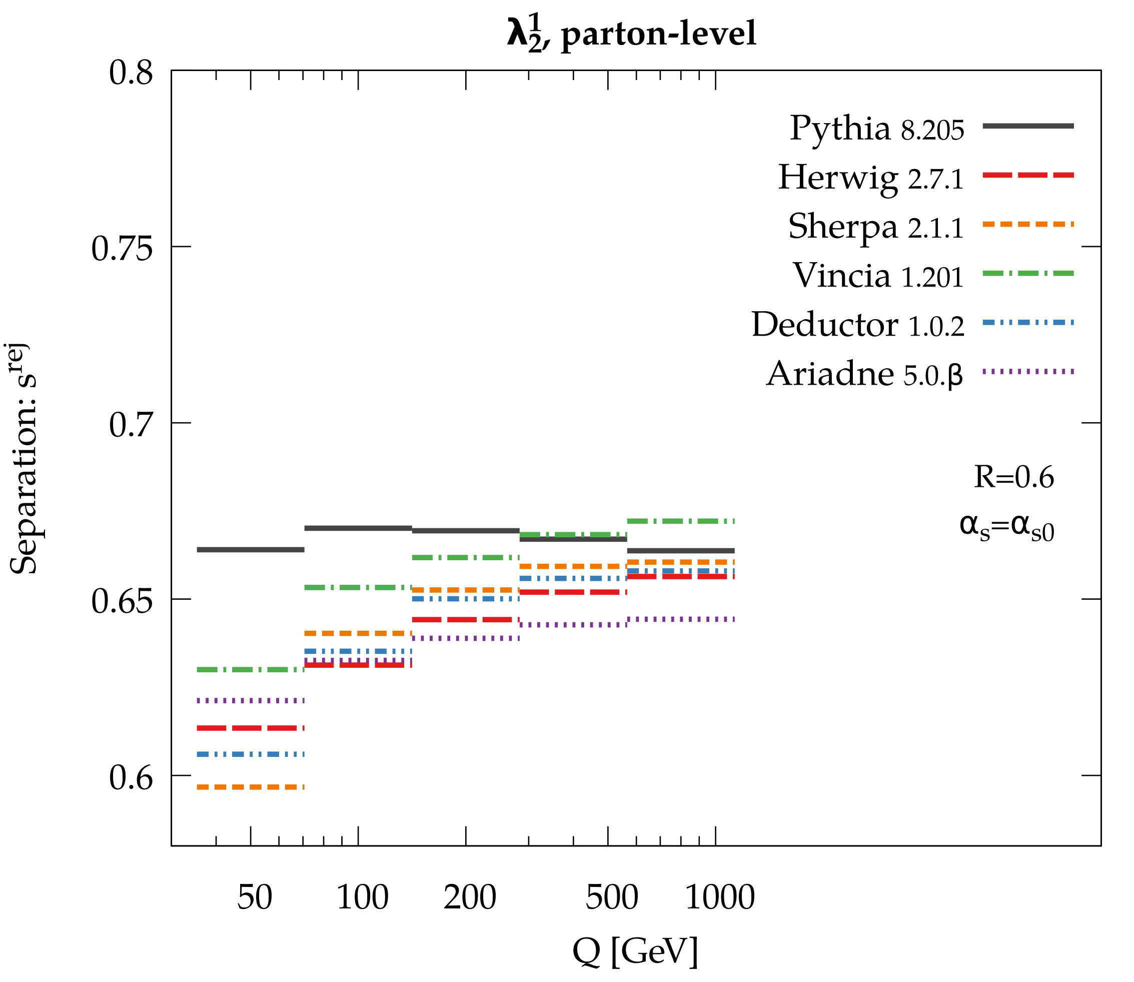

$\lambda_2^1$, parton-level
Separation: $s^{rej}$
0.8
0.75
0.7
0.65
0.6
Pythia 8.205
Herwig 2.7.1
Sherpa 2.1.1
Vincia 1.201
Deductor 1.0.2
Ariadne 5.0.β
R=0.6
$\alpha_s=\alpha_{s0}$
50
100
200
500
1000
Q [GeV]

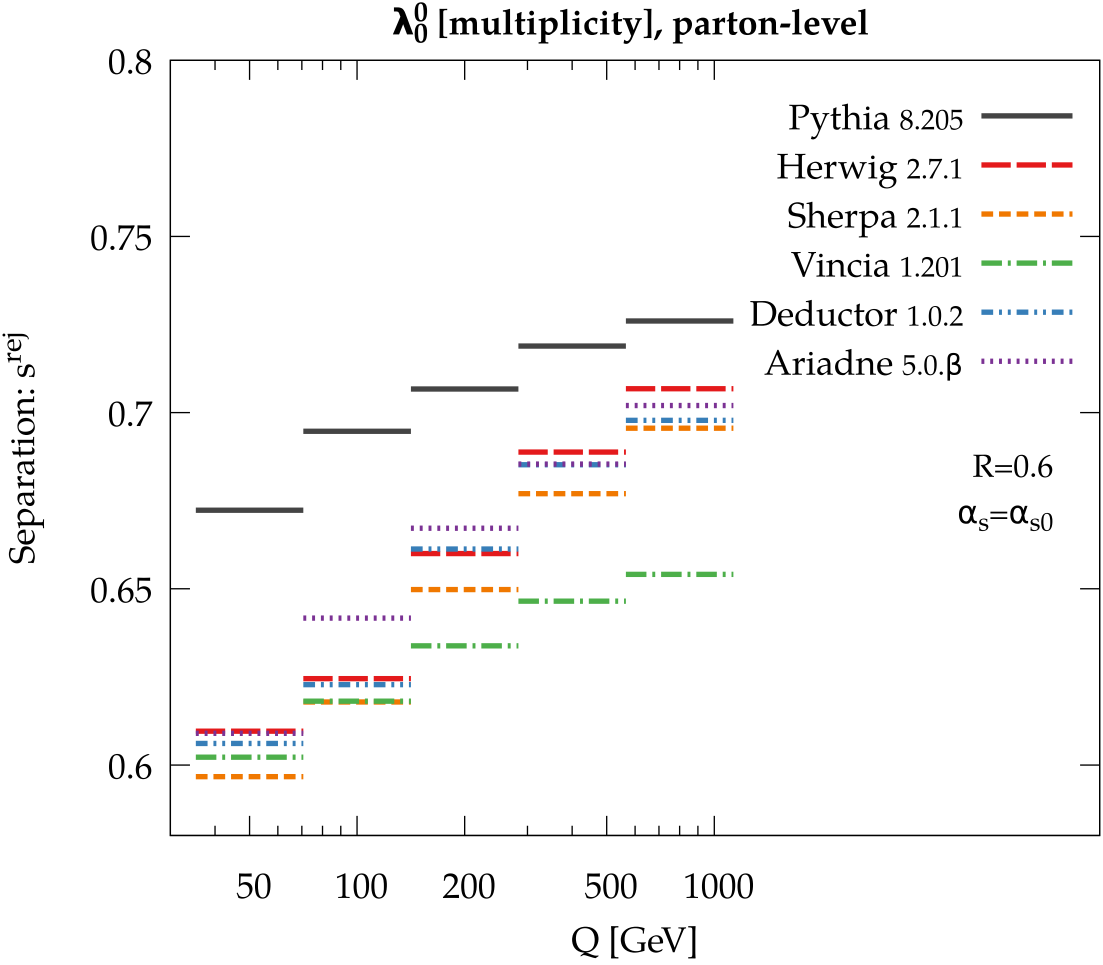
λ$_0^0$ [multiplicity], parton-level
0.8
0.75
0.7
0.65
0.6
Separation: s$^{rej}$
Pythia 8.205
Herwig 2.7.1
Sherpa 2.1.1
Vincia 1.201
Deductor 1.0.2
Ariadne 5.0.β
R=0.6
α$_s$=α$_{s0}$
50
100
200
500
1000
Q [GeV]

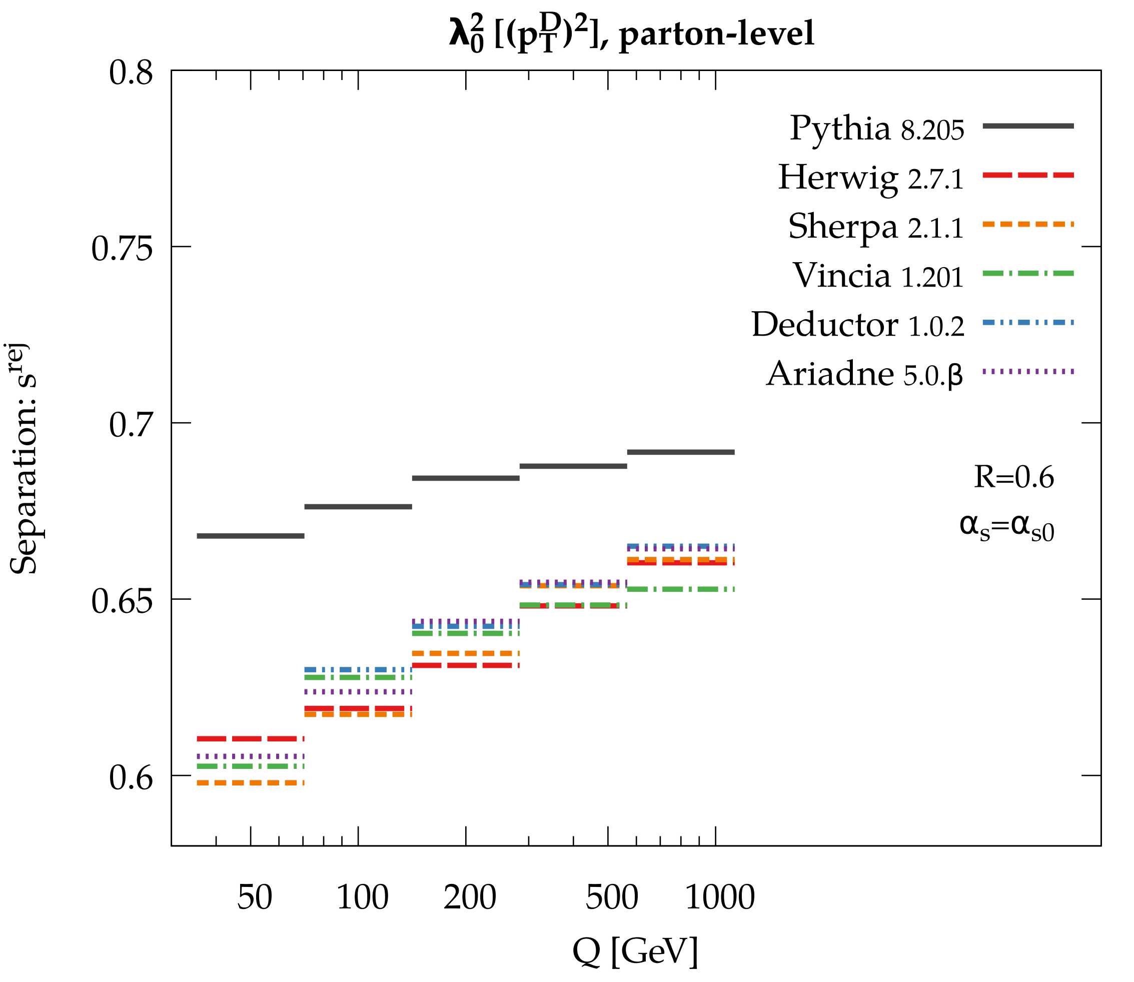

$\lambda_0^2\ [(p_T^D)^2]$, parton-level
Separation: $s^{rej}$
Q [GeV]
0.8
0.75
0.7
0.65
0.6
50
100
200
500
1000
Pythia 8.205
Herwig 2.7.1
Sherpa 2.1.1
Vincia 1.201
Deductor 1.0.2
Ariadne 5.0.β
R=0.6
$\alpha_s=\alpha_{s0}$
