# Supplementary material for: Les Houches 2015: Physics at TeV Colliders Standard Model Working Group Report
Source: arXiv:1605.04692 source file (2016-05-16)

# Separation, parton-level

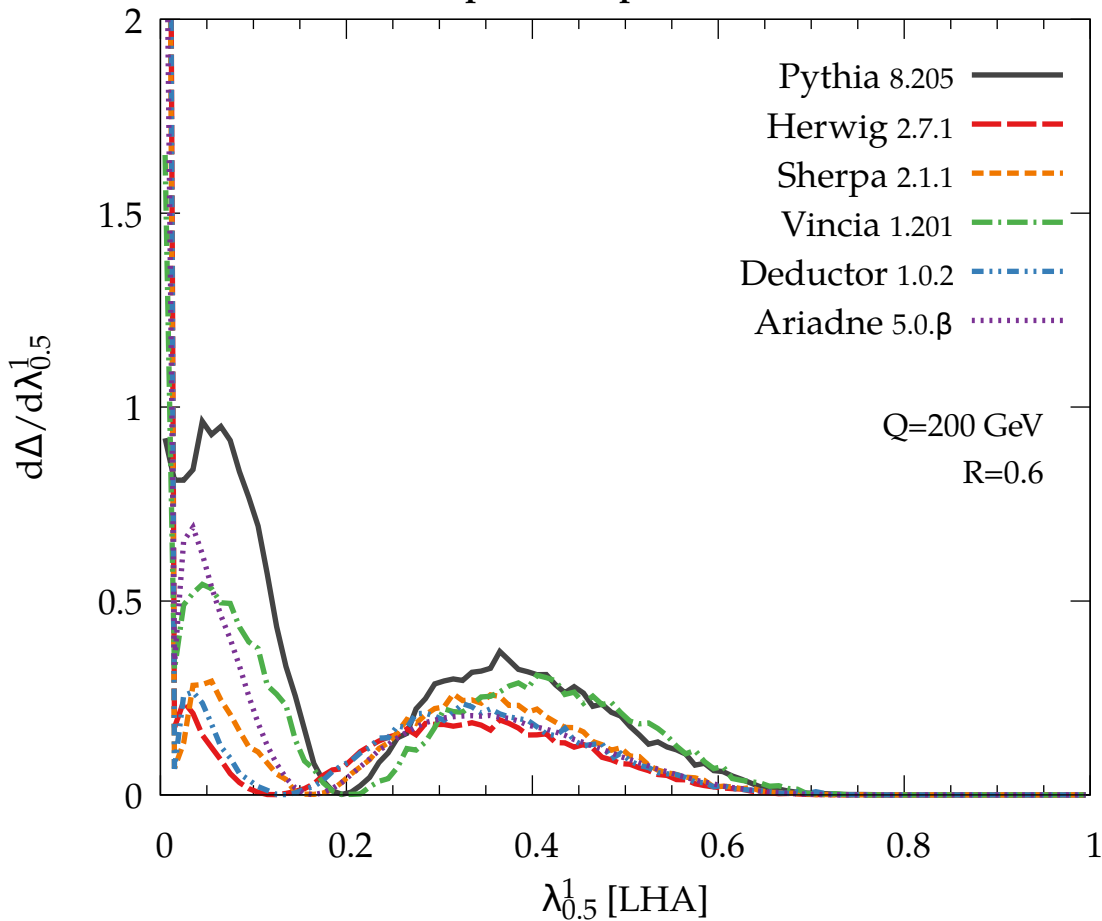

# Separation, parton-level

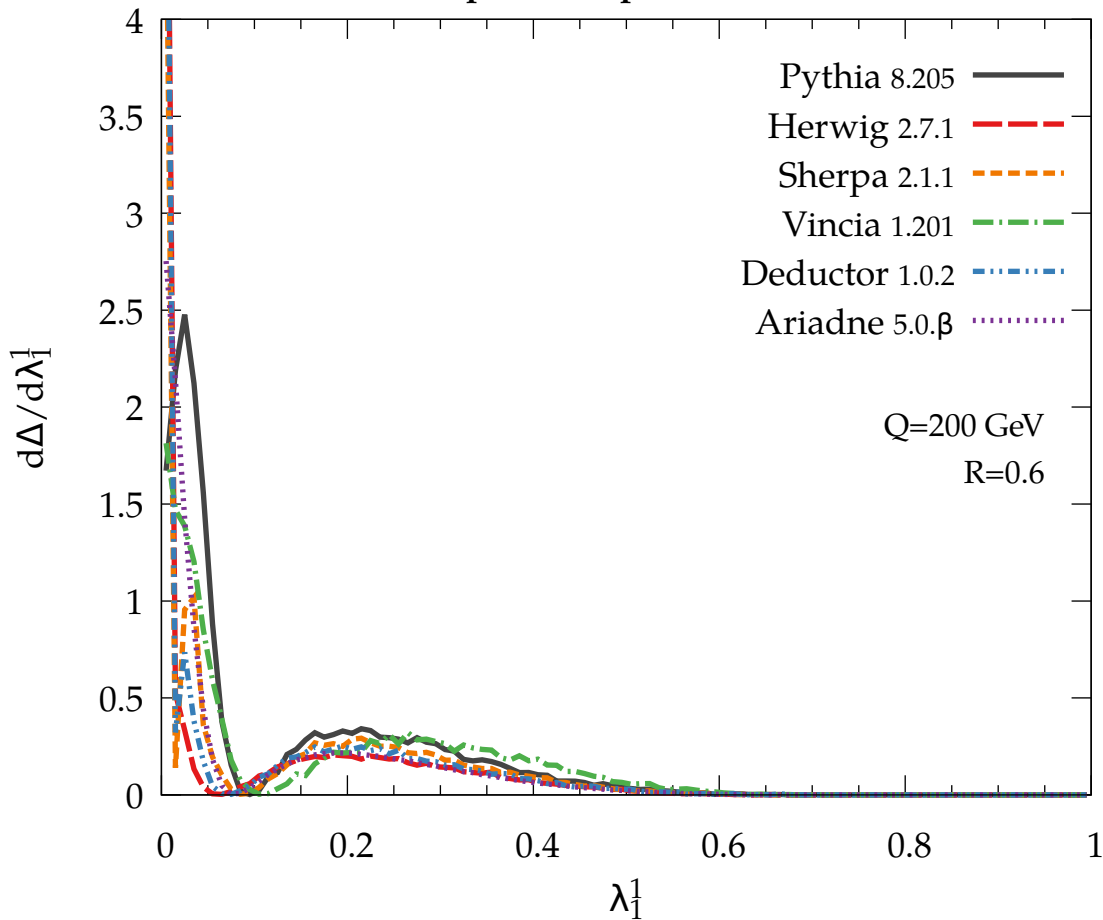

# Separation, parton-level

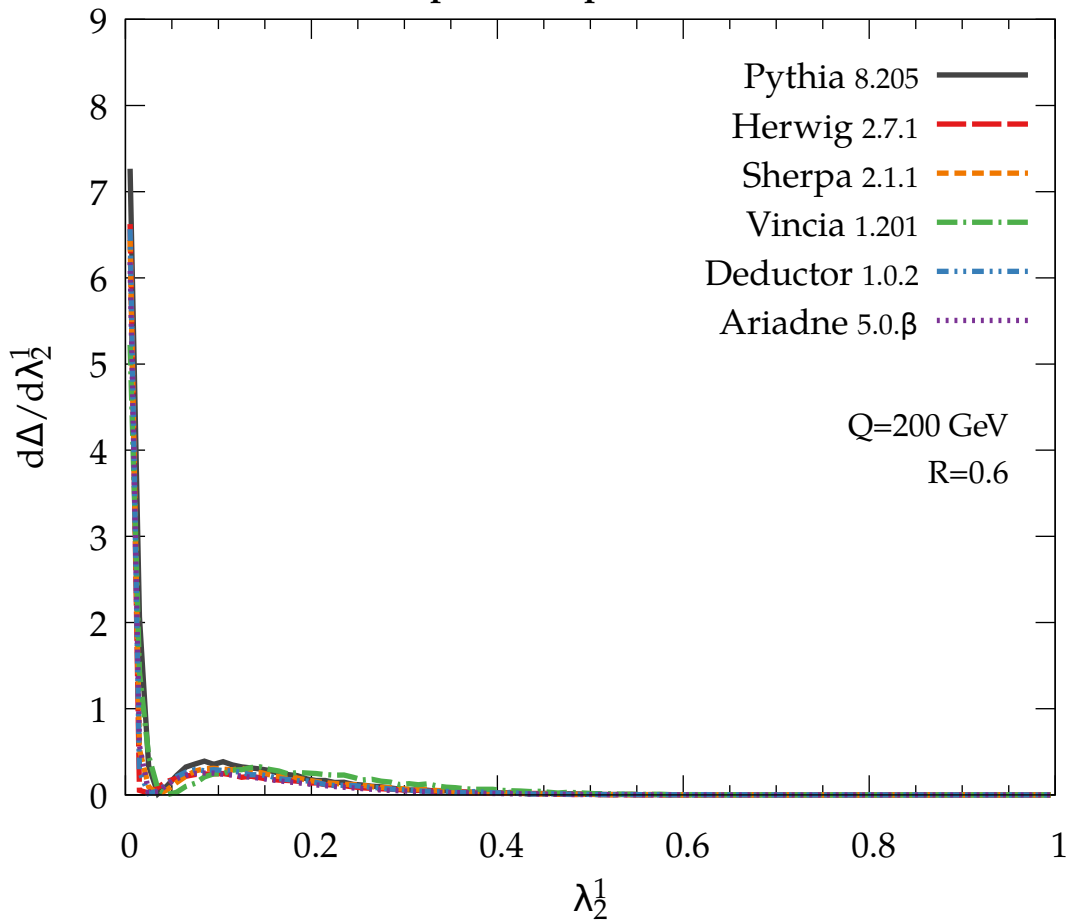

# Separation, parton-level

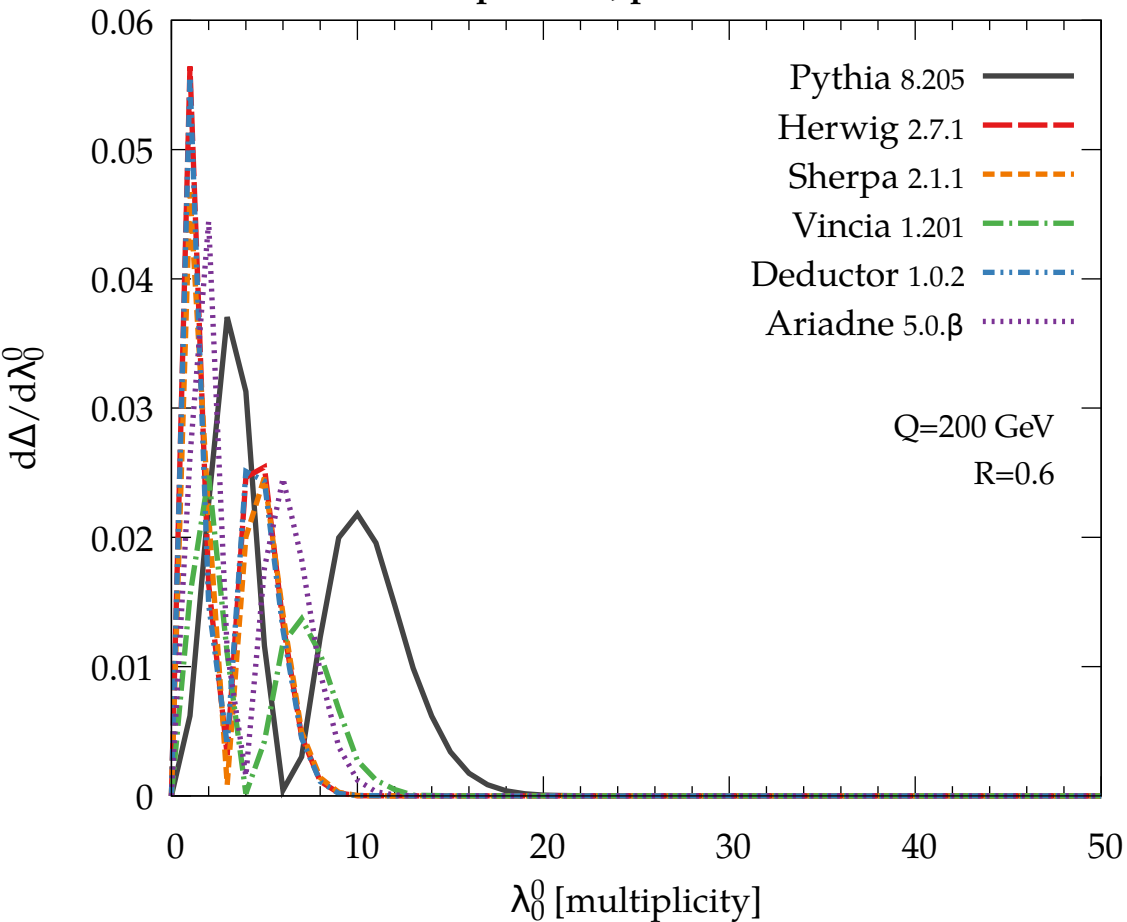

# Separation, parton-level

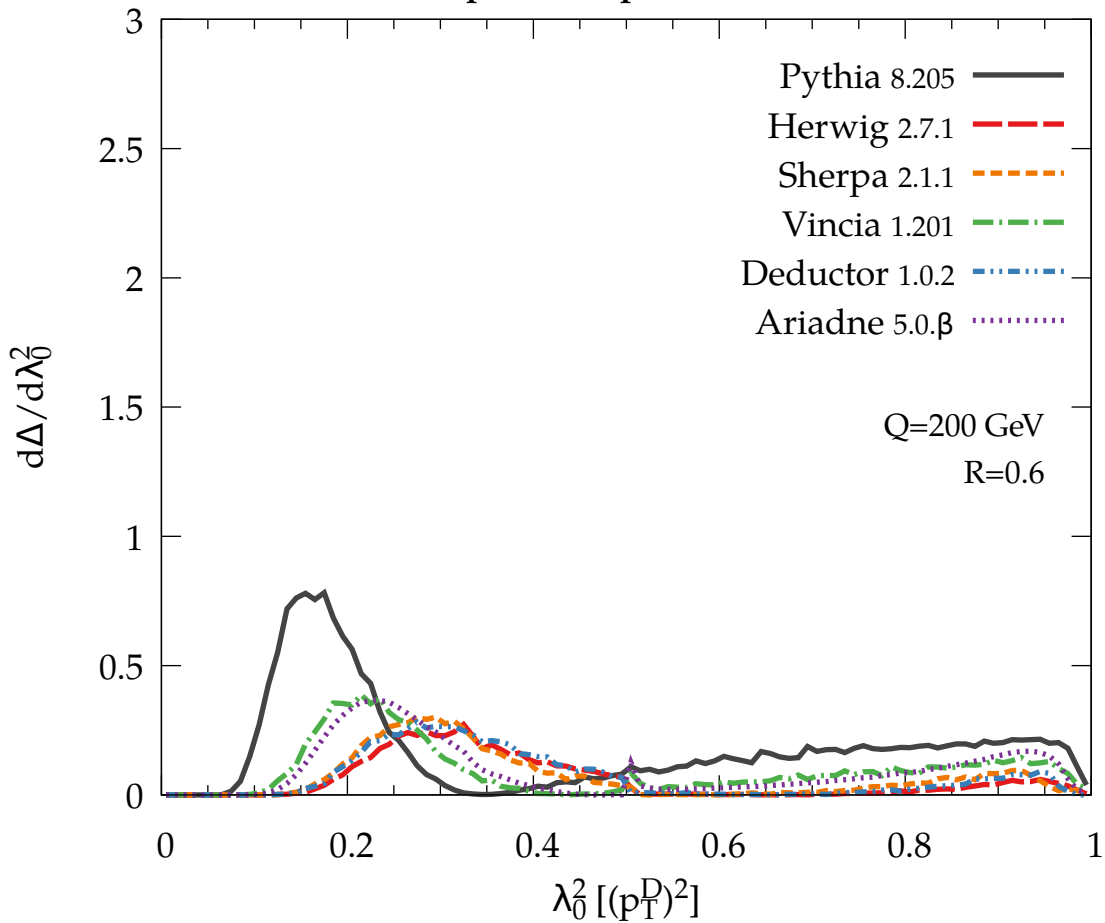

Supplement: Supplementary file 8 [file quarkgluon_fig_GA_10_05_R6_parton_separation.pdf]
