# Supplementary material for: Les Houches 2015: Physics at TeV Colliders Standard Model Working Group Report
Source: arXiv:1605.04692 source file (2016-05-16)

$\lambda_{0.5}^1$  [LHA], hadron-levelSeparation:  $\Delta$ 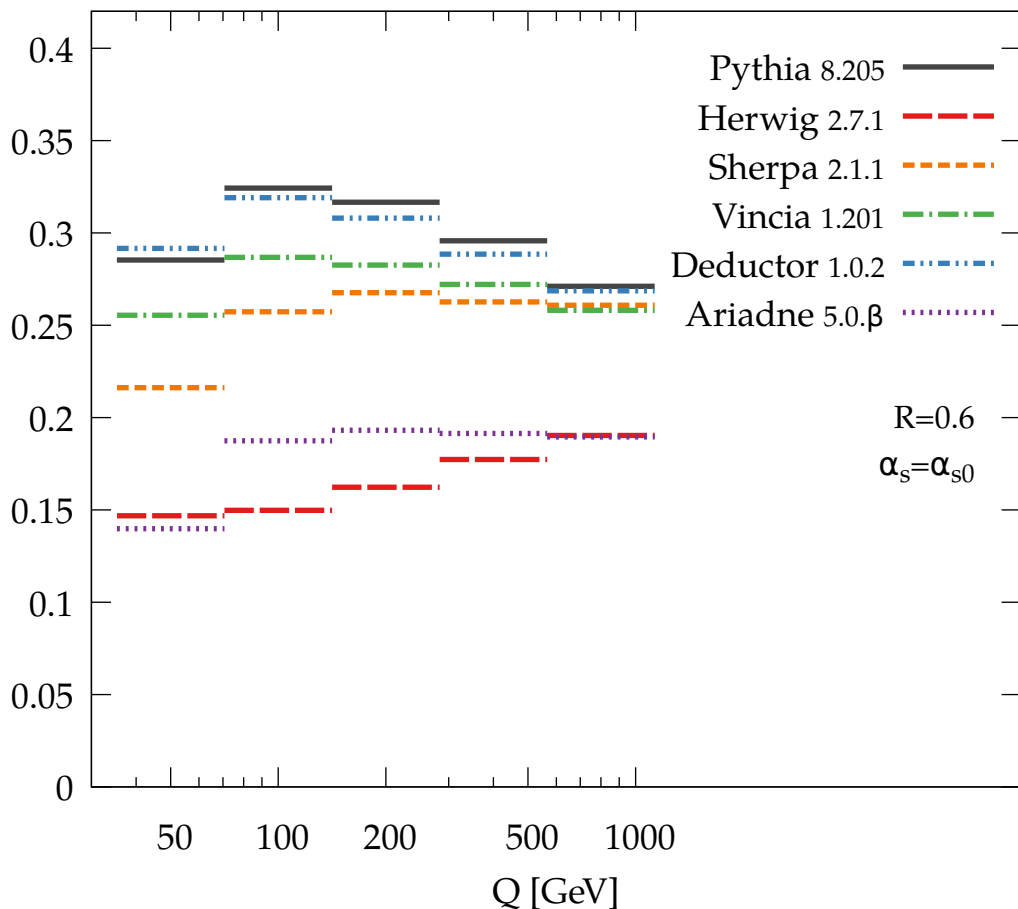

$\lambda_1^1$ , hadron-levelSeparation:  $\Delta$ 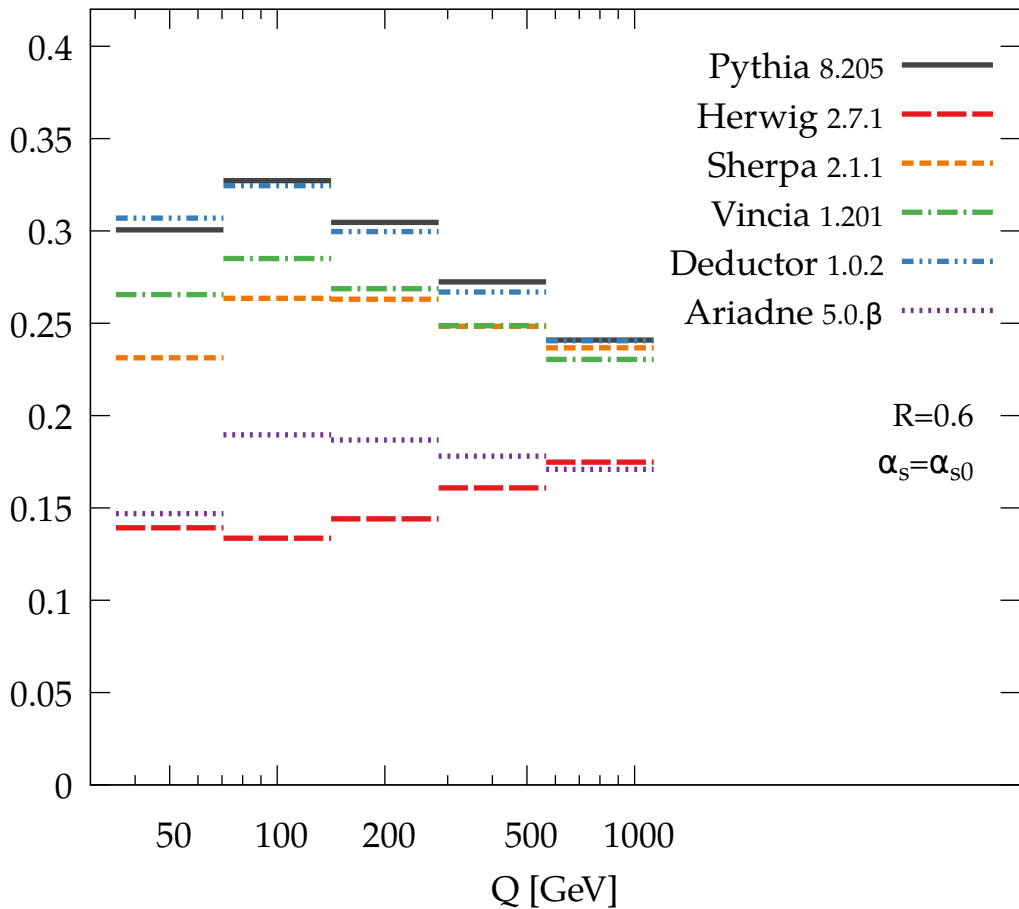

# $\lambda_2^1$ , hadron-level

Separation:  $\Delta$

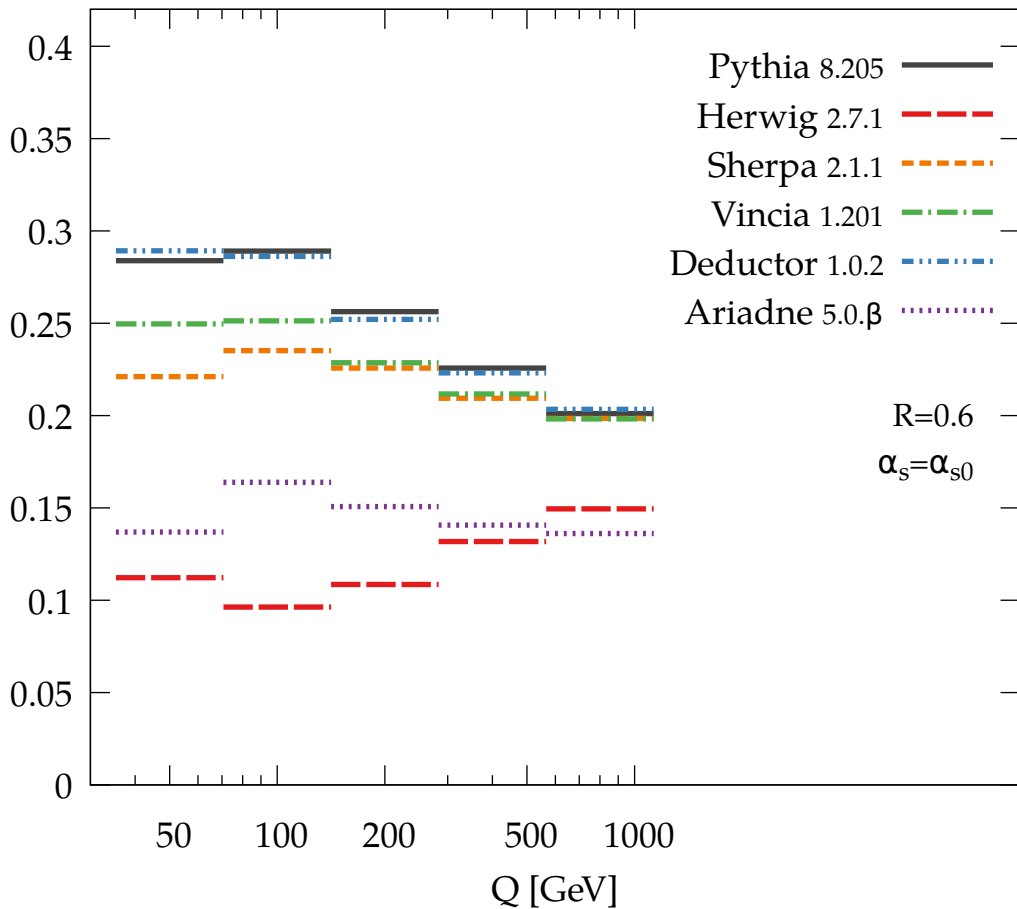

$\lambda_0^0$  [multiplicity], hadron-levelSeparation:  $\Delta$ 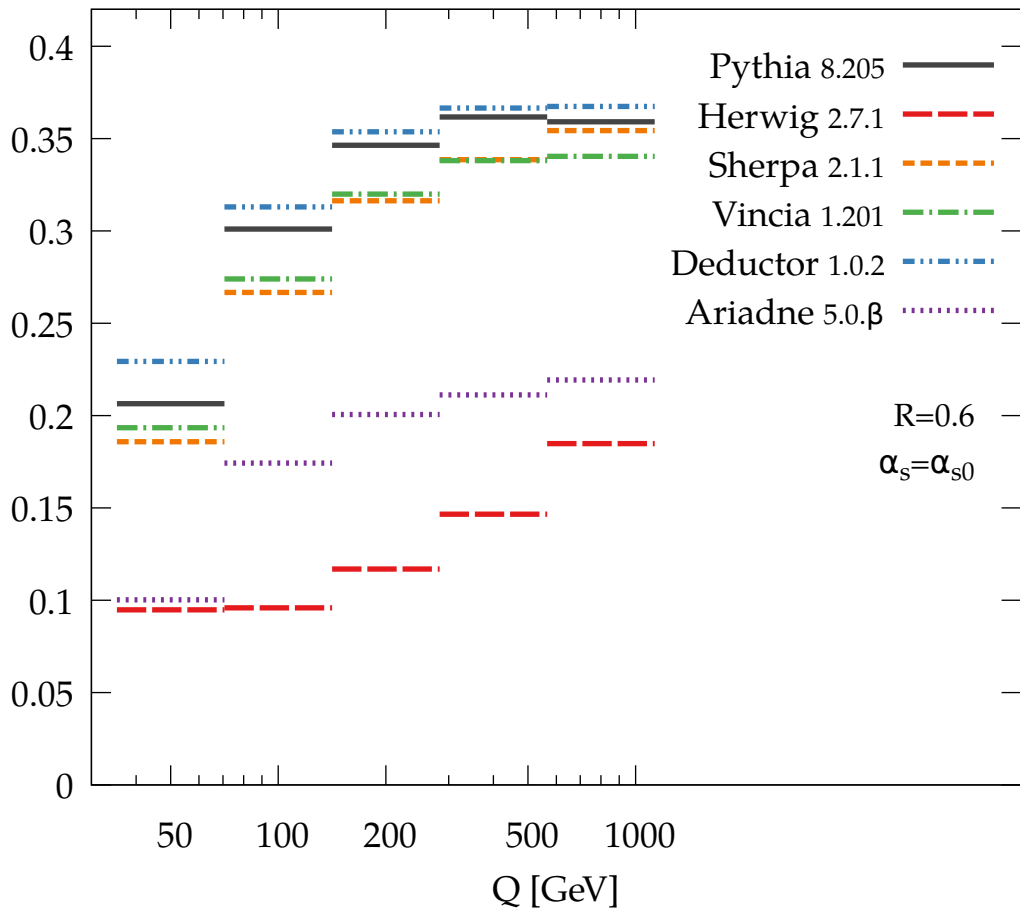

$\lambda_0^2 [(p_T^D)^2], \text{ hadron-level}$ Separation:  $\Delta$ 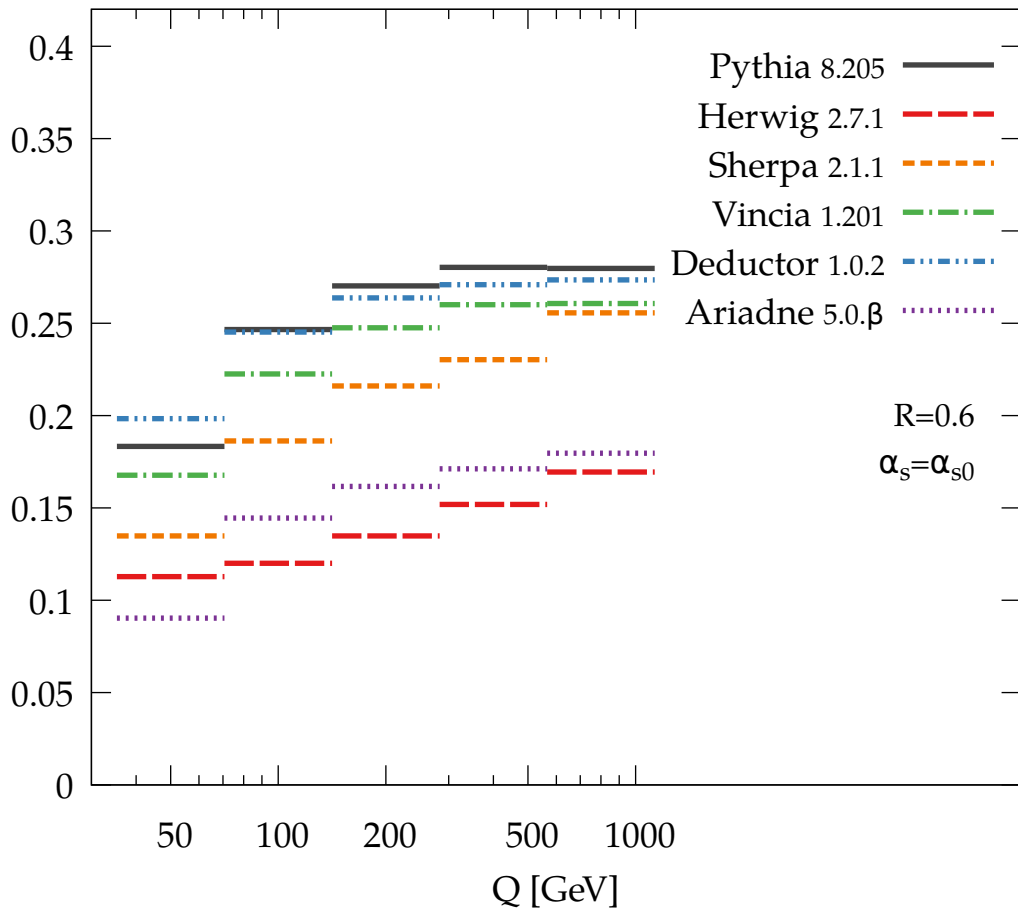

$\lambda_{0.5}^1$  [LHA], hadron-levelSeparation:  $I_{1/2}$ 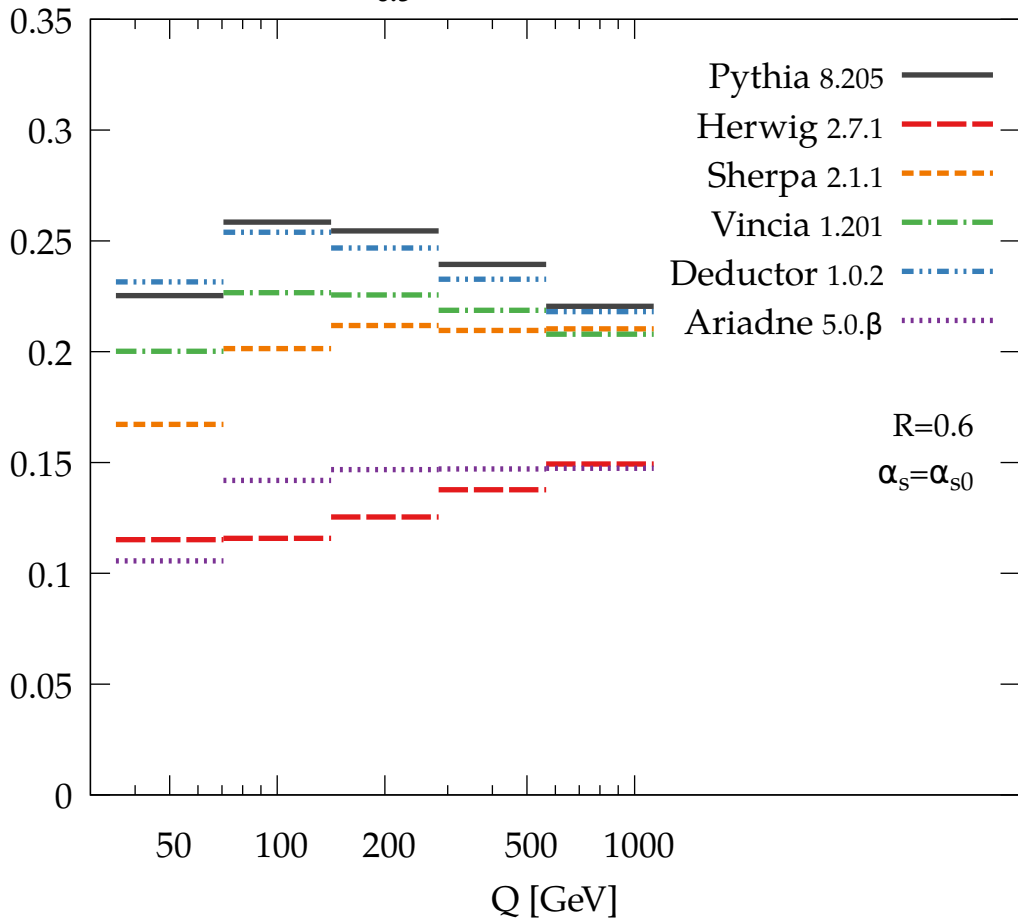

$\lambda_1^1$ , hadron-levelSeparation:  $I_{1/2}$ 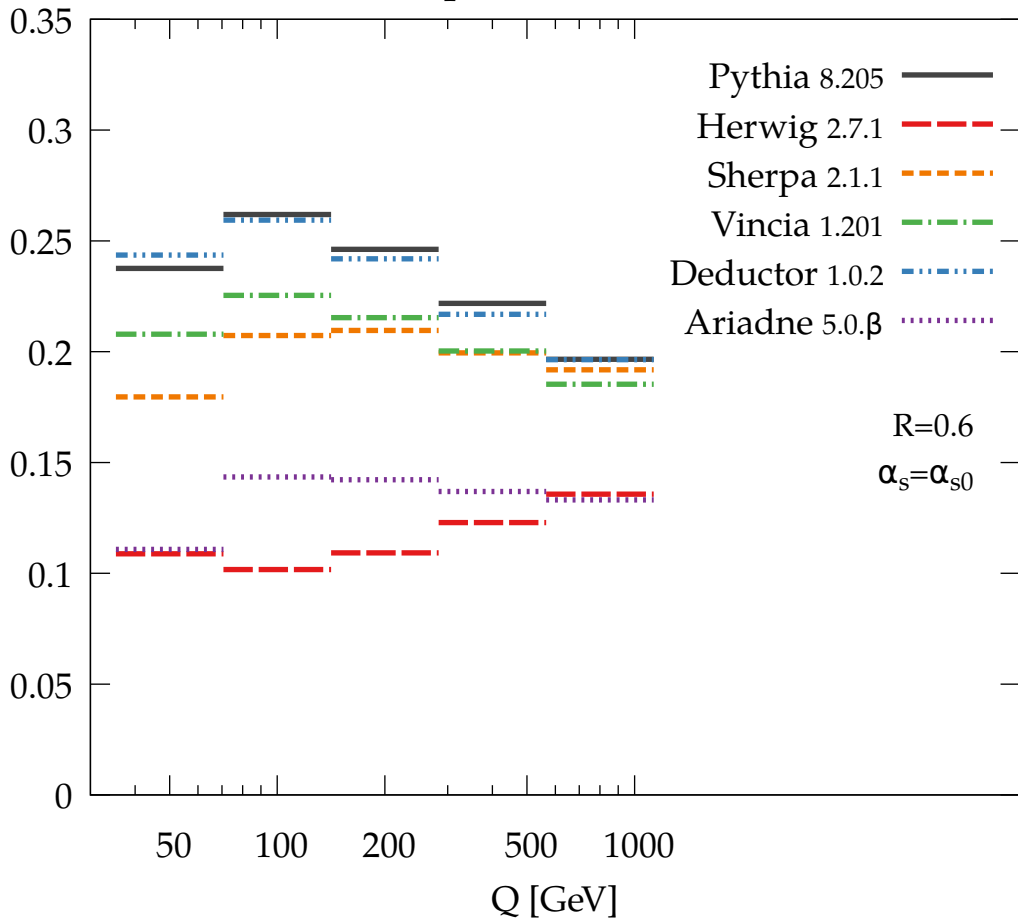

$\lambda_2^1$ , hadron-levelSeparation:  $I_{1/2}$ 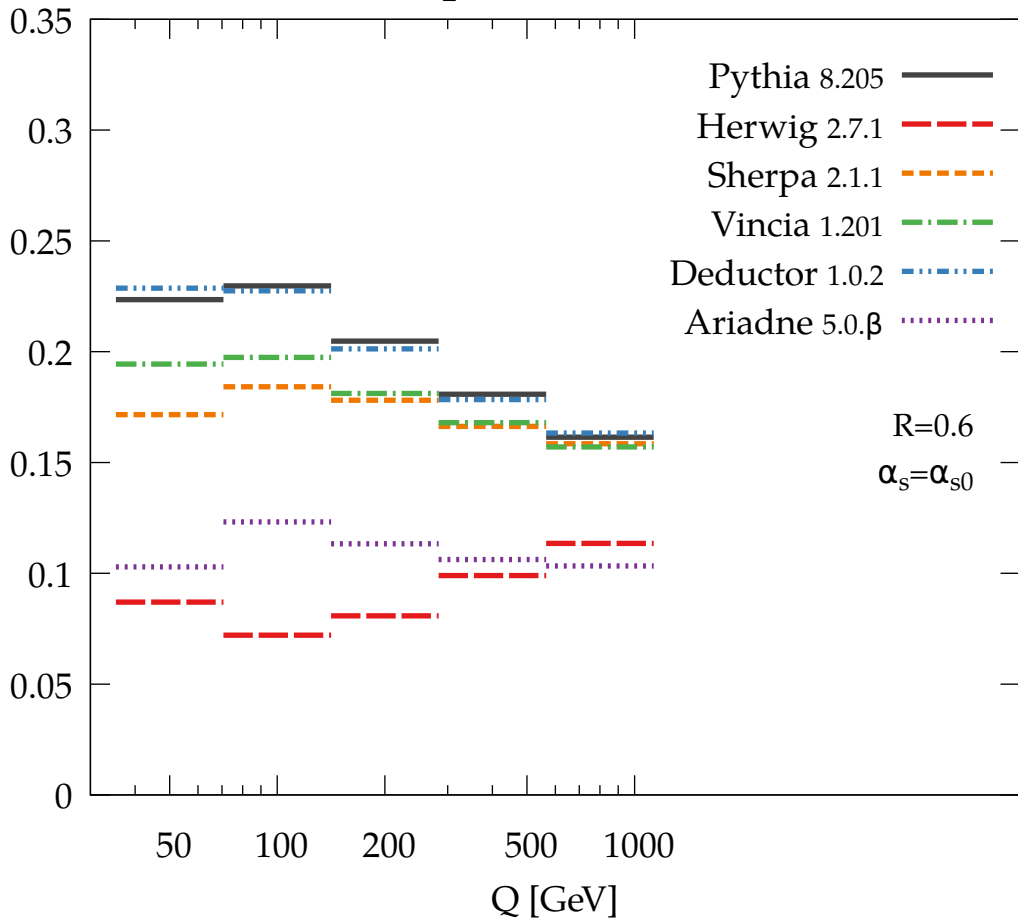



$\lambda_0^0$  [multiplicity], hadron-levelSeparation:  $I_{1/2}$ 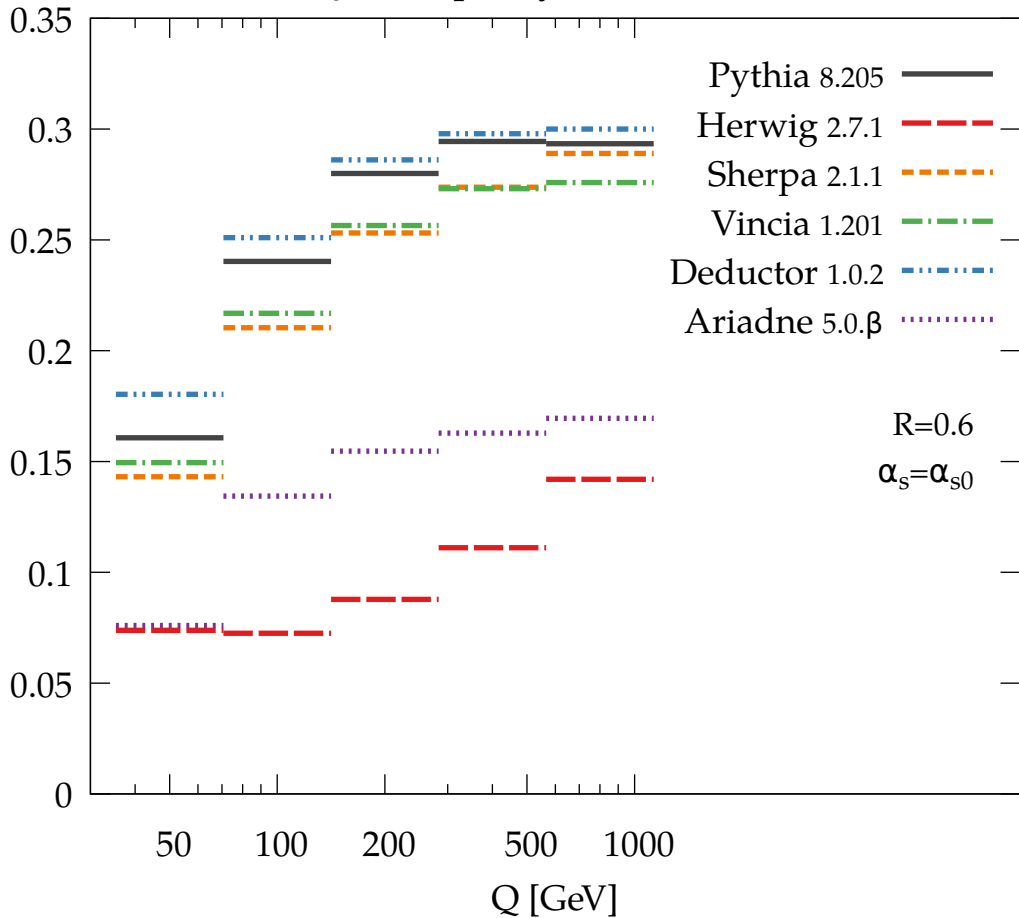

$\lambda_0^2 [(p_T^D)^2]$ , hadron-levelSeparation:  $I_{1/2}$ 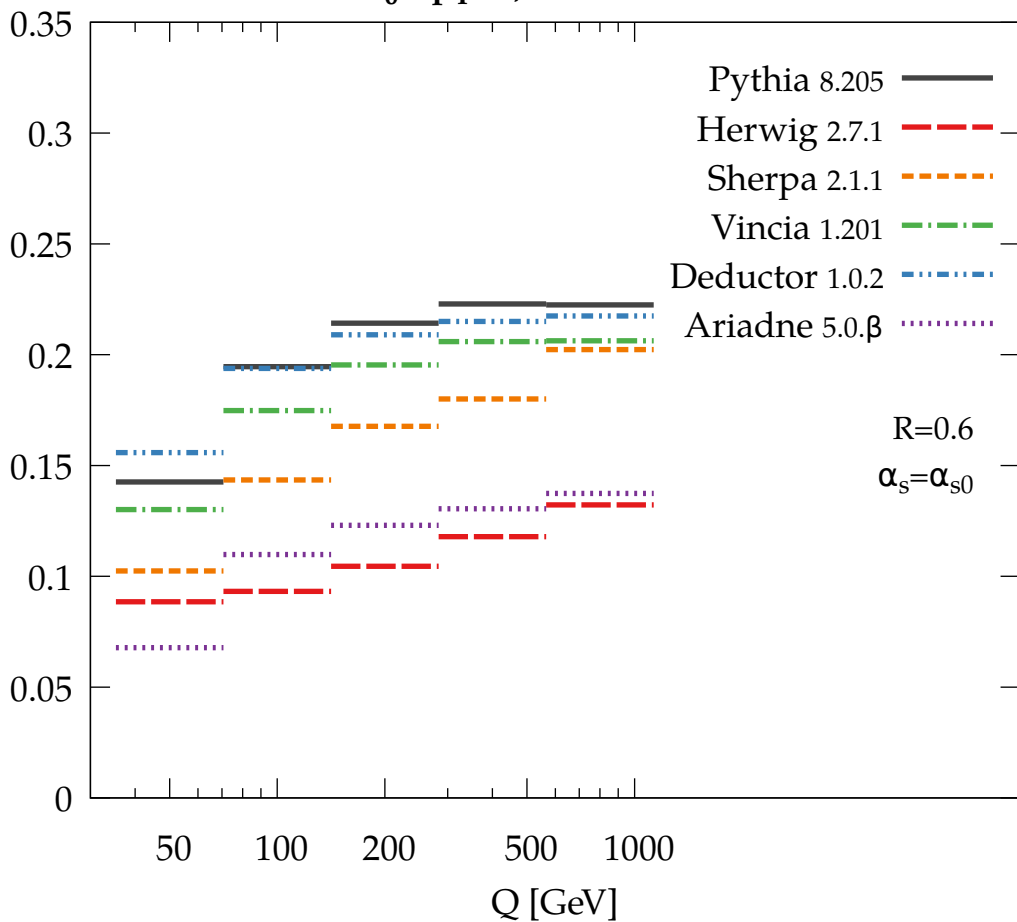

# $\lambda_{0.5}^1$ [LHA], hadron-level

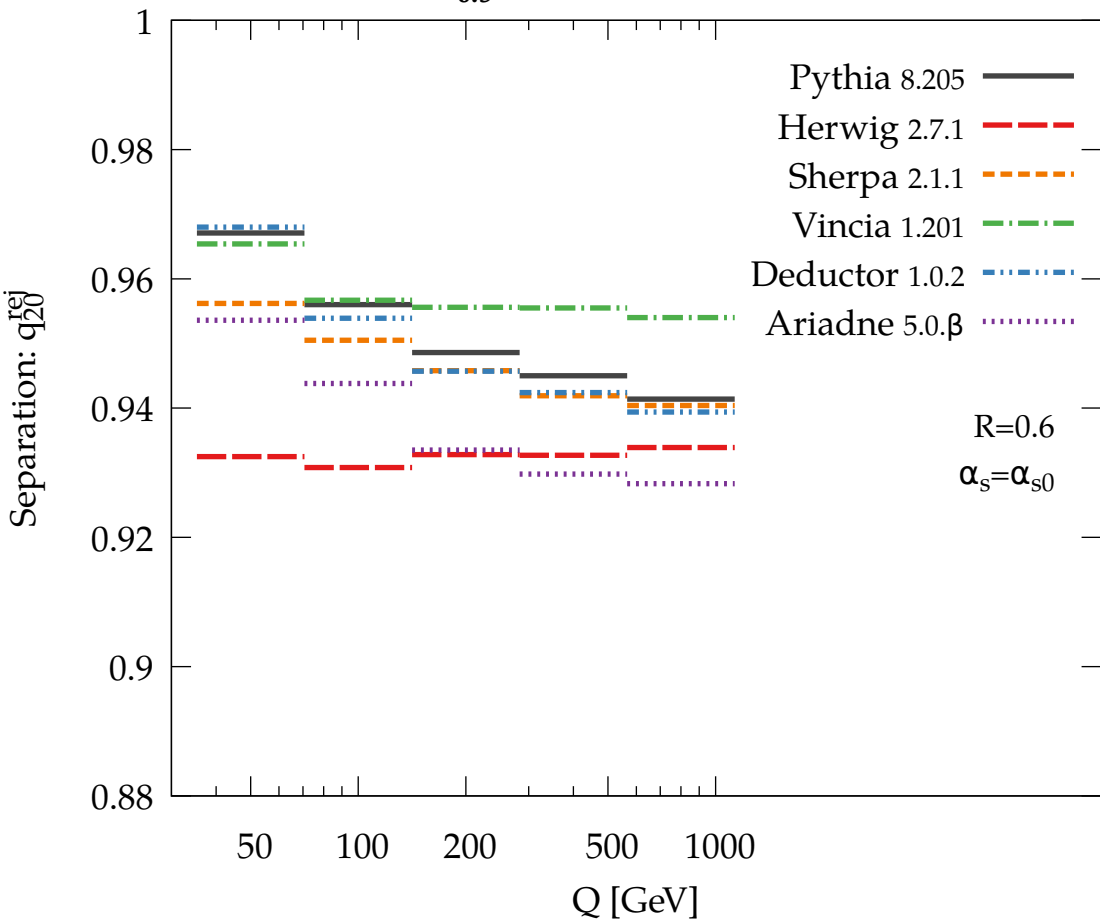

$\lambda_1^1$ , hadron-level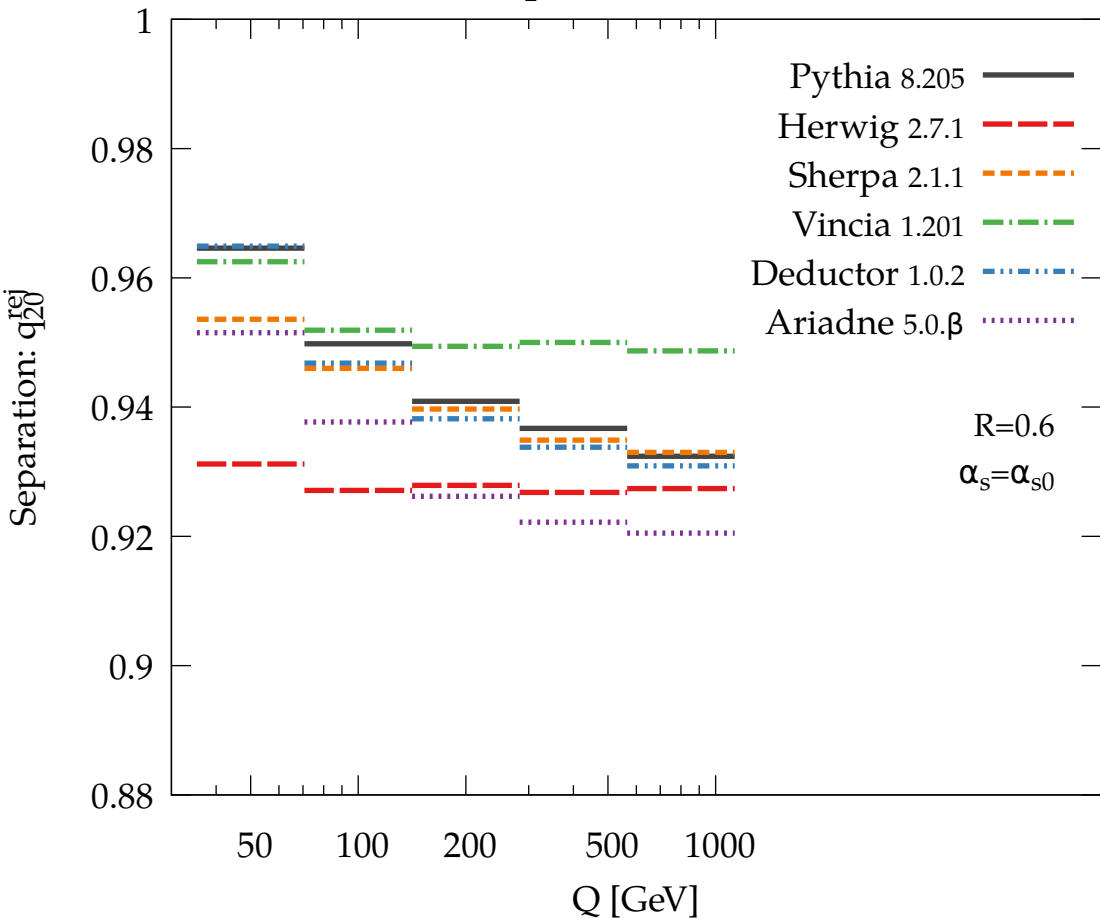

$\lambda_2^1$ , hadron-level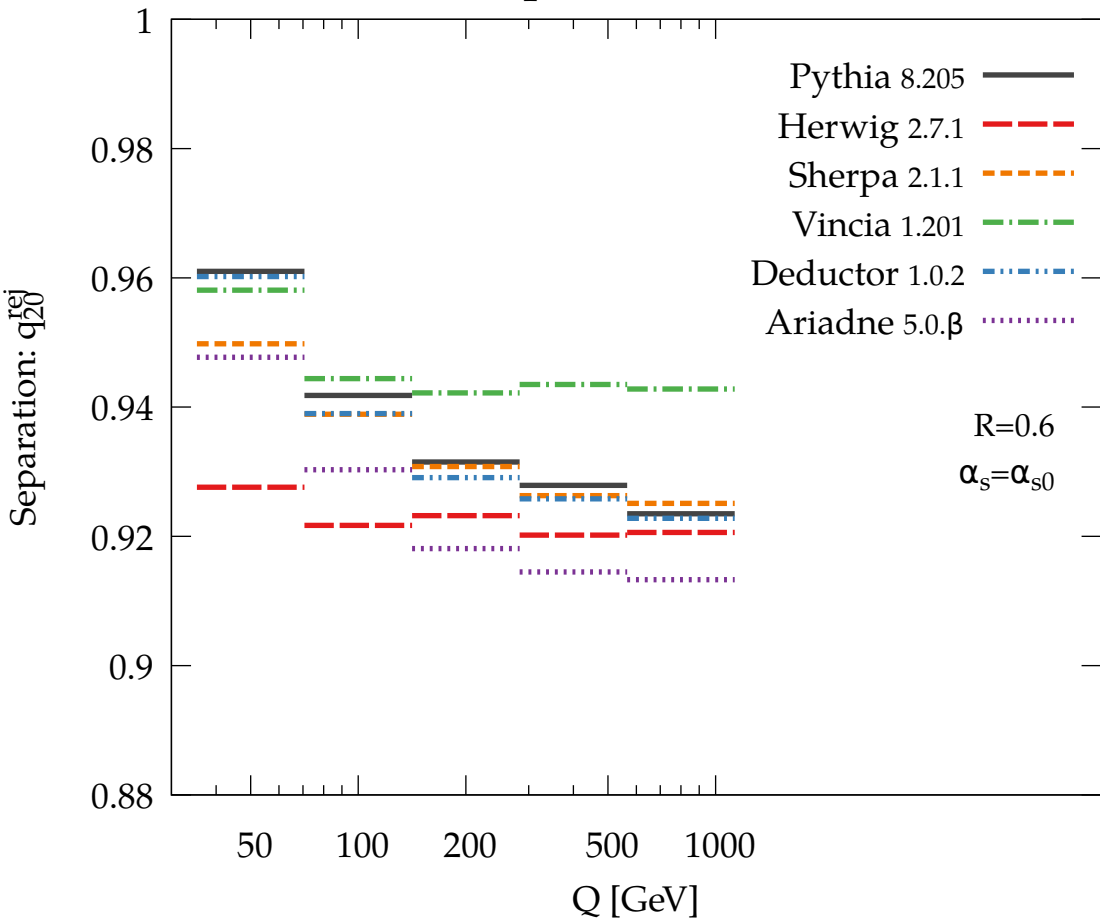

# $\lambda_0^0$ [multiplicity], hadron-level

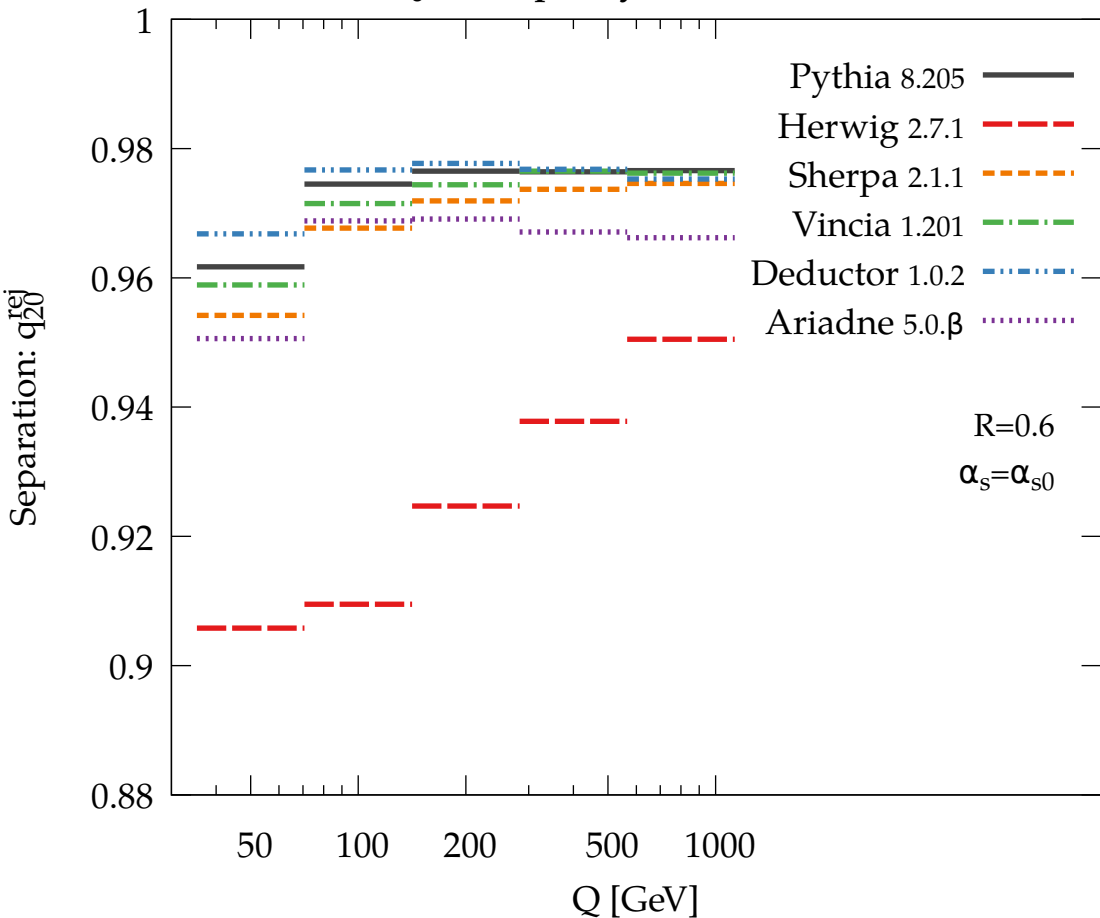

$\lambda_0^2 [(p_T^D)^2]$ , hadron-level

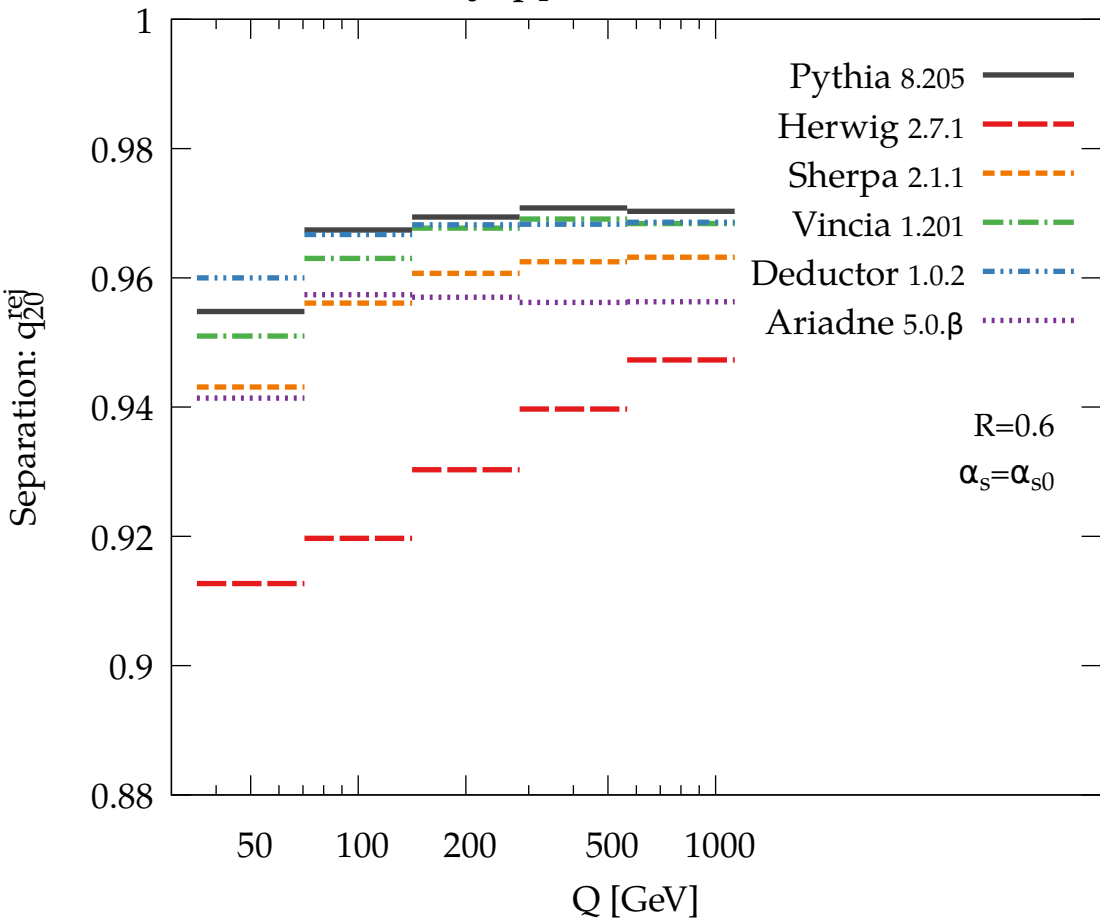

$\lambda_{0.5}^1$  [LHA], hadron-level

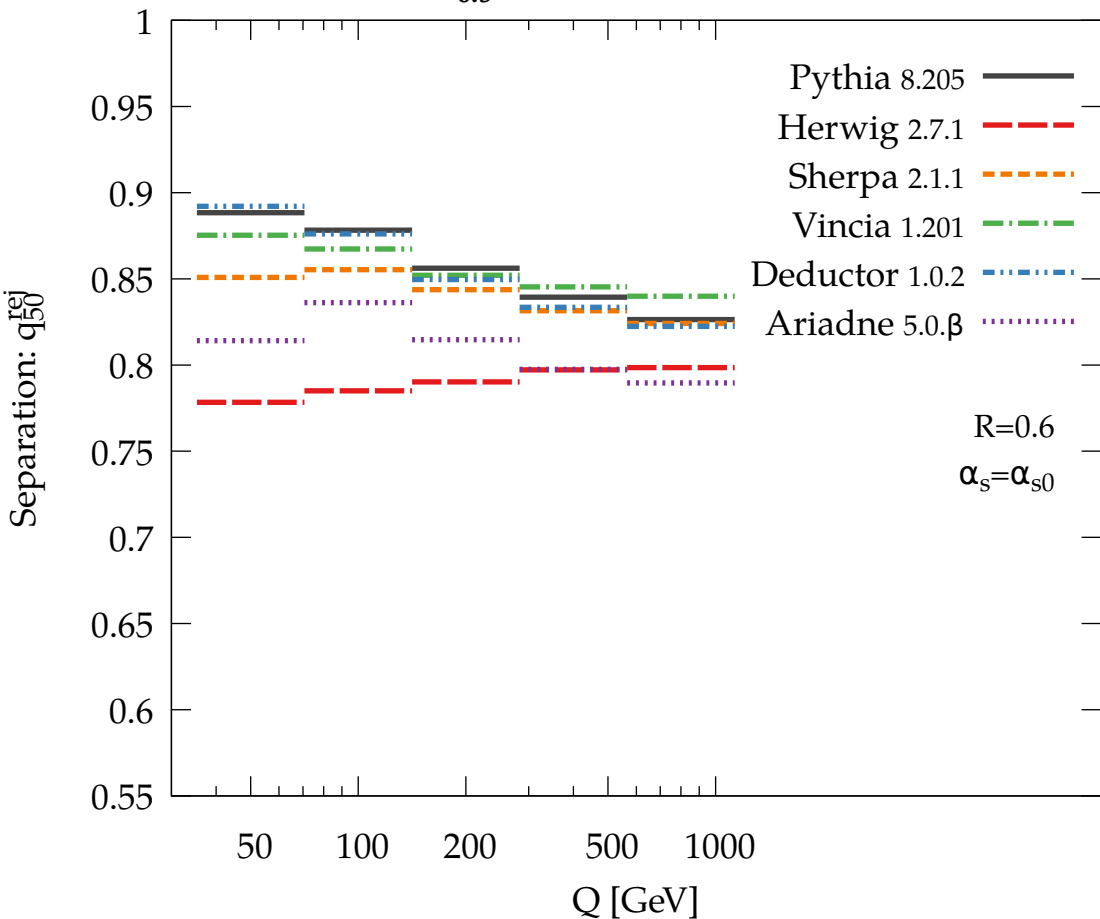



$\lambda_1^1$ , hadron-level

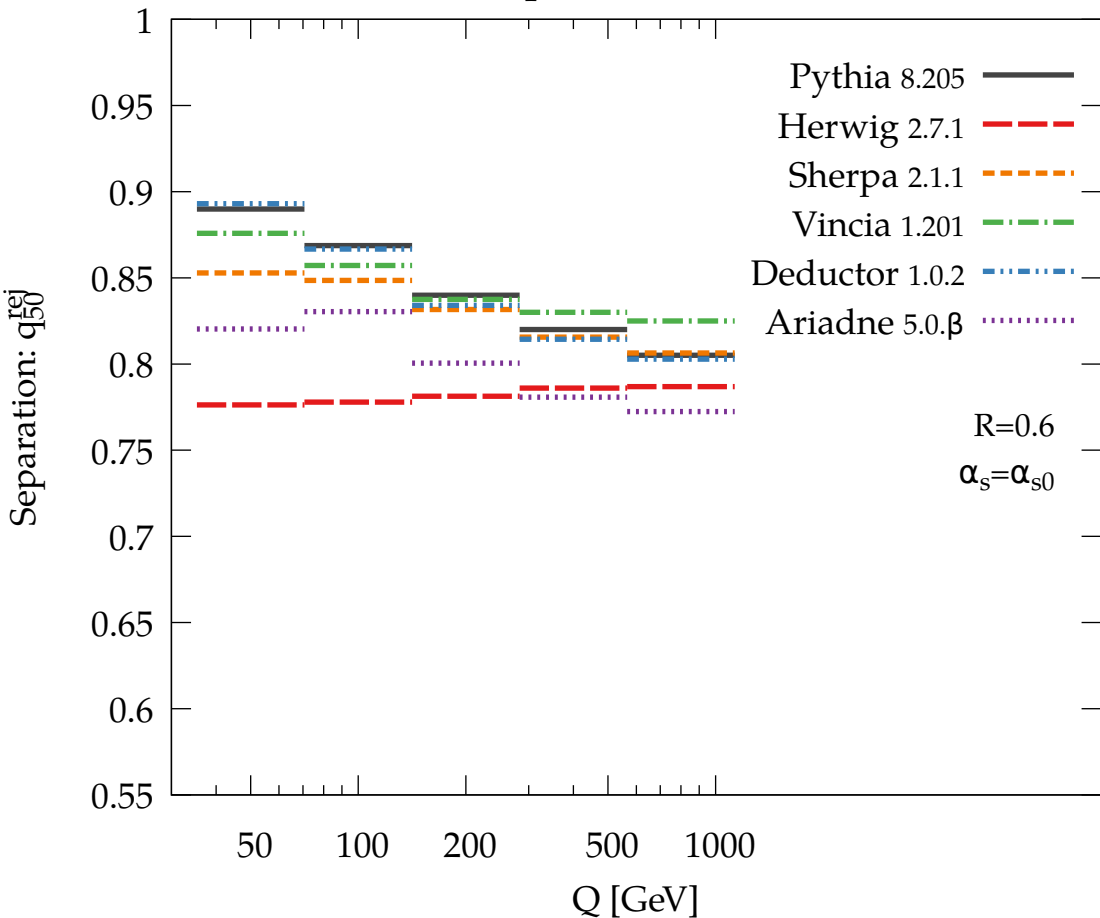

$\lambda_2^1$ , hadron-level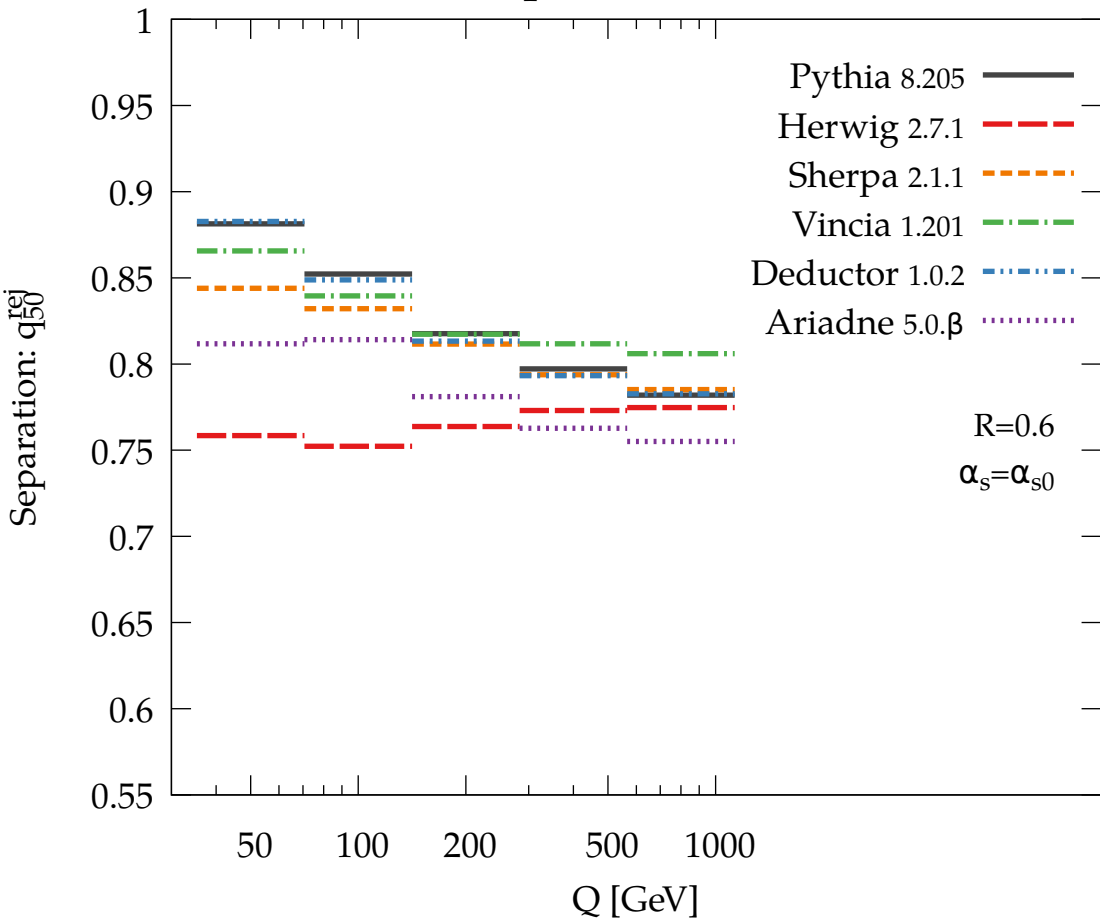

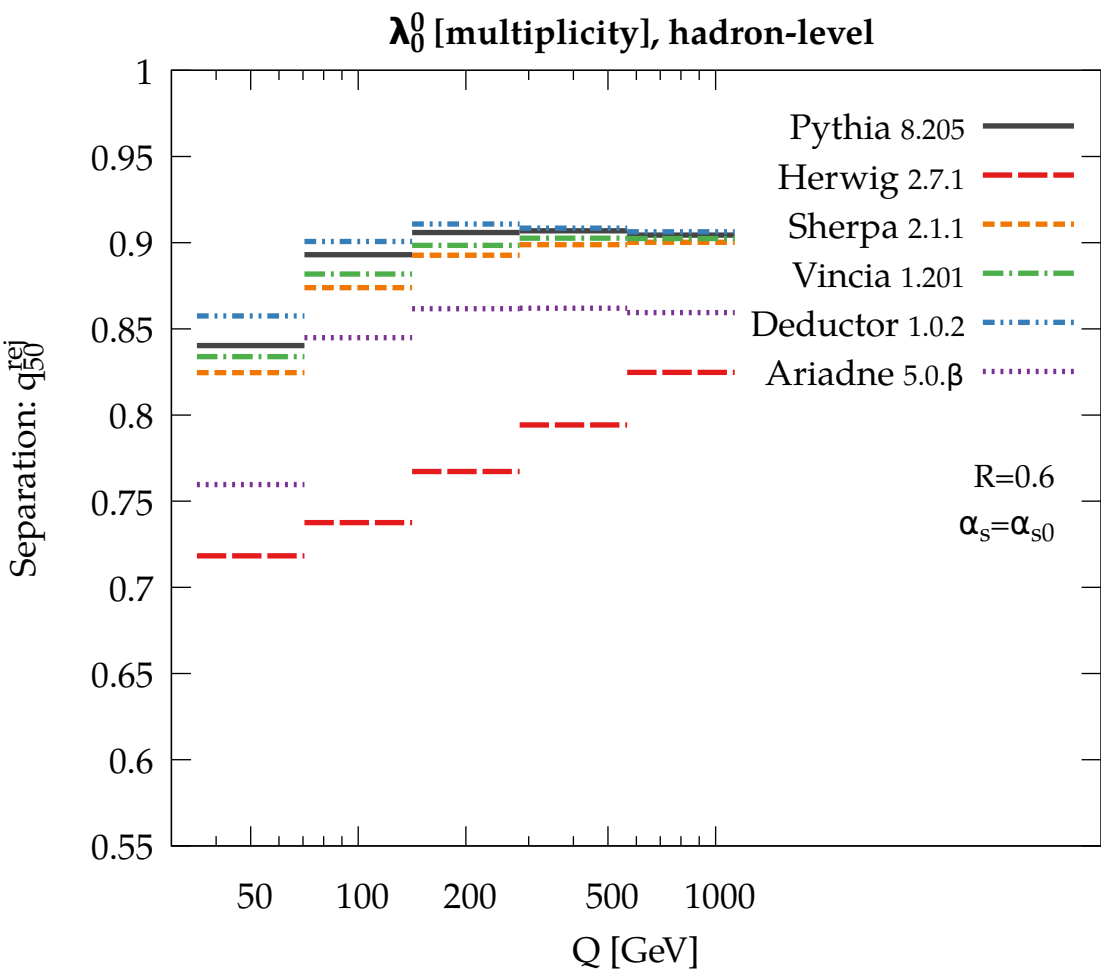

$\lambda_0^2 [(p_T^D)^2], \text{ hadron-level}$ 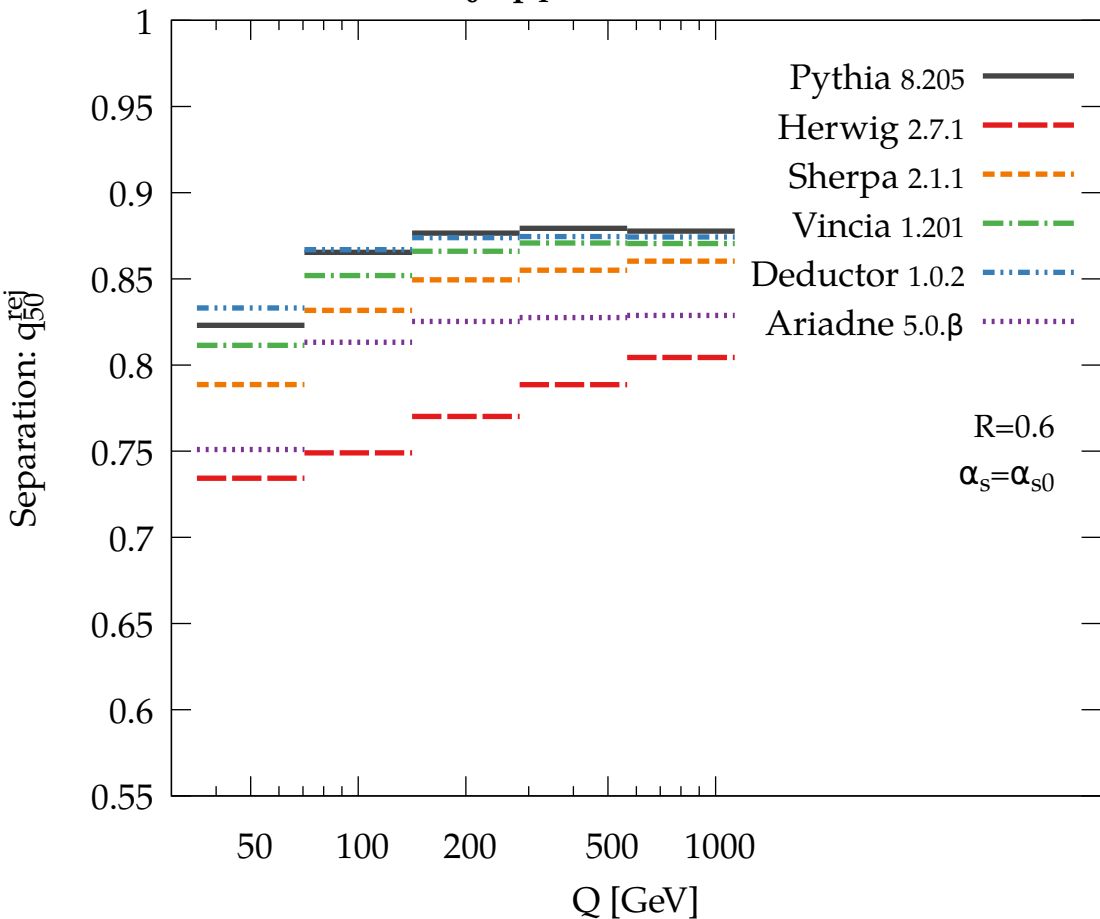

$\lambda_{0.5}^1$  [LHA], hadron-level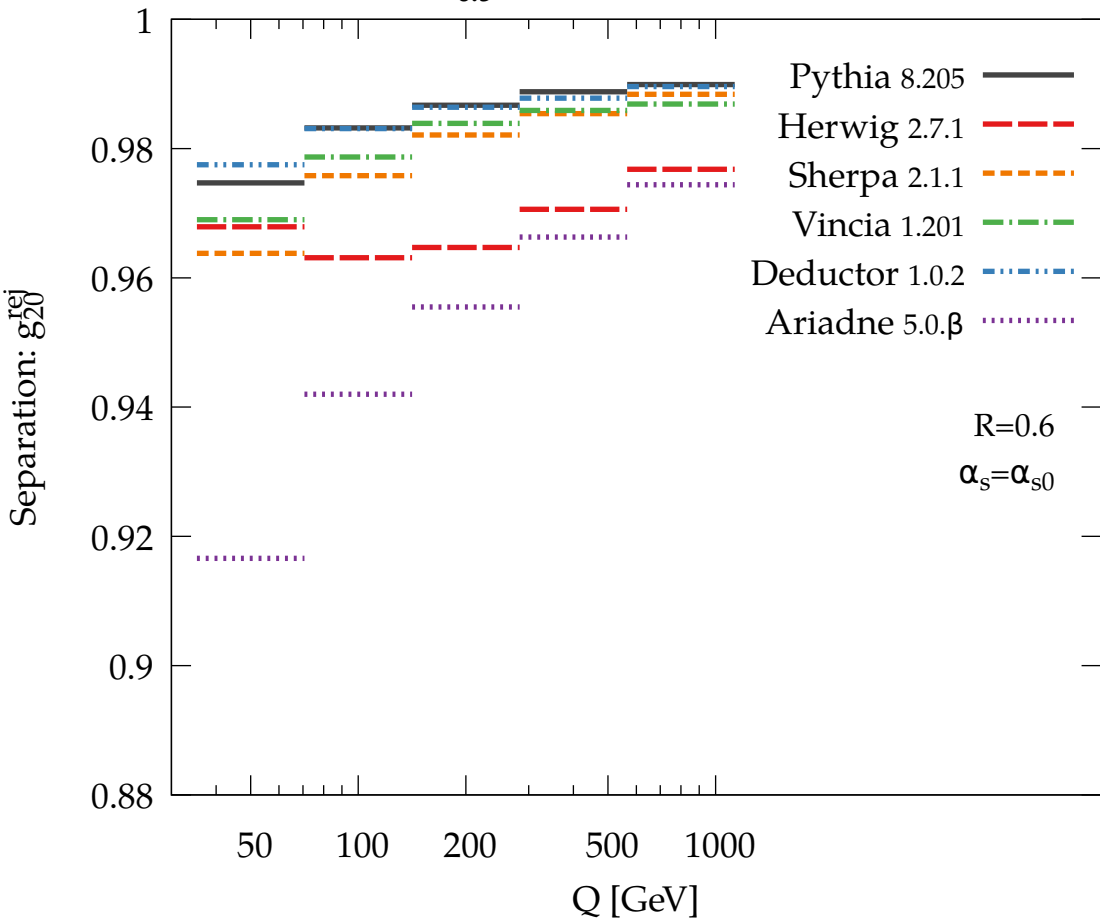

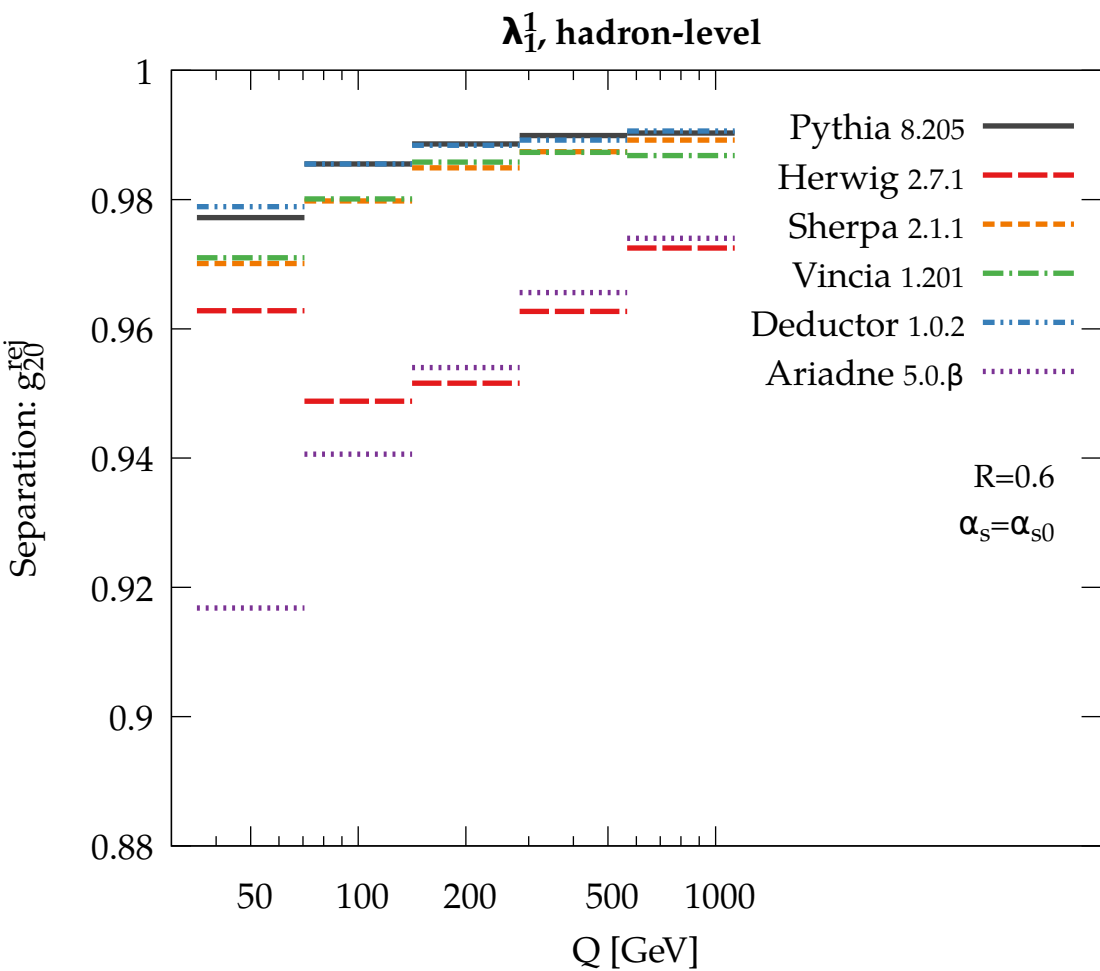

$\lambda_2^1$ , hadron-level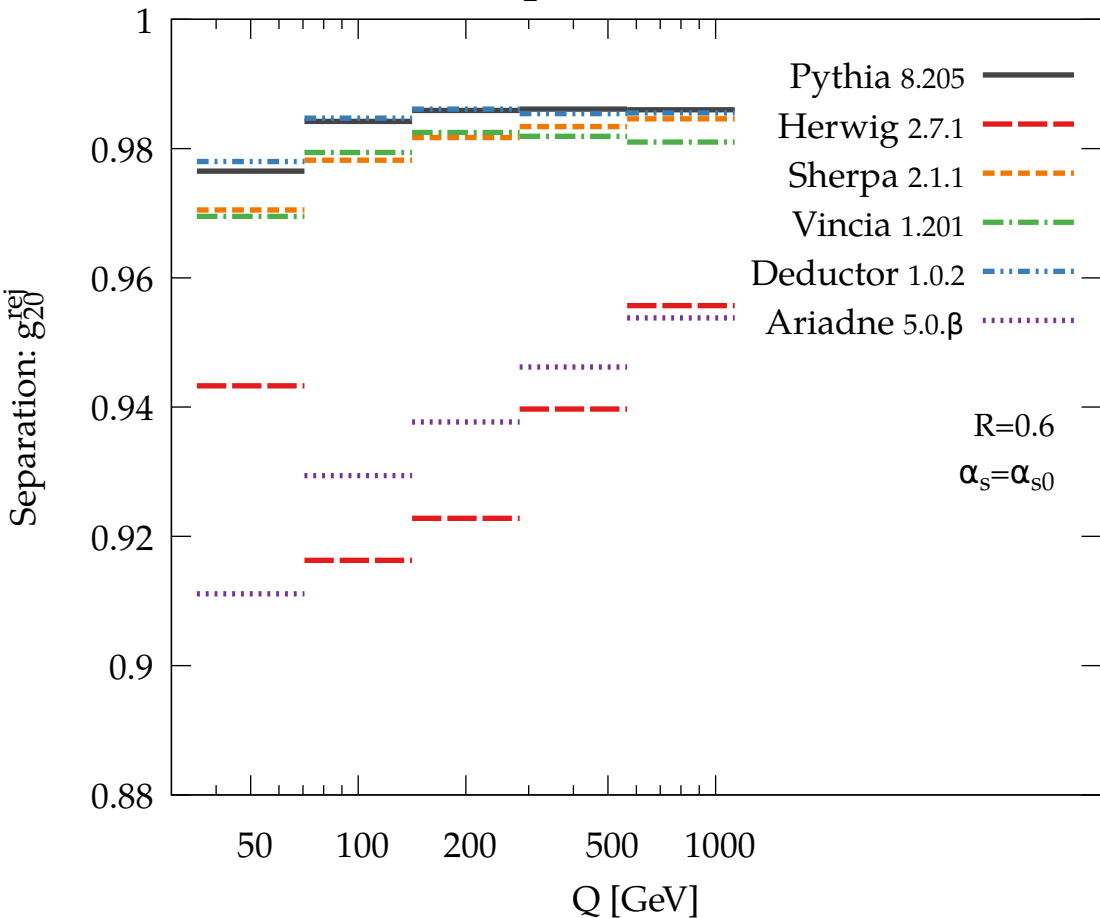

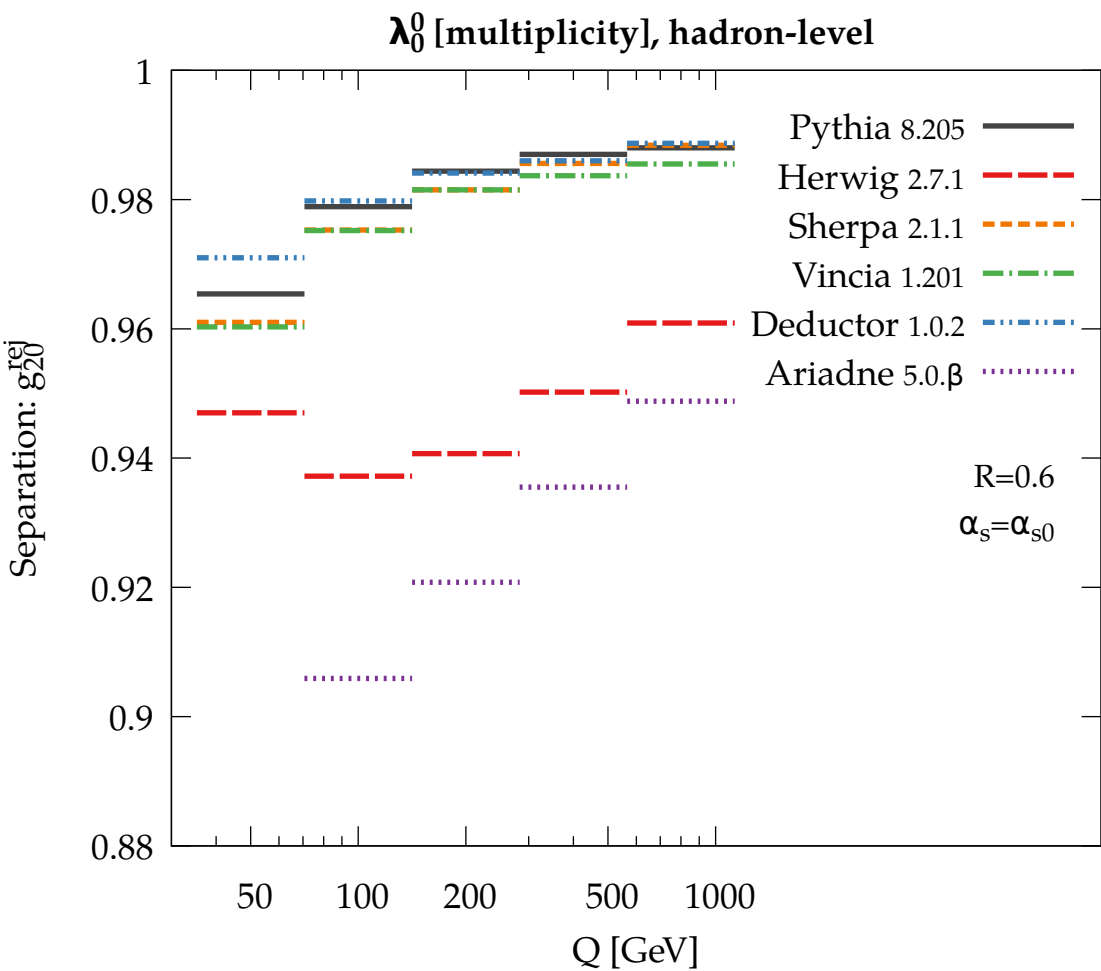



$\lambda_0^2 [(p_T^D)^2]$ , hadron-level

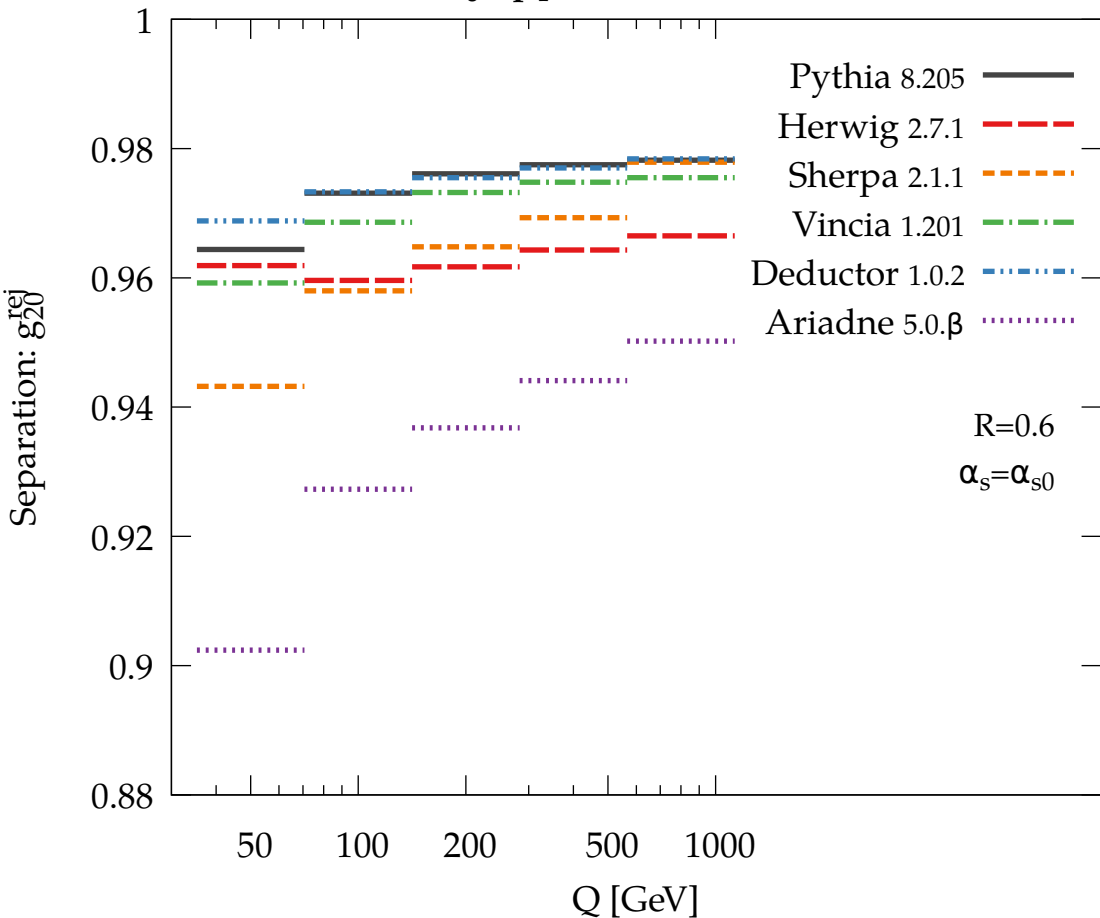

$\lambda_{0.5}^1$  [LHA], hadron-level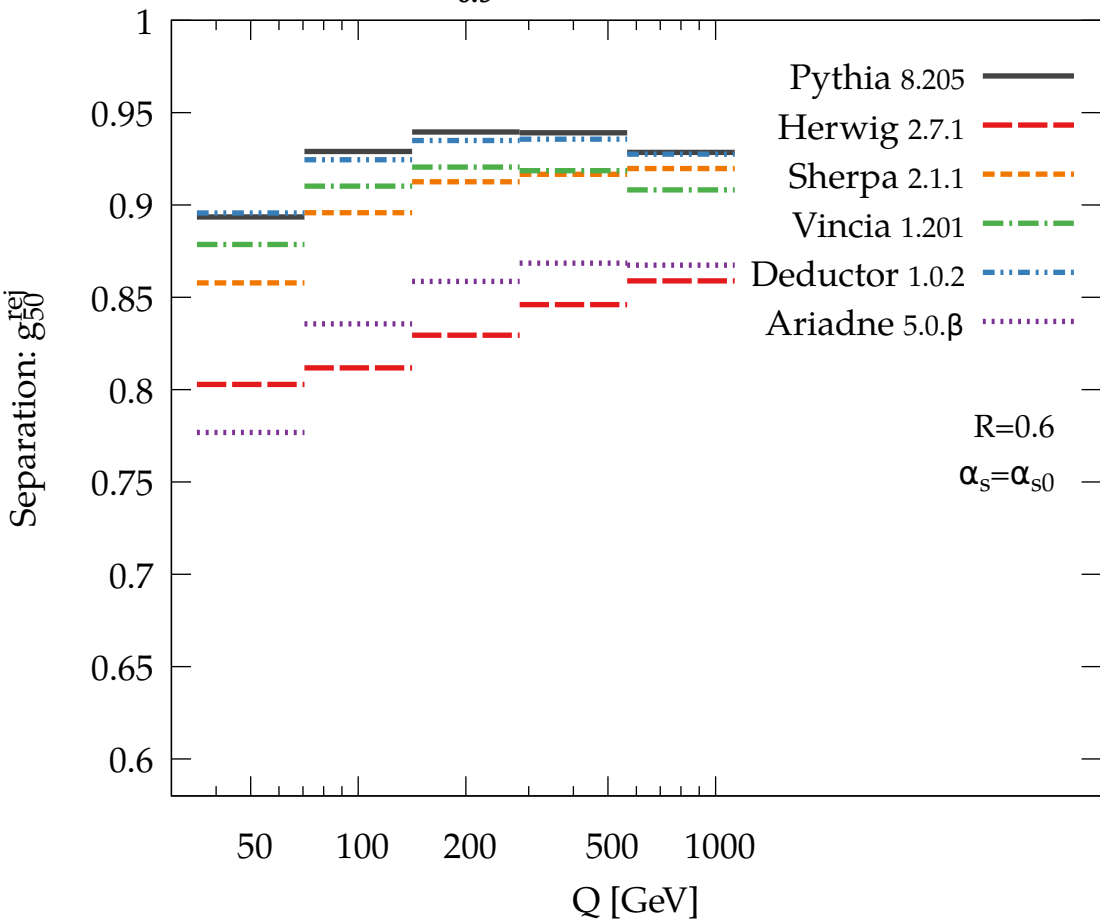

$\lambda_1^1$ , hadron-level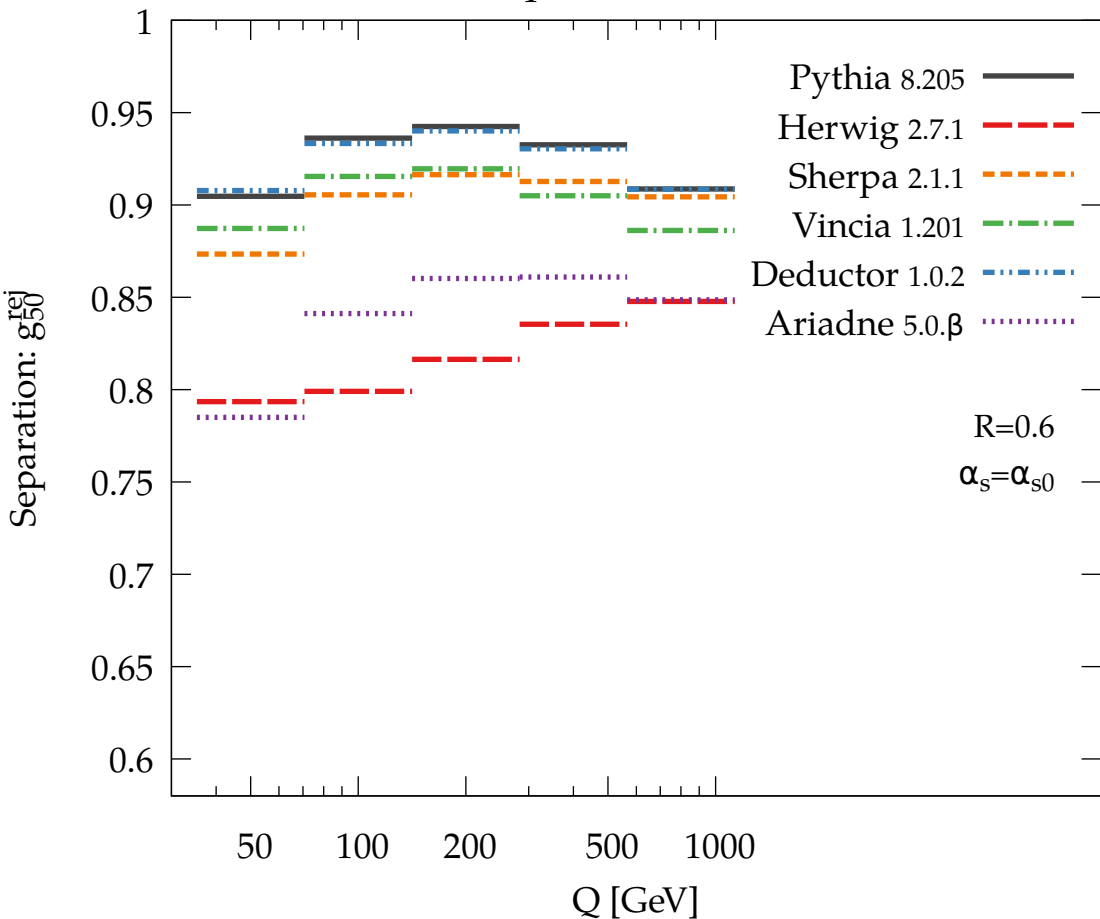

$\lambda_2^1$ , hadron-level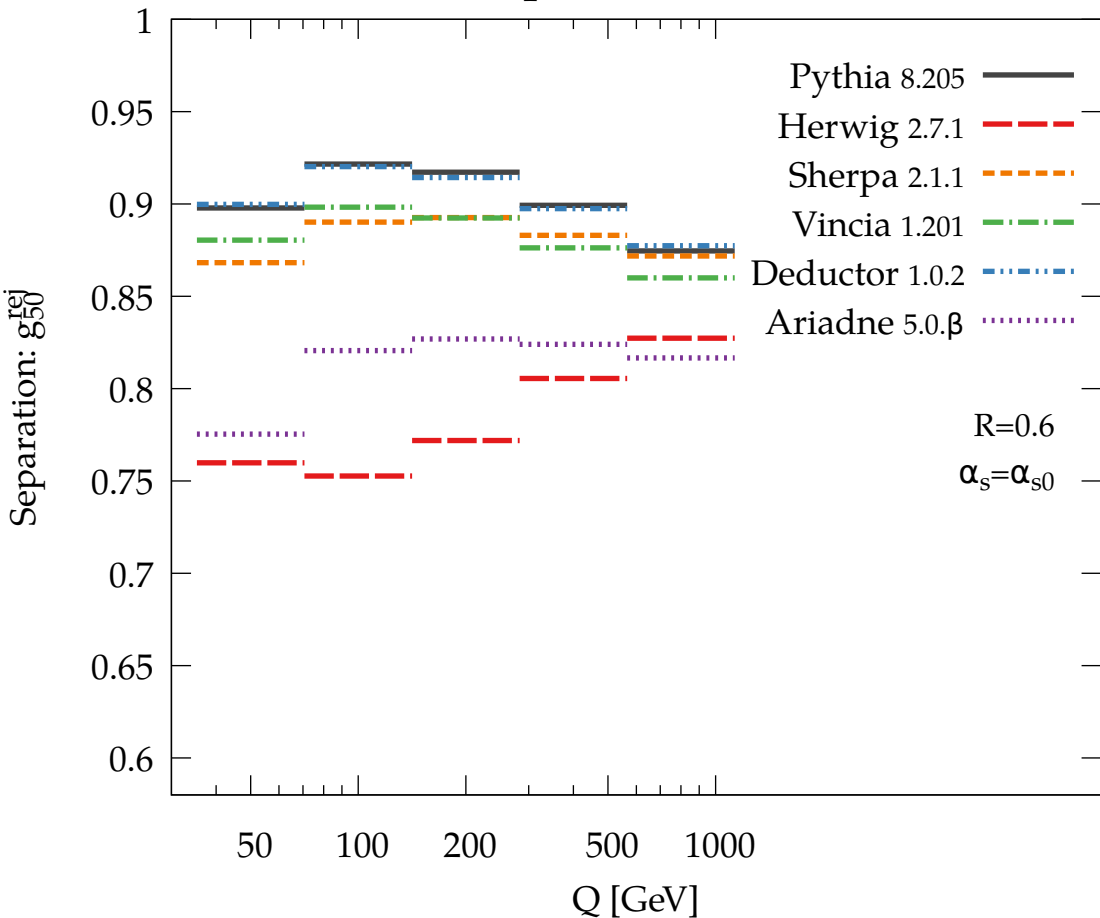

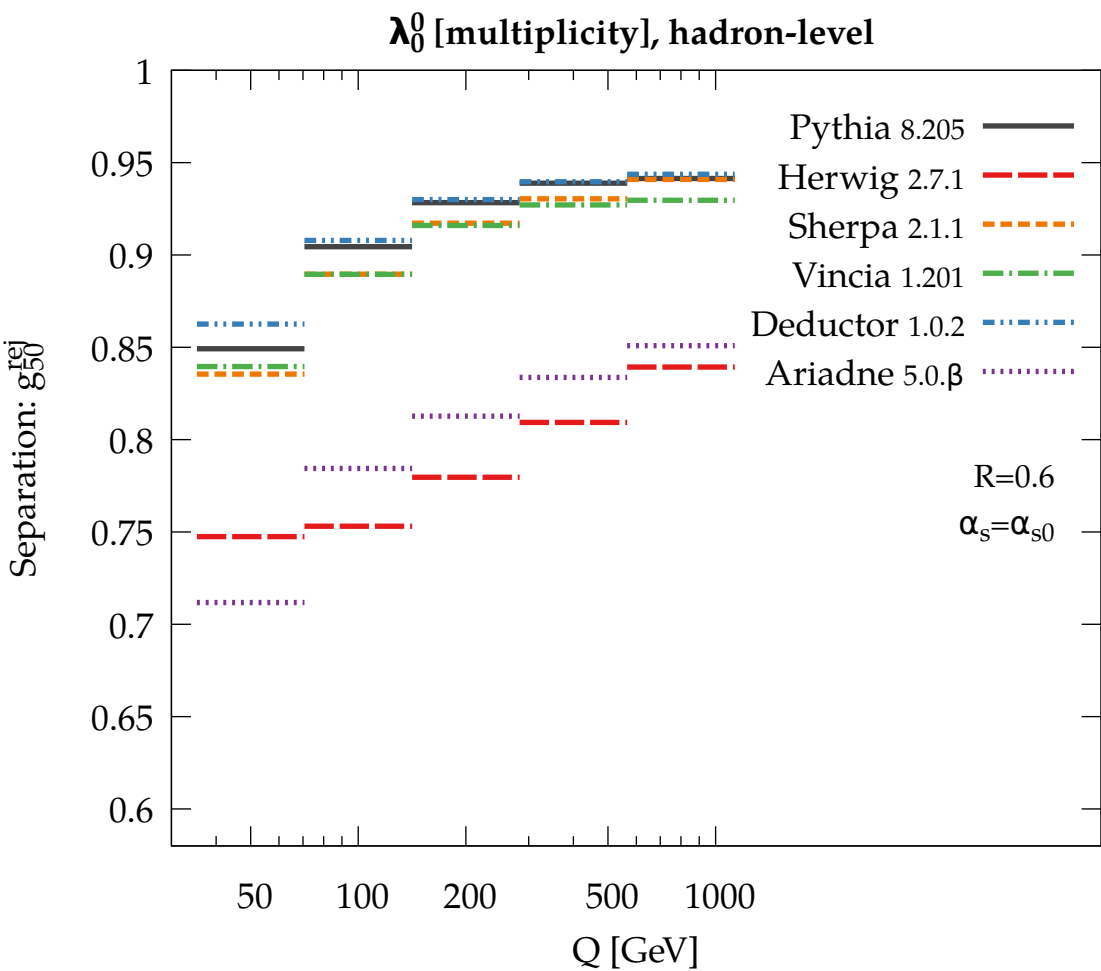

$\lambda_0^2 [(p_T^D)^2]$ , hadron-level

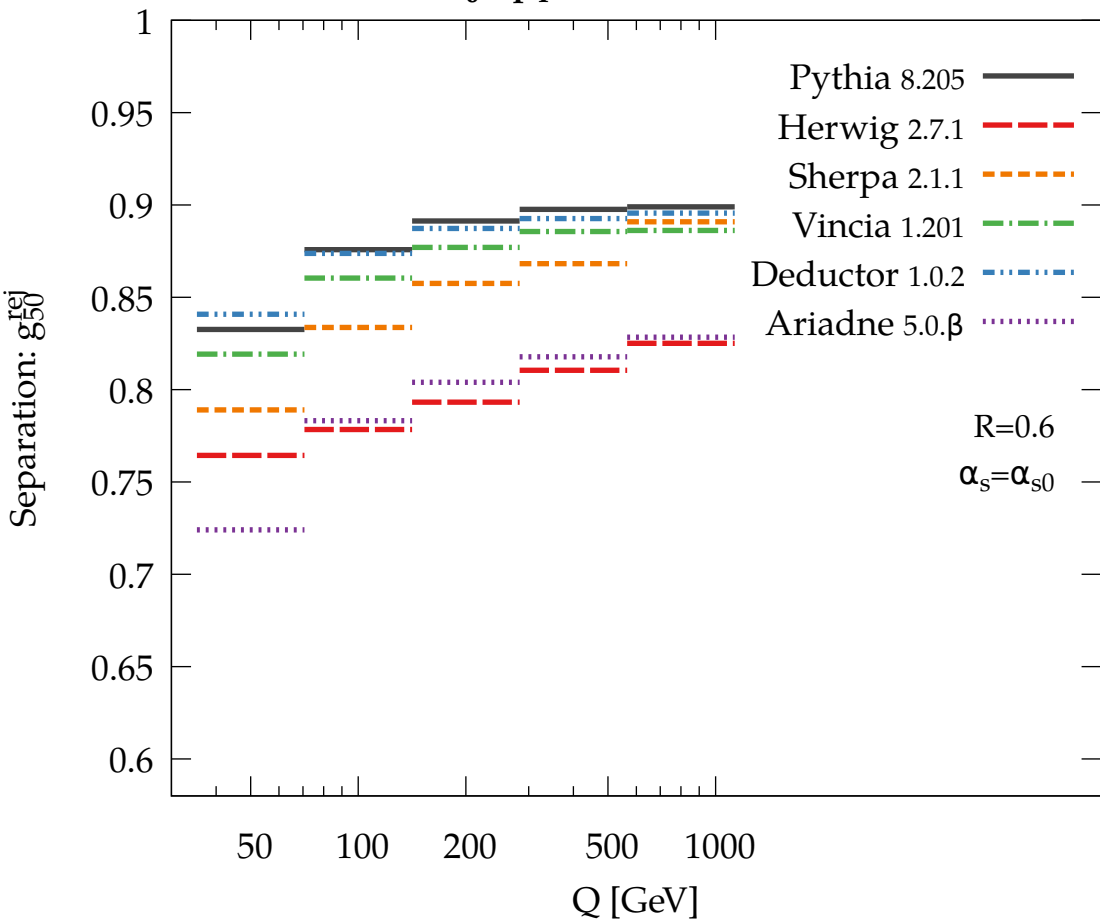

$\lambda_{0.5}^1$  [LHA], hadron-levelSeparation:  $s^{\text{rej}}$ 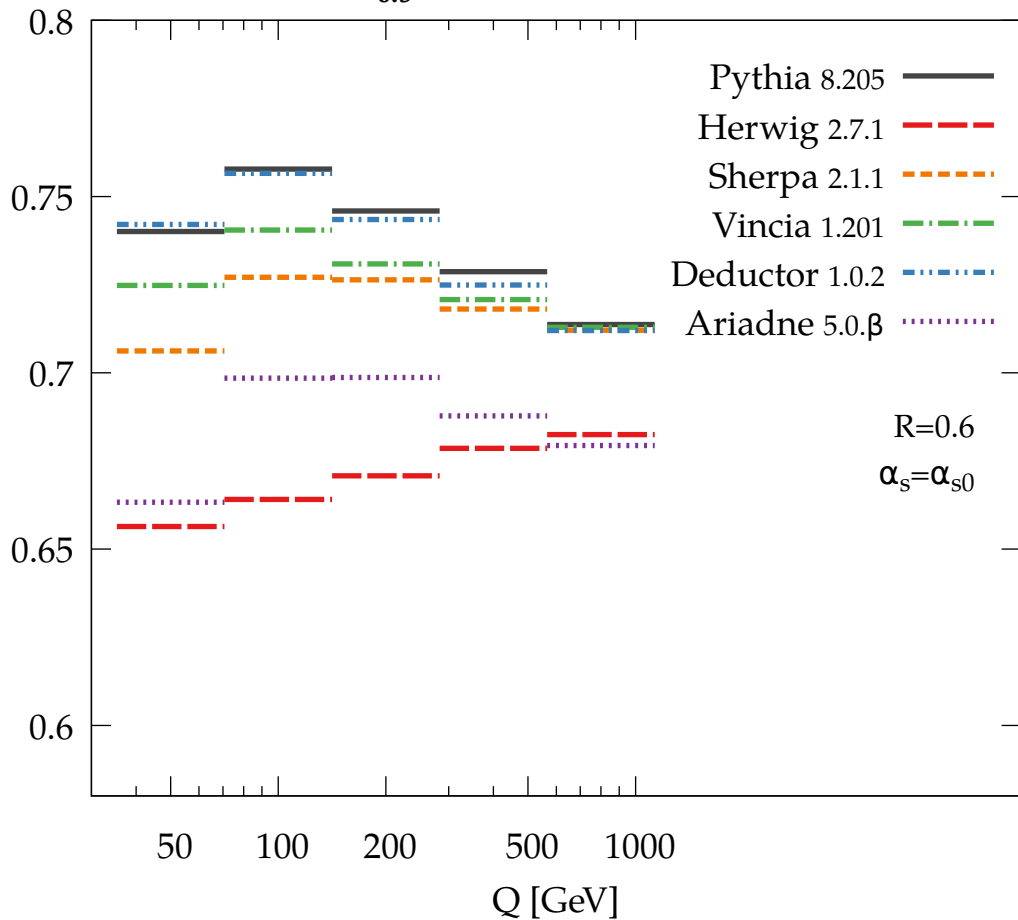

$\lambda_1^1$ , hadron-levelSeparation:  $s^{\text{rej}}$ 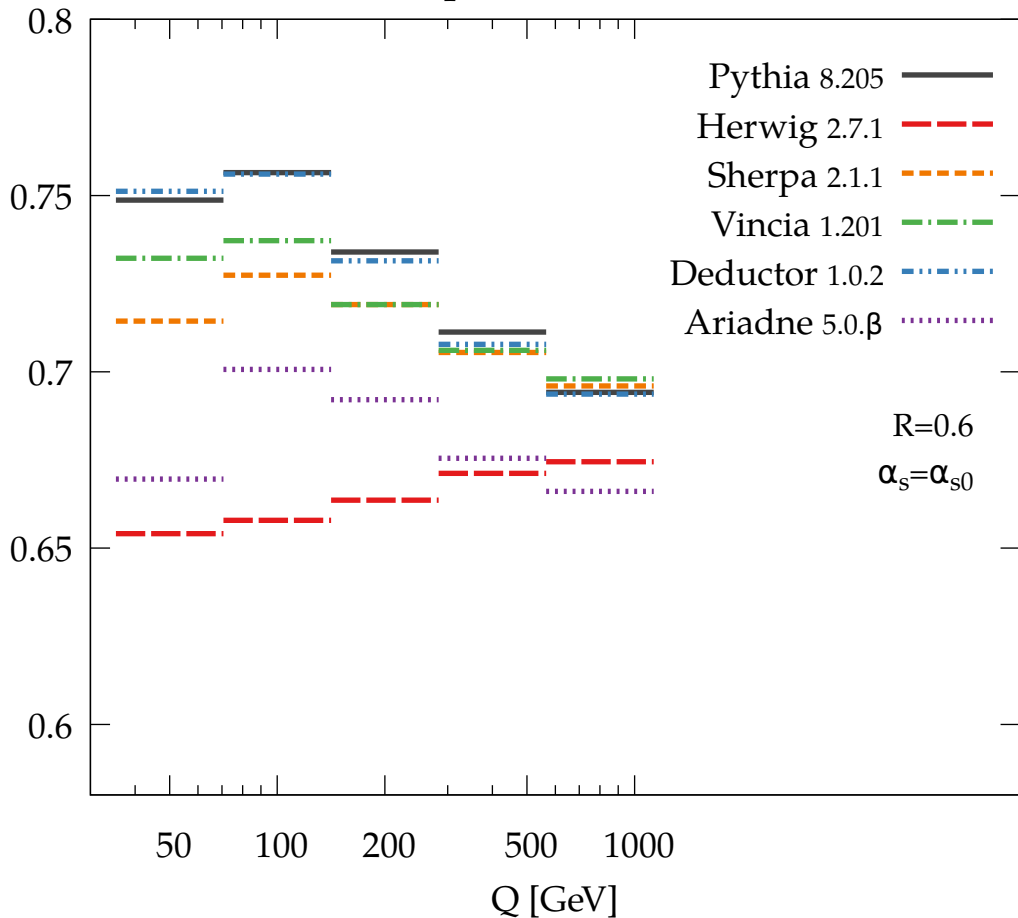



$\lambda_2^1$ , hadron-levelSeparation:  $s^{\text{rej}}$ 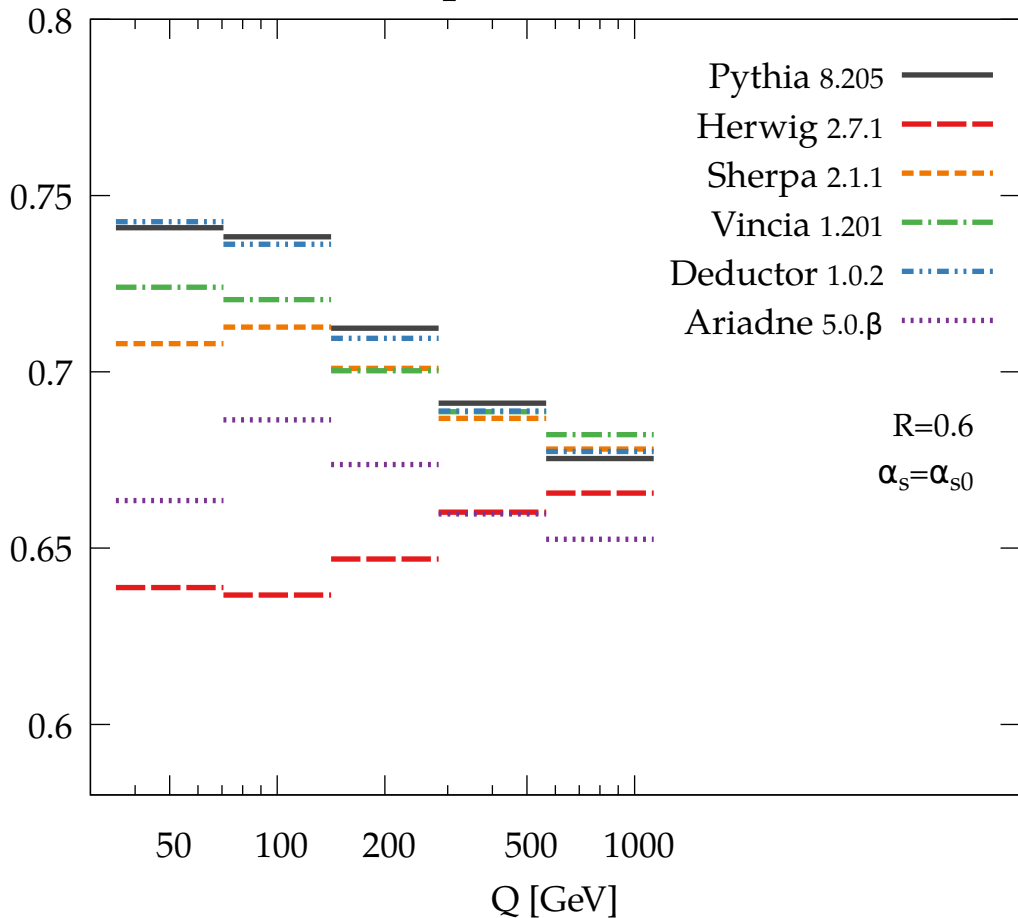

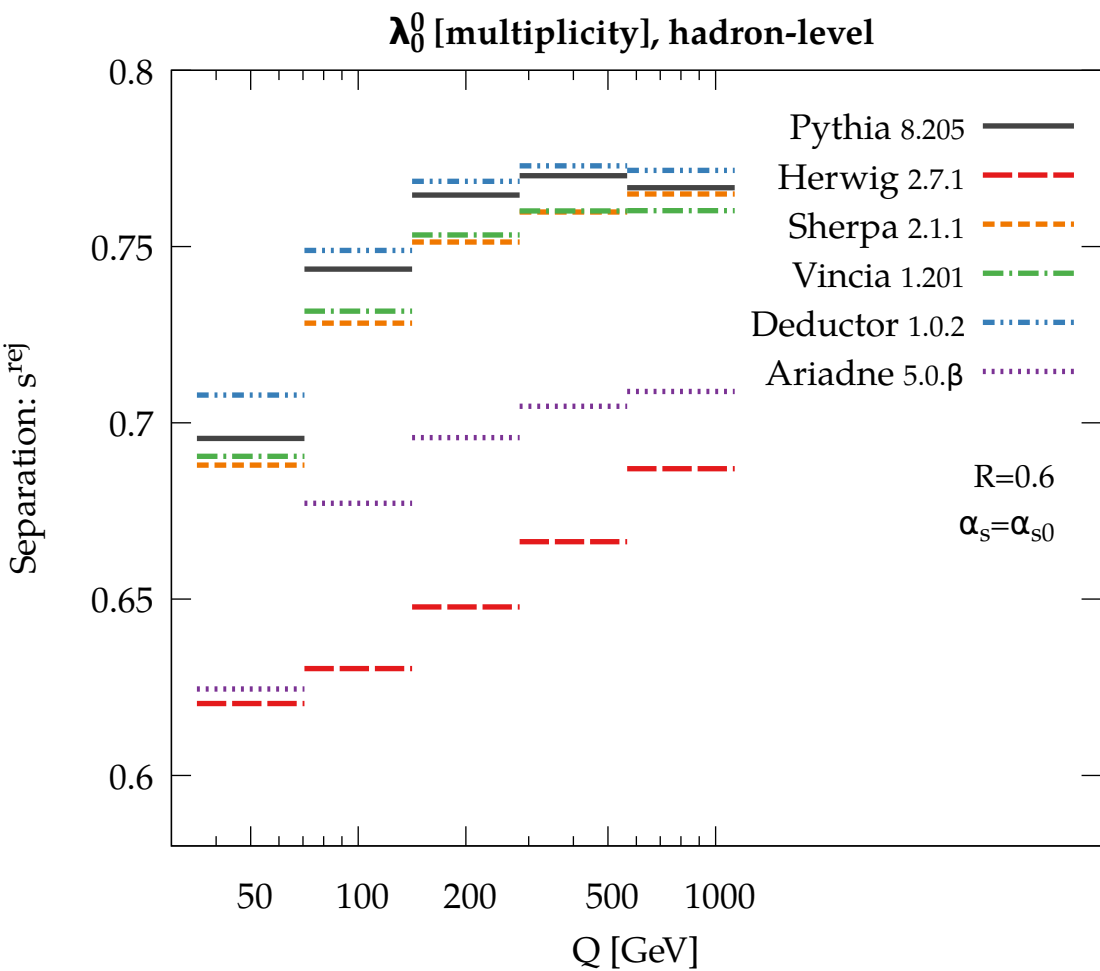

$\lambda_0^2 [(p_T^D)^2]$ , hadron-level

Separation:  $s^{\text{rej}}$

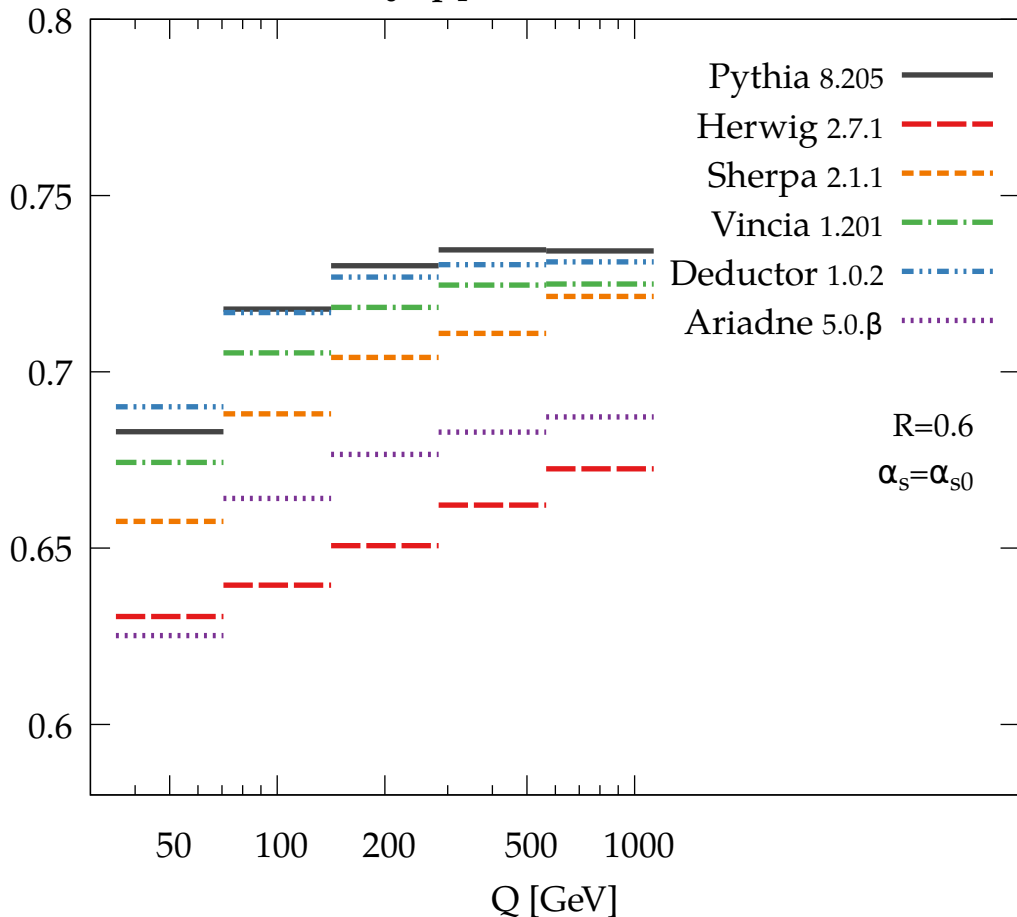

Supplement: Supplementary file 9 [file quarkgluon_fig_I2_GA_10_05_hadron_Qdep.pdf]
