# Supplementary material for: Les Houches 2015: Physics at TeV Colliders Standard Model Working Group Report
Source: arXiv:1605.04692 source file (2016-05-16)

# $\lambda_{0.5}^1$ [LHA], parton-level

Separation:  $\Delta$

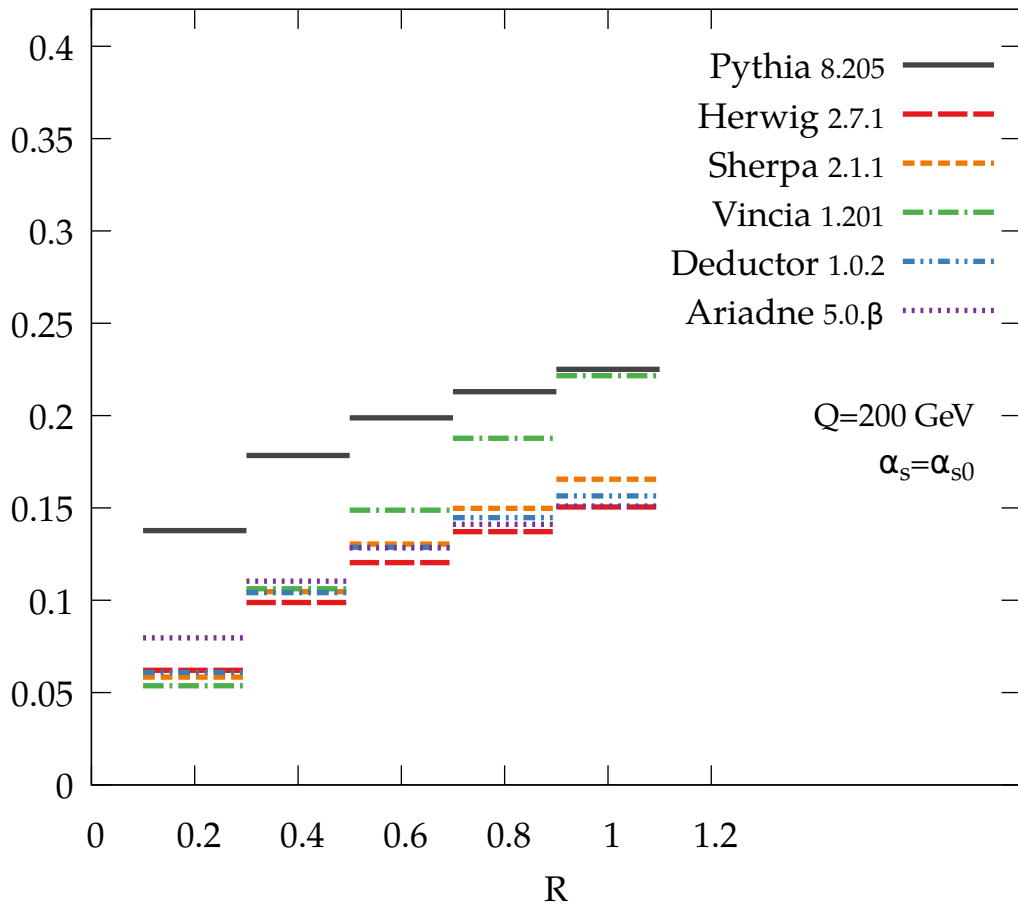

$\lambda_1^1$ , parton-levelSeparation:  $\Delta$ 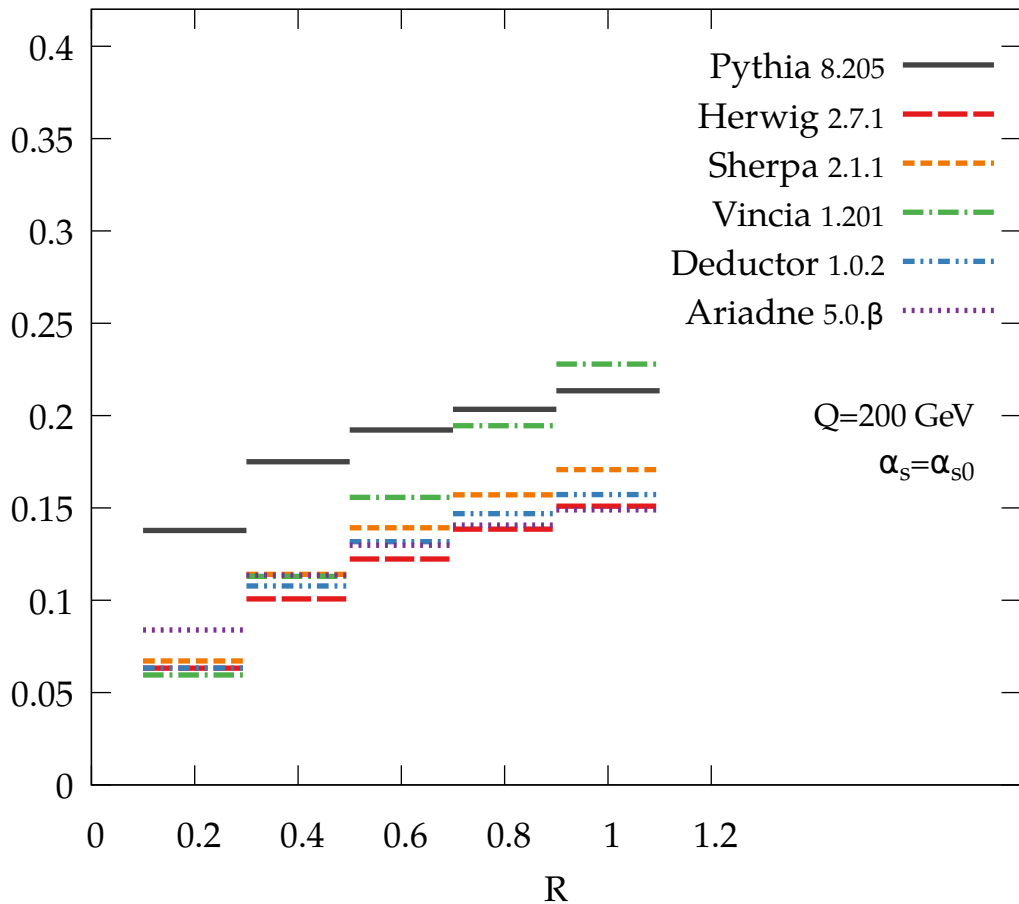

$\lambda_2^1$ , parton-level

Separation:  $\Delta$

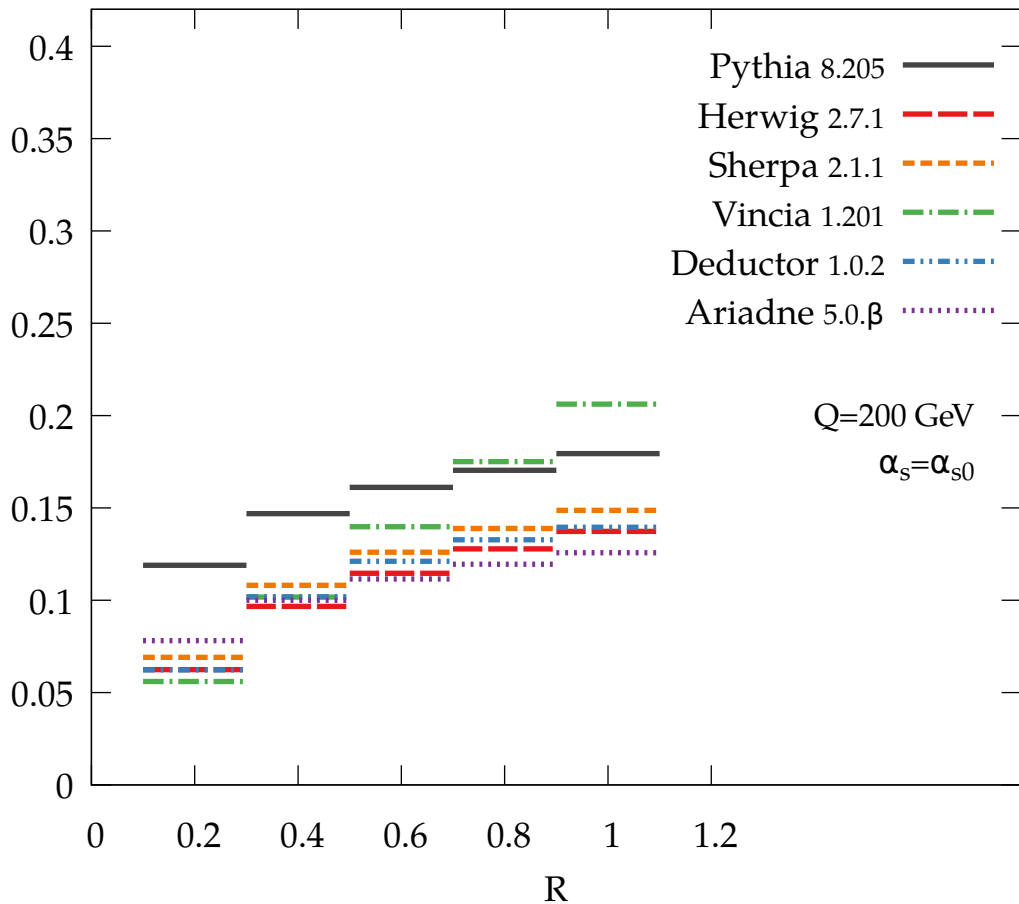

$\lambda_0^0$  [multiplicity], parton-level

Separation:  $\Delta$

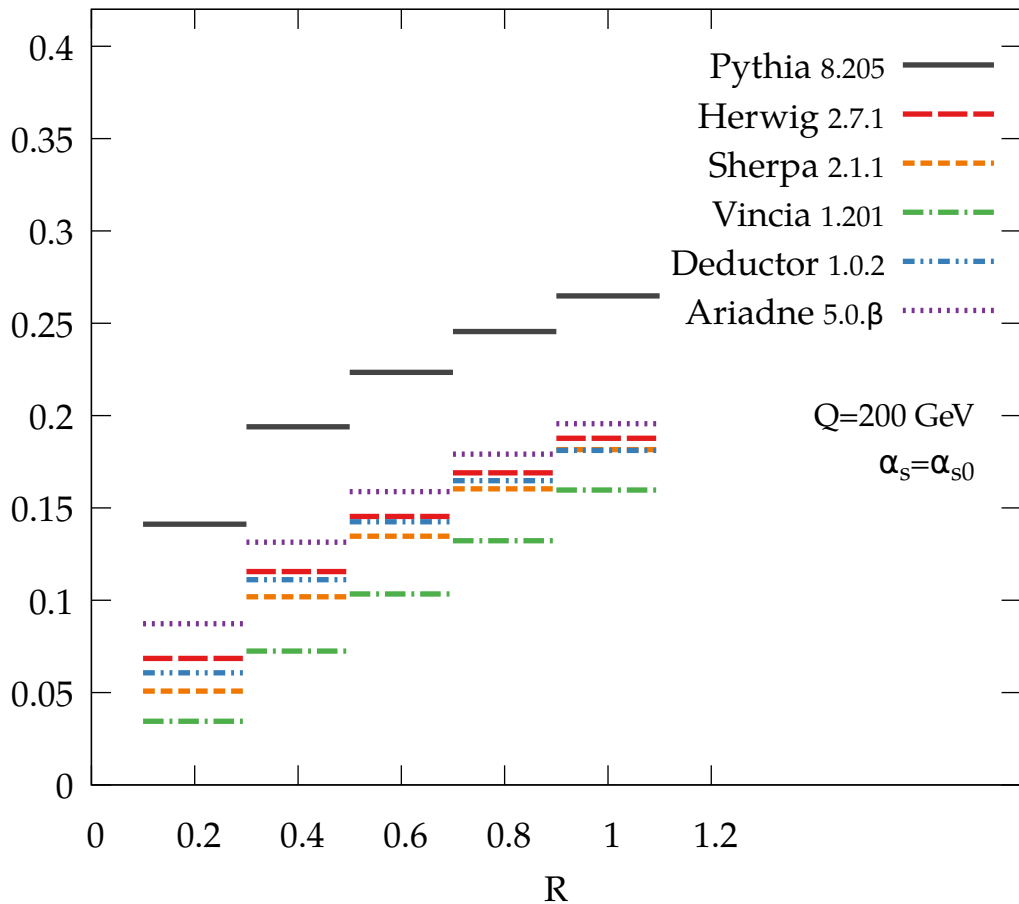

$\lambda_0^2 [(p_T^D)^2]$ , parton-level

Separation:  $\Delta$

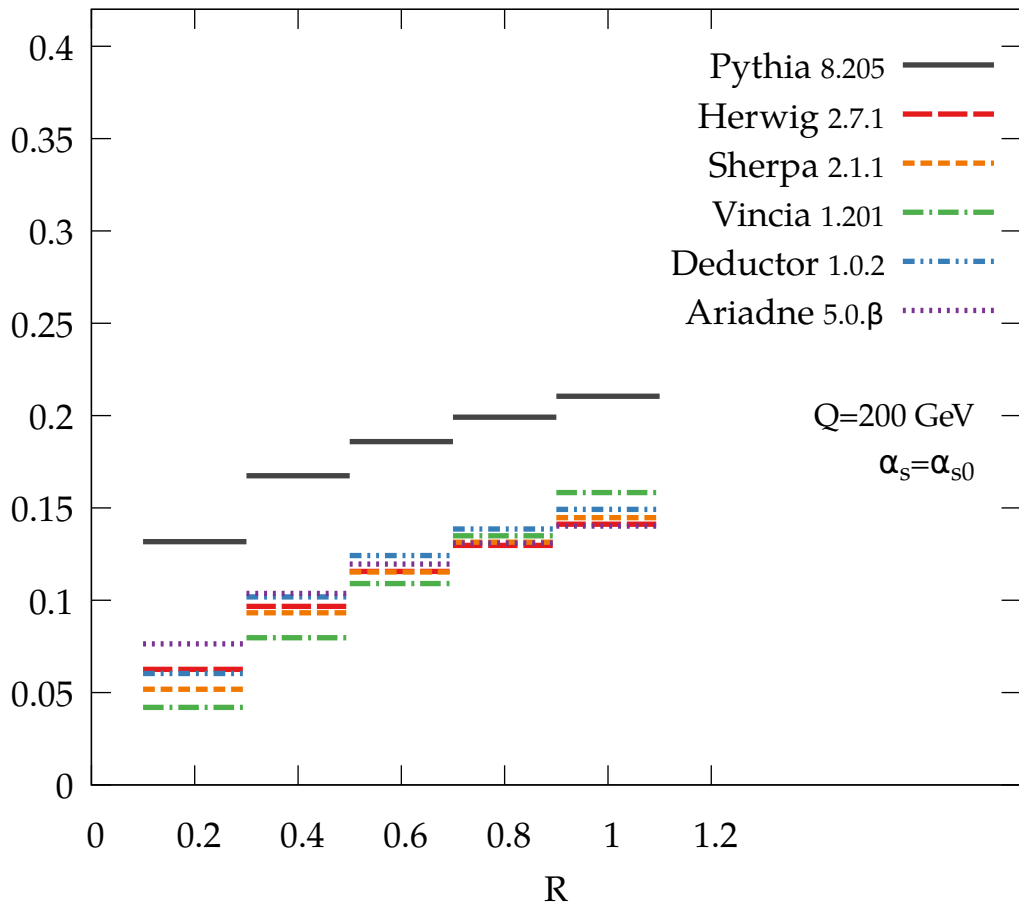

$\lambda_{0.5}^1$  [LHA], parton-levelSeparation:  $I_{1/2}$ 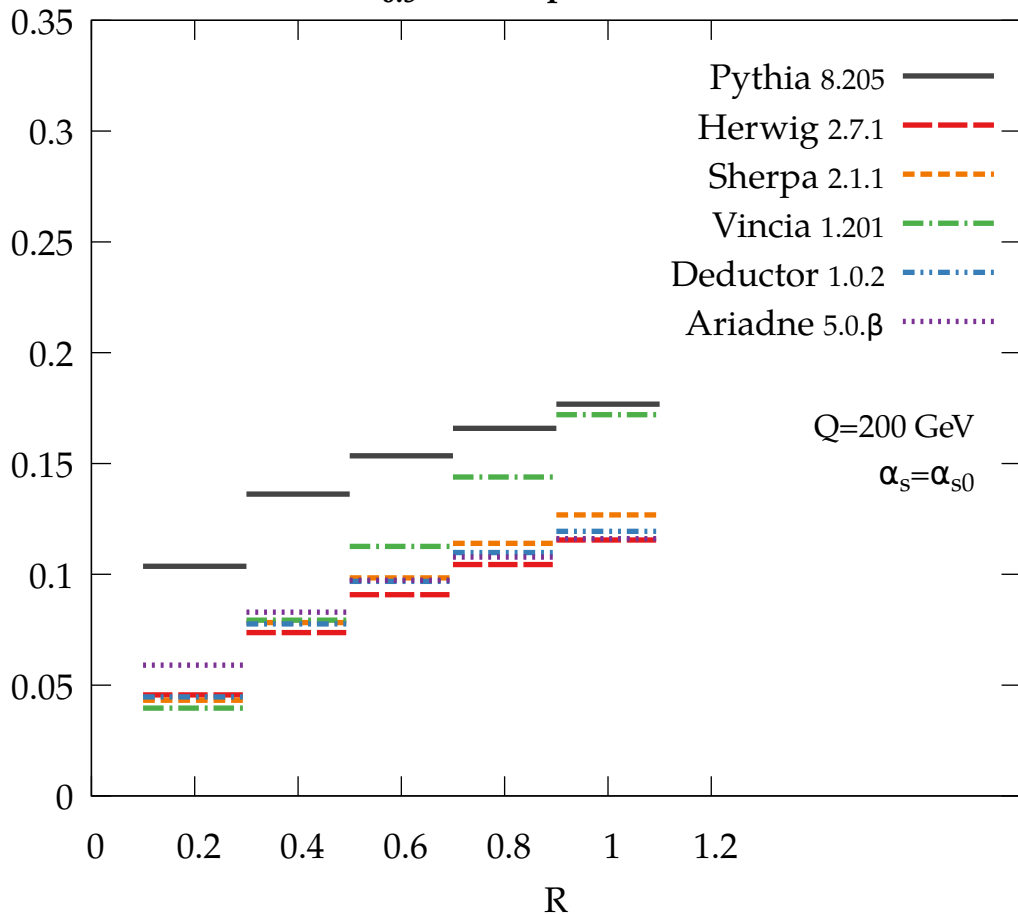

$\lambda_1^1$ , parton-level

Separation:  $I_{1/2}$

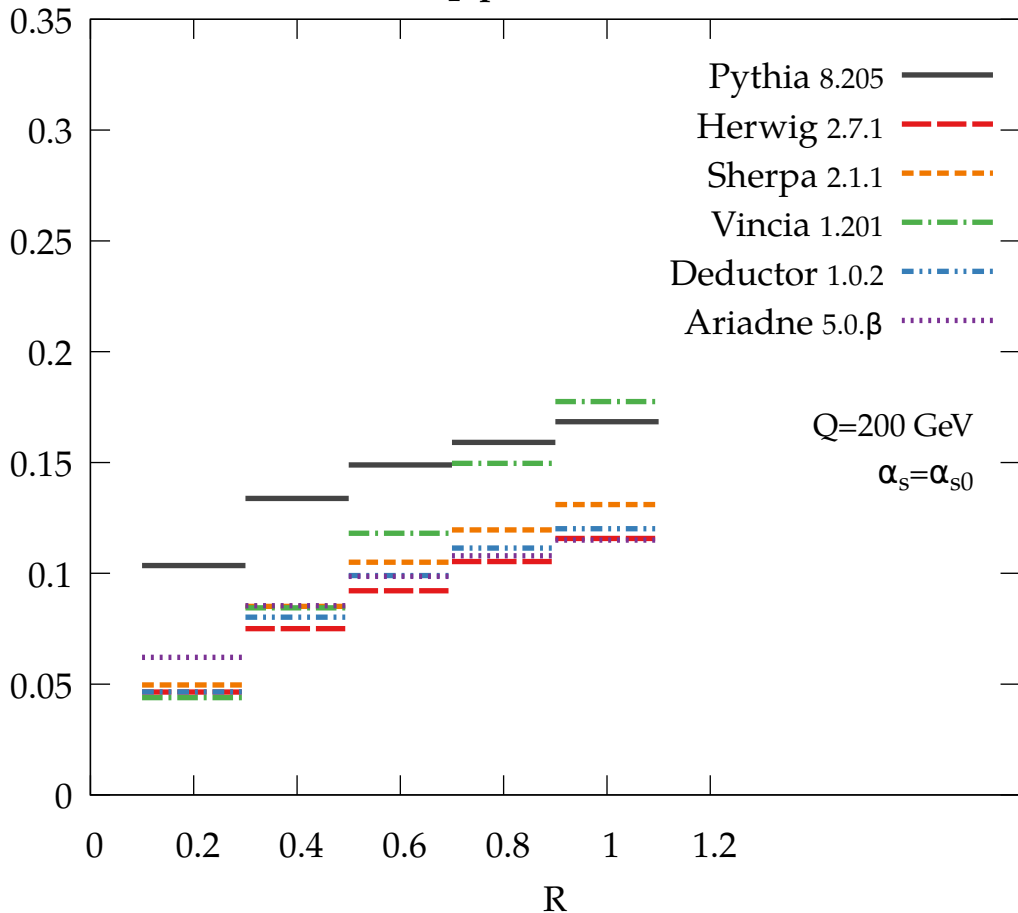

$\lambda_2^1$ , parton-level

Separation:  $I_{1/2}$

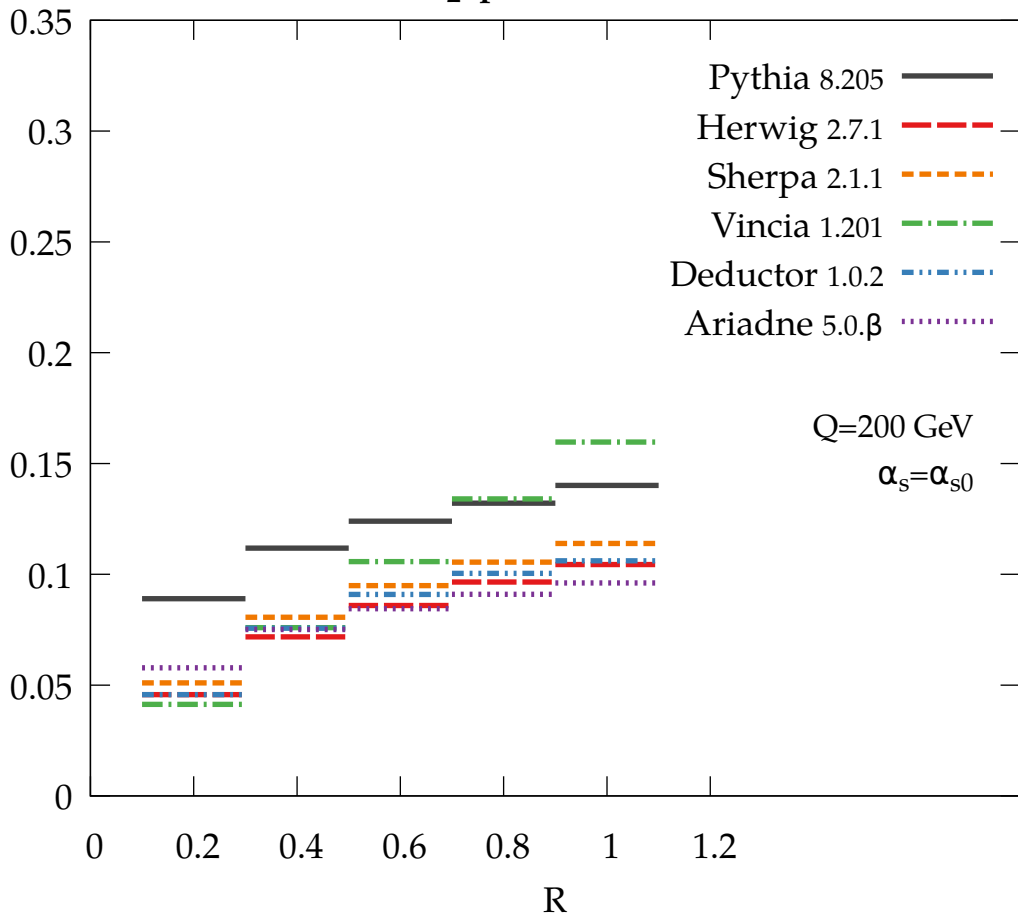



$\lambda_0^0$  [multiplicity], parton-level

Separation:  $I_{1/2}$

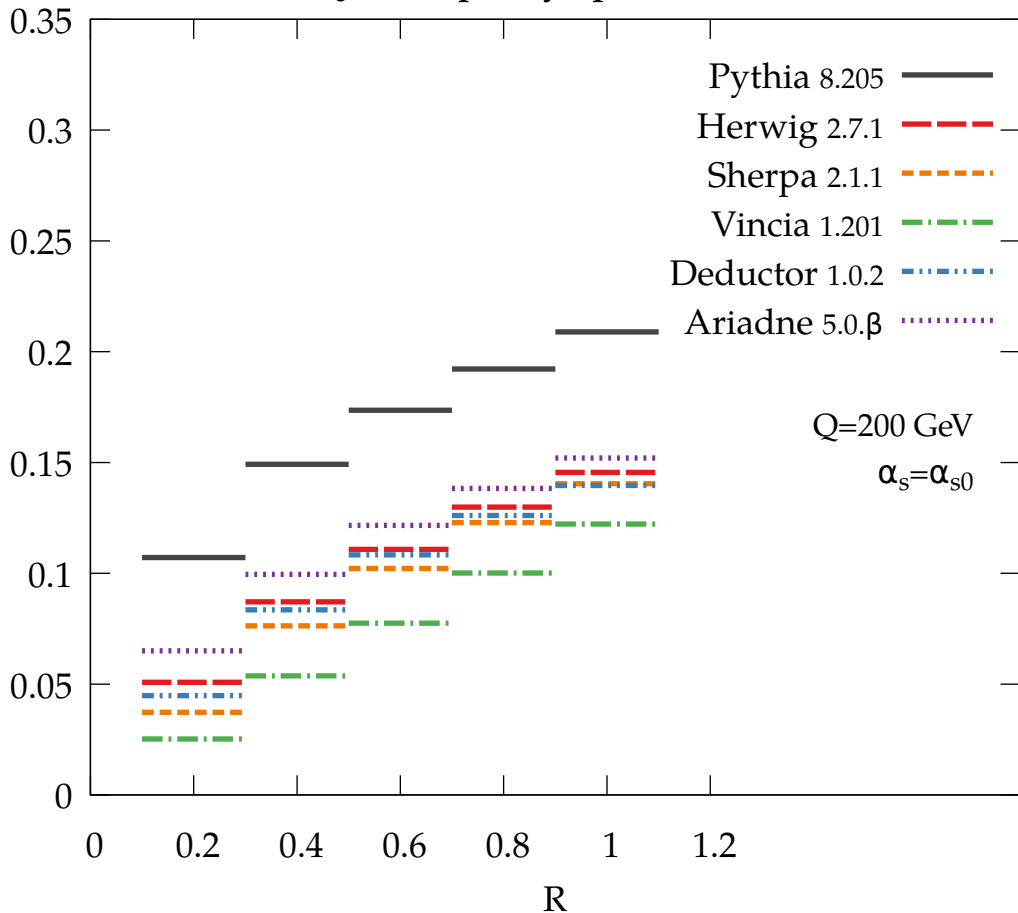

$\lambda_0^2 [(\mathbf{p}_T^D)^2]$ , parton-level

Separation:  $I_{1/2}$

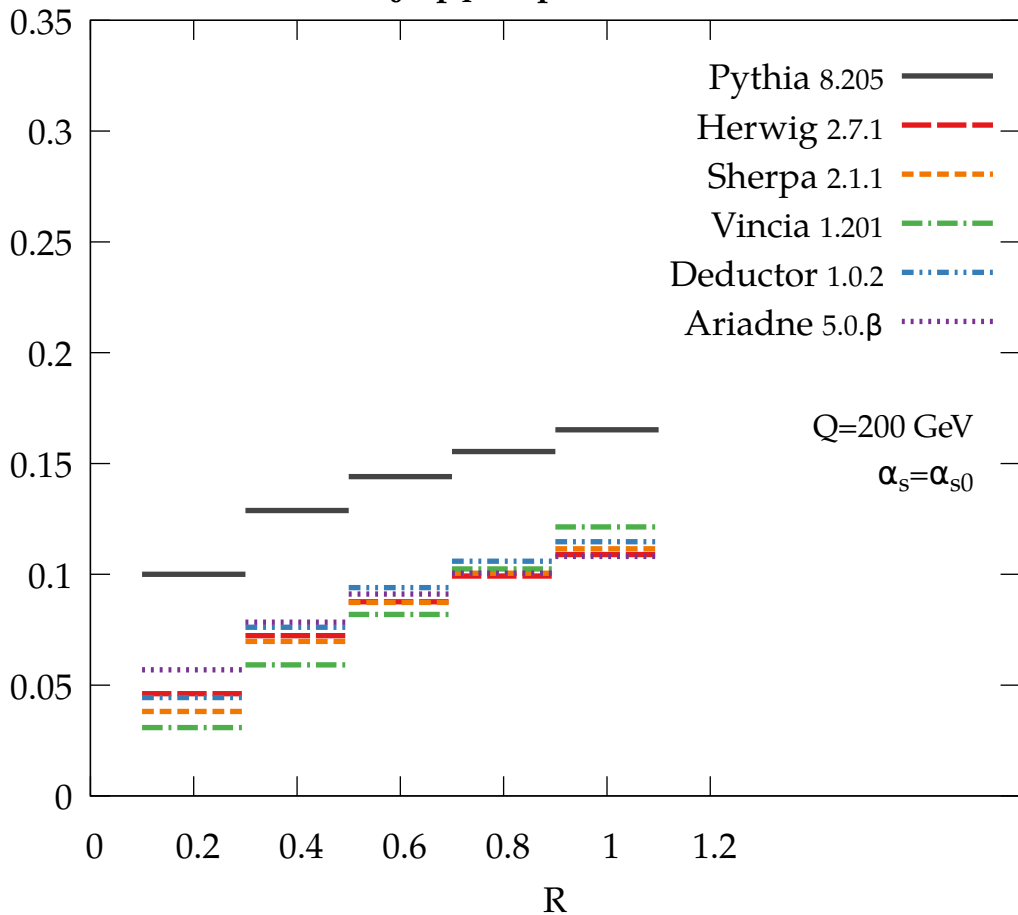

$\lambda_{0.5}^1$  [LHA], parton-level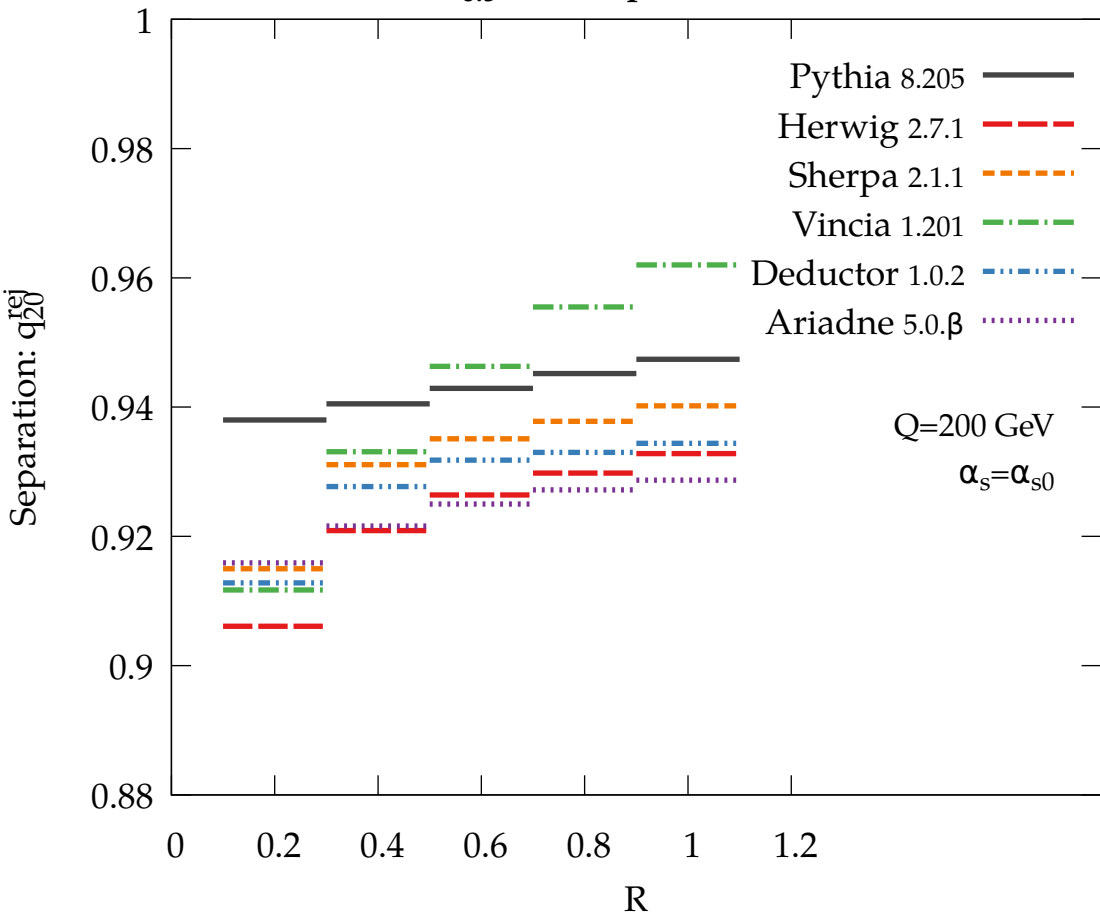

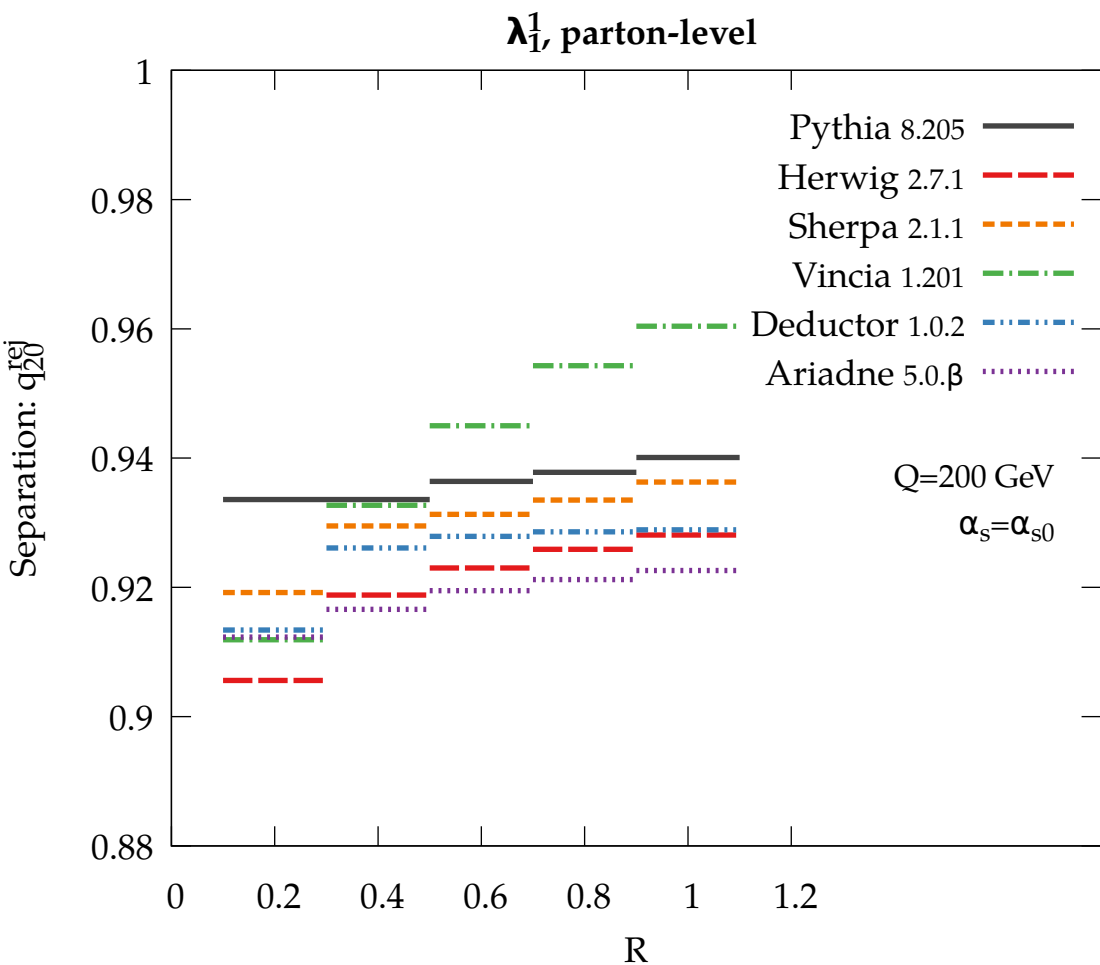

$\lambda_2^1$ , parton-level

Separation:  $q_{20}^{\text{rej}}$

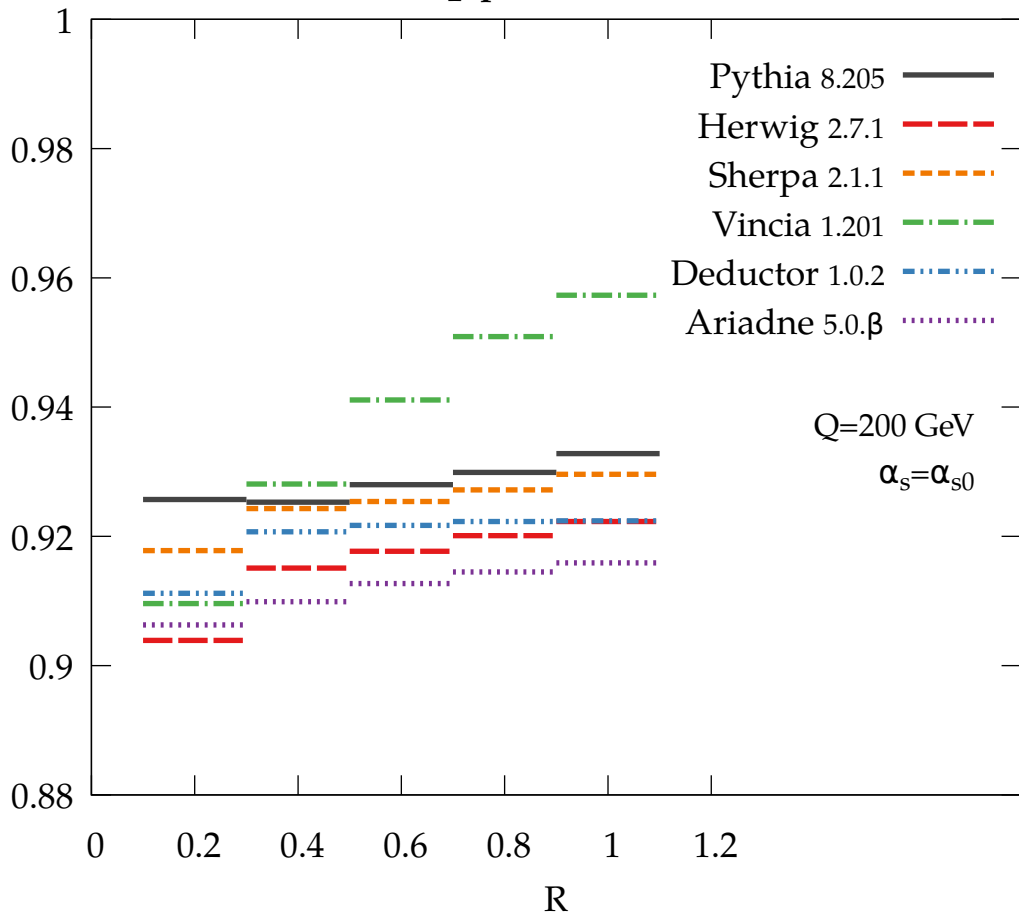

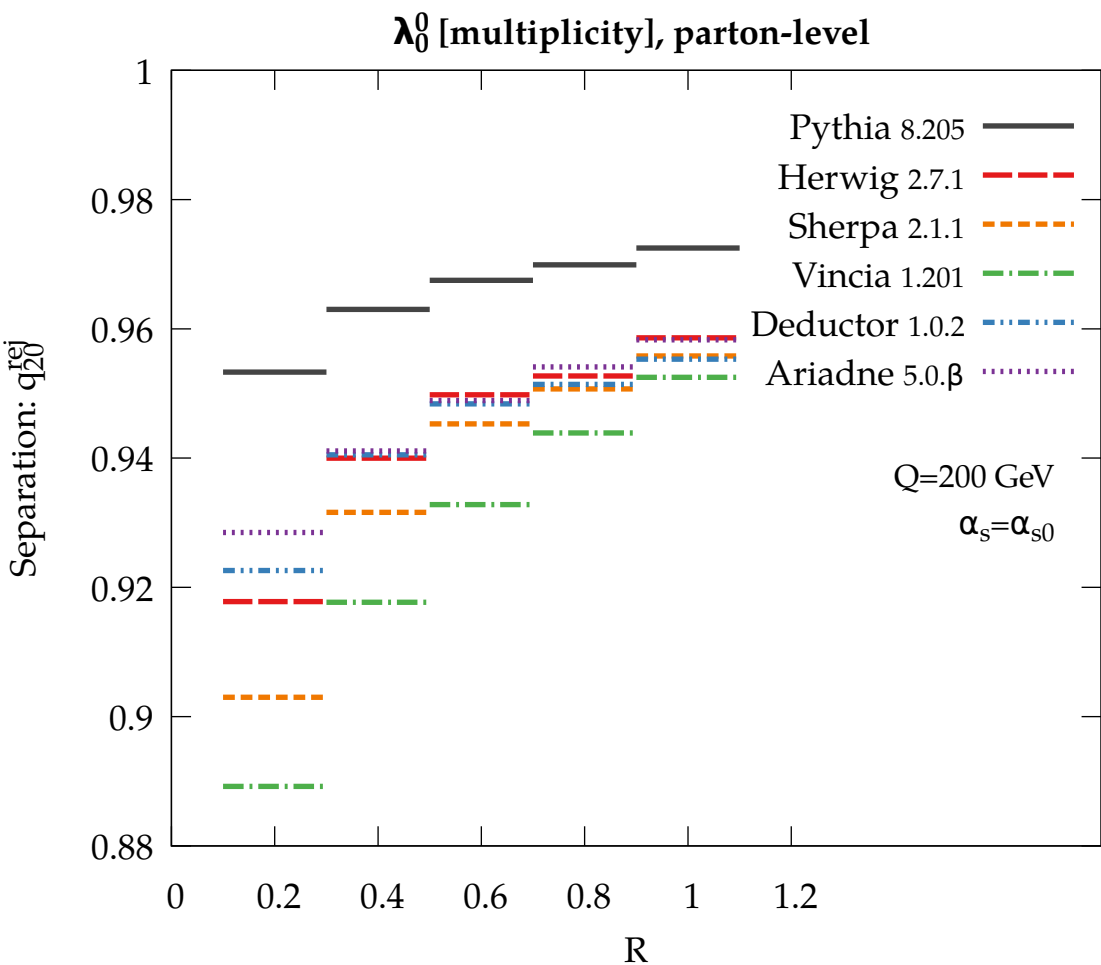

$\lambda_0^2 [(p_T^D)^2]$ , parton-level

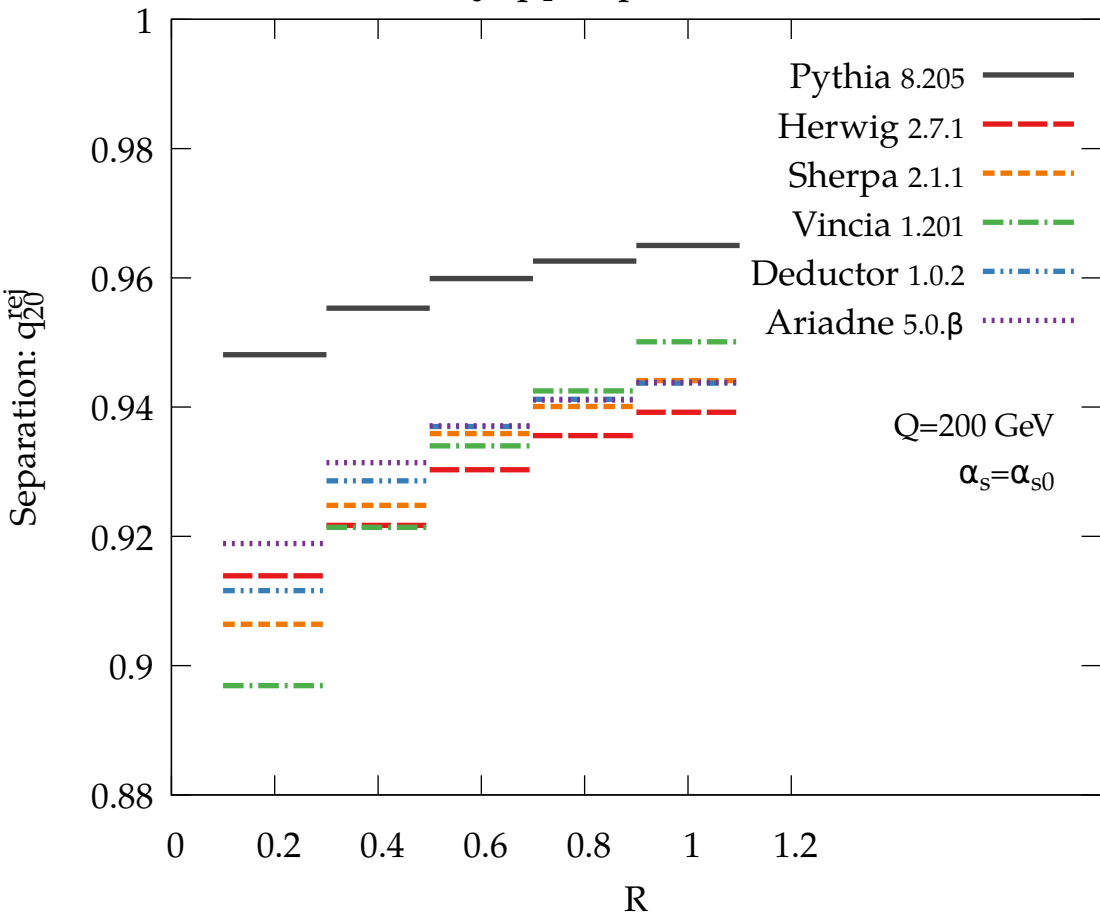

$\lambda_{0.5}^1$  [LHA], parton-level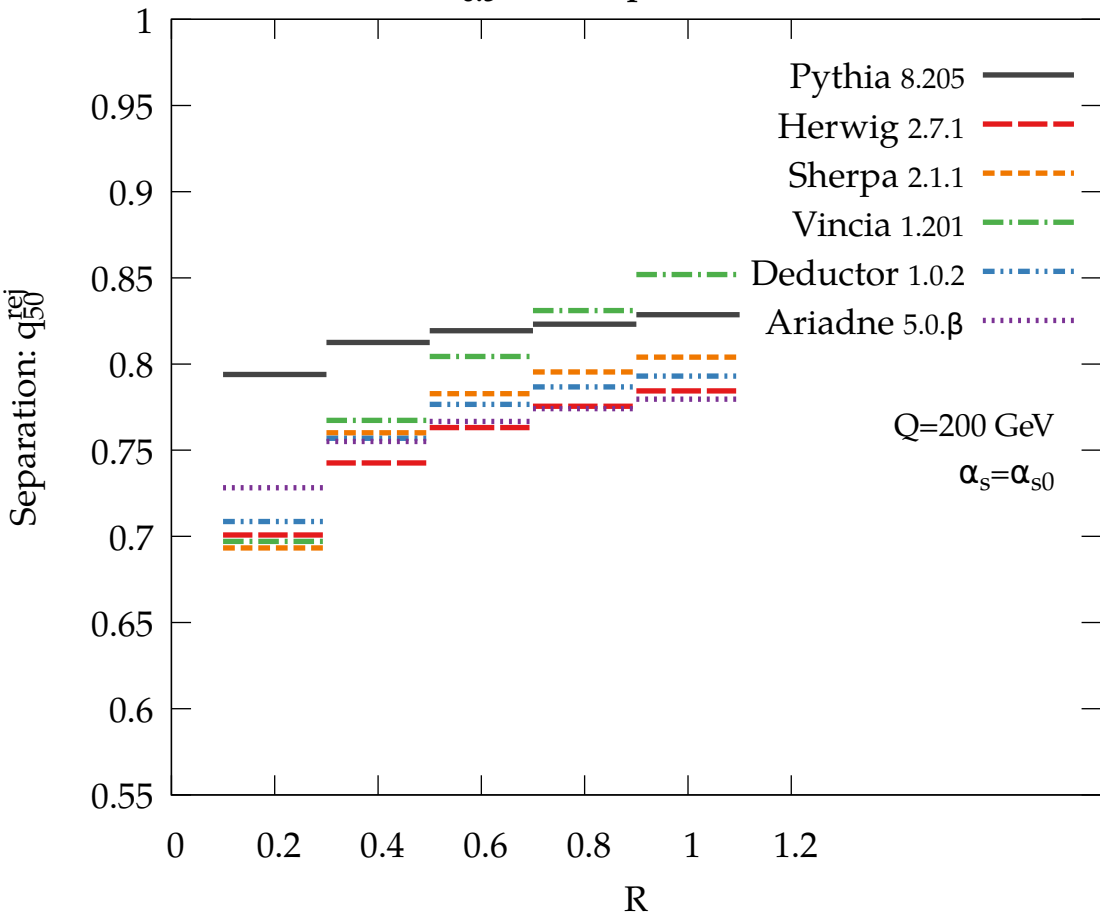



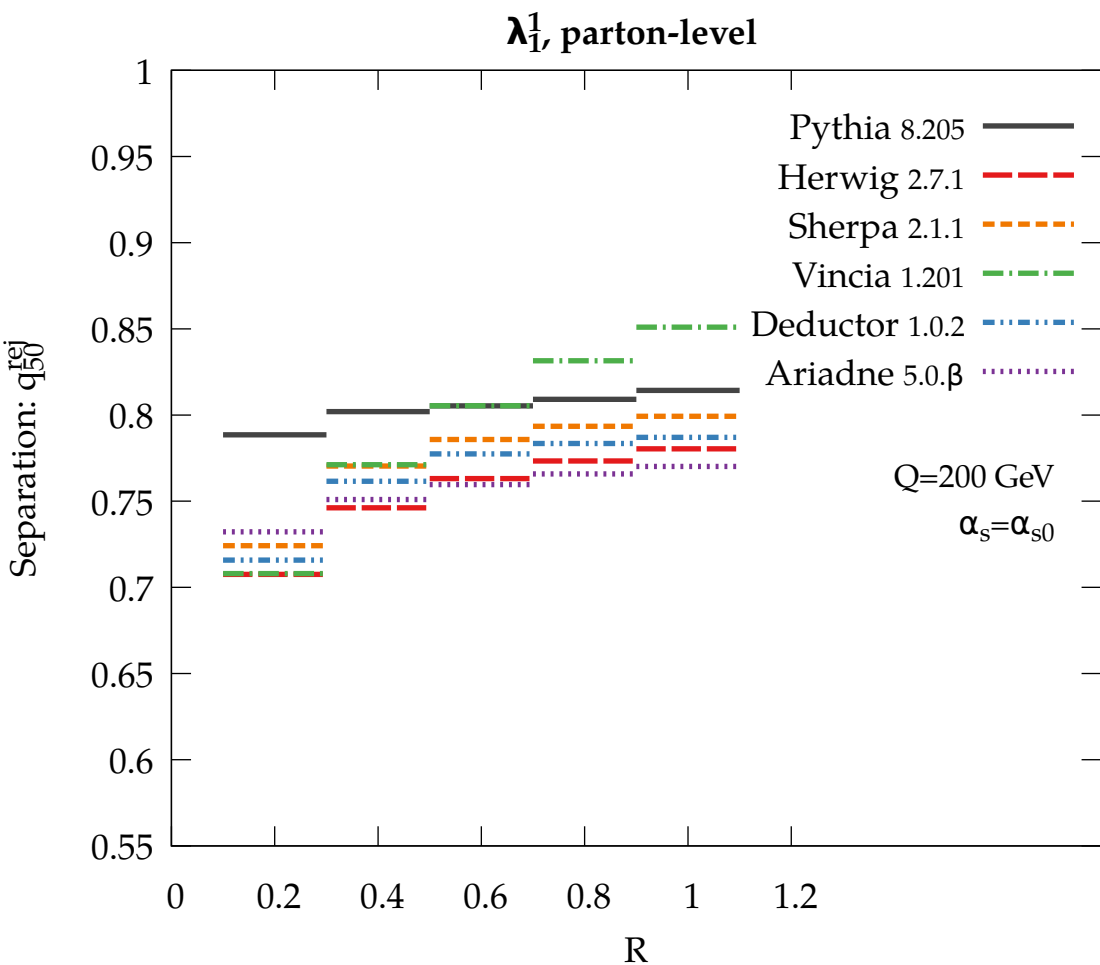

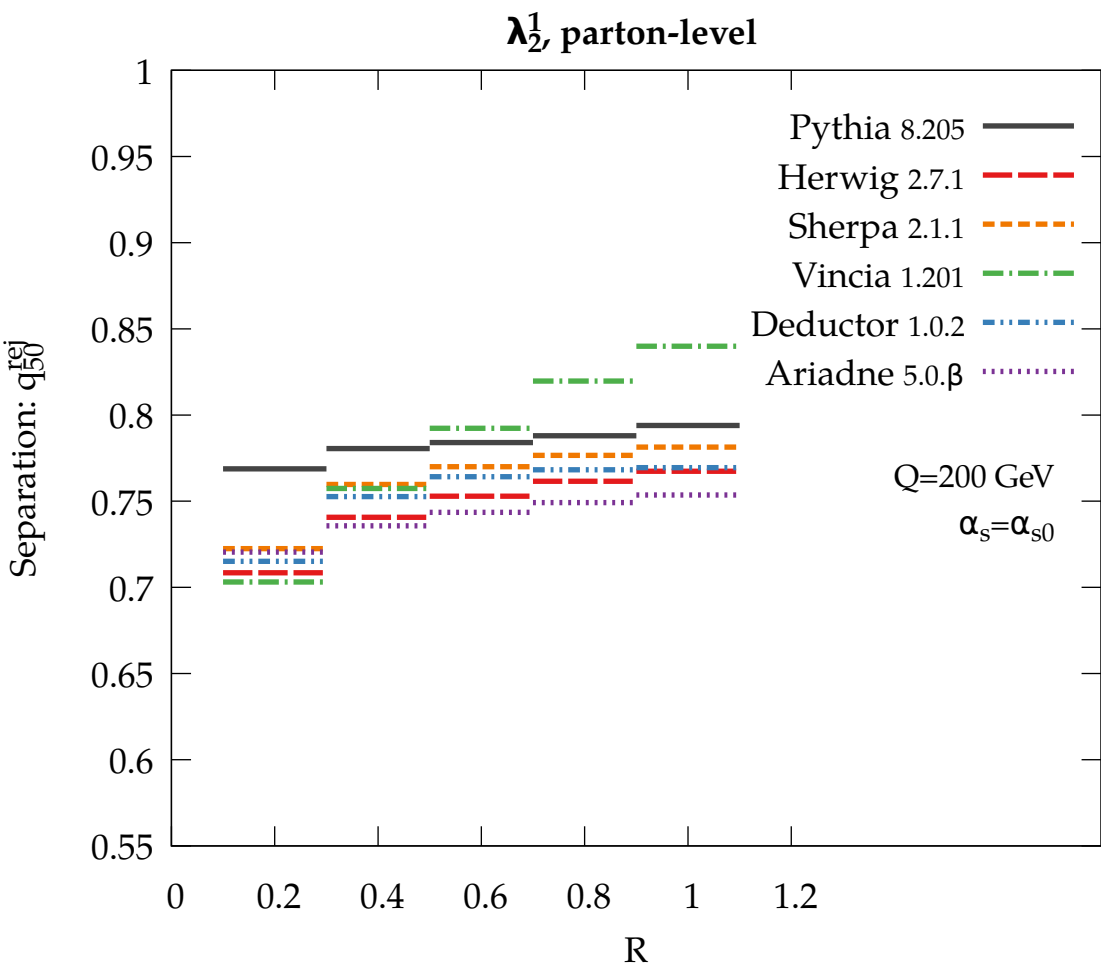

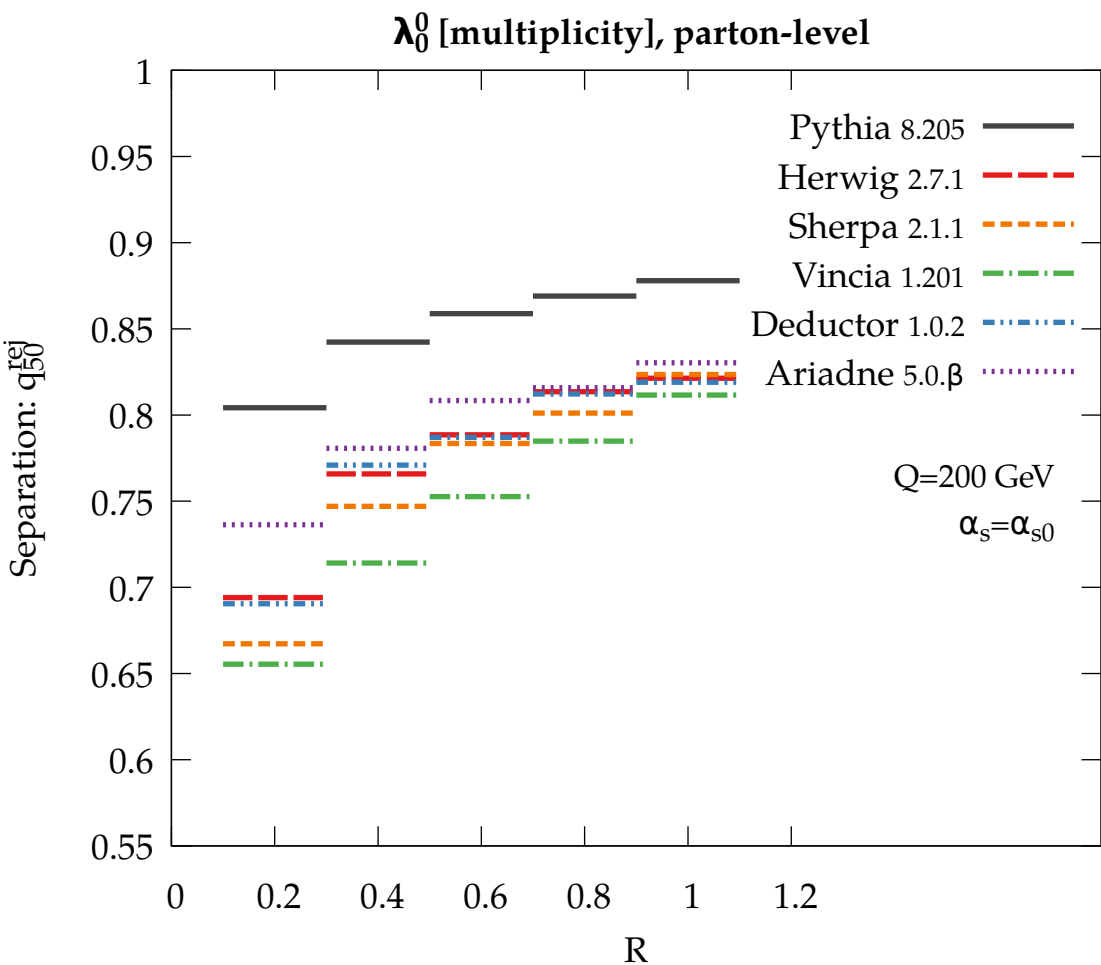

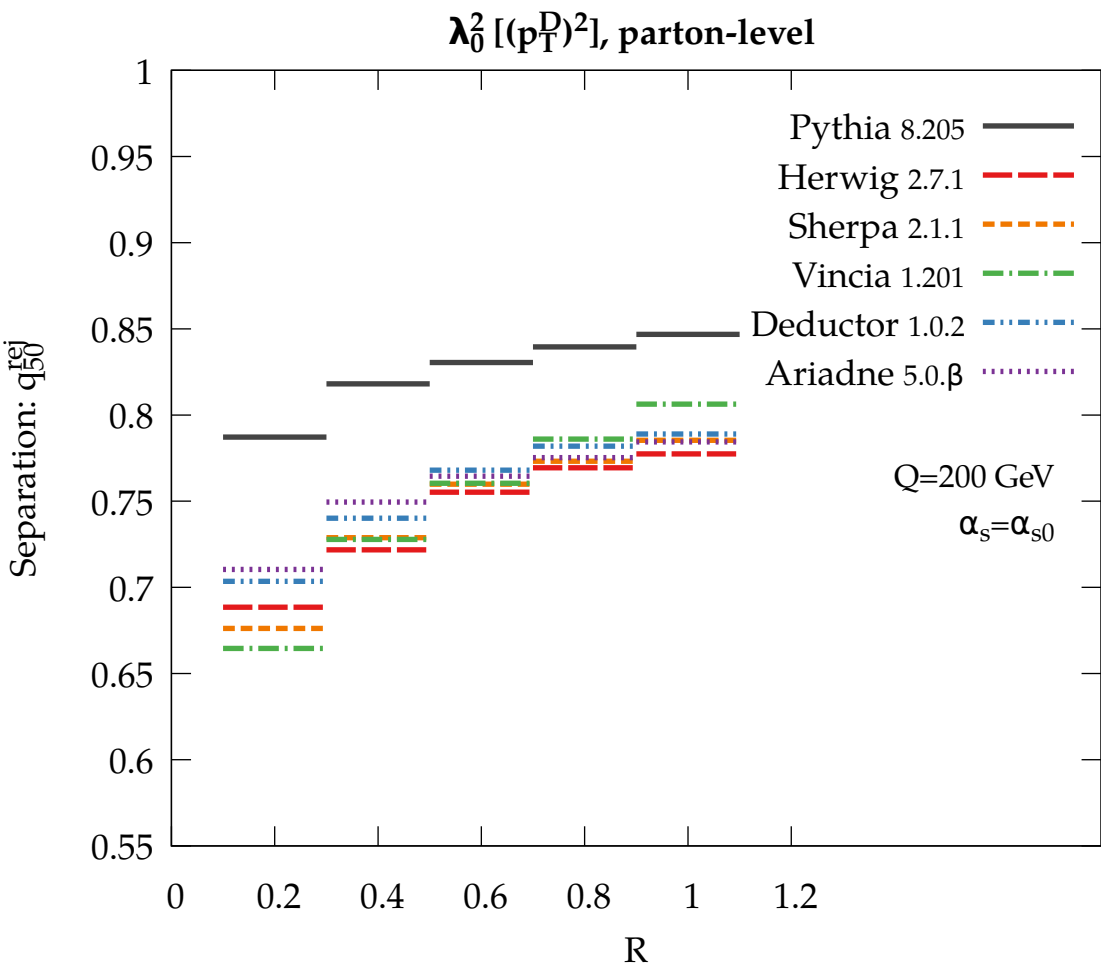

$\lambda_{0.5}^1$  [LHA], parton-level

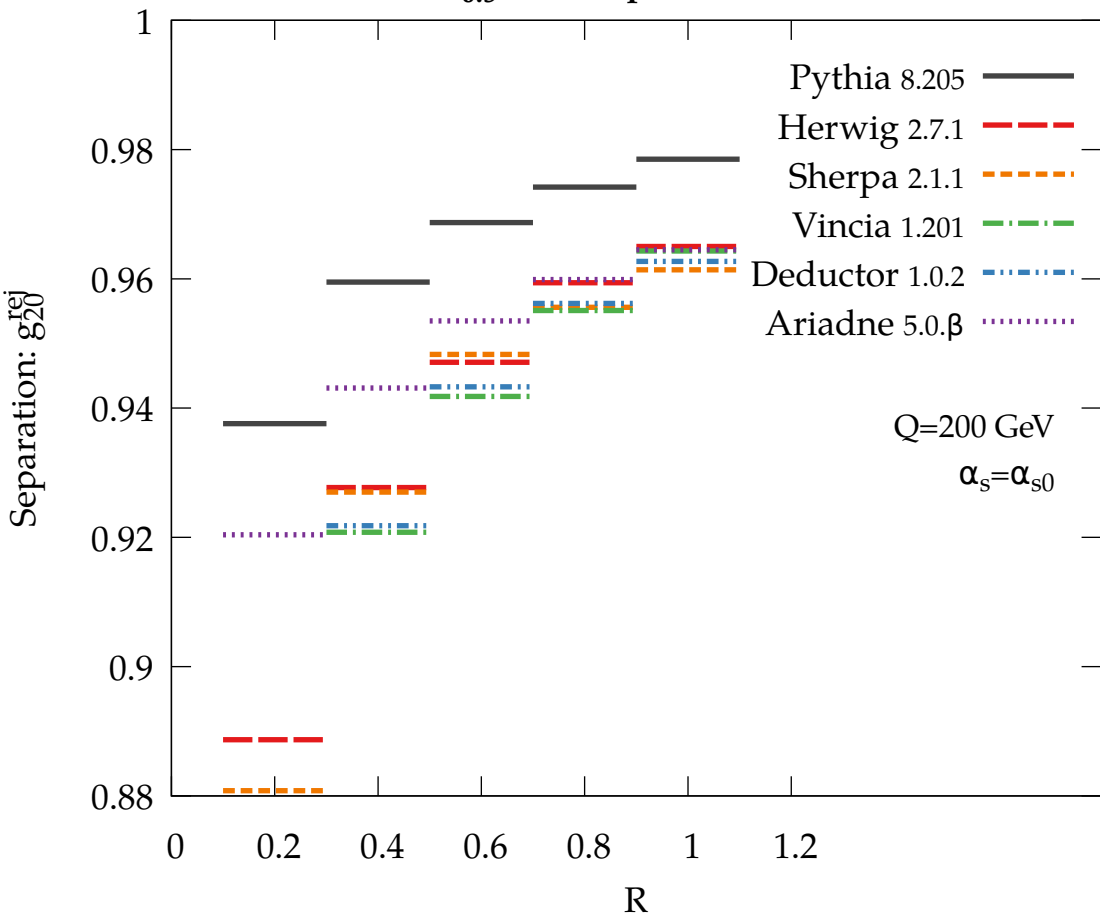

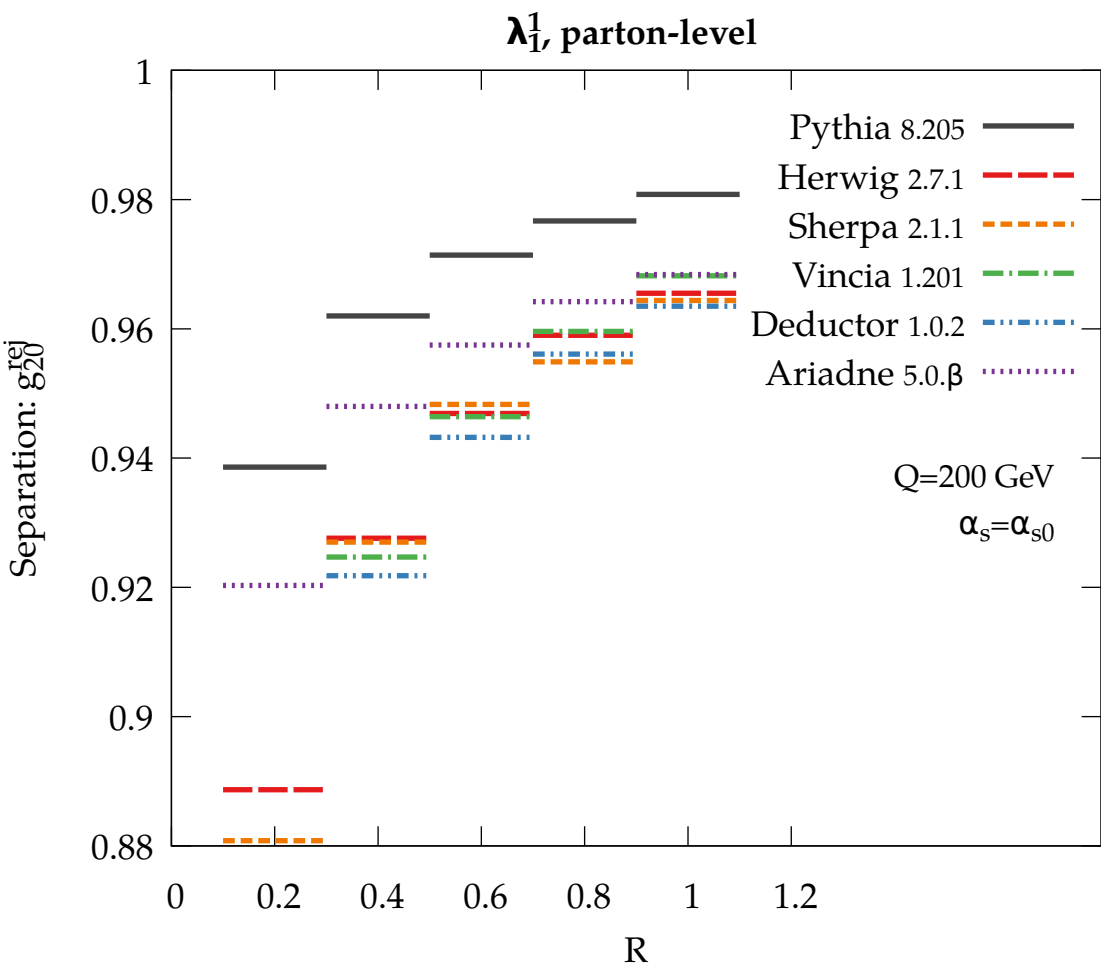

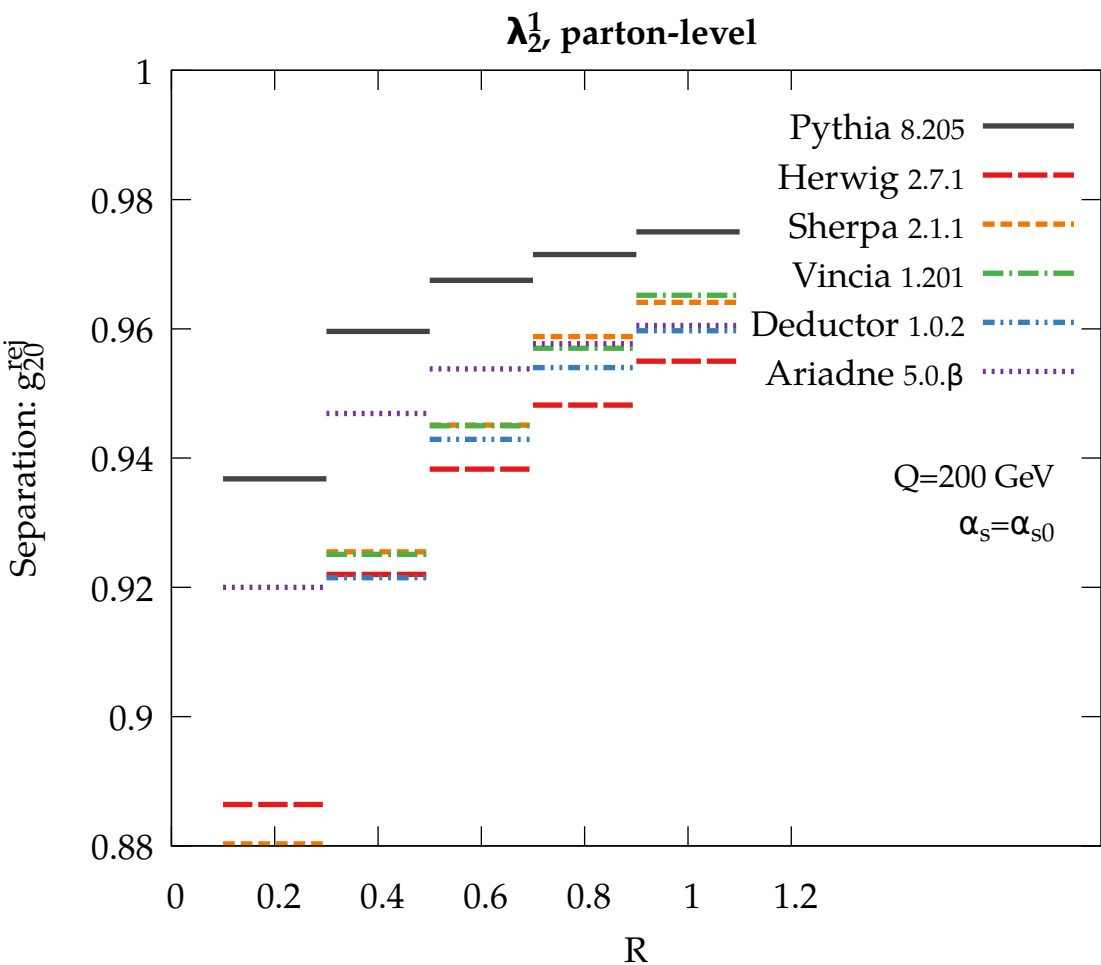

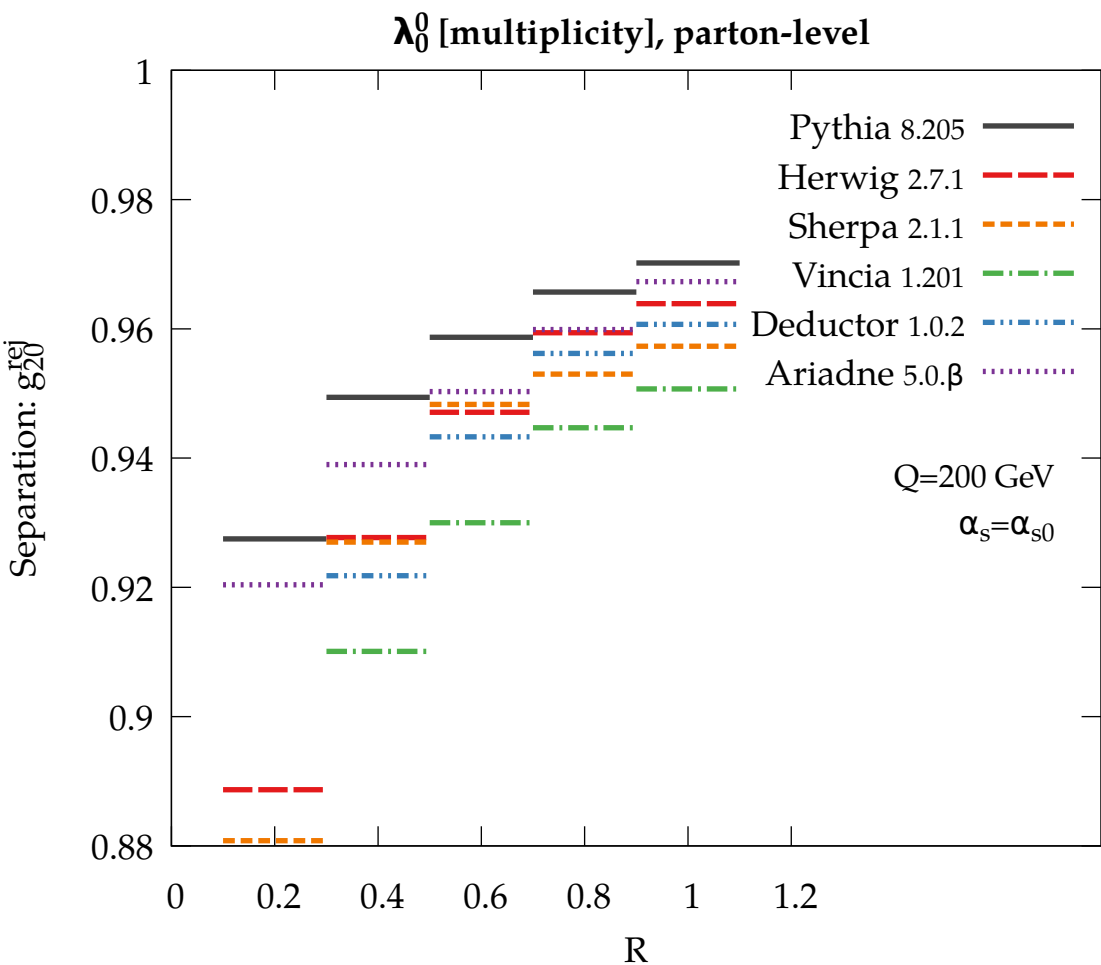



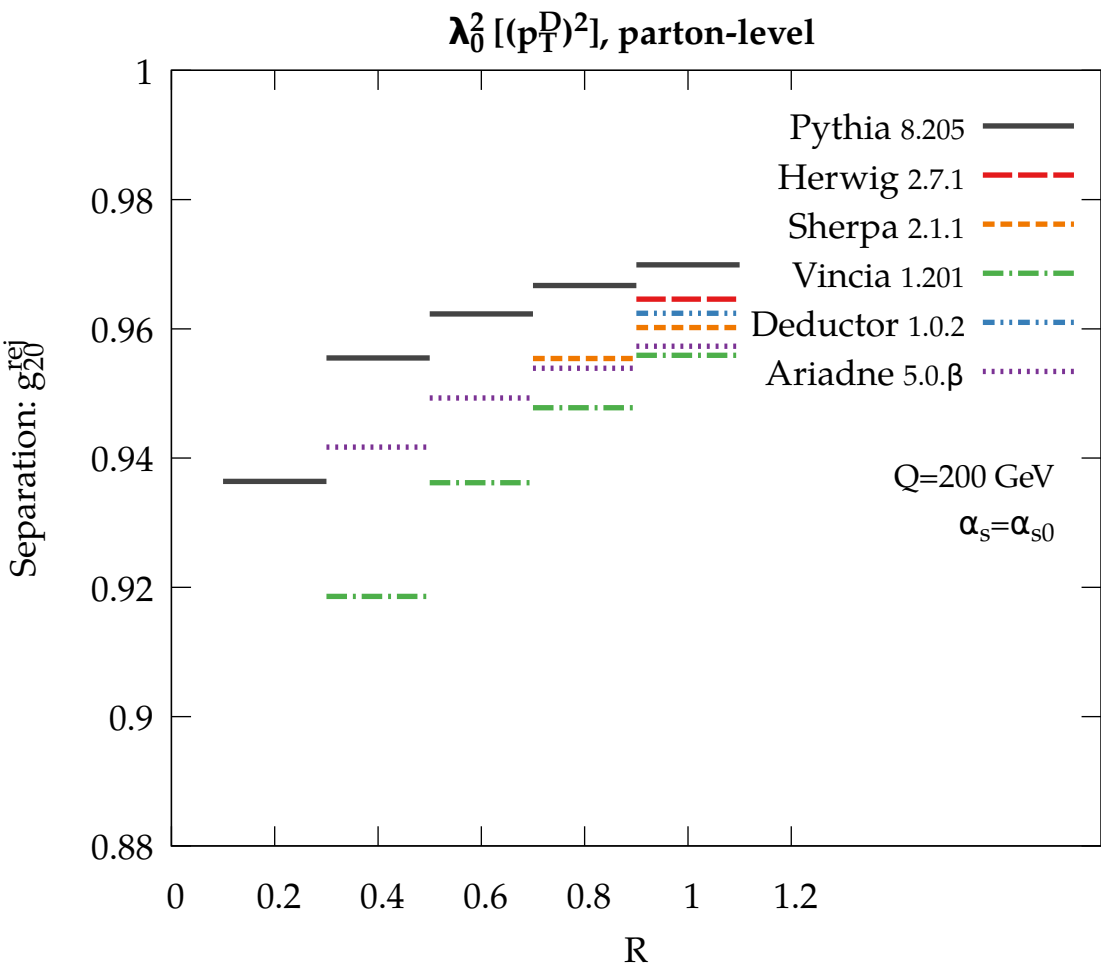

$\lambda_{0.5}^1$  [LHA], parton-level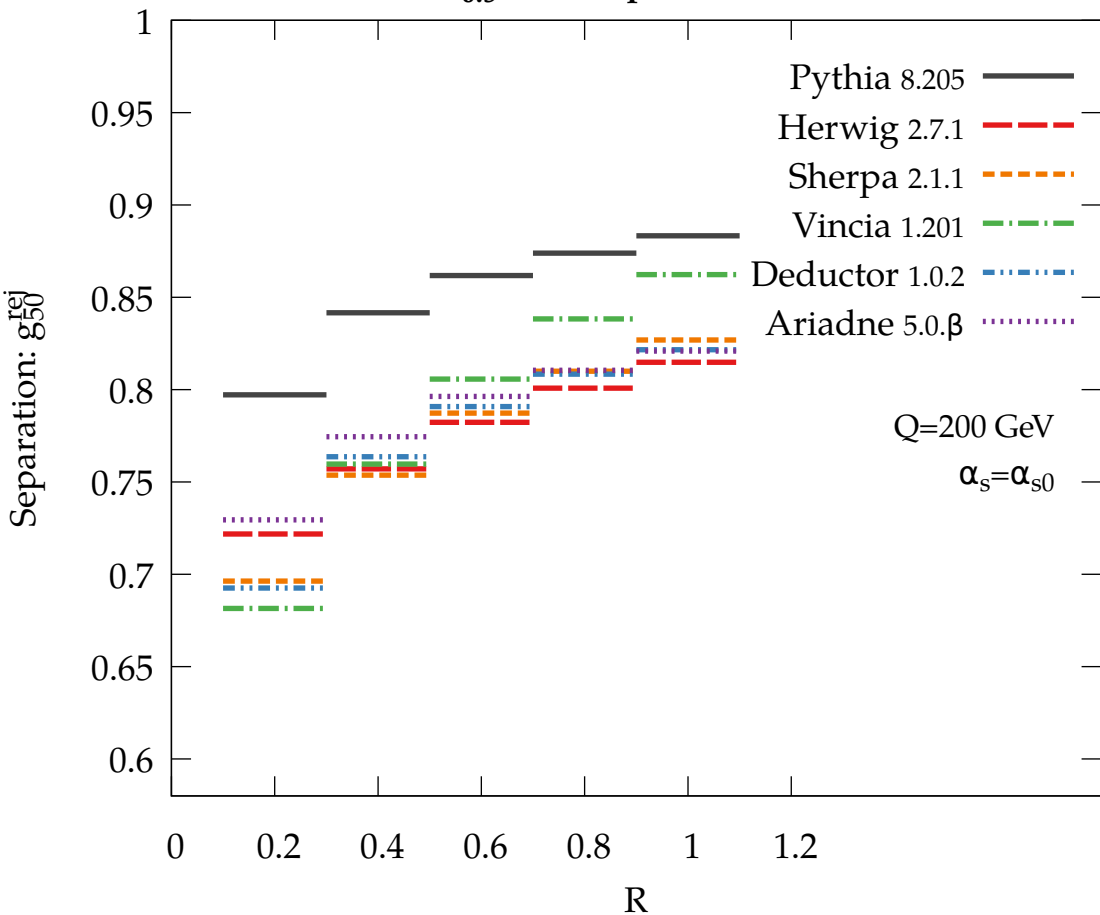

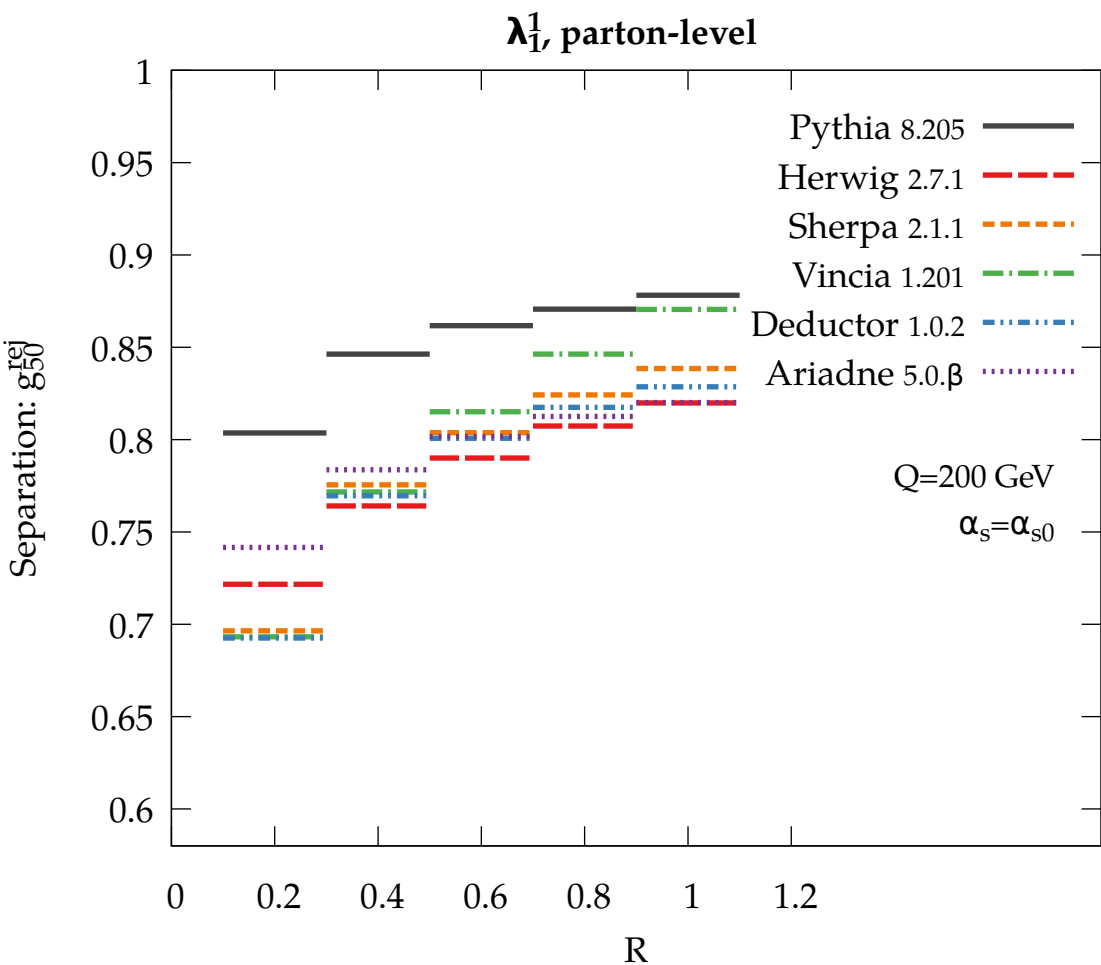

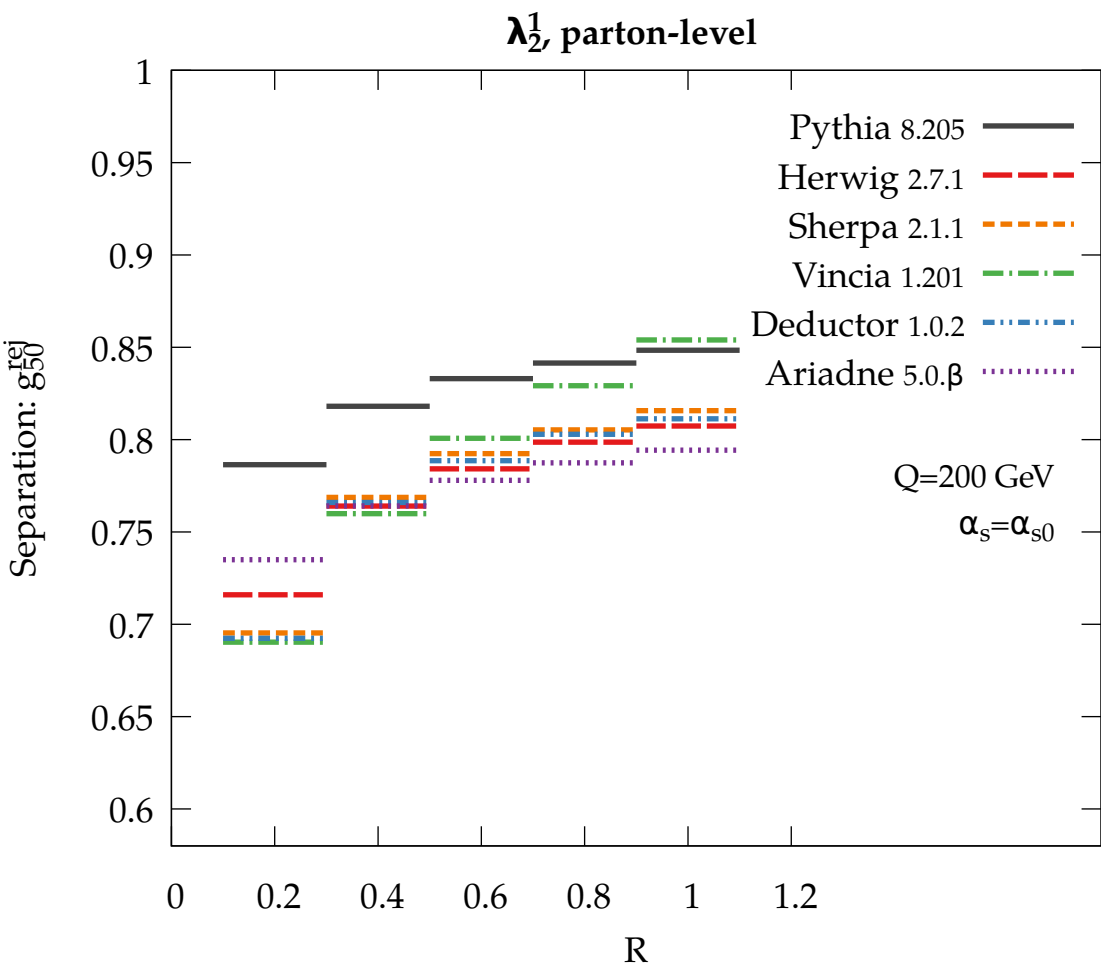

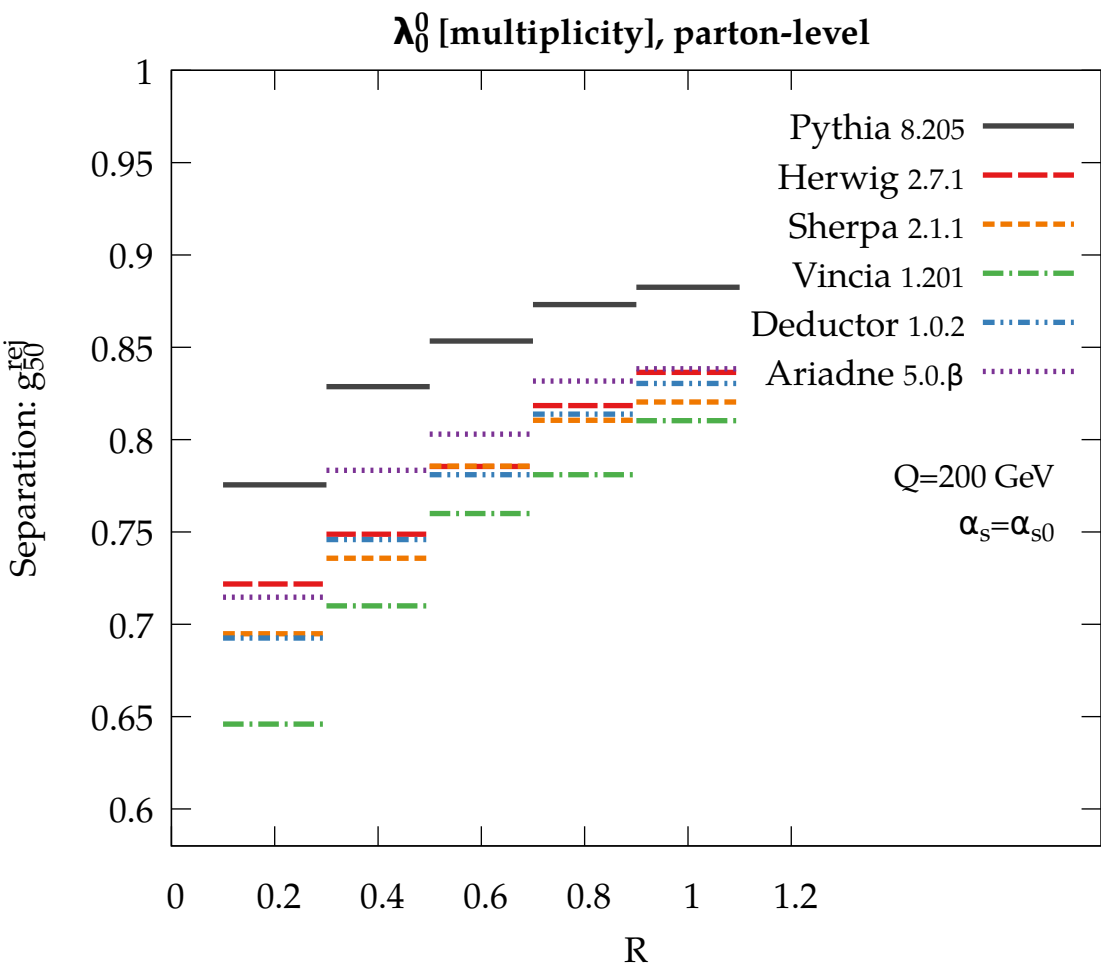

$\lambda_0^2 [(p_T^D)^2]$ , parton-level

Separation:  $g_{50}^{\text{rej}}$

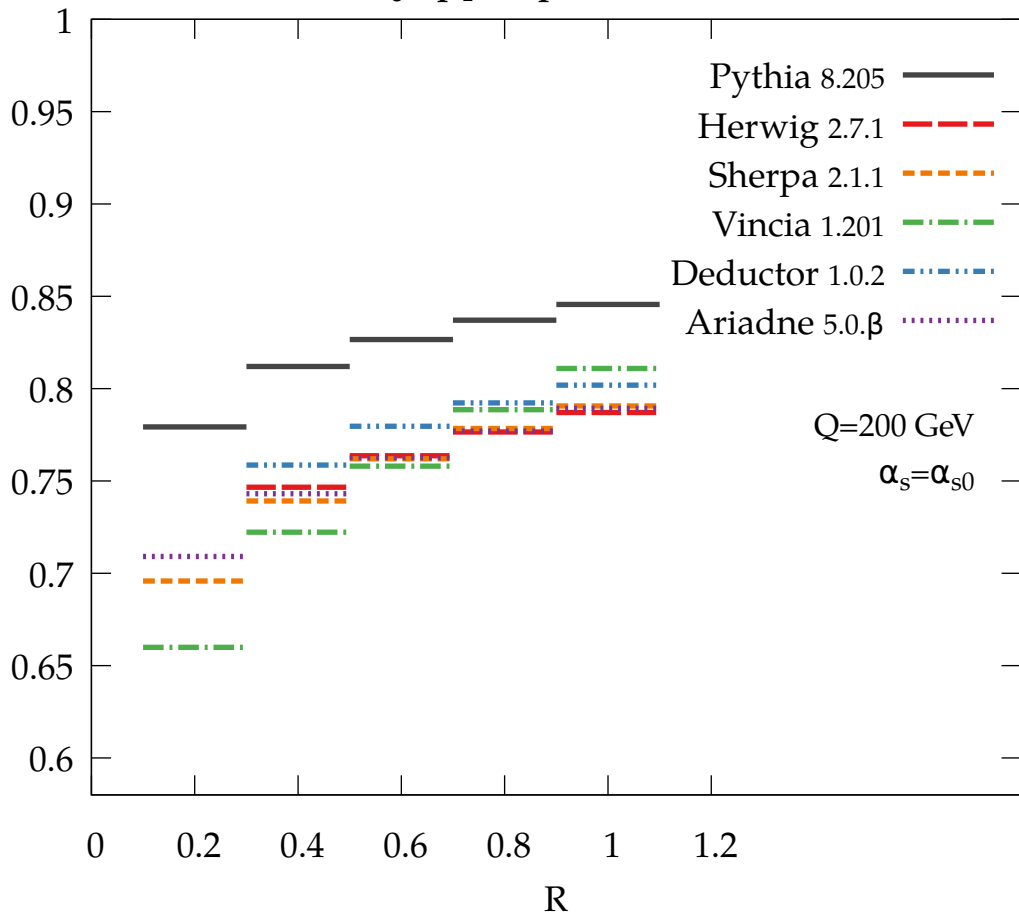

$\lambda_{0.5}^1$  [LHA], parton-level

Separation:  $s^{\text{rej}}$

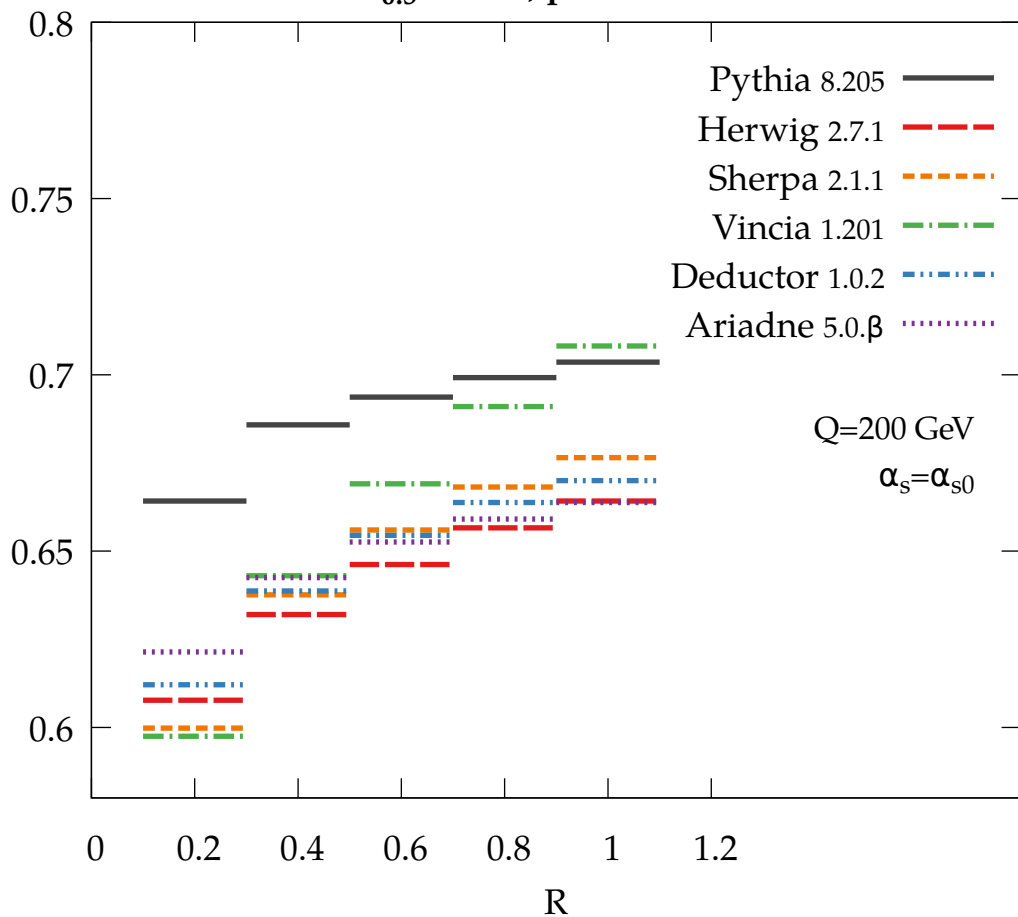

$\lambda_1^1$ , parton-level

Separation:  $s^{\text{rej}}$

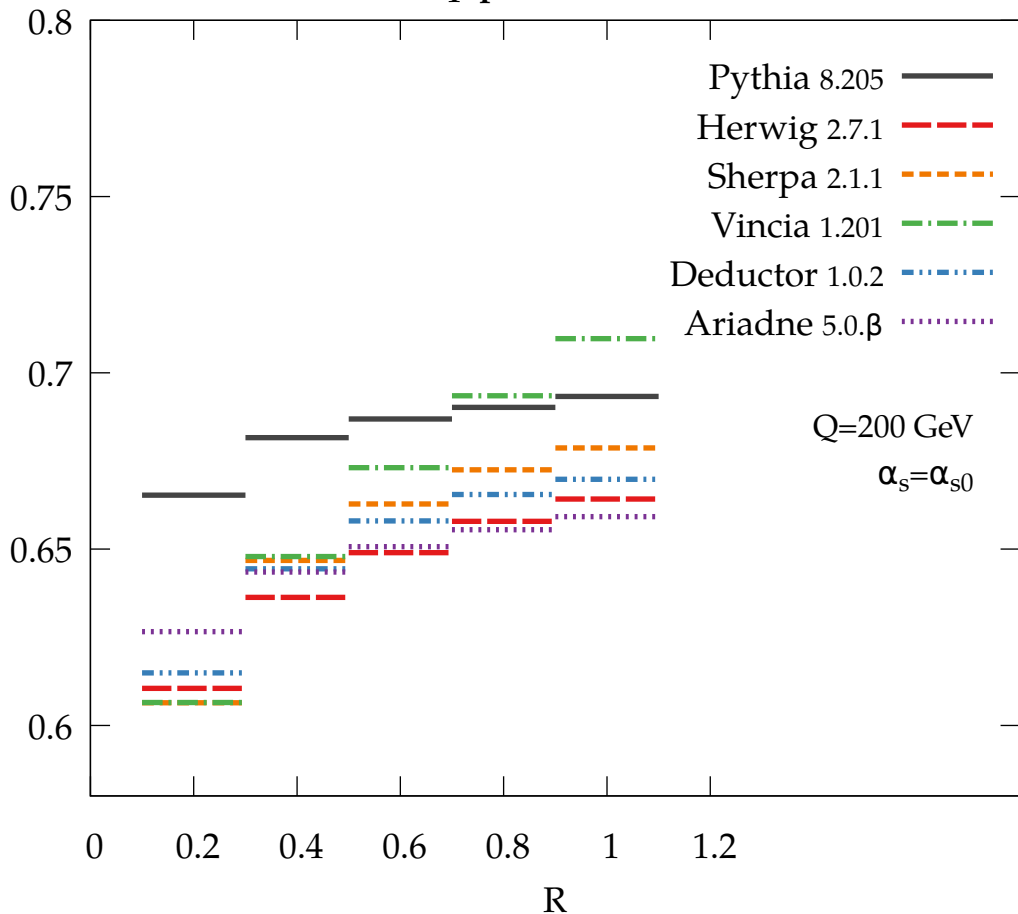



$\lambda_2^1$ , parton-level

Separation:  $s^{\text{rej}}$

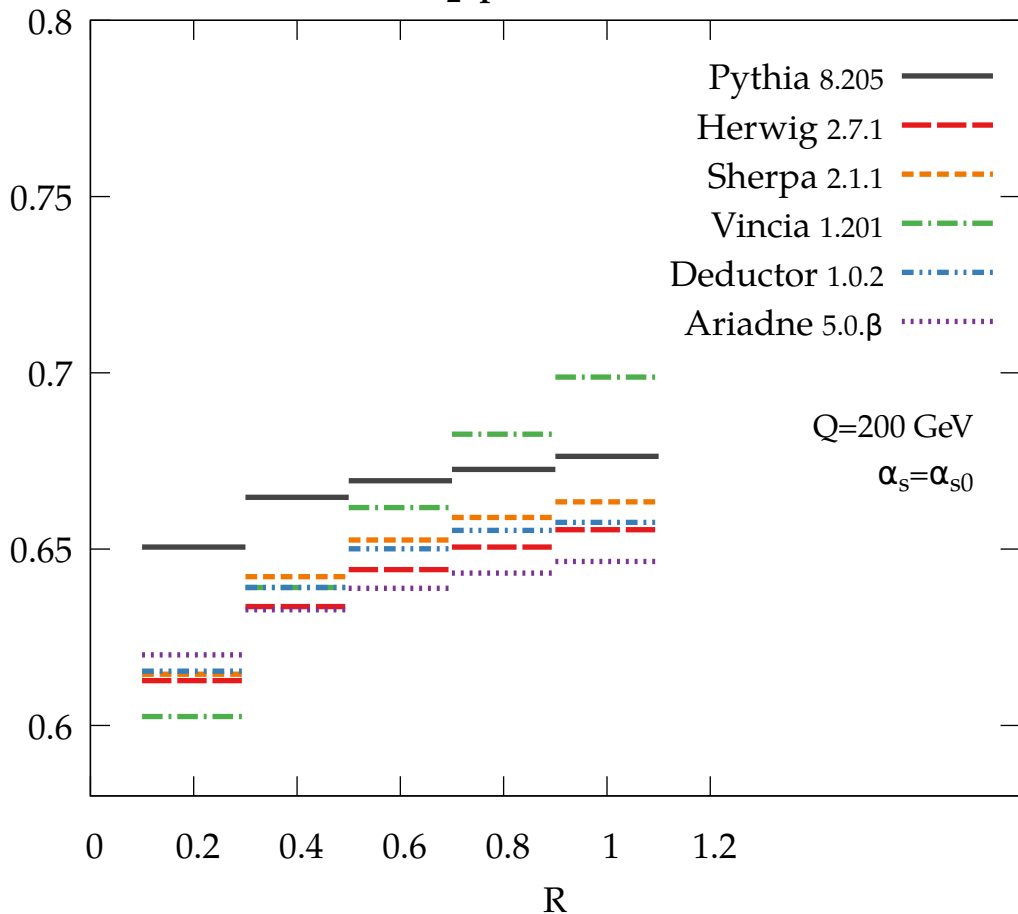

$\lambda_0^0$  [multiplicity], parton-level

Separation:  $s^{\text{rej}}$

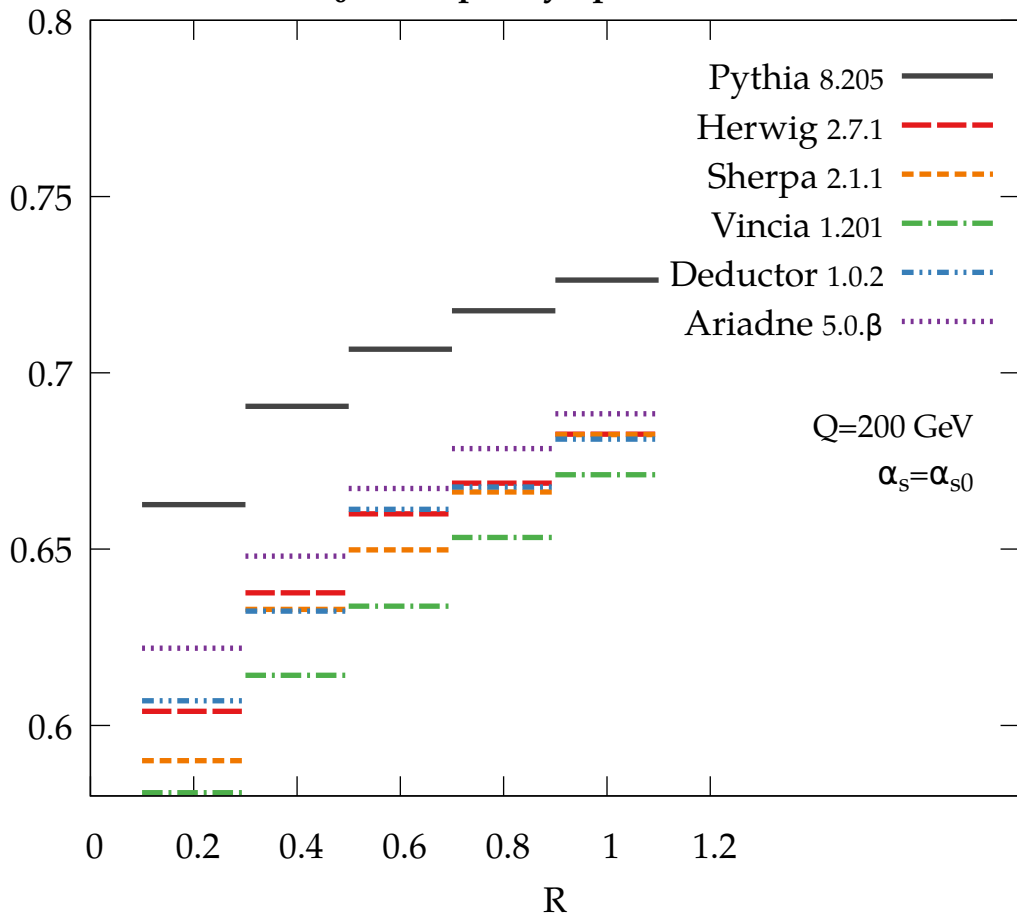

$\lambda_0^2 [(p_T^D)^2]$ , parton-level

Separation:  $s^{\text{rej}}$

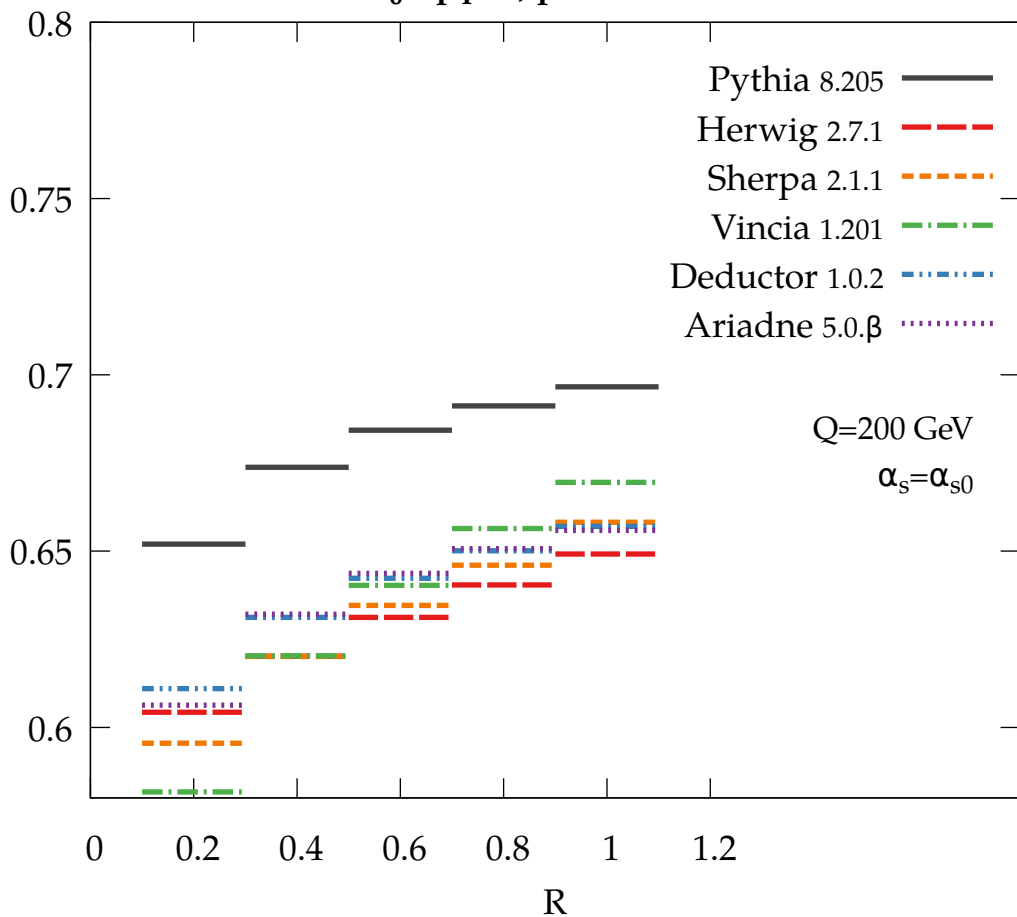

Supplement: Supplementary file 11 [file quarkgluon_fig_I2_GA_10_05_parton_Rdep.pdf]
