# Supplementary material for: Les Houches 2015: Physics at TeV Colliders Standard Model Working Group Report
Source: arXiv:1605.04692 source file (2016-05-16)

# Hadron-level

Separation:  $\Delta$

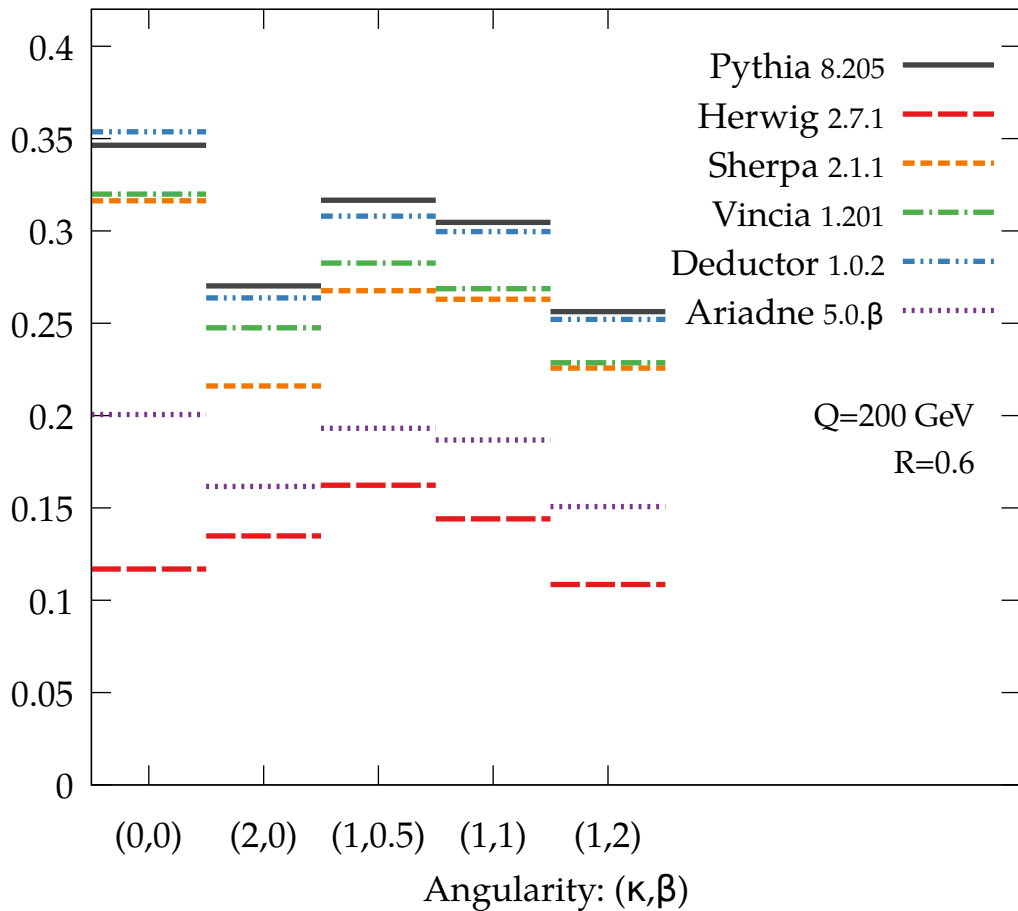

# Hadron-level

Separation:  $I_{1/2}$

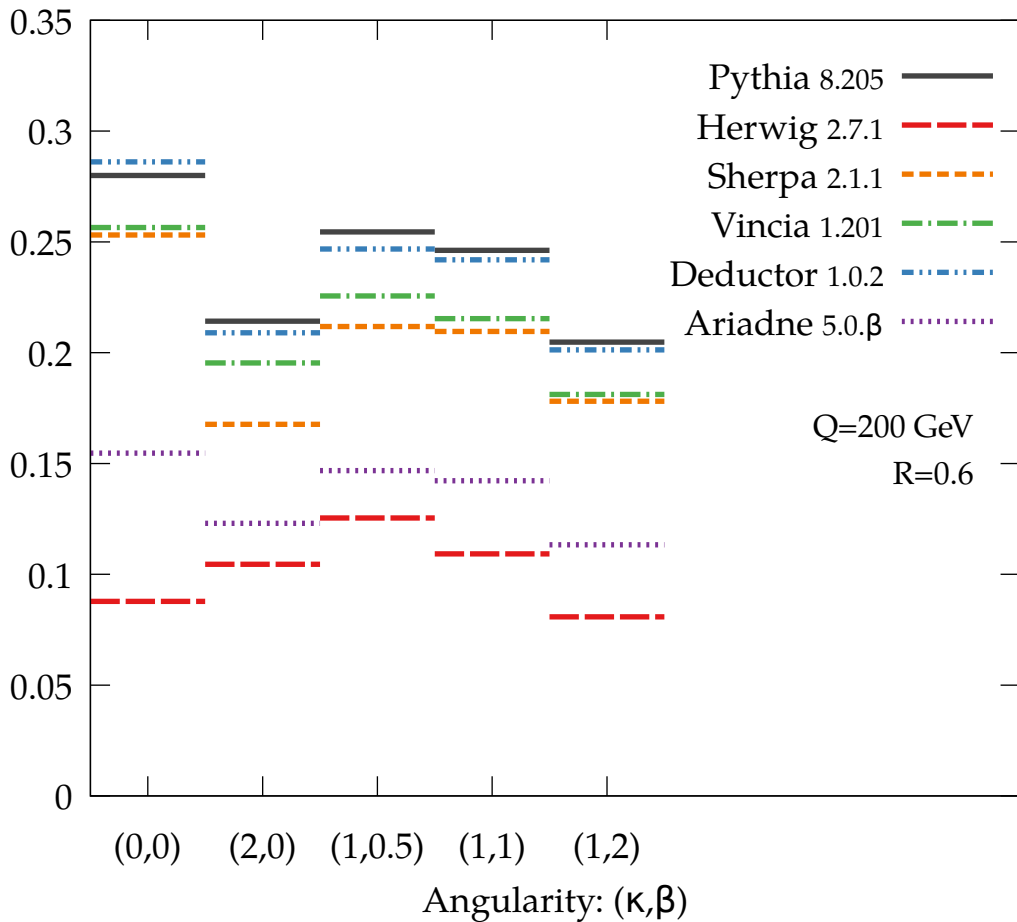

# Hadron-level

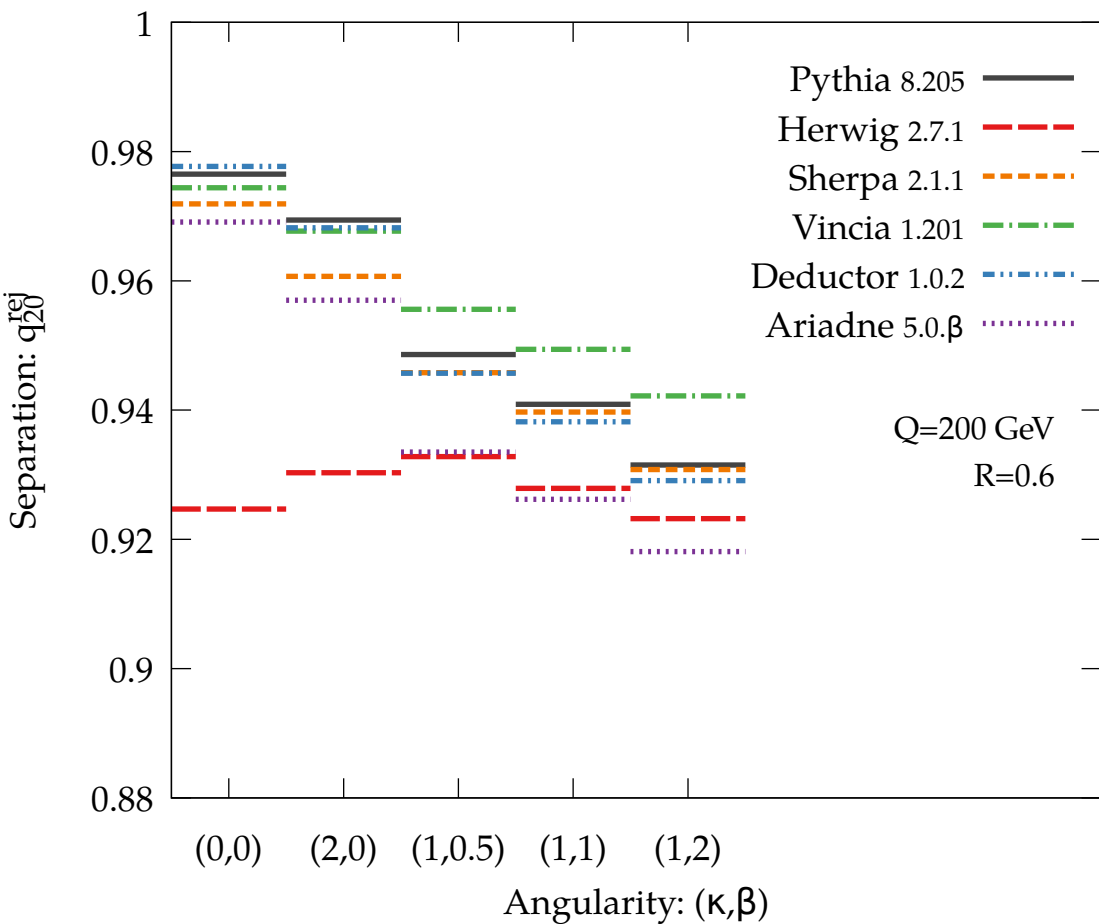

# Hadron-level

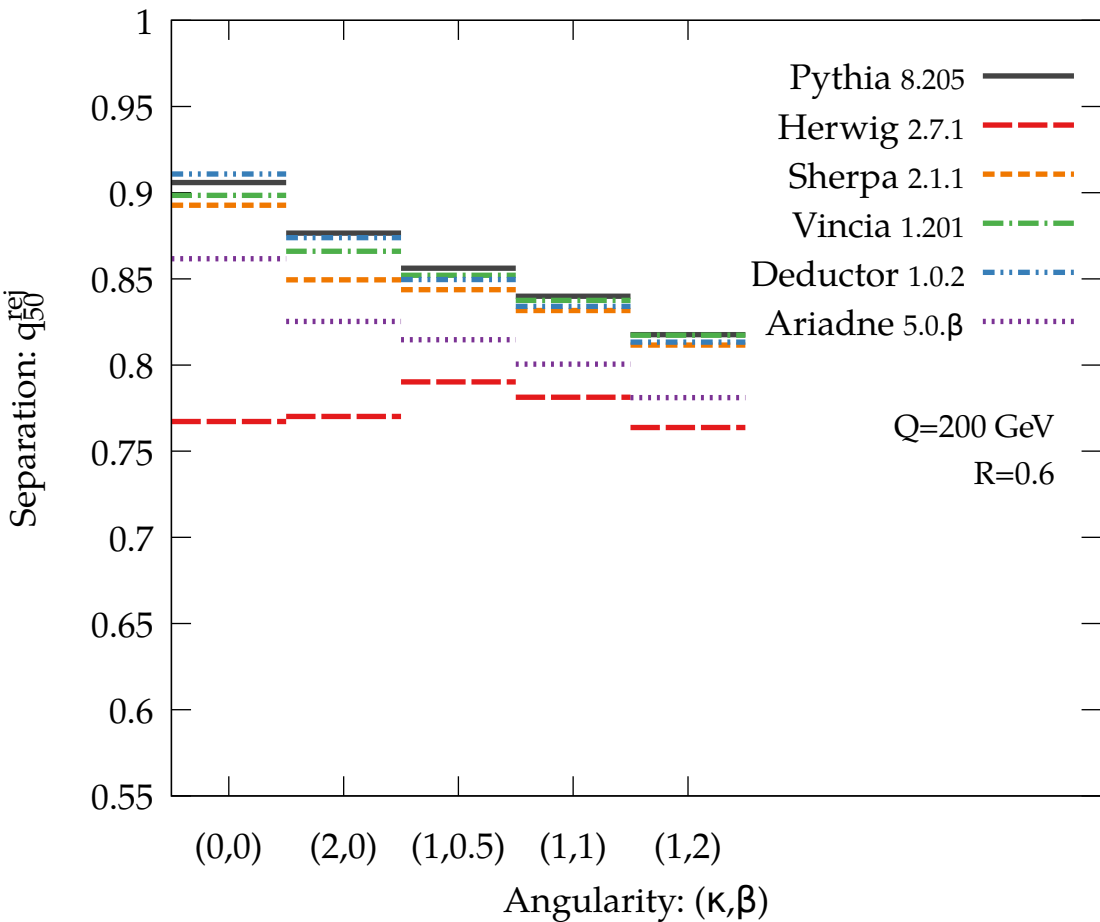

# Hadron-level

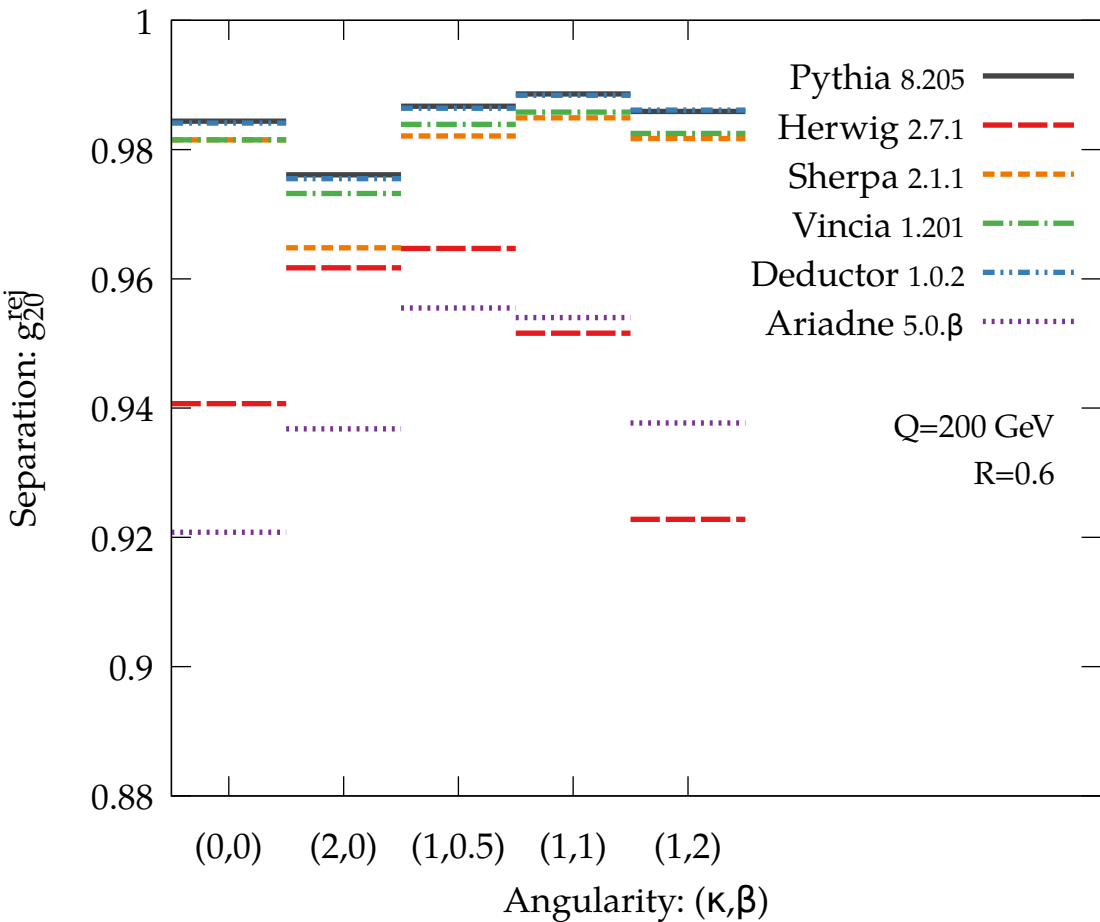

# Hadron-level

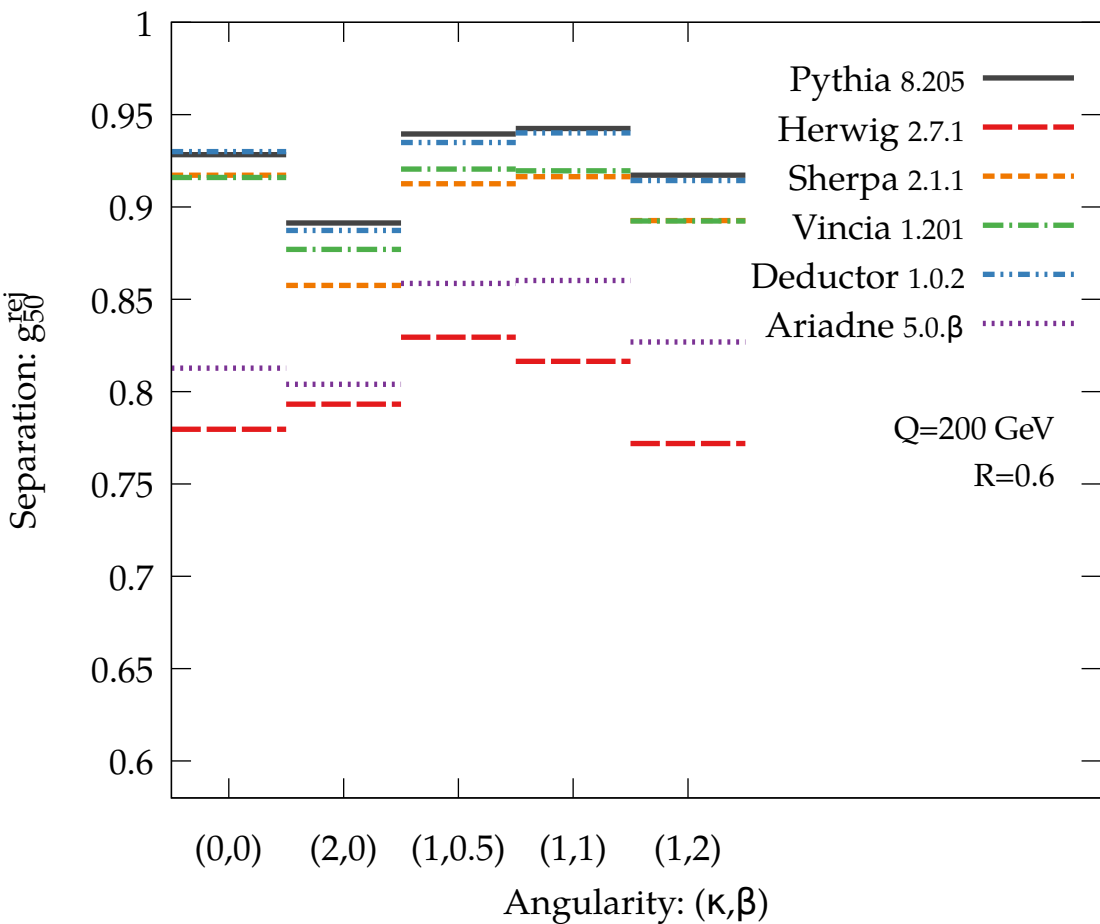

# Hadron-level

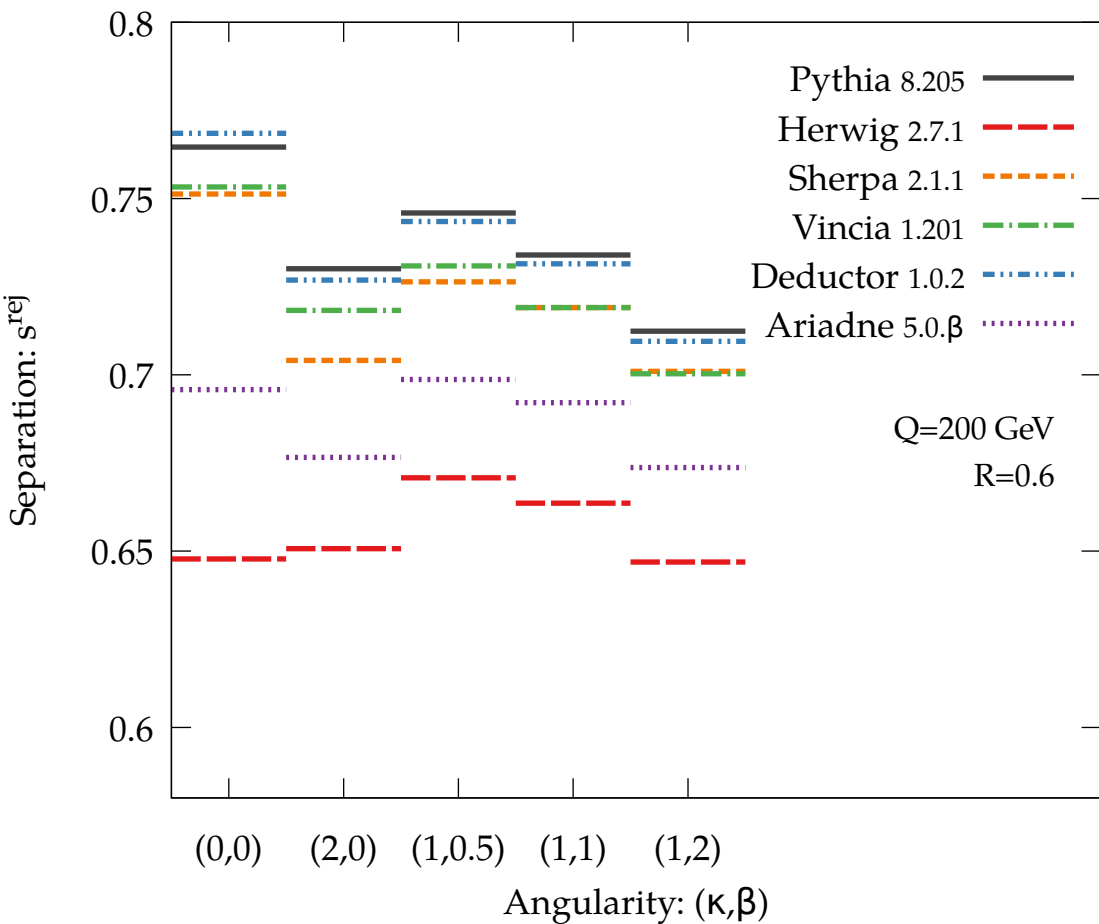

Supplement: Supplementary file 13 [file quarkgluon_fig_I2_R6_hadron__all.pdf]
