# Supplementary material for: Les Houches 2015: Physics at TeV Colliders Standard Model Working Group Report
Source: arXiv:1605.04692 source file (2016-05-16)

# Ariadne 5.0.β, hadron-level

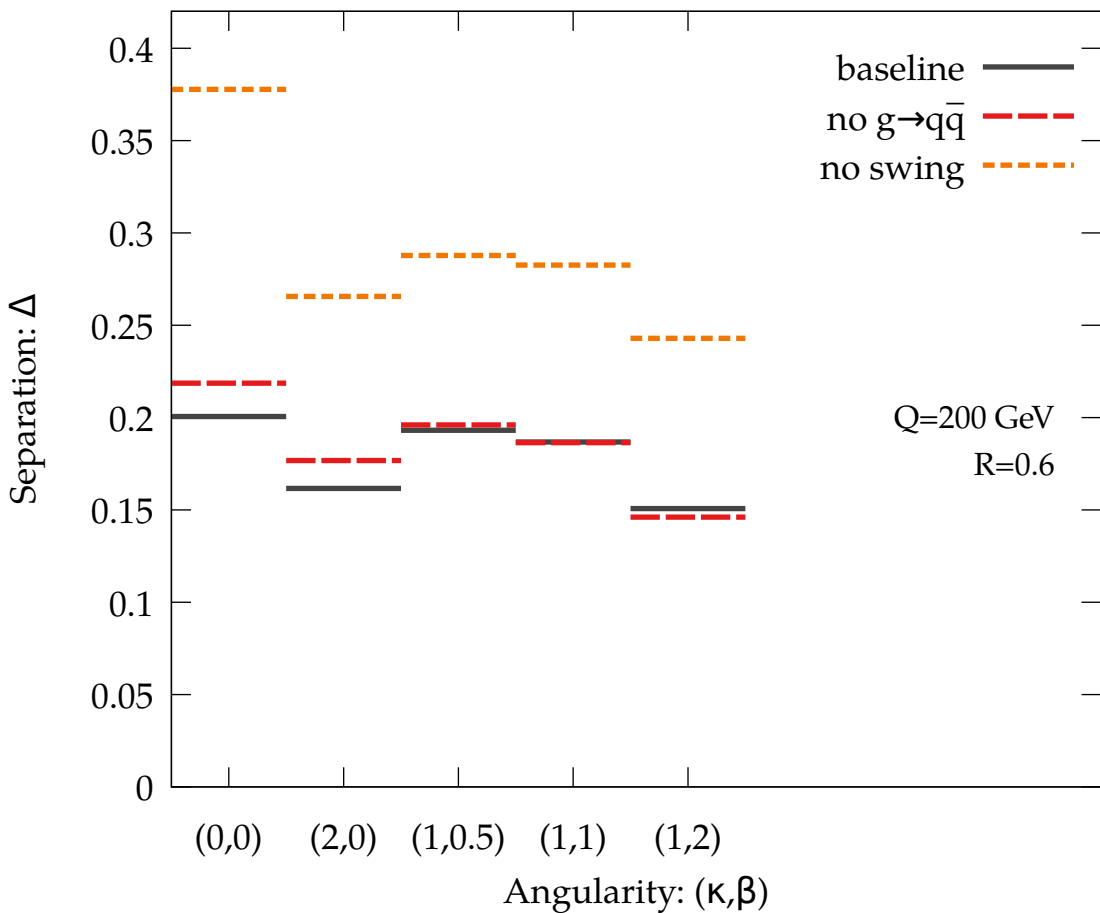

# Ariadne 5.0. $\beta$ , hadron-level

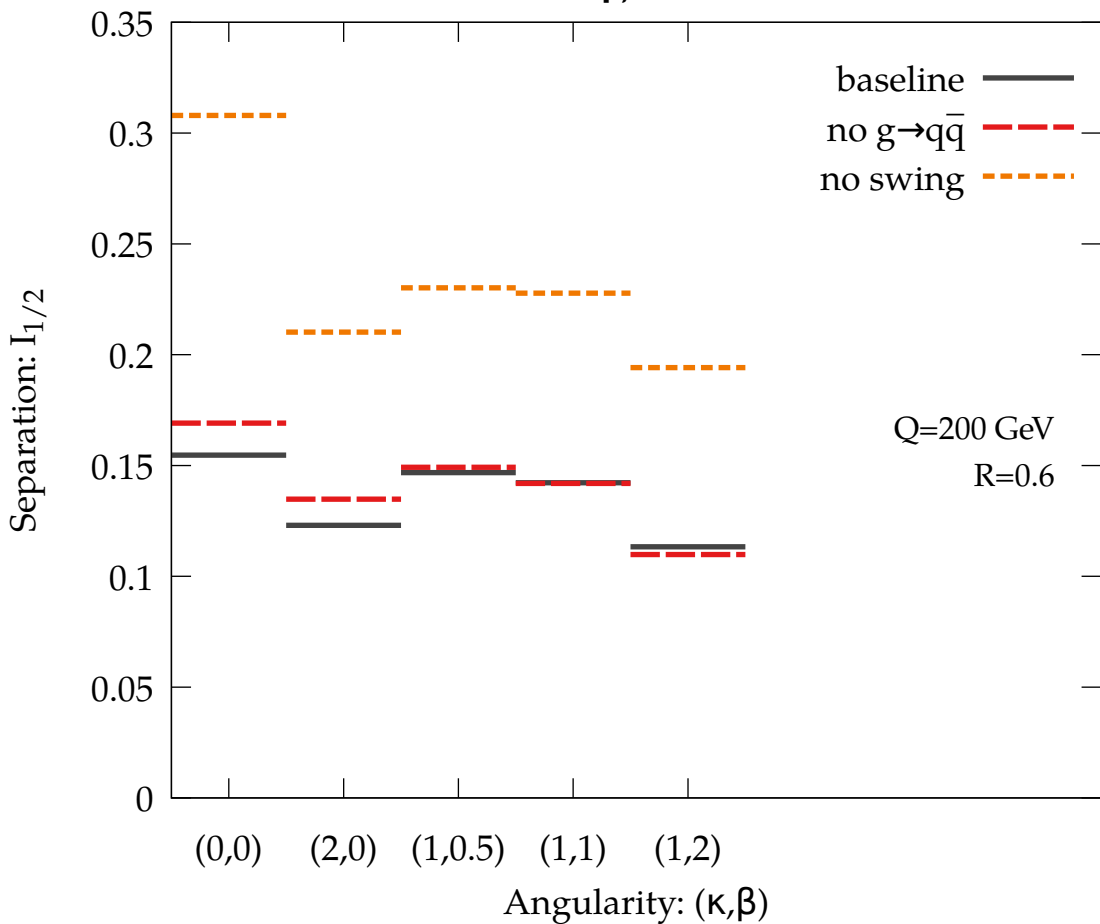

# Ariadne 5.0.β, hadron-level

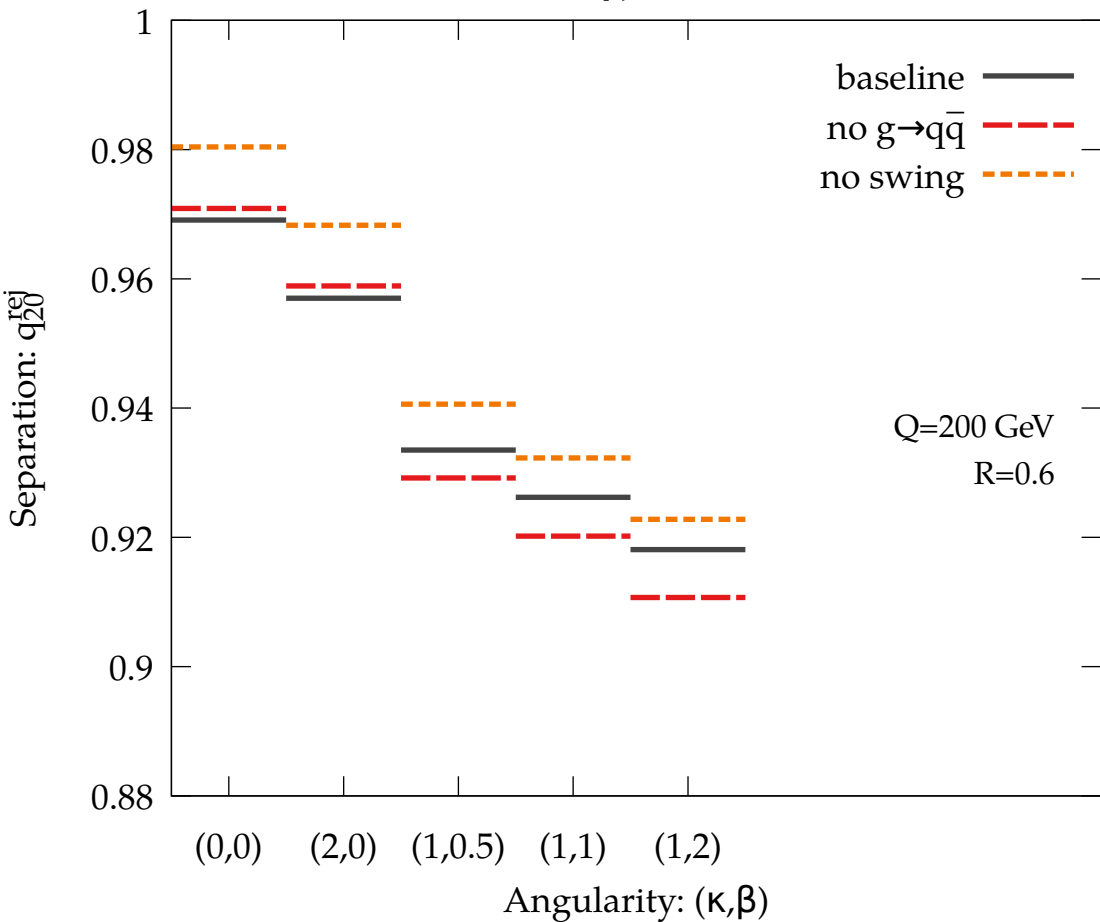

# Ariadne 5.0.β, hadron-level

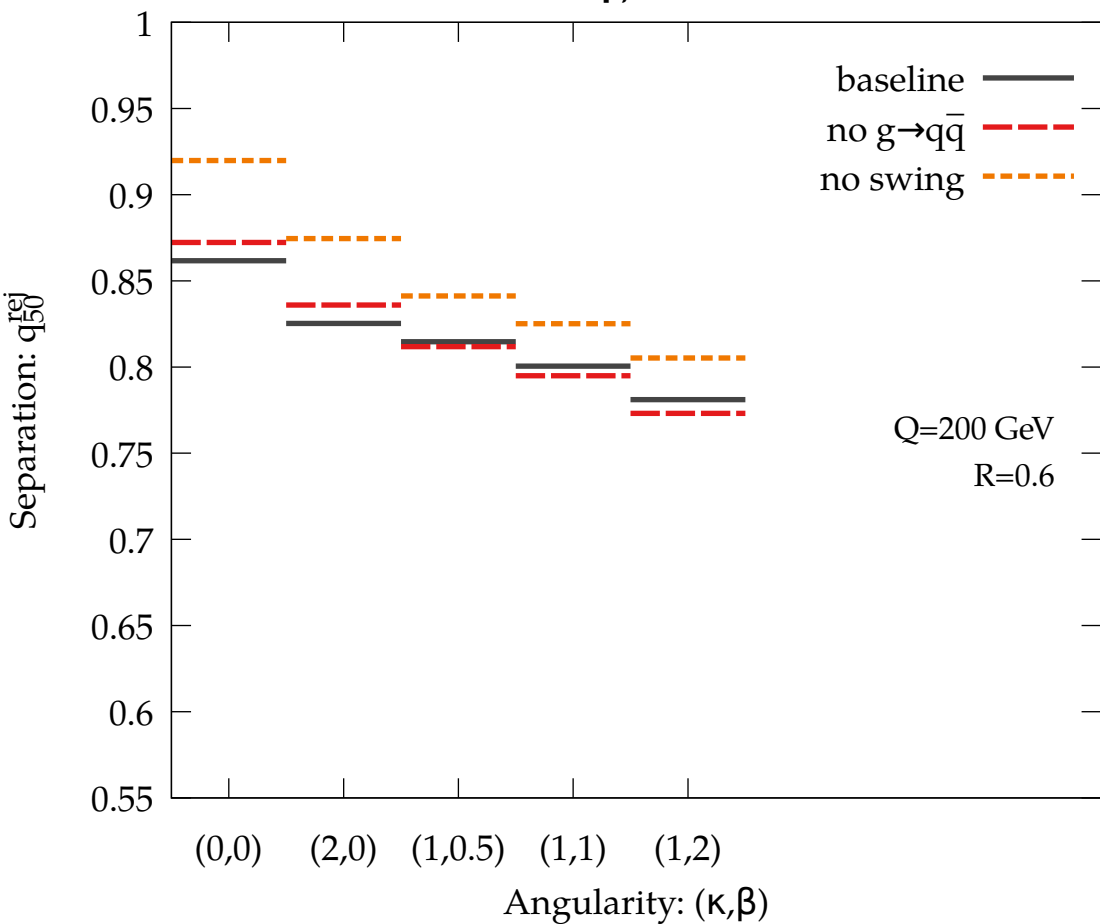

# Ariadne 5.0.β, hadron-level

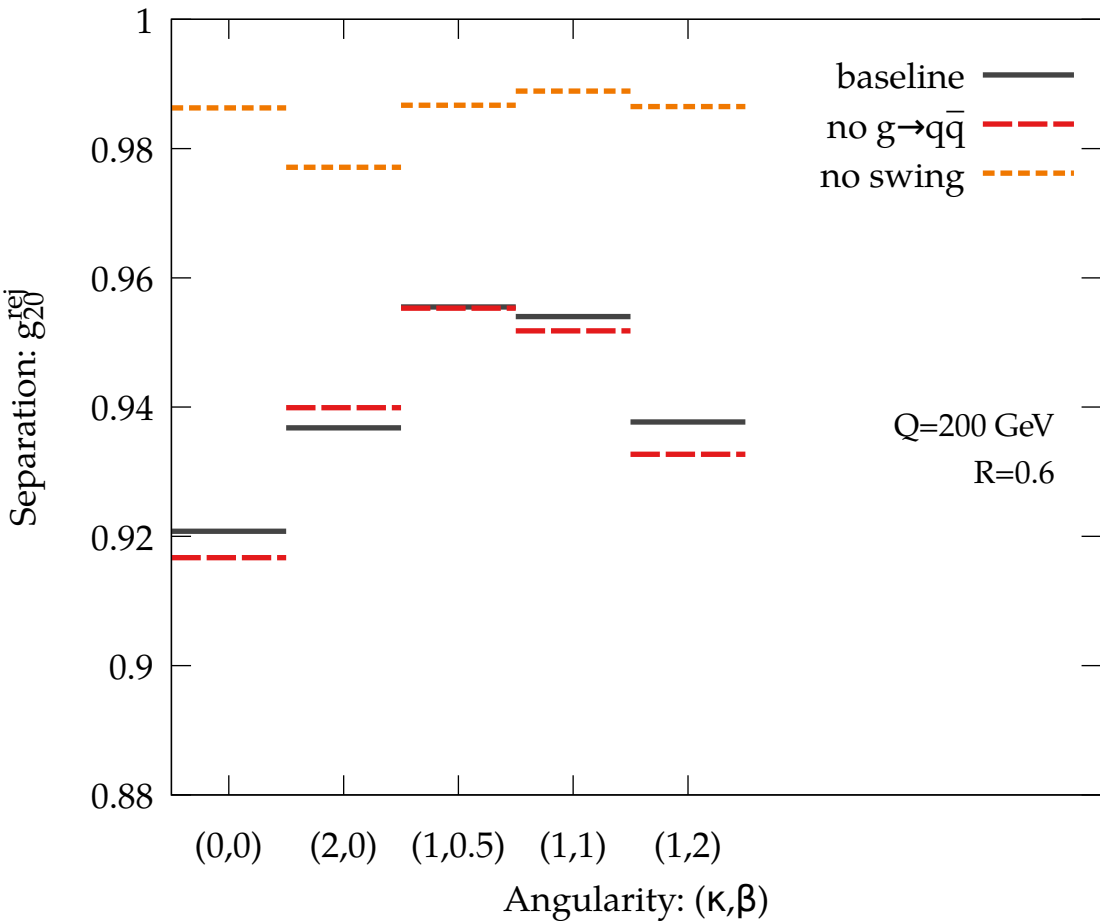

# Ariadne 5.0.β, hadron-level

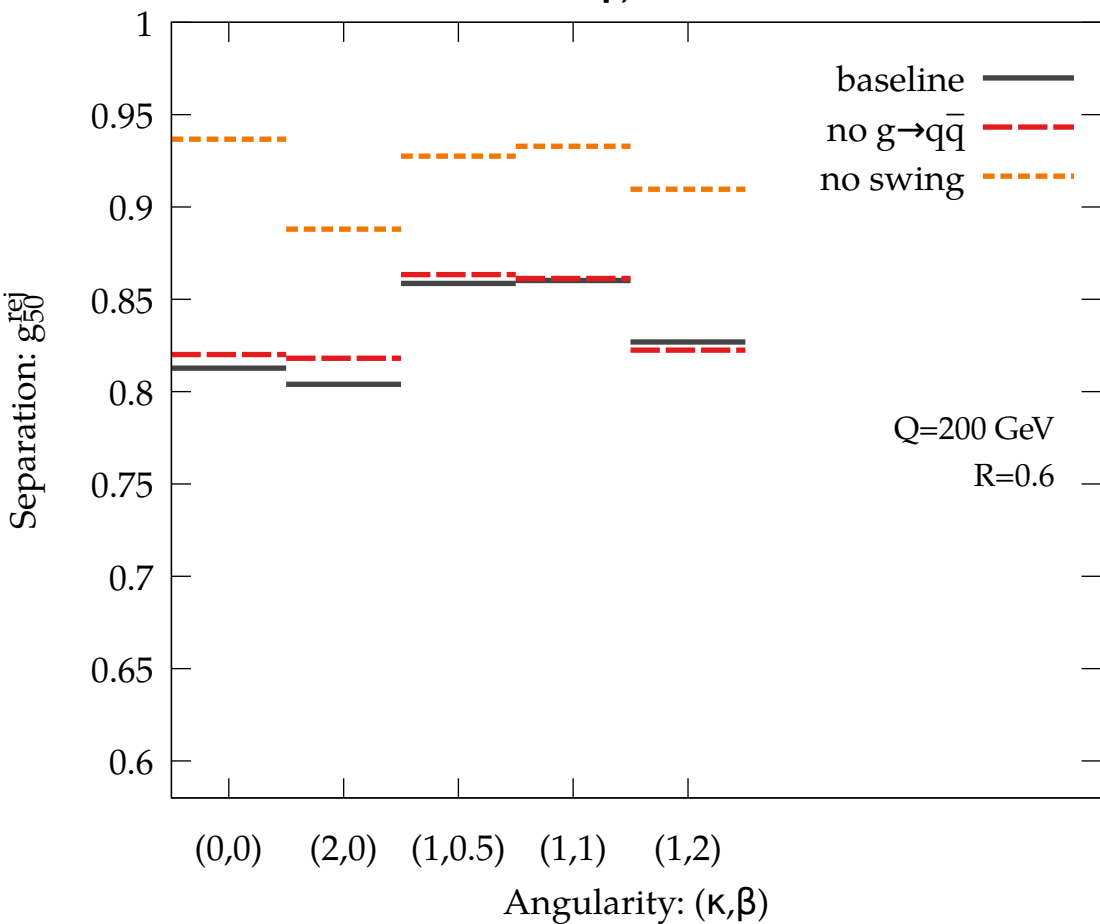

# Ariadne 5.0.β, hadron-level

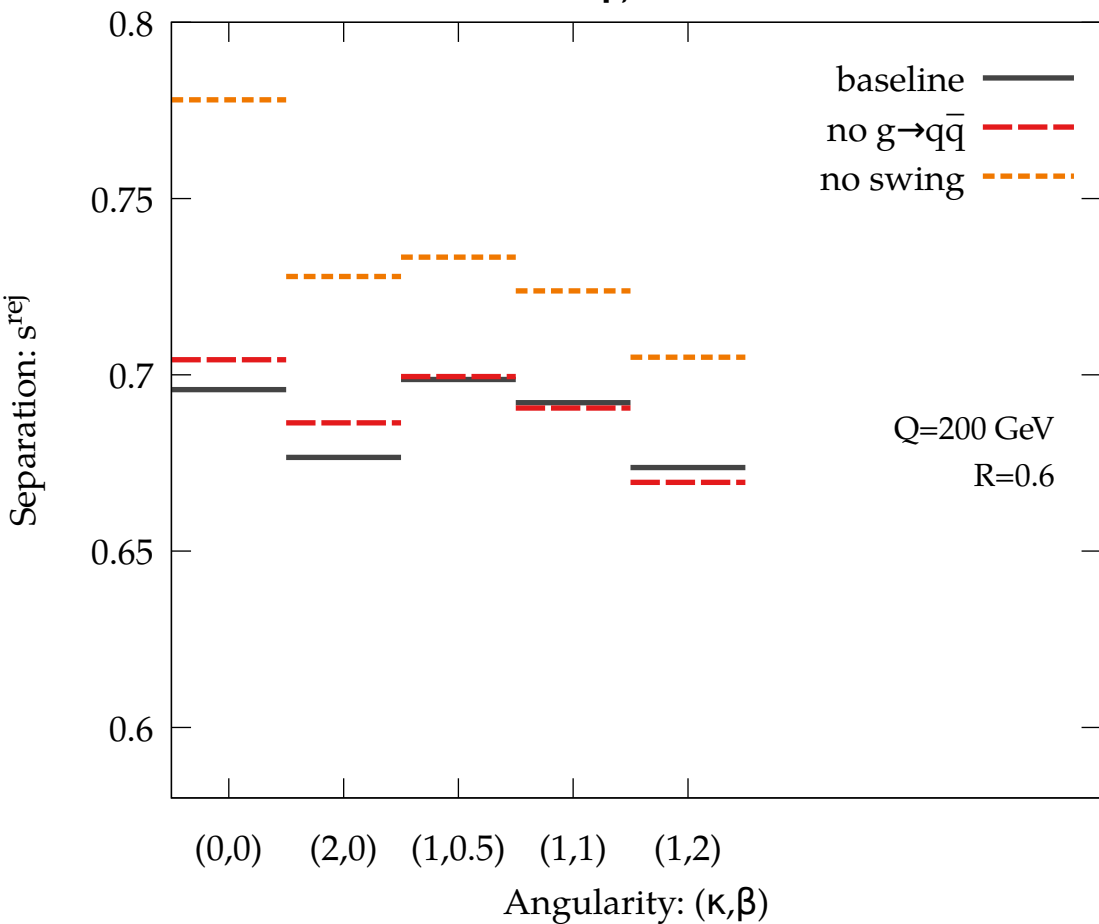

Supplement: Supplementary file 14 [file quarkgluon_fig_I2_R6_hadron_ariadne.pdf]
