# Supplementary material for: Les Houches 2015: Physics at TeV Colliders Standard Model Working Group Report
Source: arXiv:1605.04692 source file (2016-05-16)

# Pythia 8.205, hadron-level

Separation:  $\Delta$

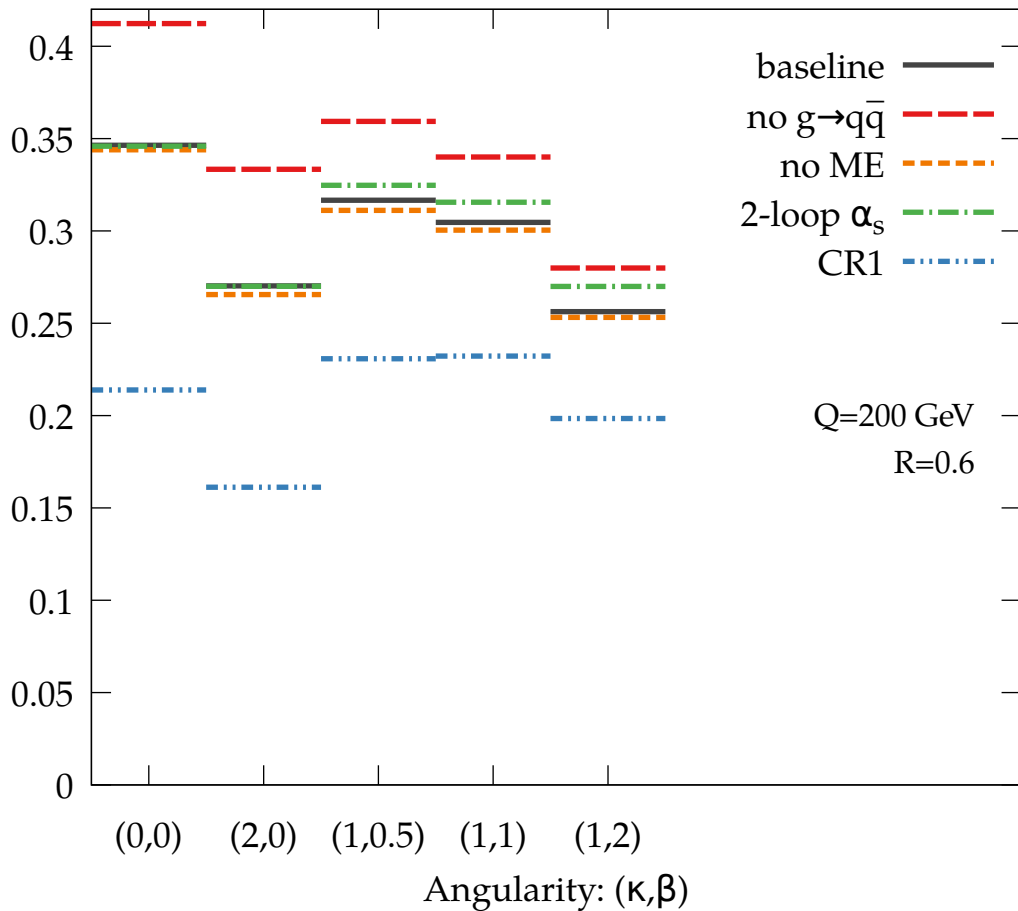

# Pythia 8.205, hadron-level

Separation:  $I_{1/2}$

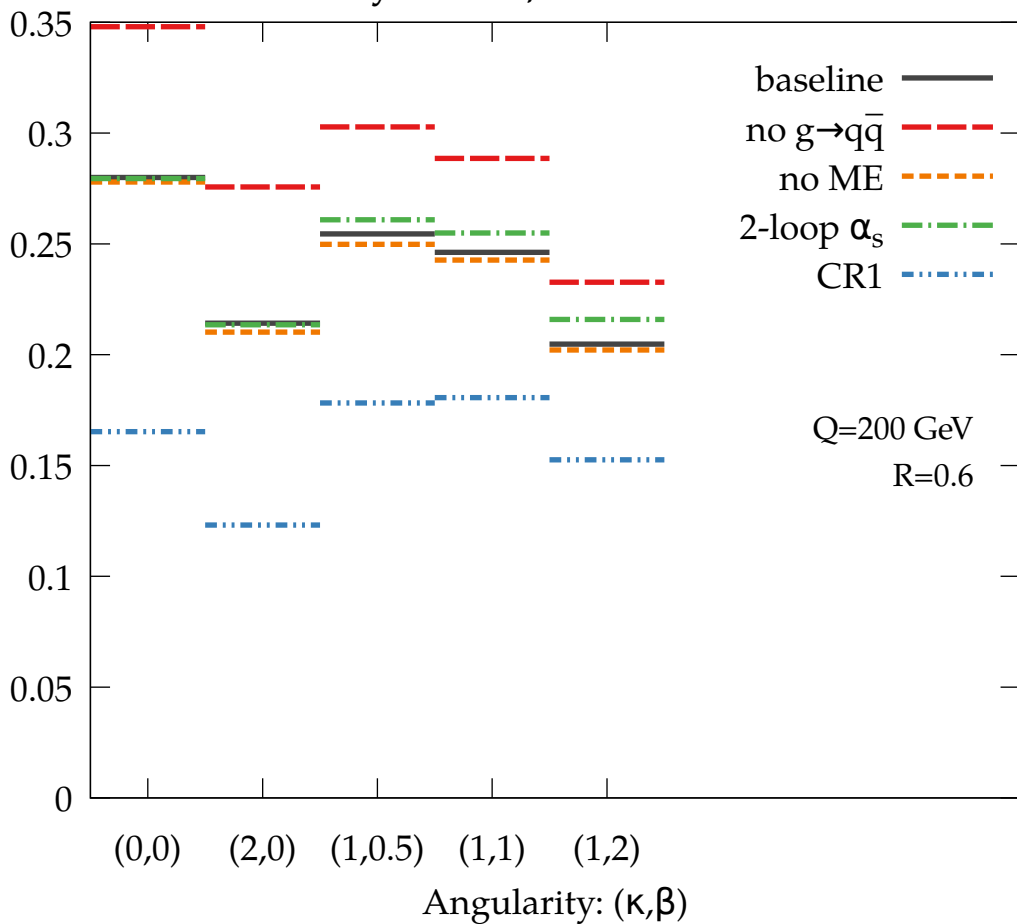

# Pythia 8.205, hadron-level

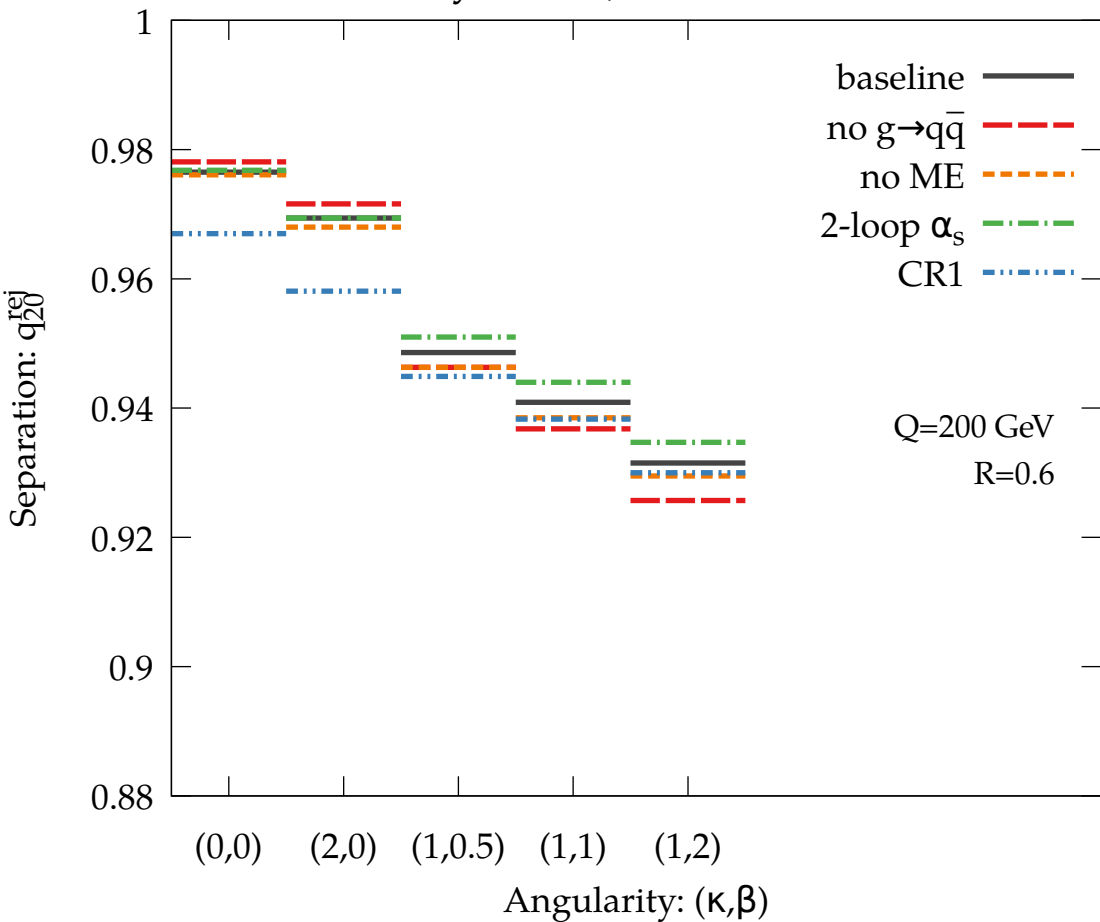

# Pythia 8.205, hadron-level

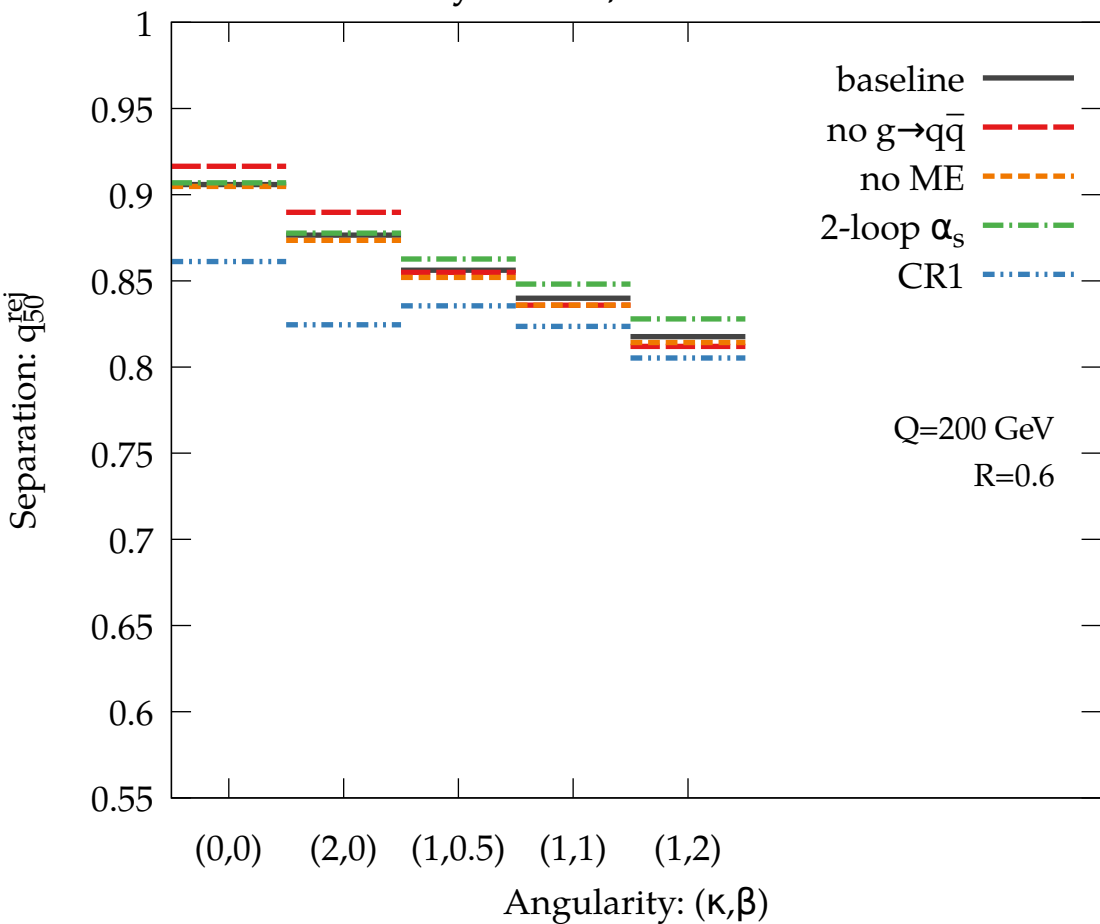

# Pythia 8.205, hadron-level

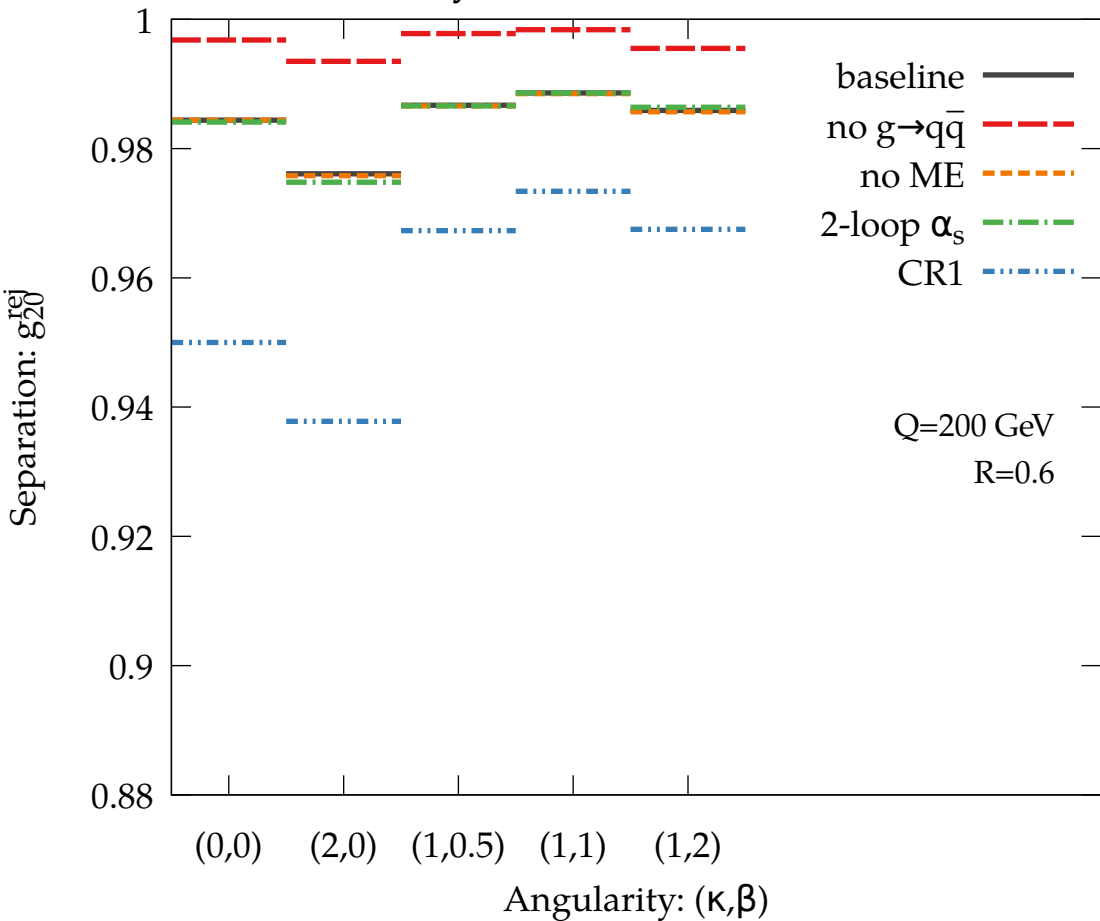

# Pythia 8.205, hadron-level

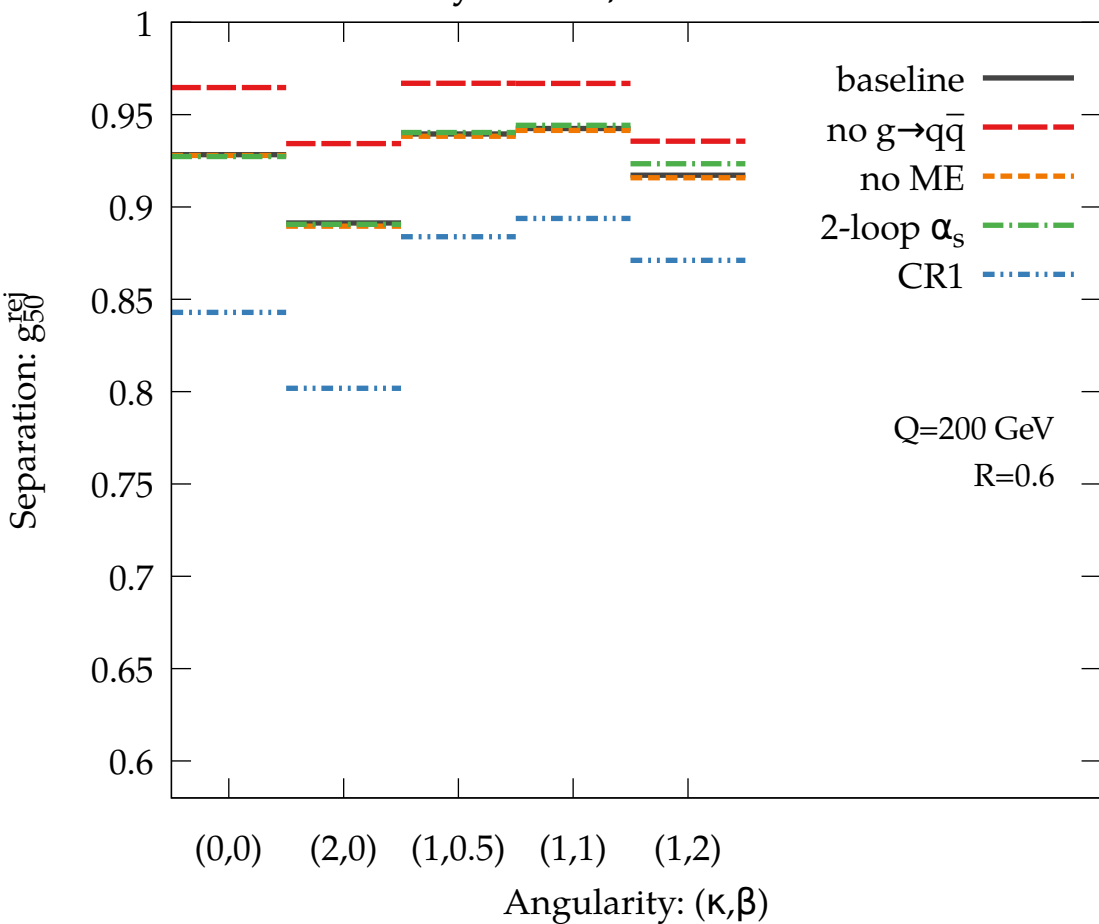

# Pythia 8.205, hadron-level

Separation:  $s^{\text{rej}}$

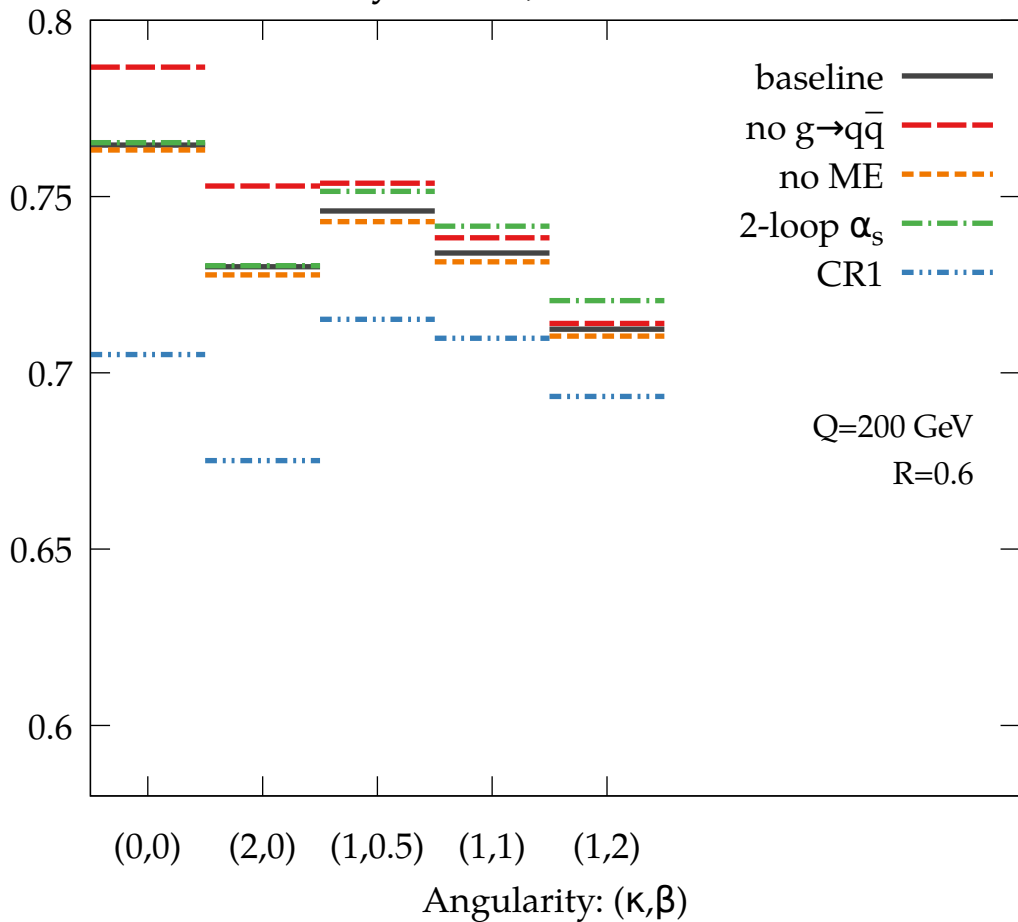

Supplement: Supplementary file 16 [file quarkgluon_fig_I2_R6_hadron_pythia.pdf]
