# Supplementary material for: Les Houches 2015: Physics at TeV Colliders Standard Model Working Group Report
Source: arXiv:1605.04692 source file (2016-05-16)

# Parton-level

Separation:  $\Delta$

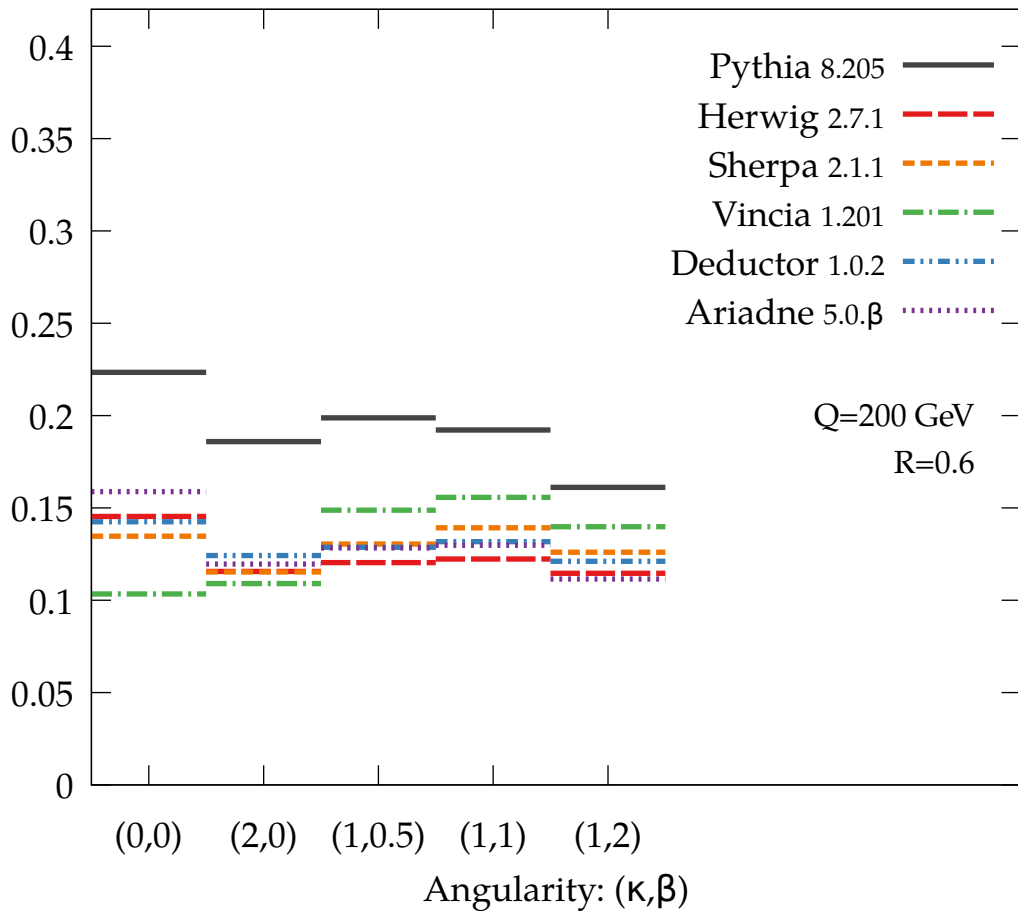

# Parton-level

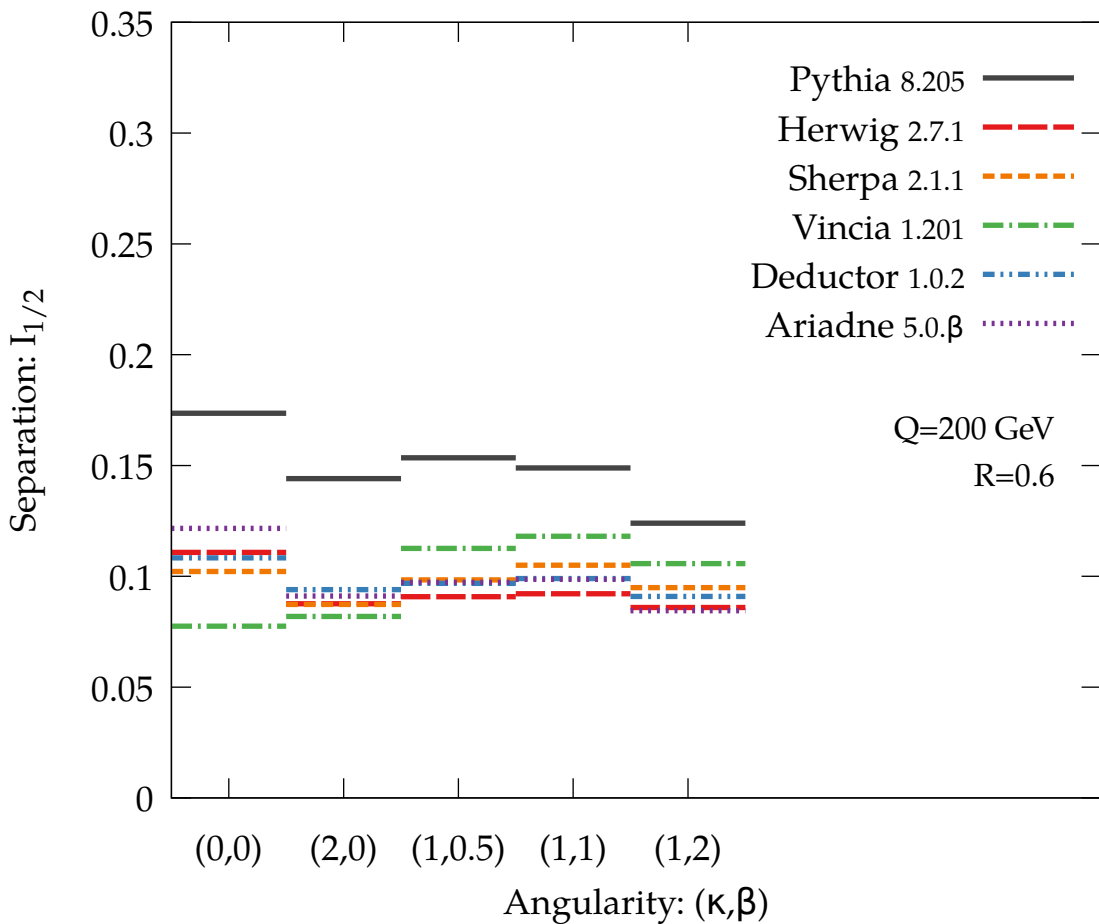

# Parton-level

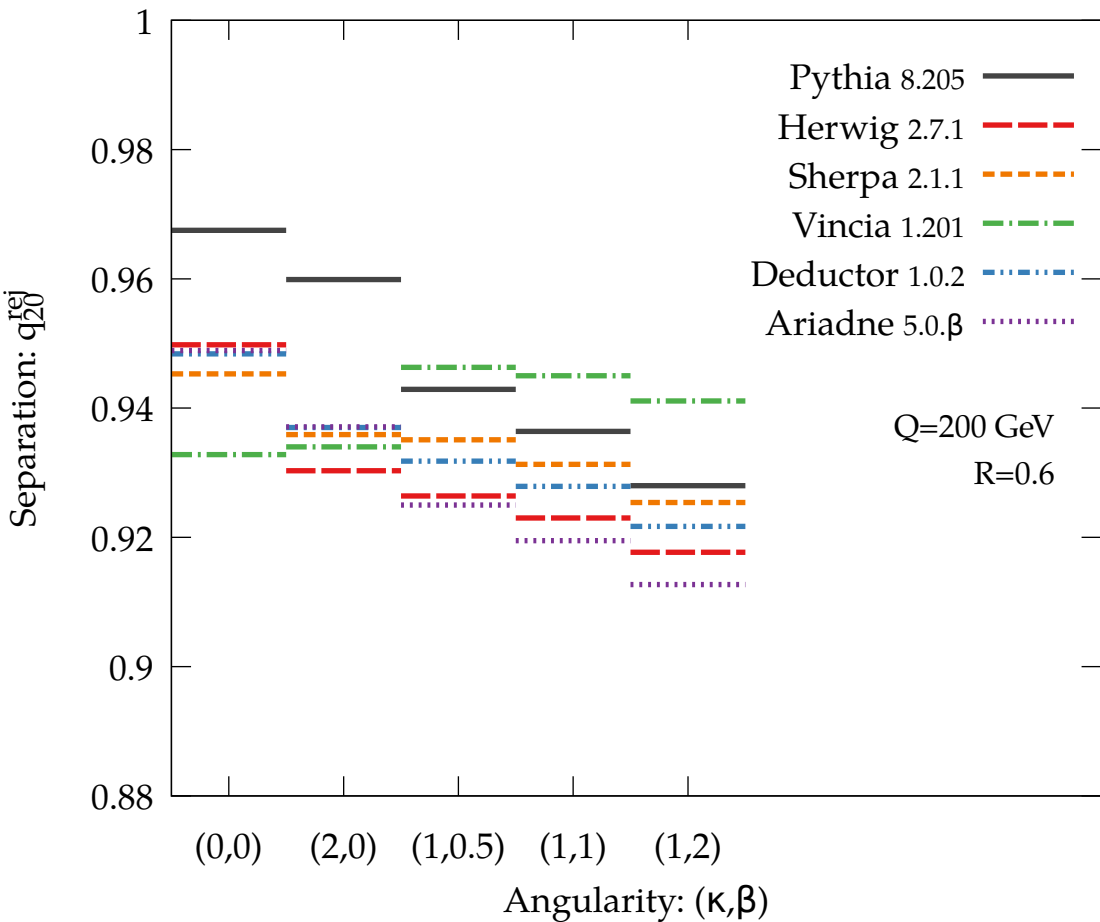

# Parton-level

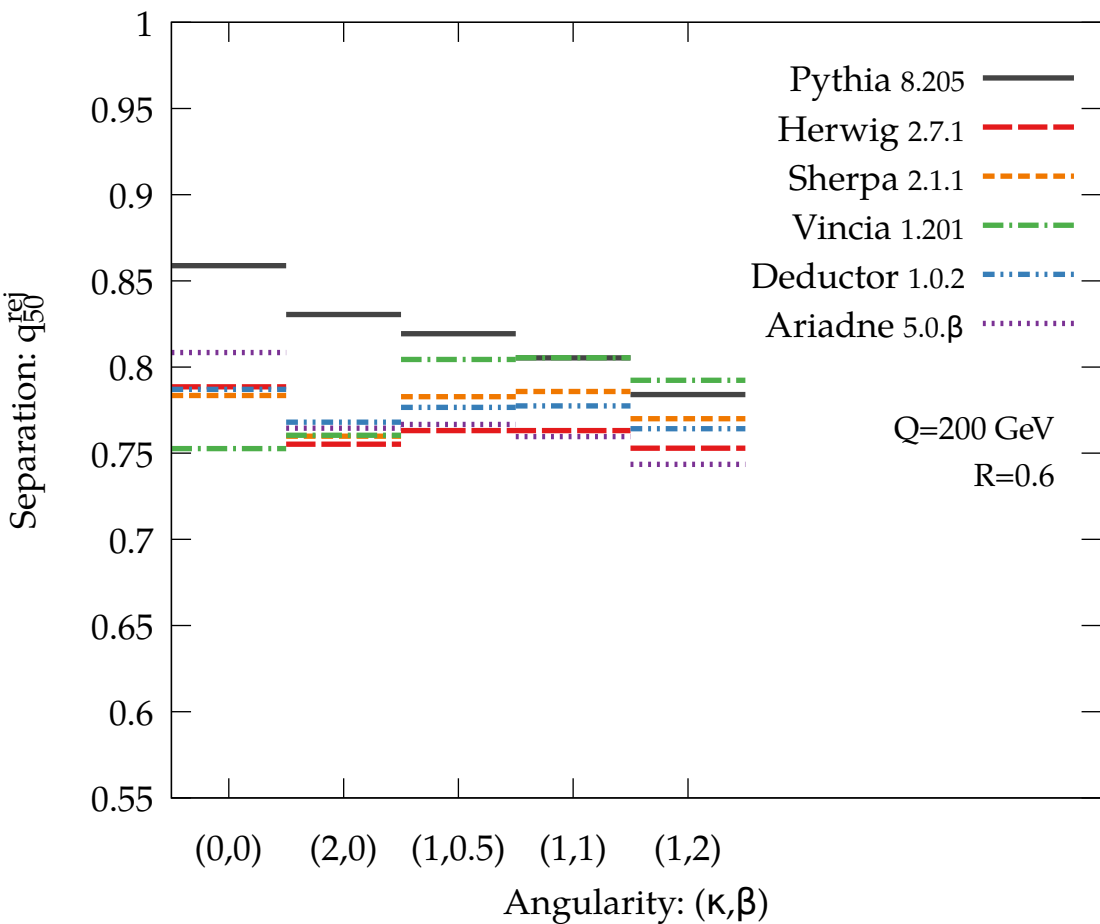

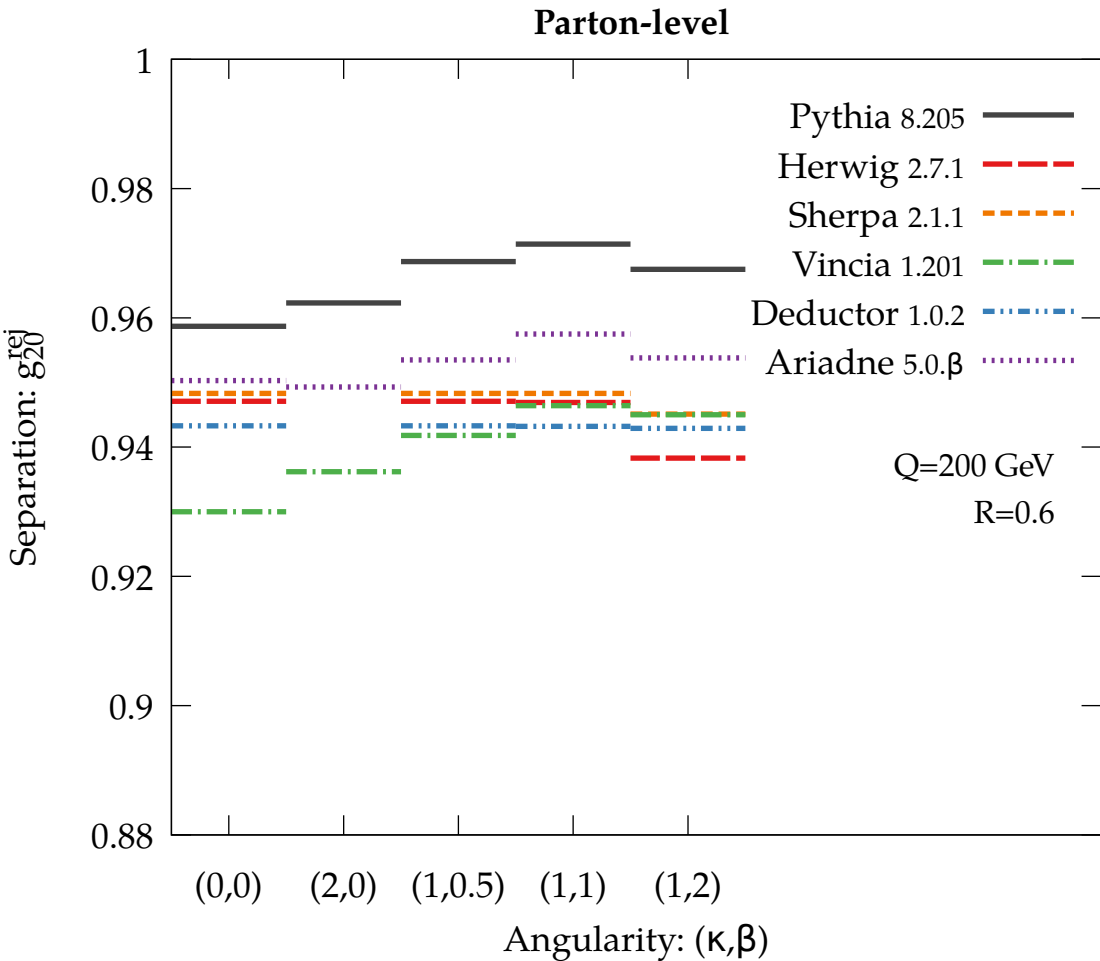

# Parton-level

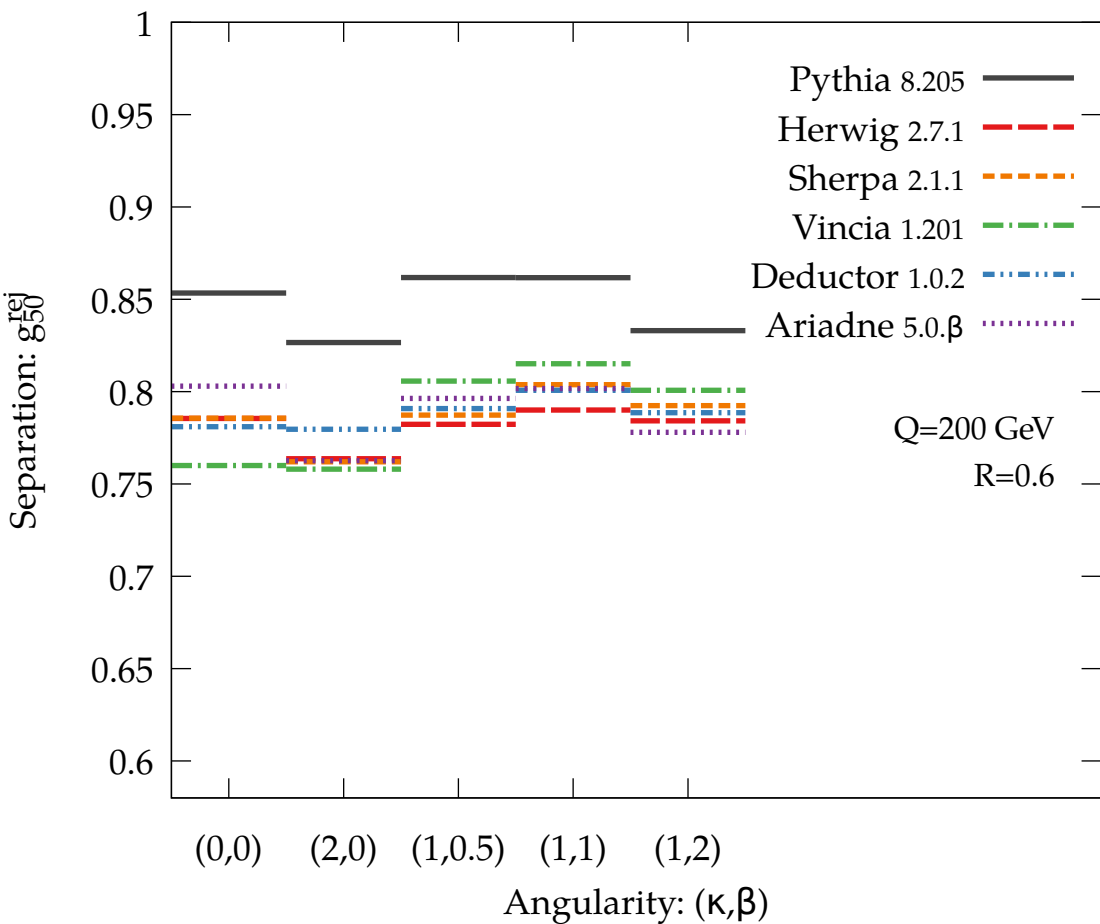

# Parton-level

Separation:  $s^{\text{rej}}$

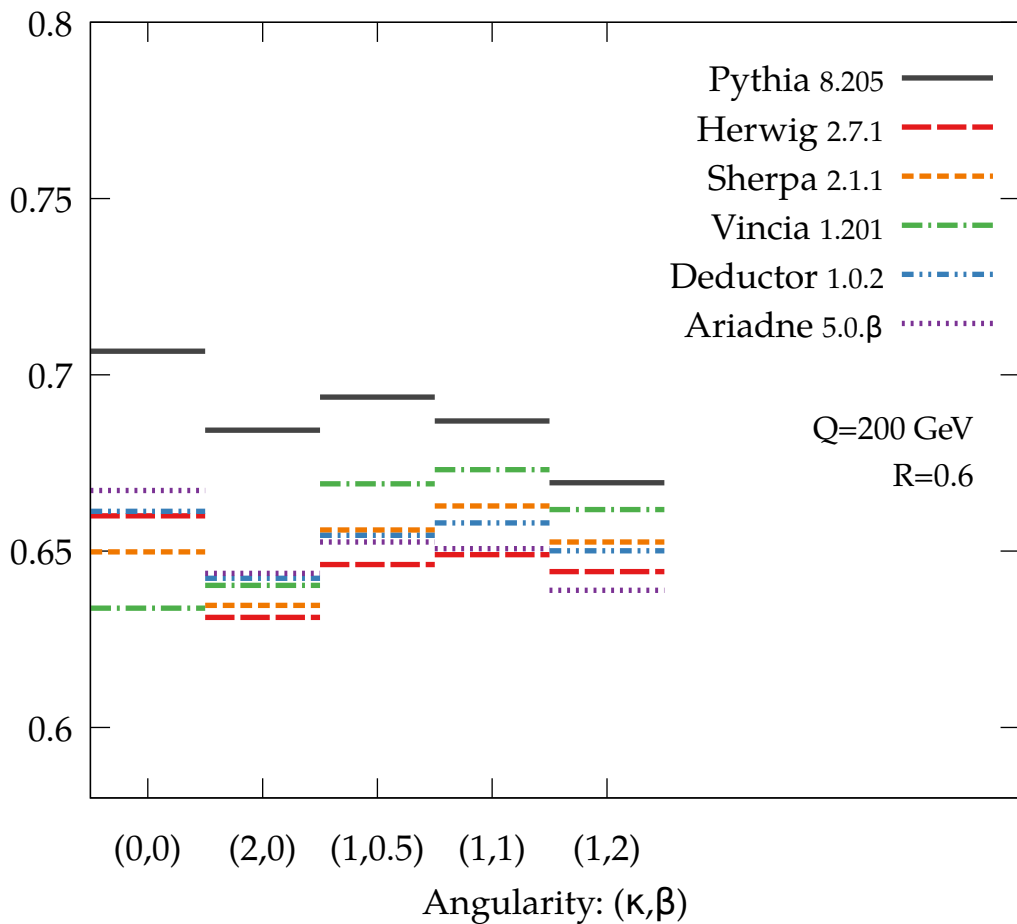

Supplement: Supplementary file 19 [file quarkgluon_fig_I2_R6_parton__all.pdf]
