# Supplementary material for: Les Houches 2015: Physics at TeV Colliders Standard Model Working Group Report
Source: arXiv:1605.04692 source file (2016-05-16)

# Ariadne 5.0.β, parton-level

Separation:  $\Delta$

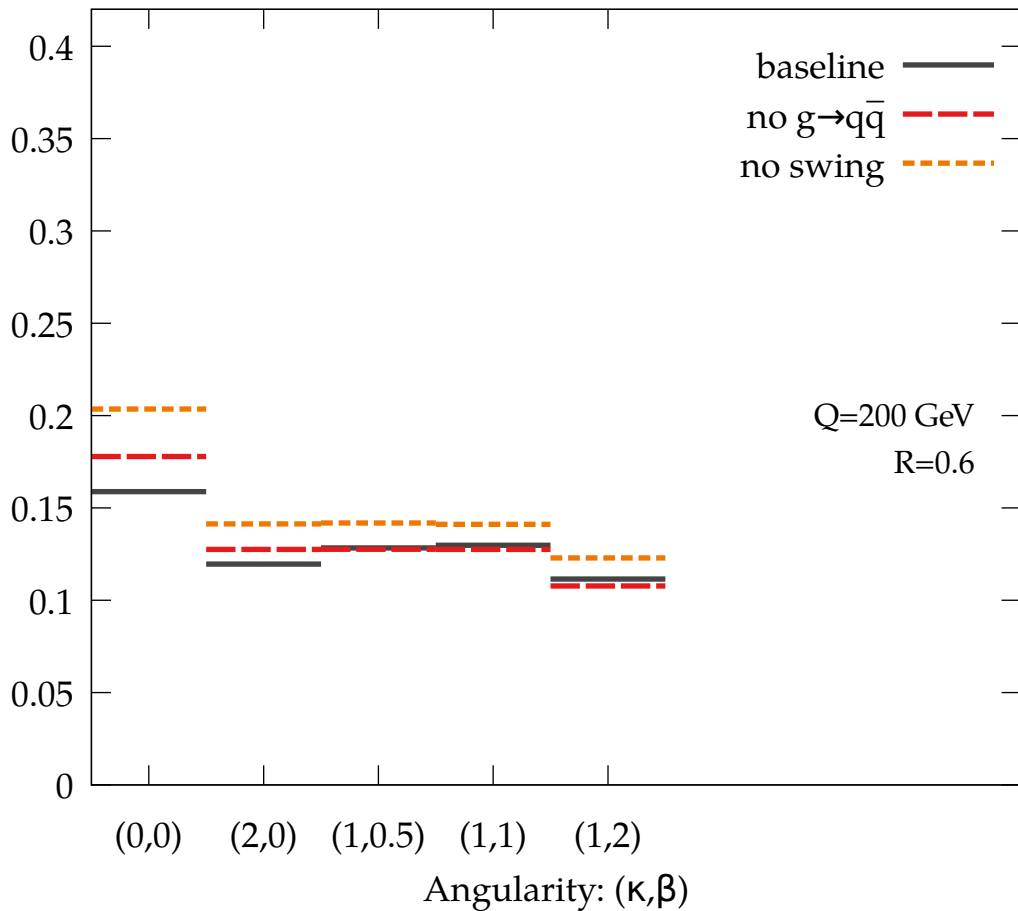

# Ariadne 5.0.β, parton-level

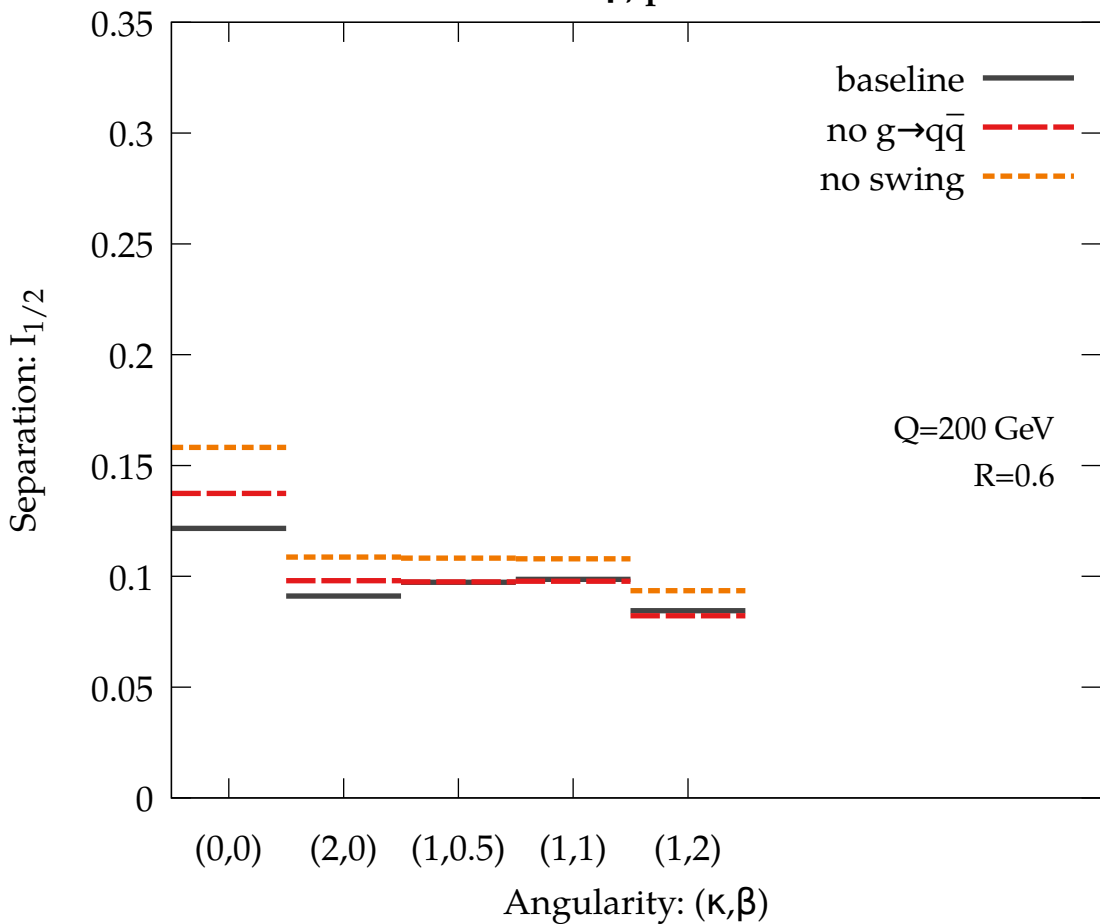

# Ariadne 5.0.β, parton-level

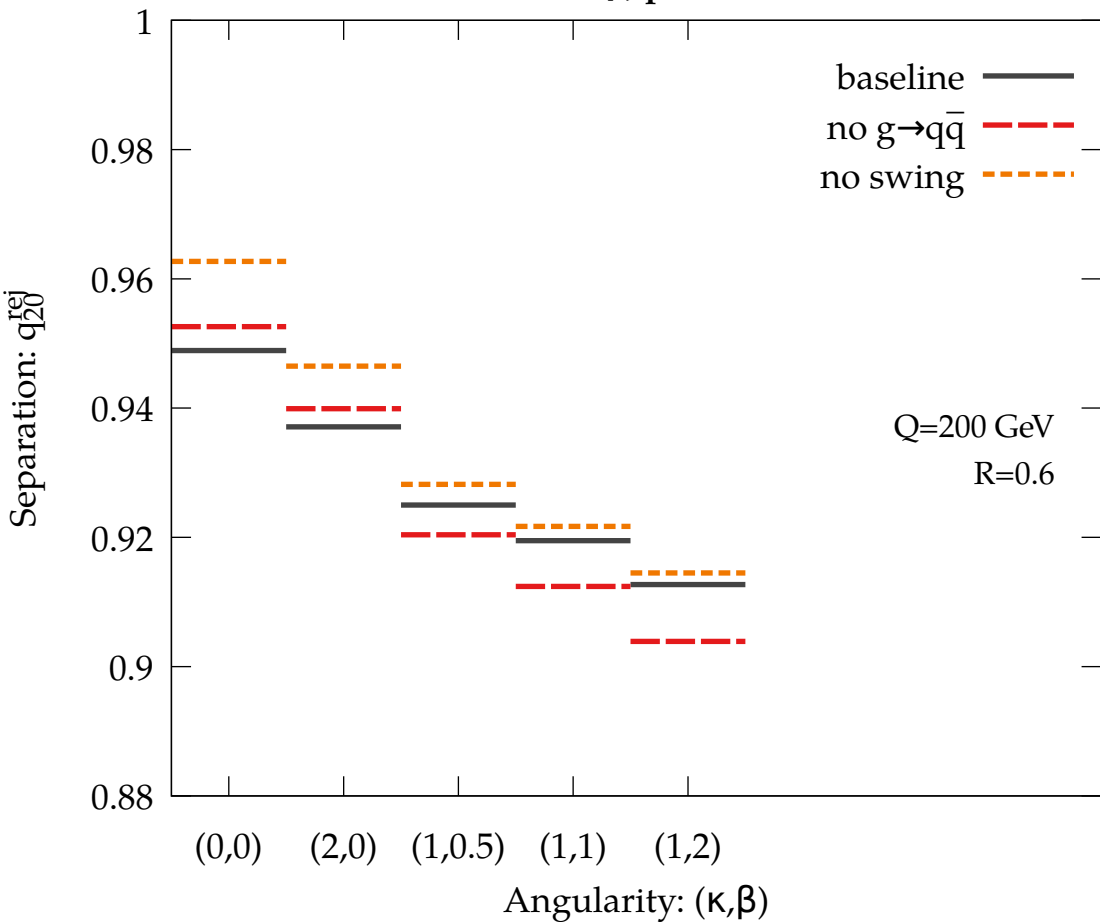

# Ariadne 5.0.β, parton-level

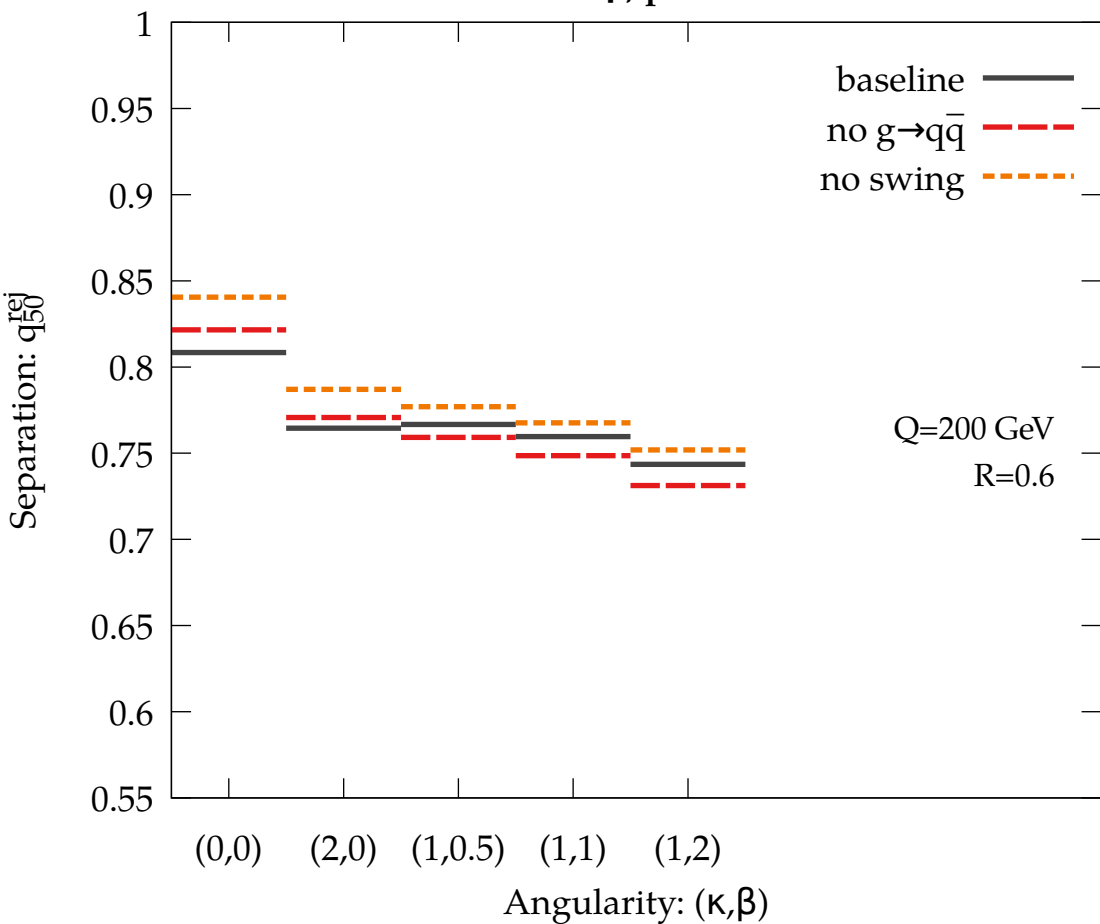

# Ariadne 5.0.β, parton-level

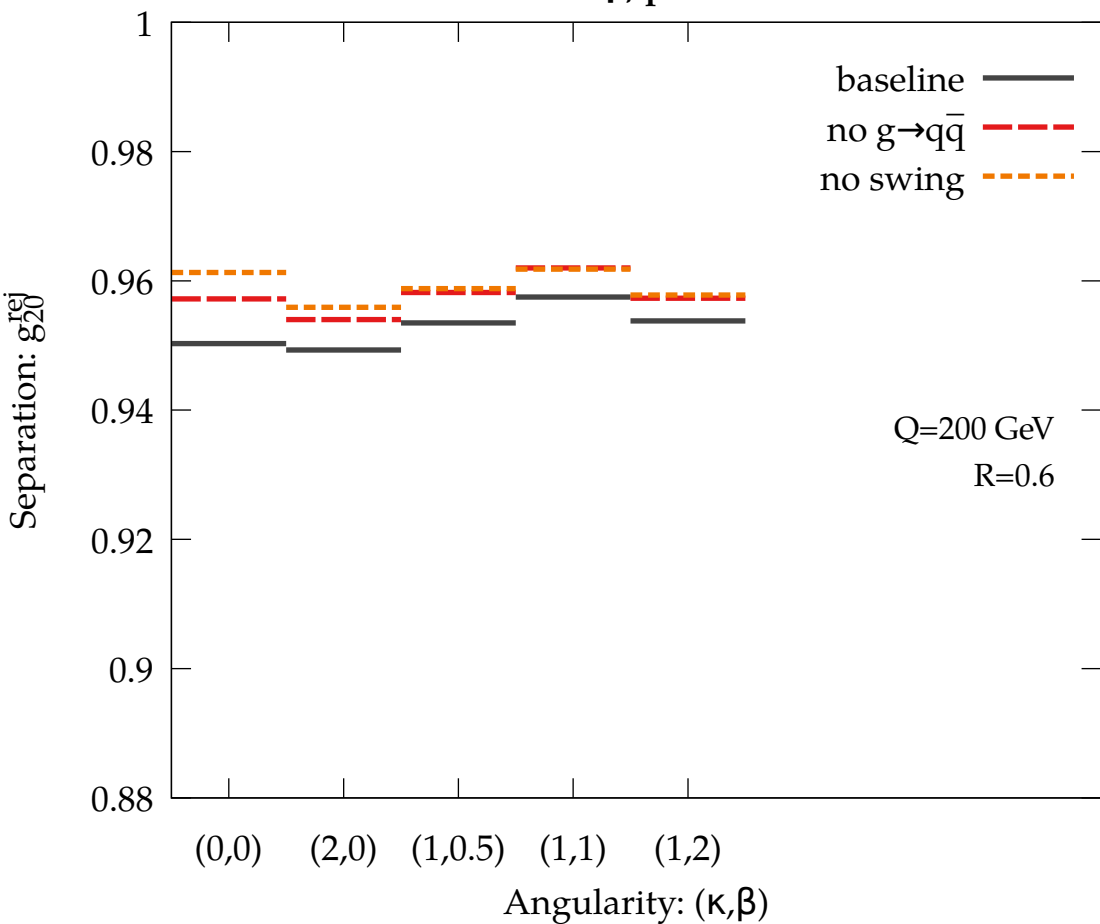

# Ariadne 5.0.β, parton-level

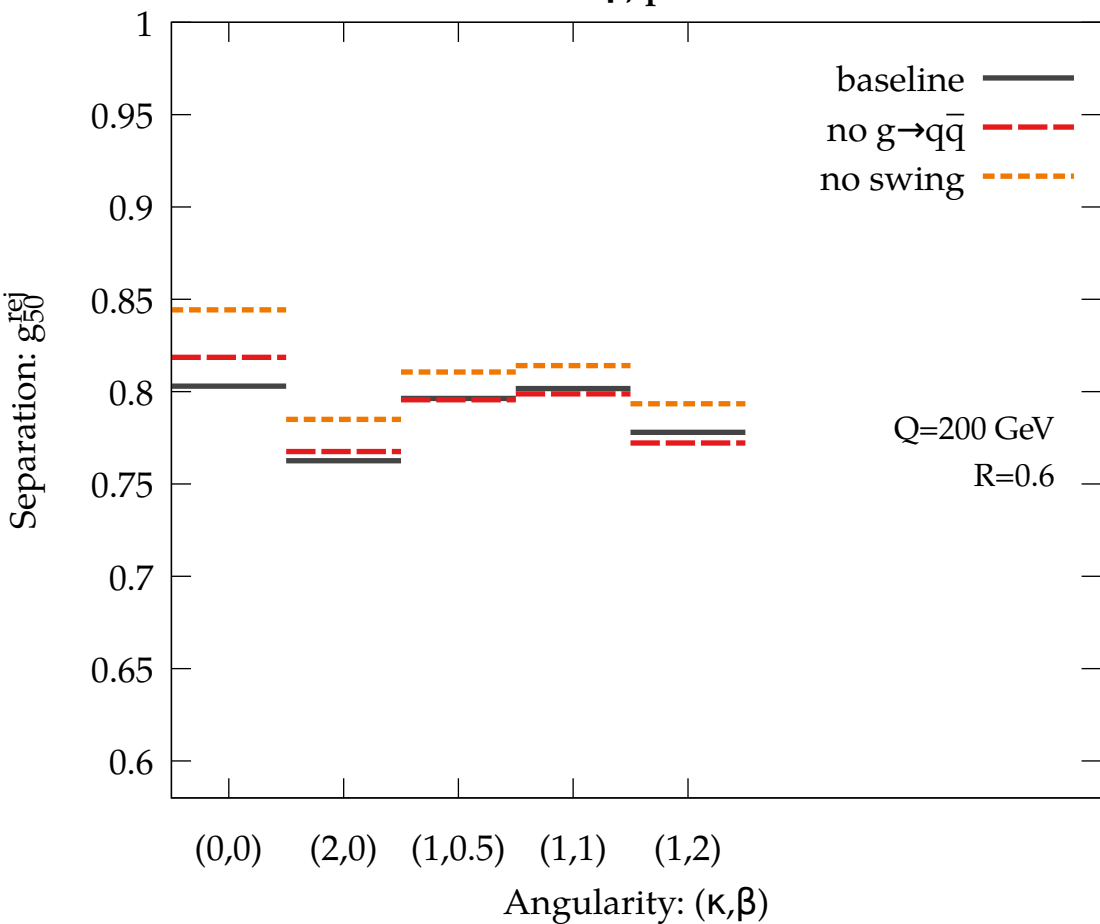

# Ariadne 5.0.β, parton-level

Separation:  $s^{\text{rej}}$

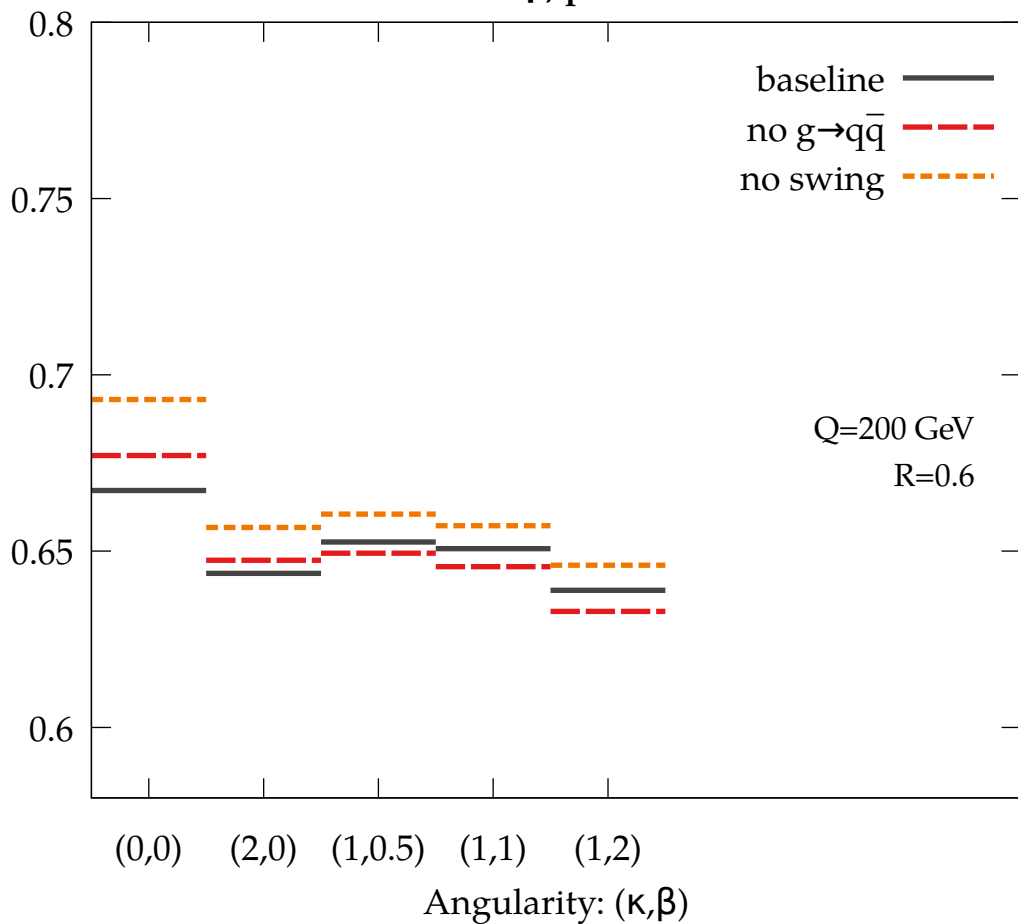

Supplement: Supplementary file 20 [file quarkgluon_fig_I2_R6_parton_ariadne.pdf]
